# Supplementary material for: Accounting for Seasonality in Extreme Sea Level Estimation
Source: arXiv:2207.09870 source file (2022-07-20)
Supplement: Supplementary file 1 [file suppfig.tex]

%%%%%%%%%%%%%%%%%%%%%%%%%%%%%%%%%%%%%%%%%%%%%%%%%%%%%%%%%%%%%%%%%%%%%%%%%%%%%%%%%%%%%%%%%%%%%%%%%%%%%% SUPP FIGS %%%%%%%%%%%%%%%%%%%%%%%%%%%%%%%%%%%%%%%%%
\newpage
\section{Supplementary Figures}

%\subsection{Skew Surge and Peak Tide Seasonality}

\begin{figure}[h]
    \centering
    \includegraphics[width=0.49\textwidth]{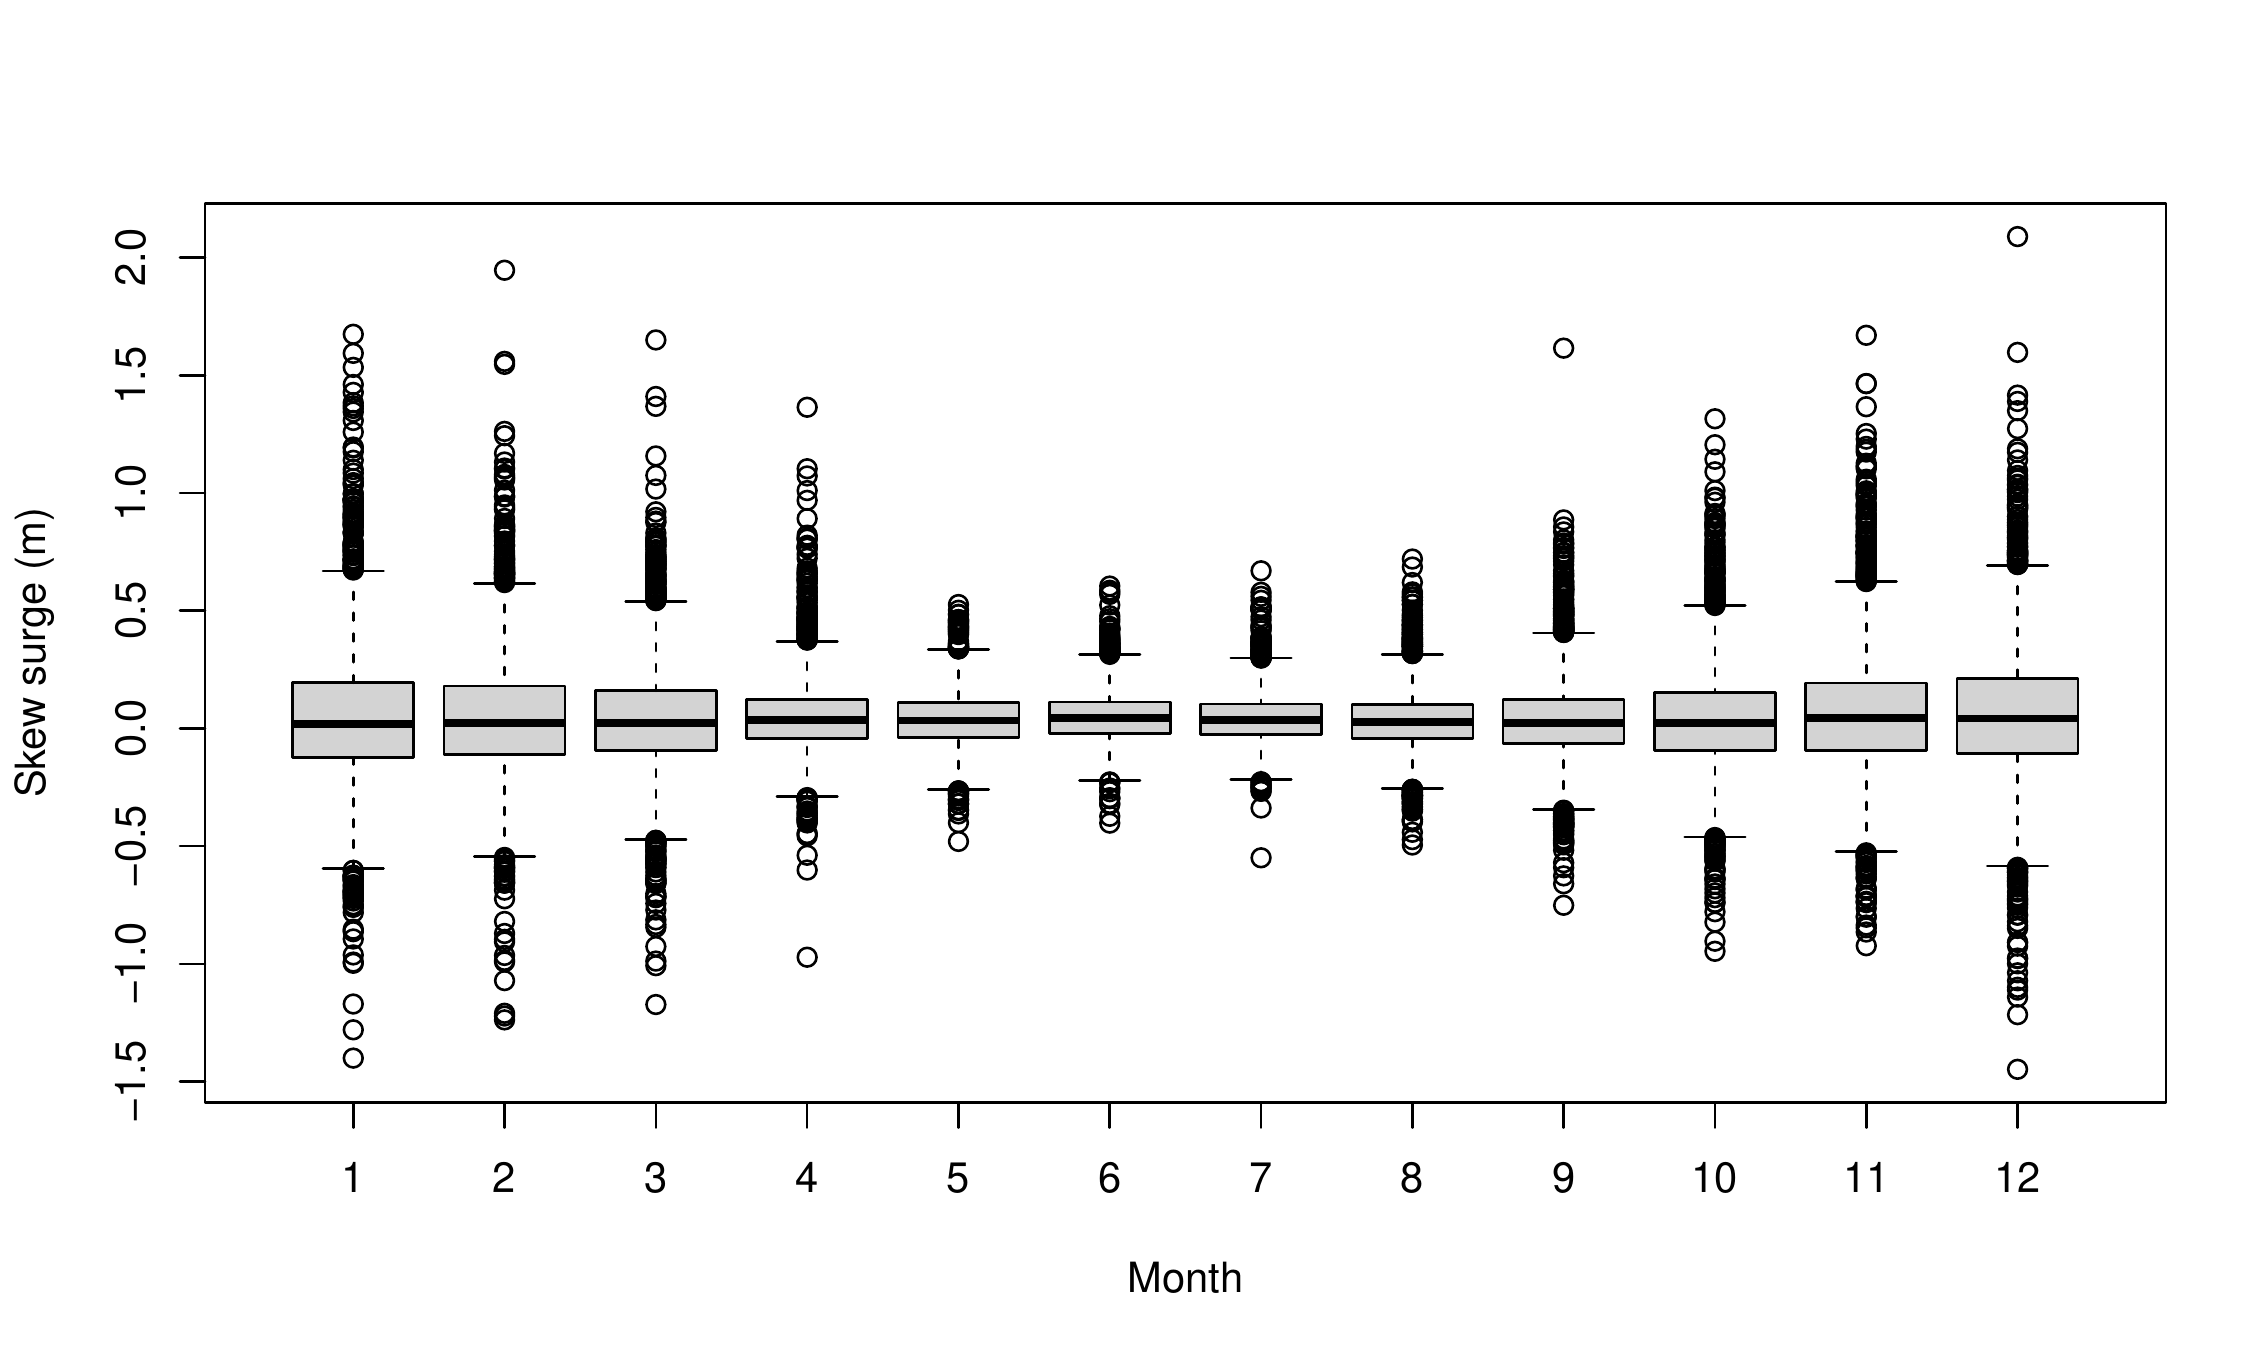}    \includegraphics[width=0.49\textwidth]{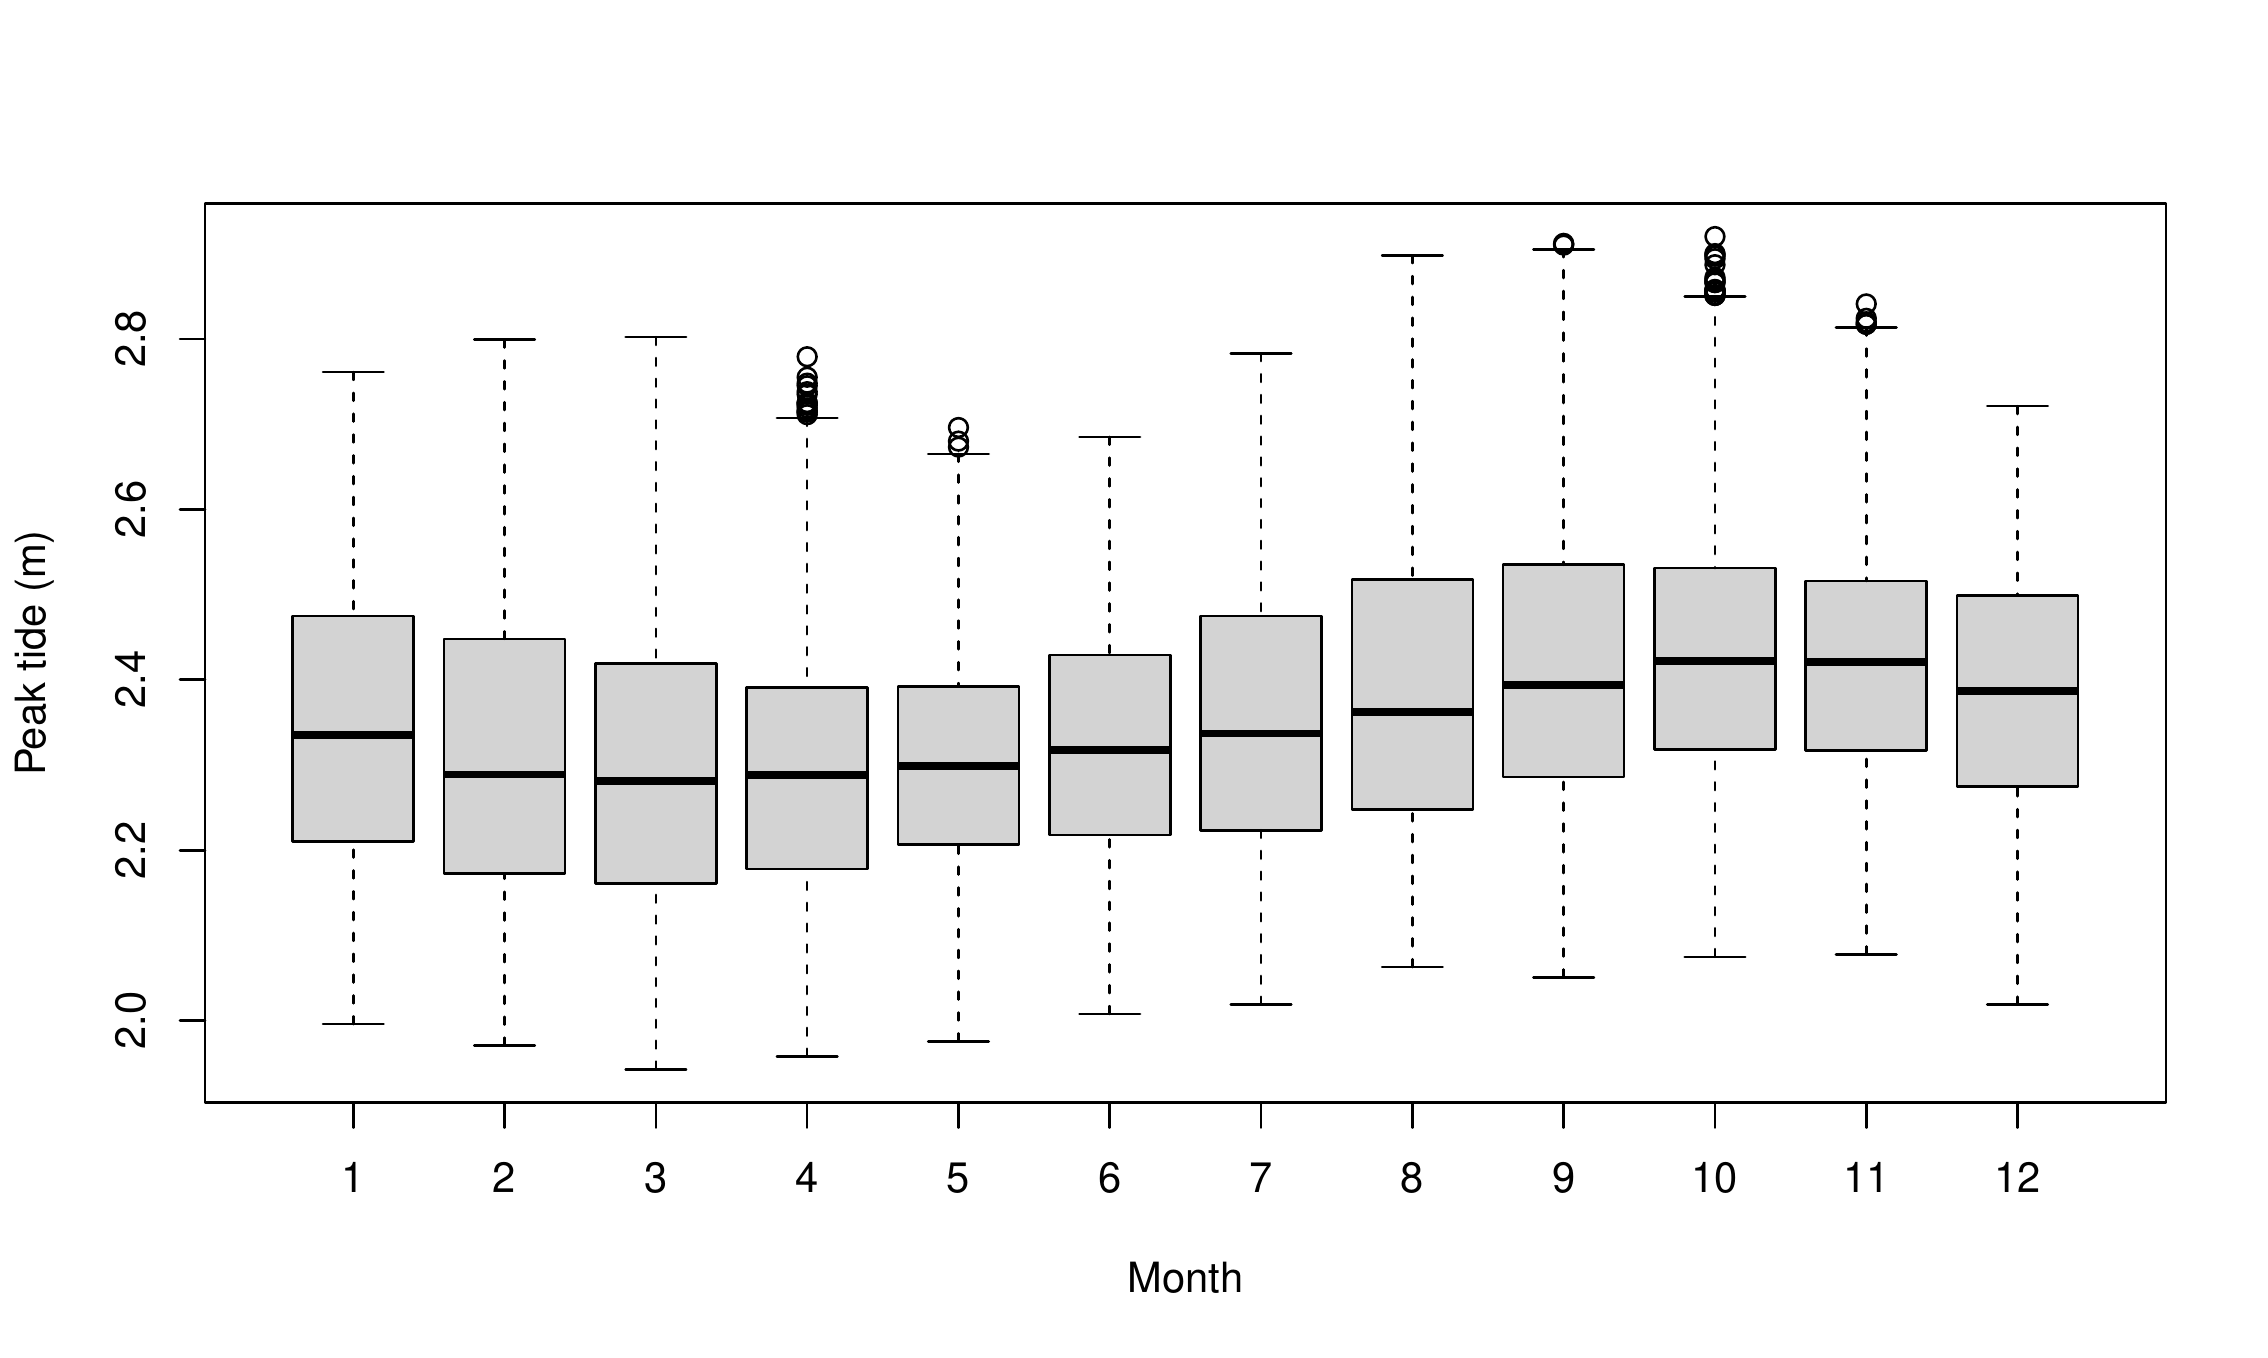}    \includegraphics[width=0.49\textwidth]{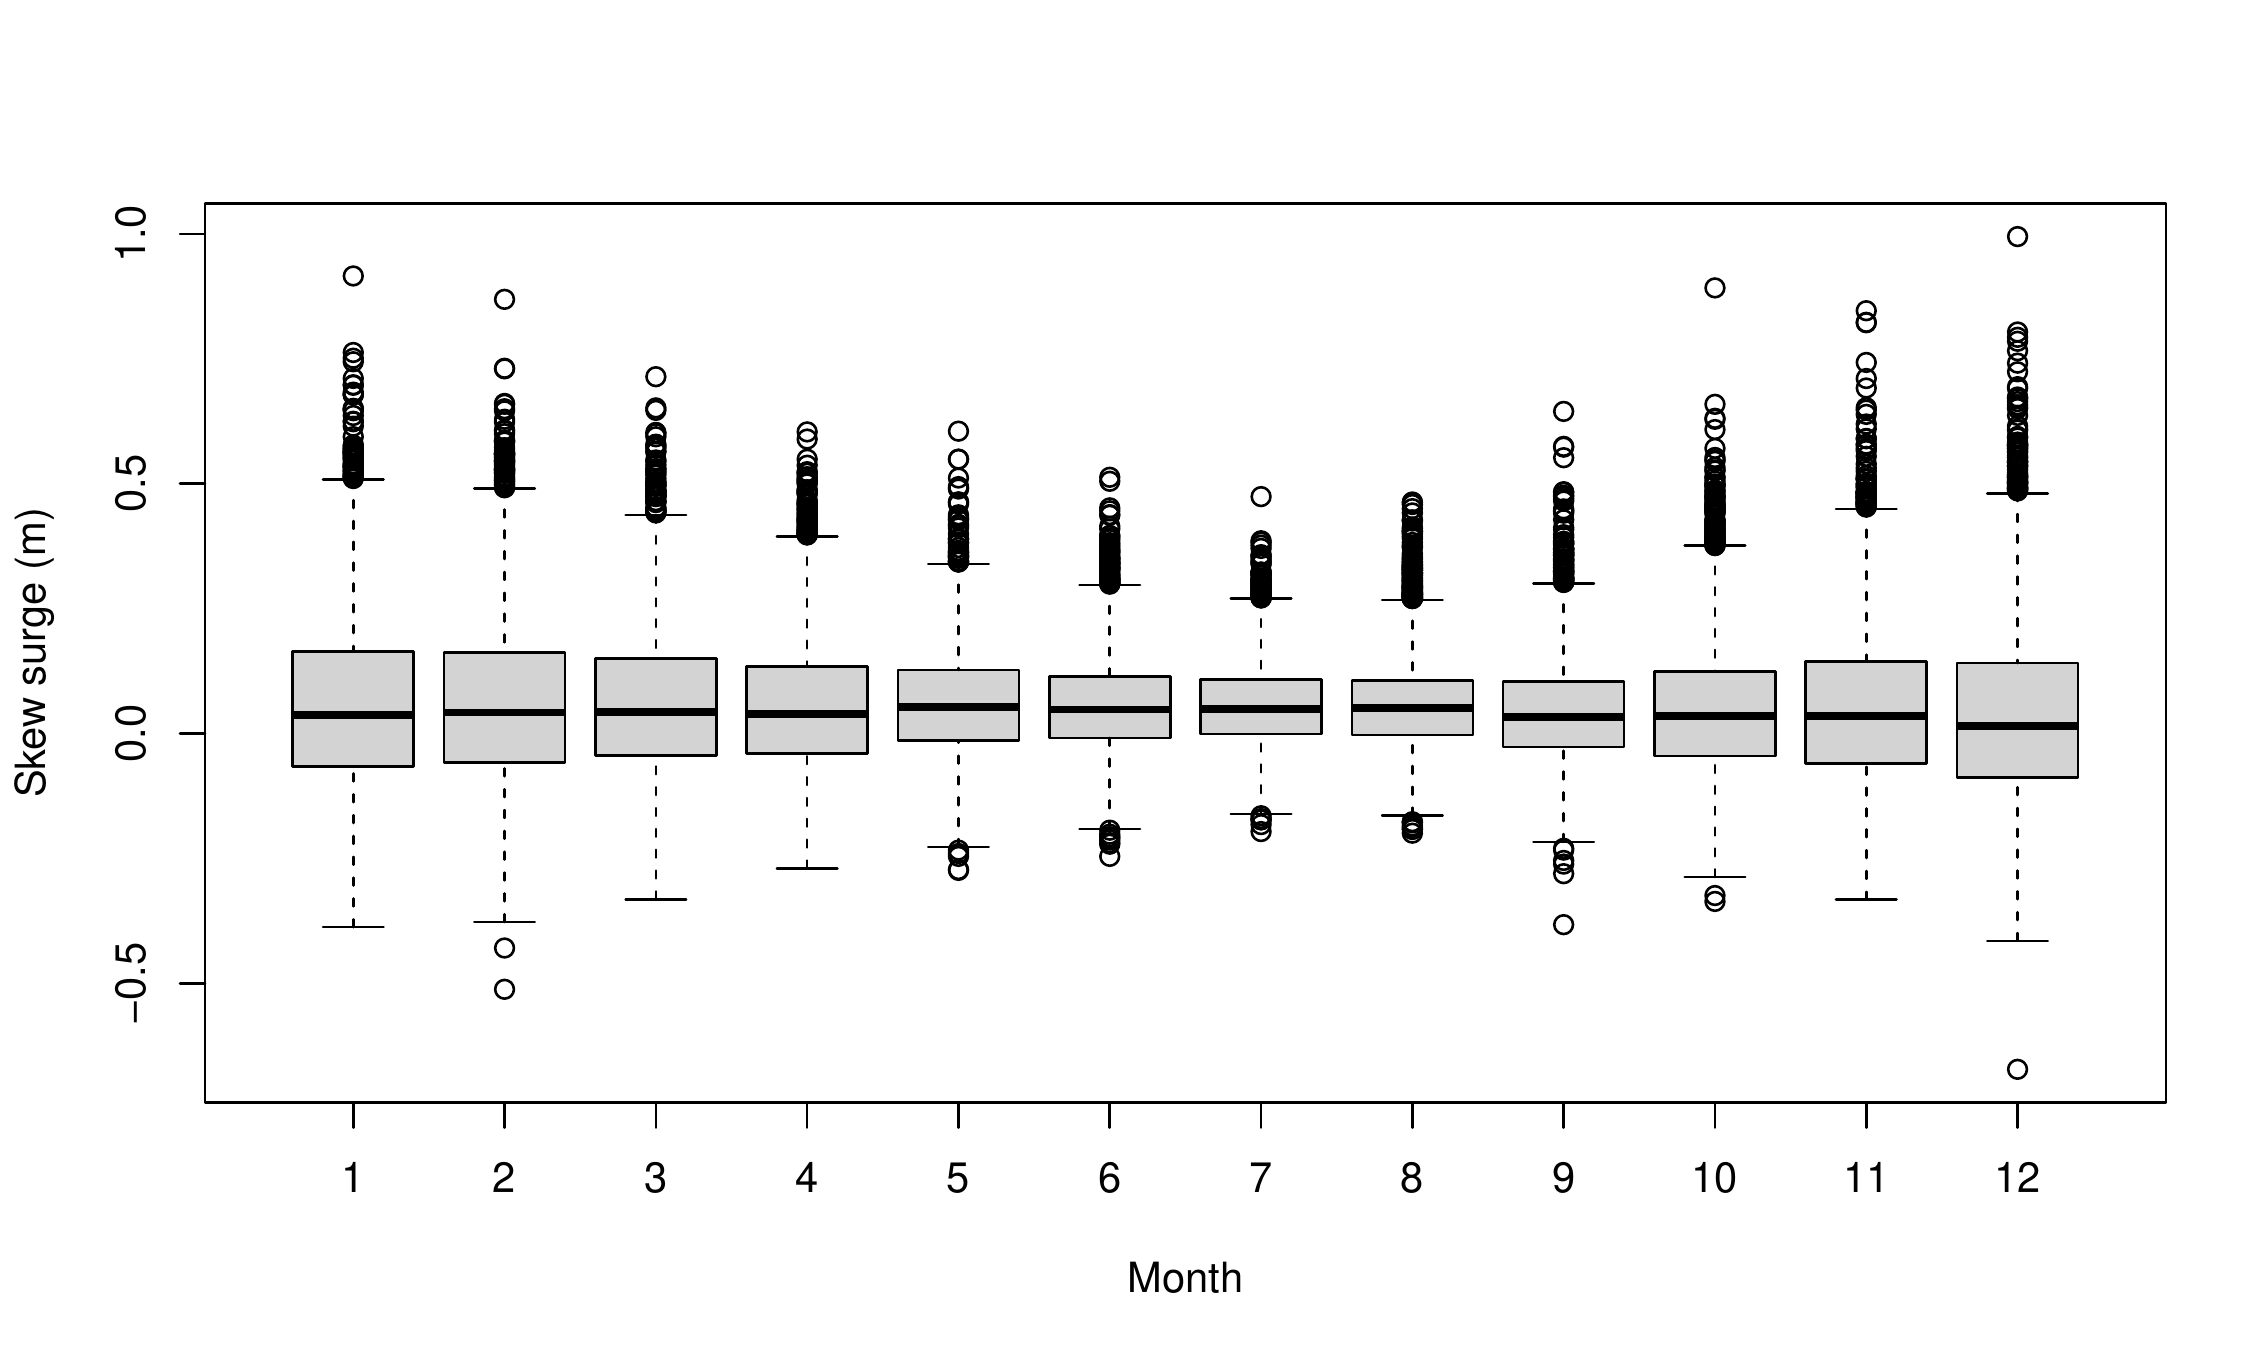}    \includegraphics[width=0.49\textwidth]{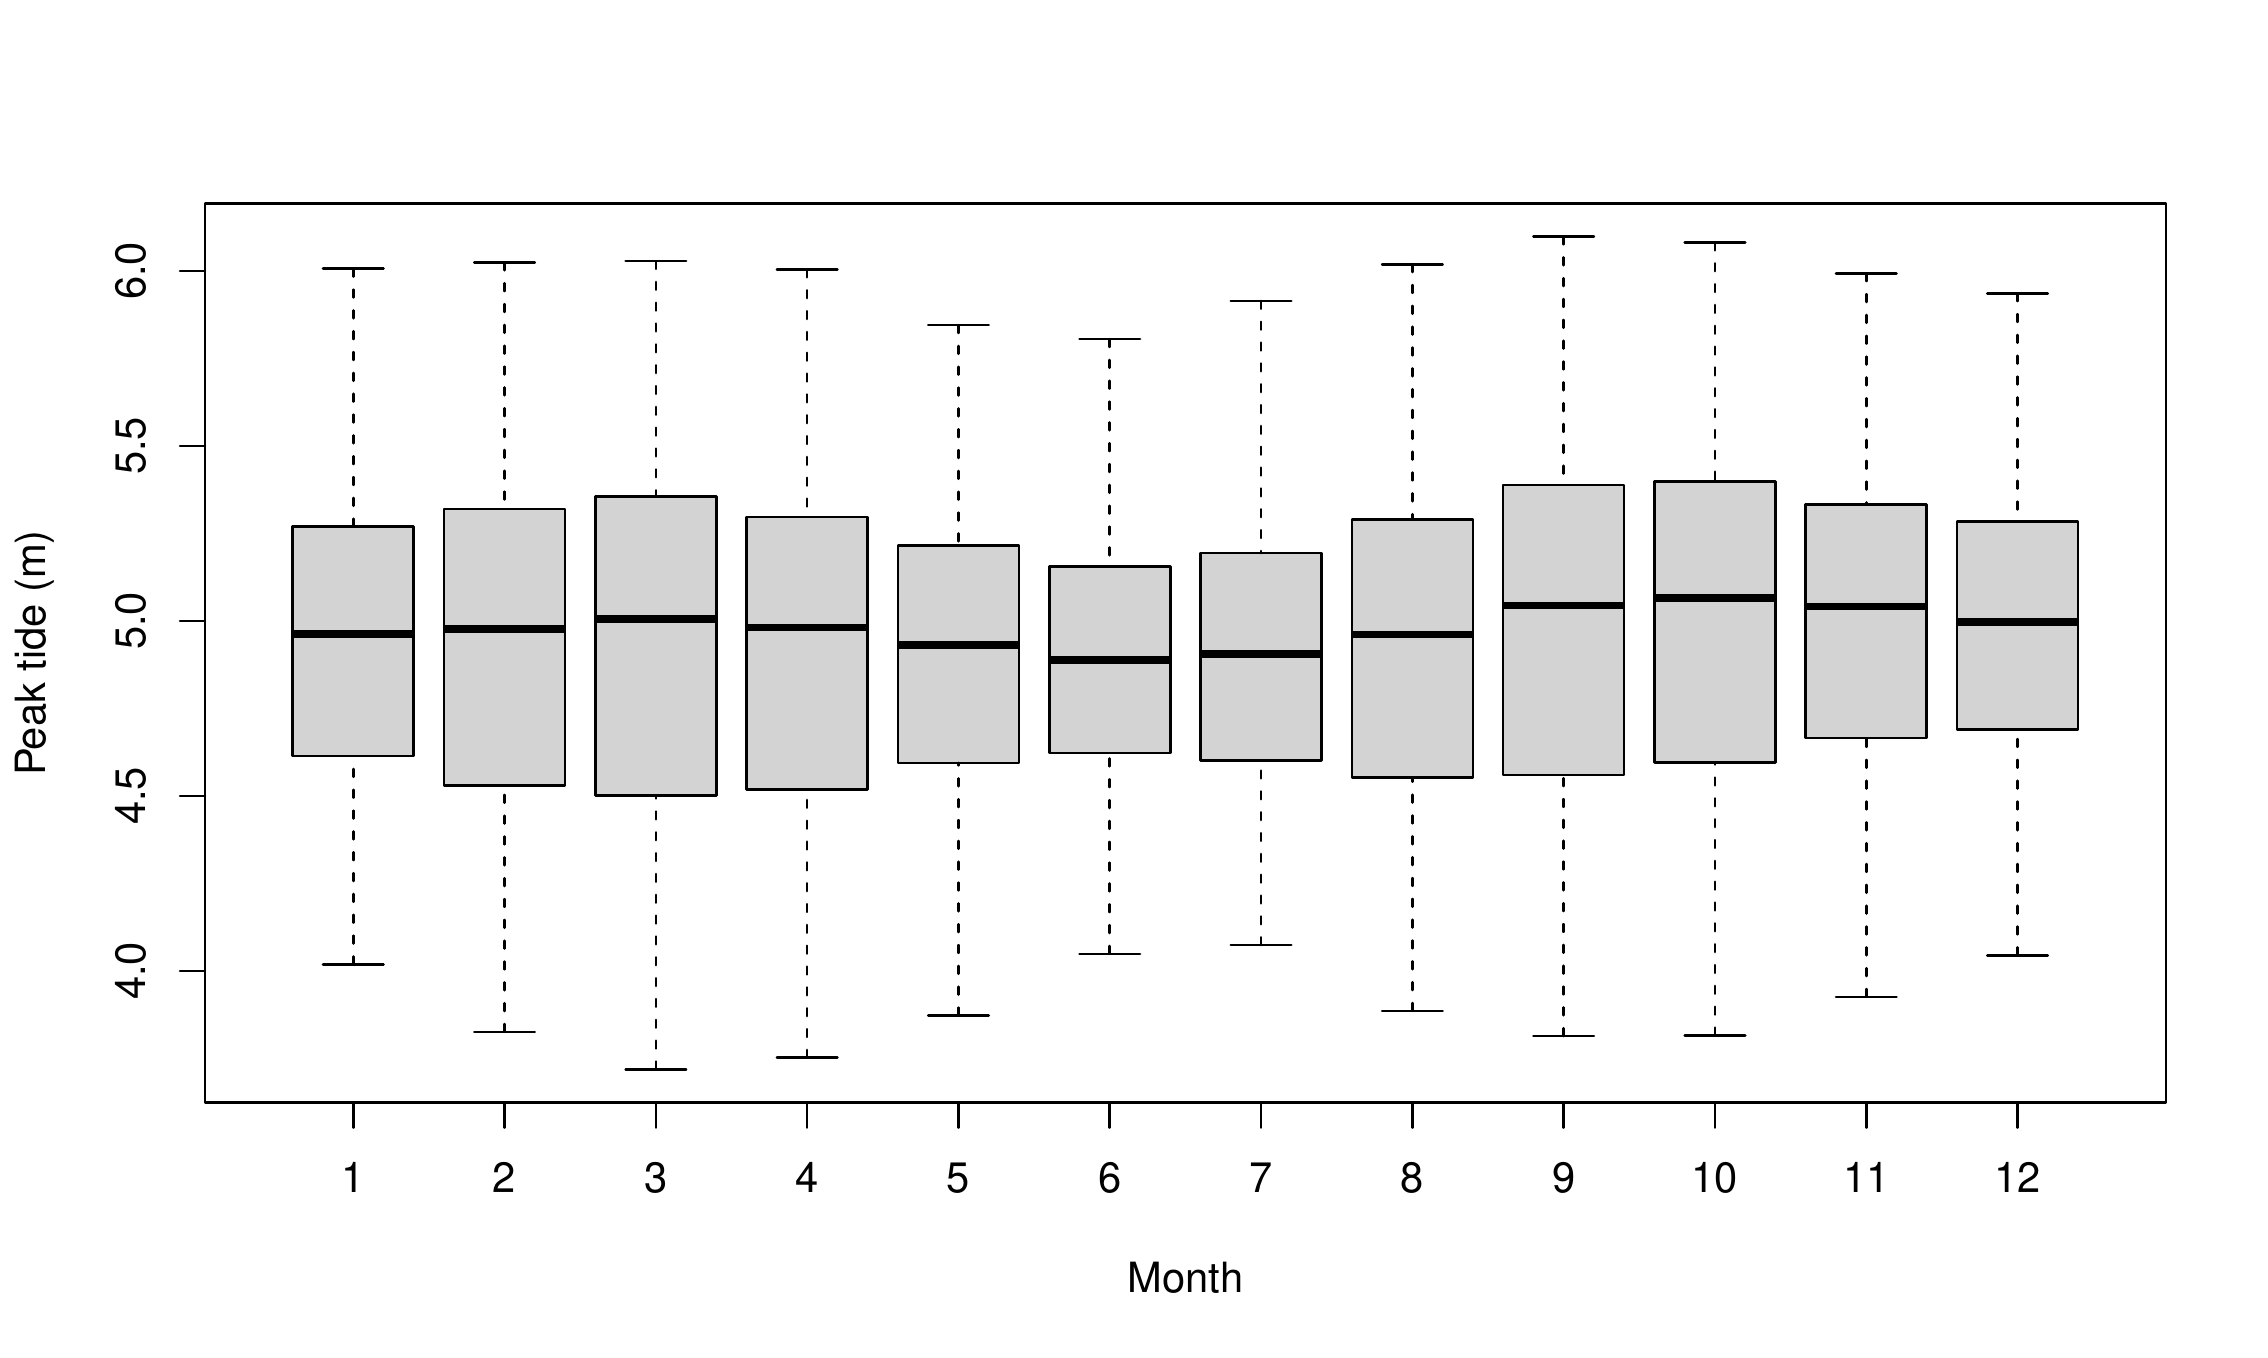}
    \includegraphics[width=0.49\textwidth]{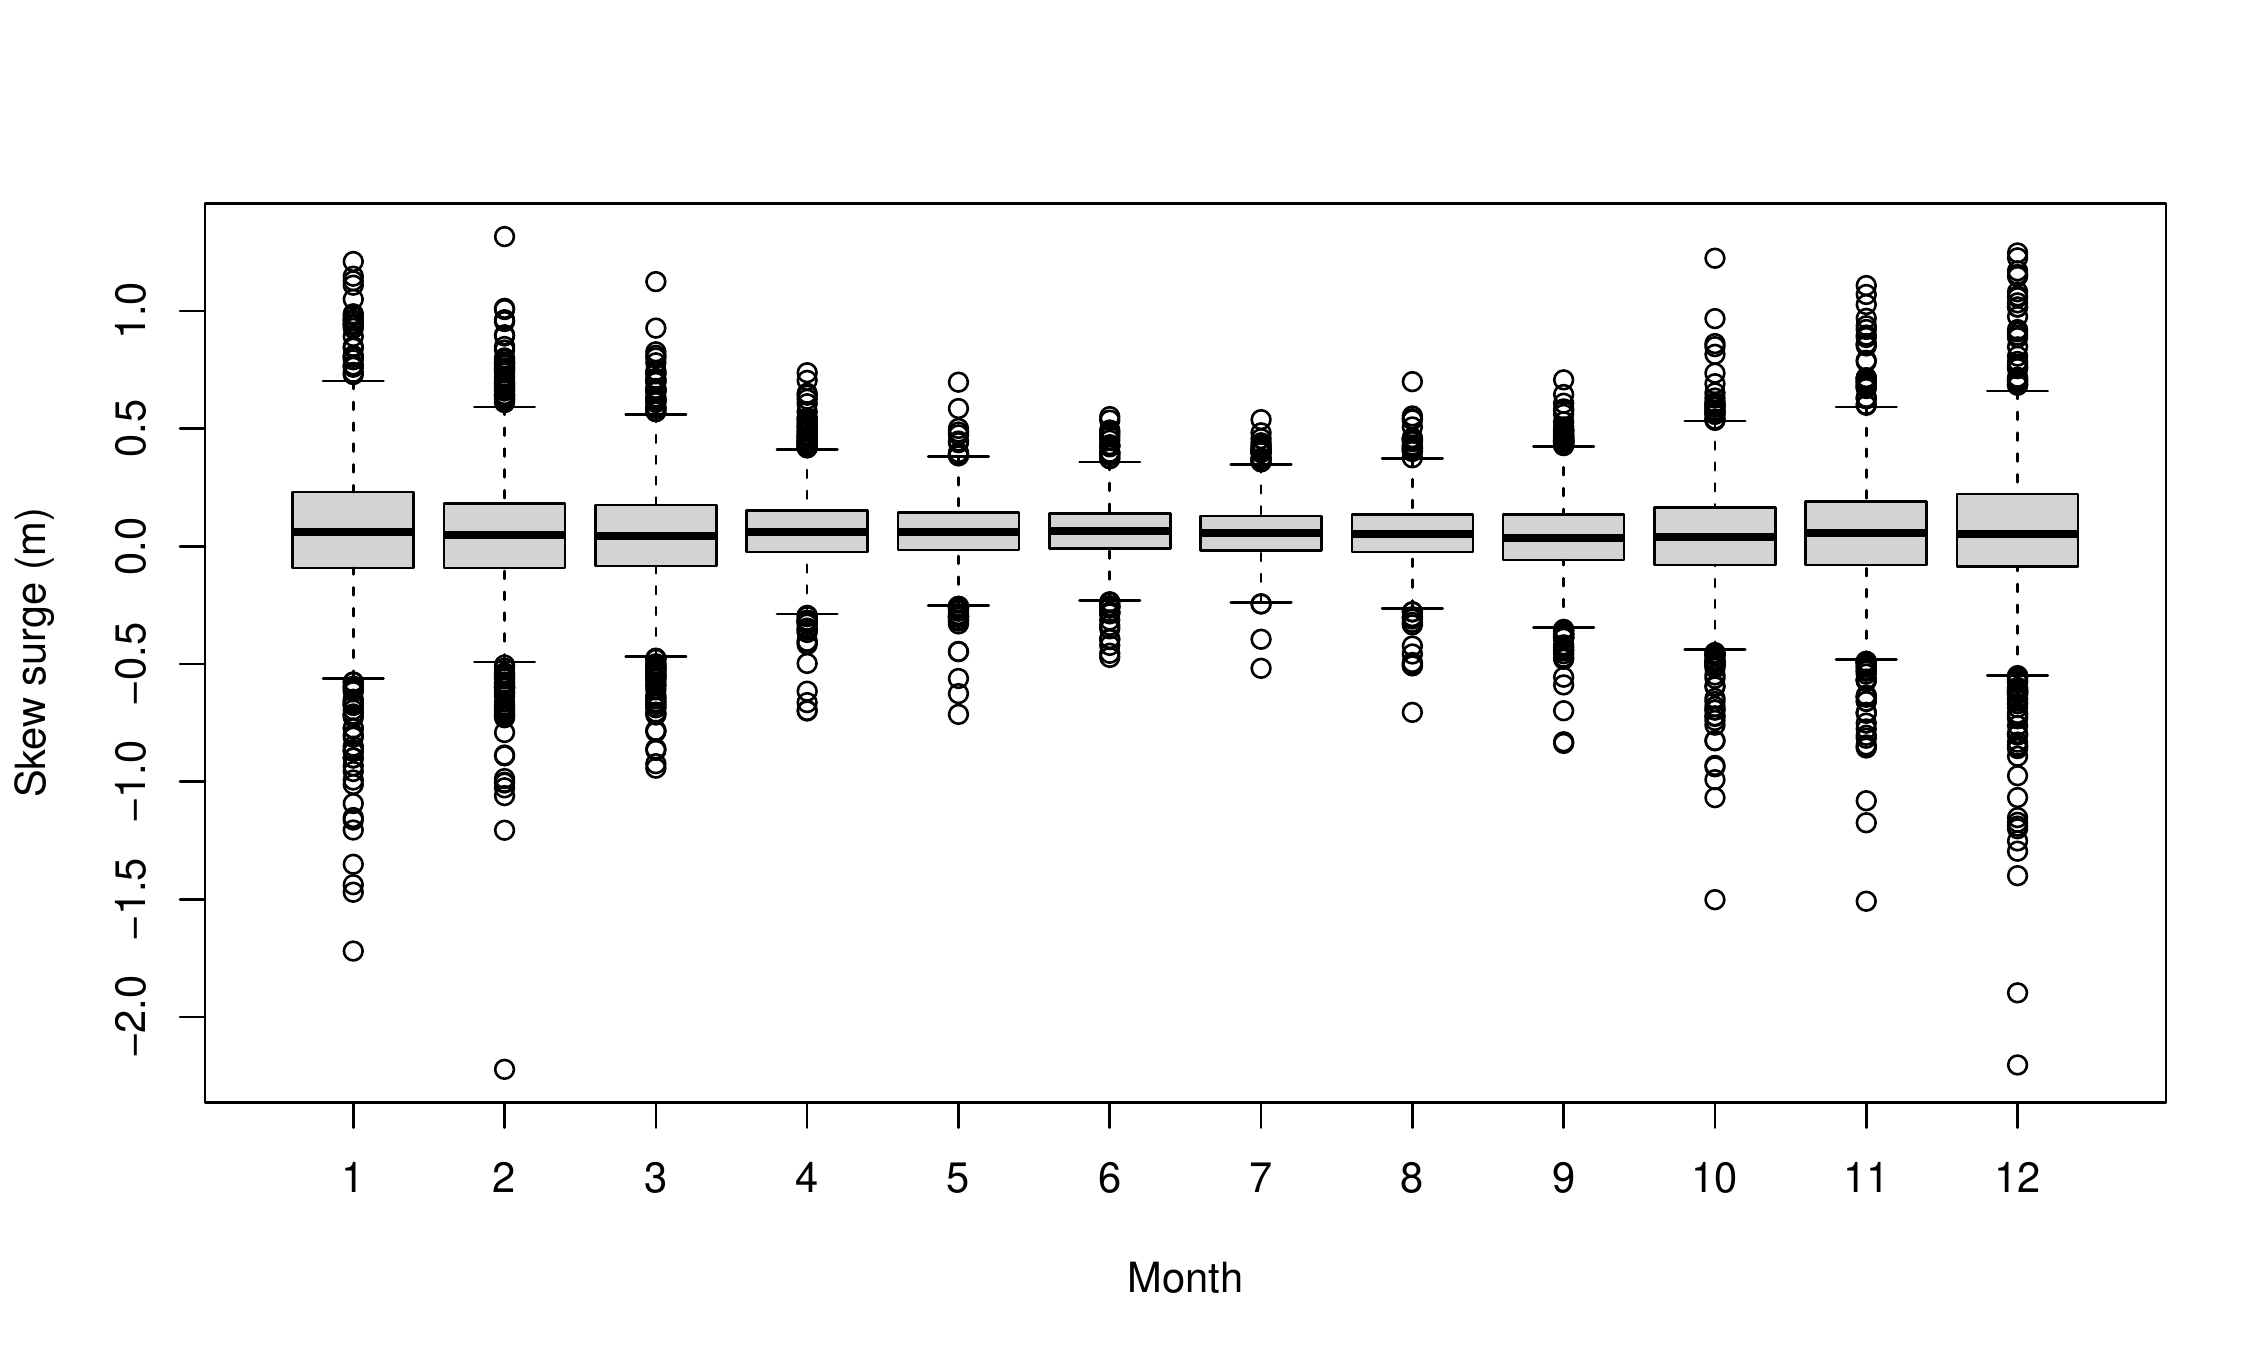}    \includegraphics[width=0.49\textwidth]{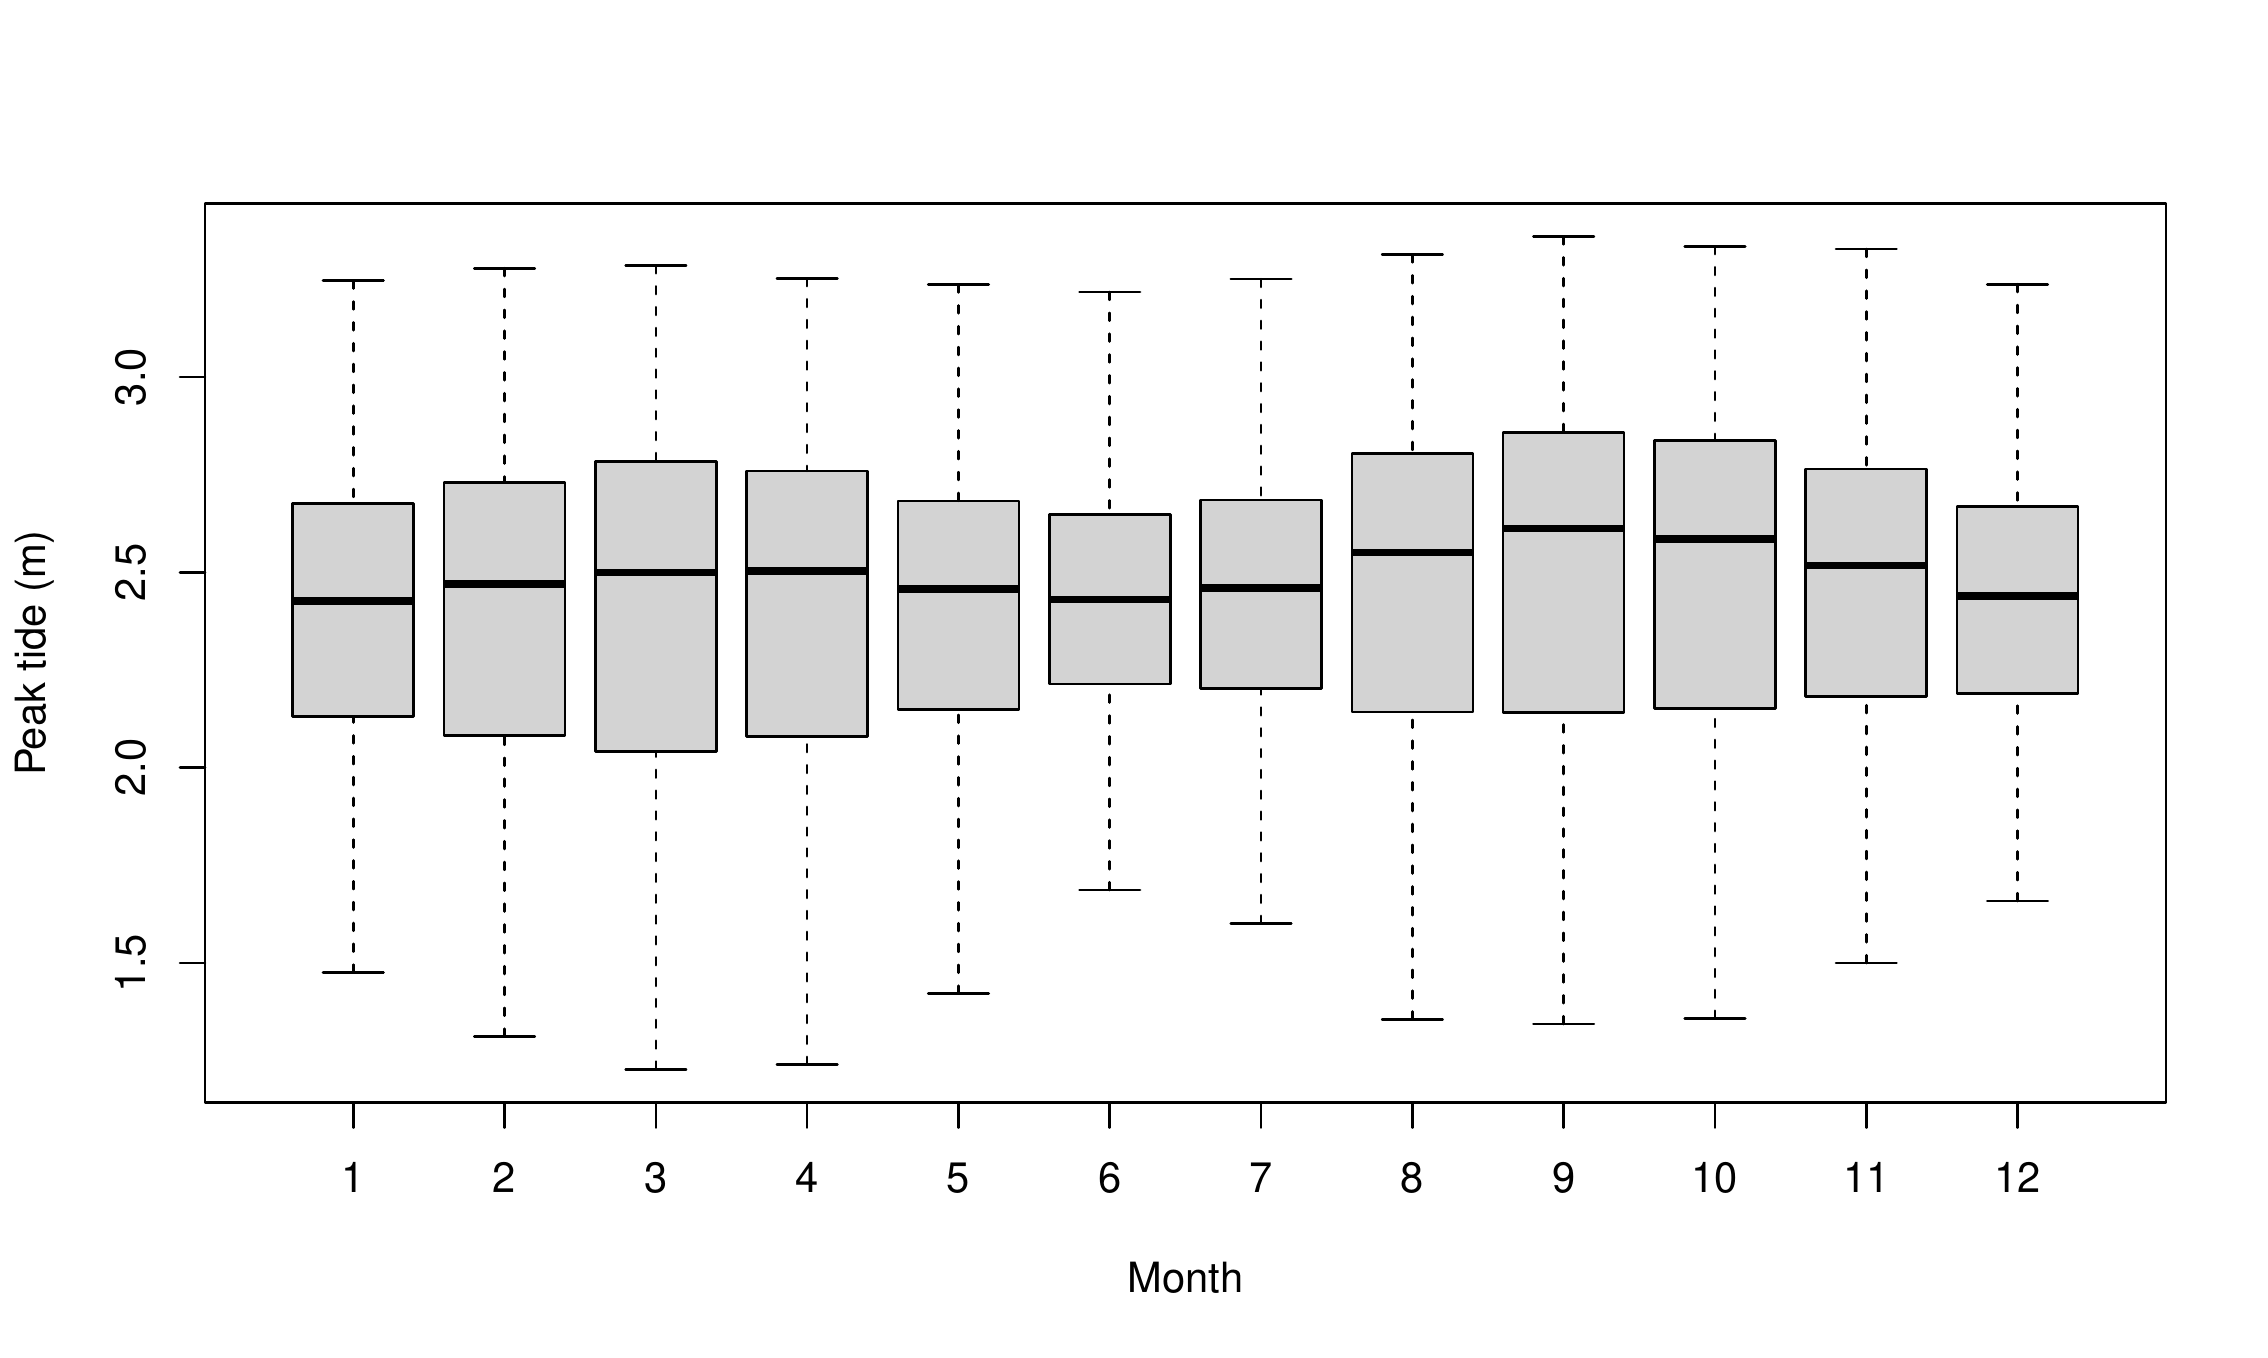}
    \caption{Skew surge (left) and peak tide (right) monthly boxplots at Lowestoft (top), Newlyn (middle) and Sheerness (bottom)}
    \label{ss_mt_bps_all}
\end{figure}

%In Section \ref{ss_seasonality}, we discussed the within-year seasonality of skew surge and peak tide. At Heysham (Figure \ref{ss_mt_bps_HEY}), peak tides are greatest in March and September. Figure \ref{ss_mt_bps_all} shows the a boxplot per month for the distribution of skew surge and peak tide at Lowestoft, Newlyn, and Sheerness. We observe the same seasonality for all sites. At Newlyn the autumn peak is slightly greater than the spring peak. The median of the peak tides is fairly constant across months for Heysham, Newlyn and Sheerness. However, at Lowestoft the median has a clear seasonal pattern, reaching its lowest point in March before steadily increasing to its peak in October. The upper tail of the distributions still peak in spring and autumn, but the autumn peak is significantly larger.

%Figure \ref{mt_seasonality_plot} shows the estimates of $p_j(q;R)$ defined in equation \eqref{prob}, for $R$ representing peak tides and for various quantiles $q$ at Lowestoft, Newlyn and Sheerness. We also add 95\% confidence intervals to the estimates of $p_j(0.999;R)$ at each site. A full discussion of these results is given in Section \ref{ss_seasonality}. 

\begin{figure}
    \centering
    \includegraphics[width=0.49\textwidth]{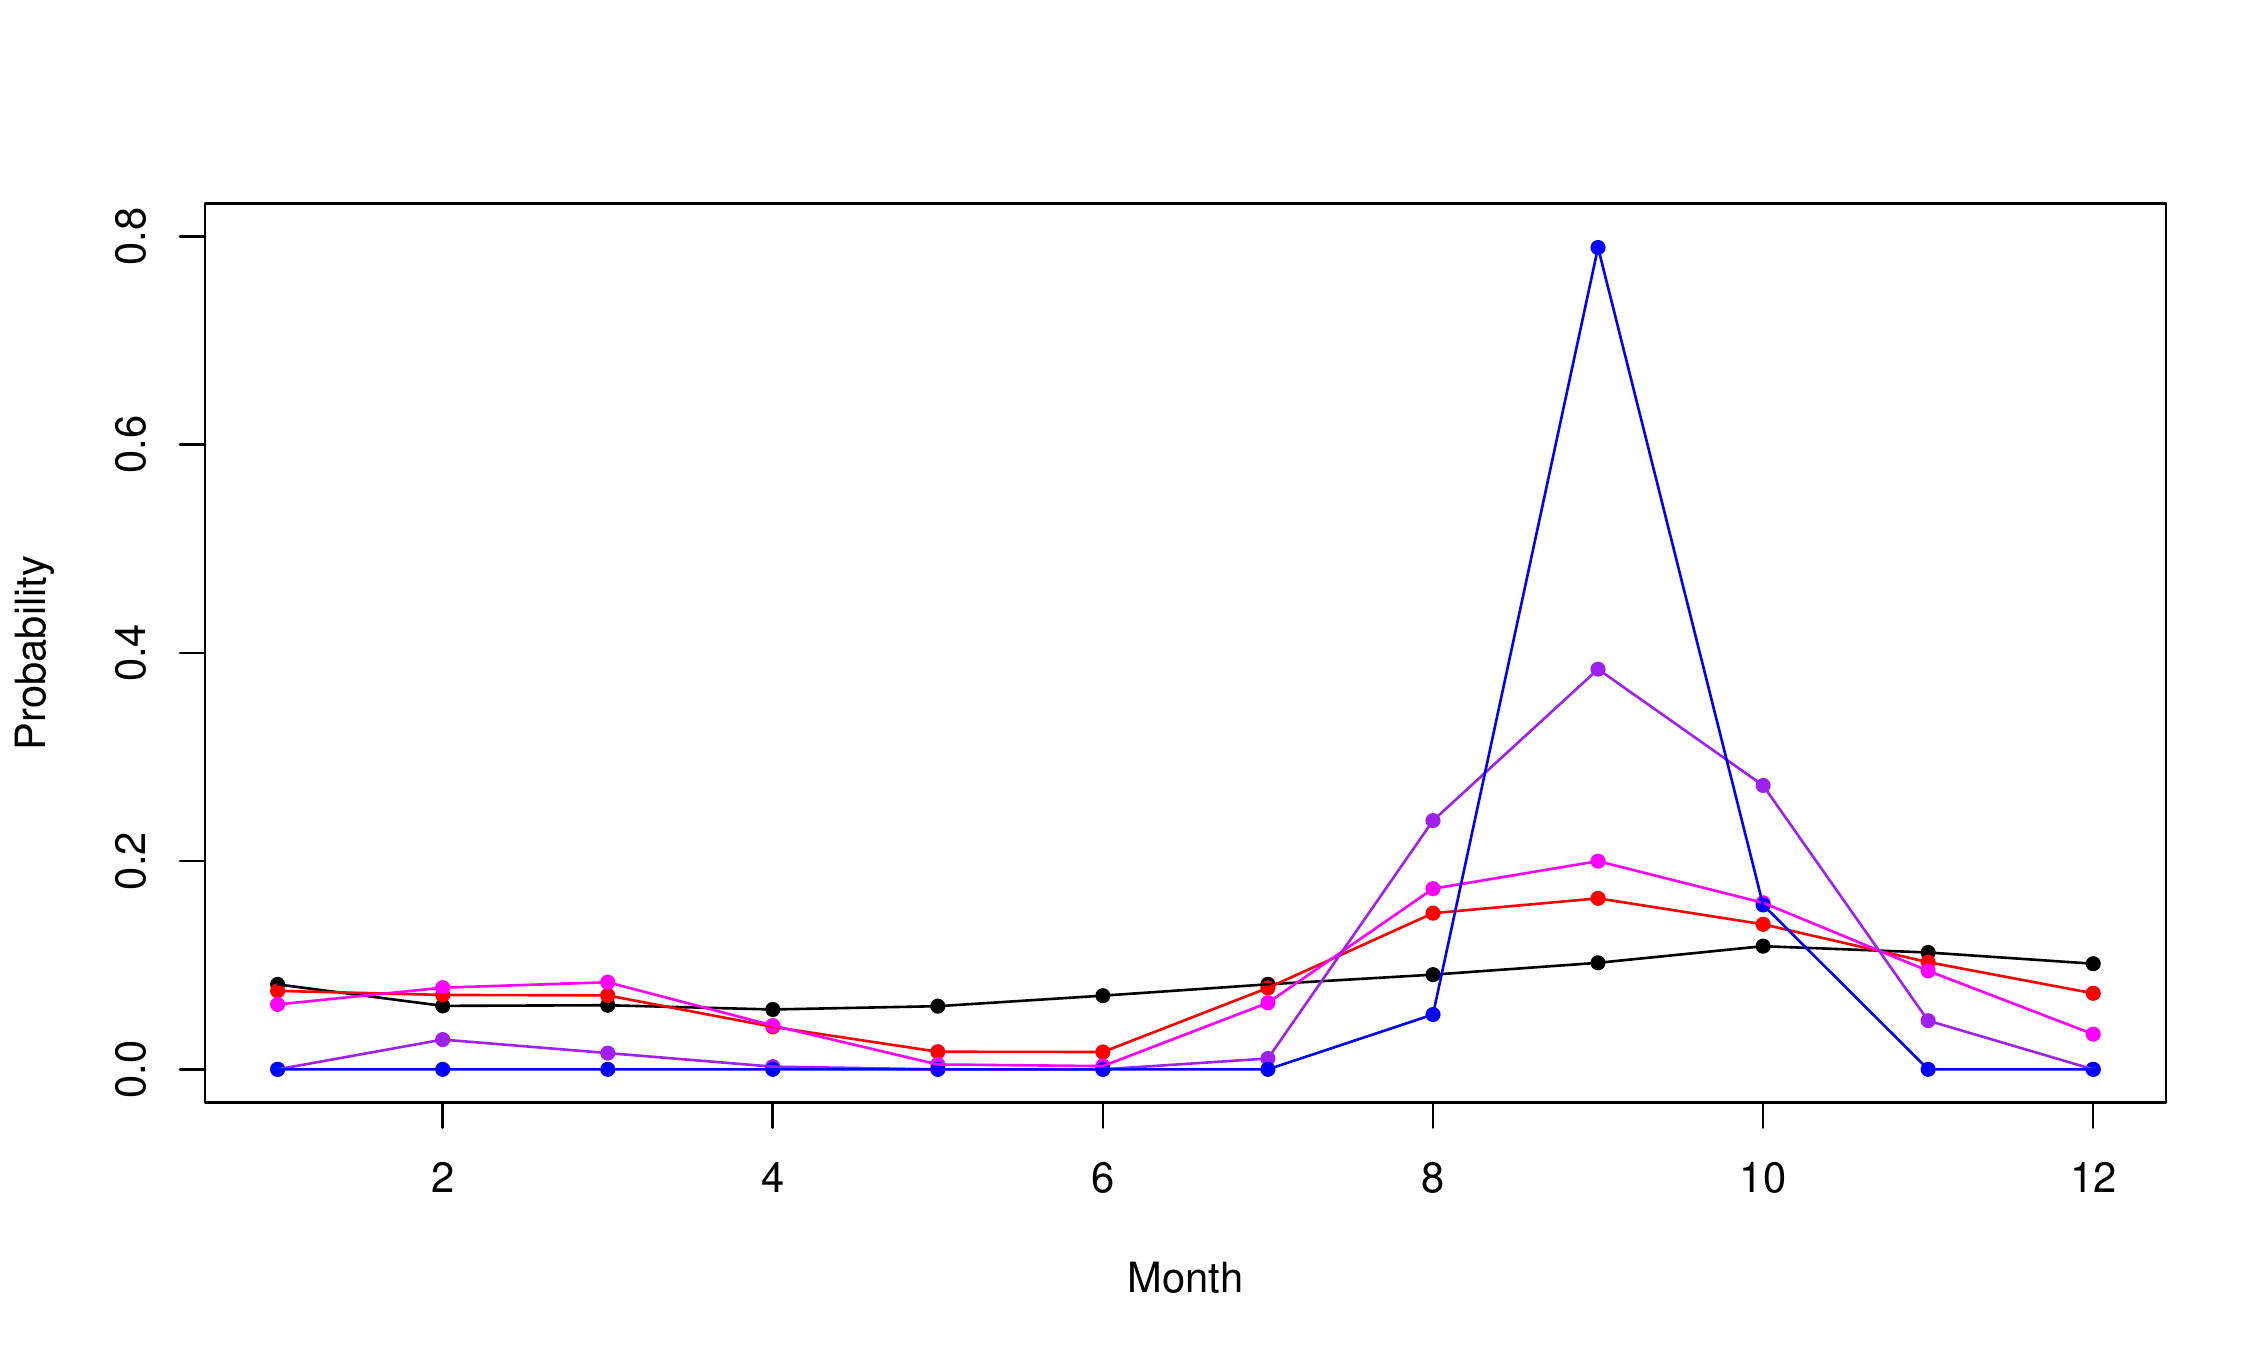}
    \includegraphics[width=0.49\textwidth]{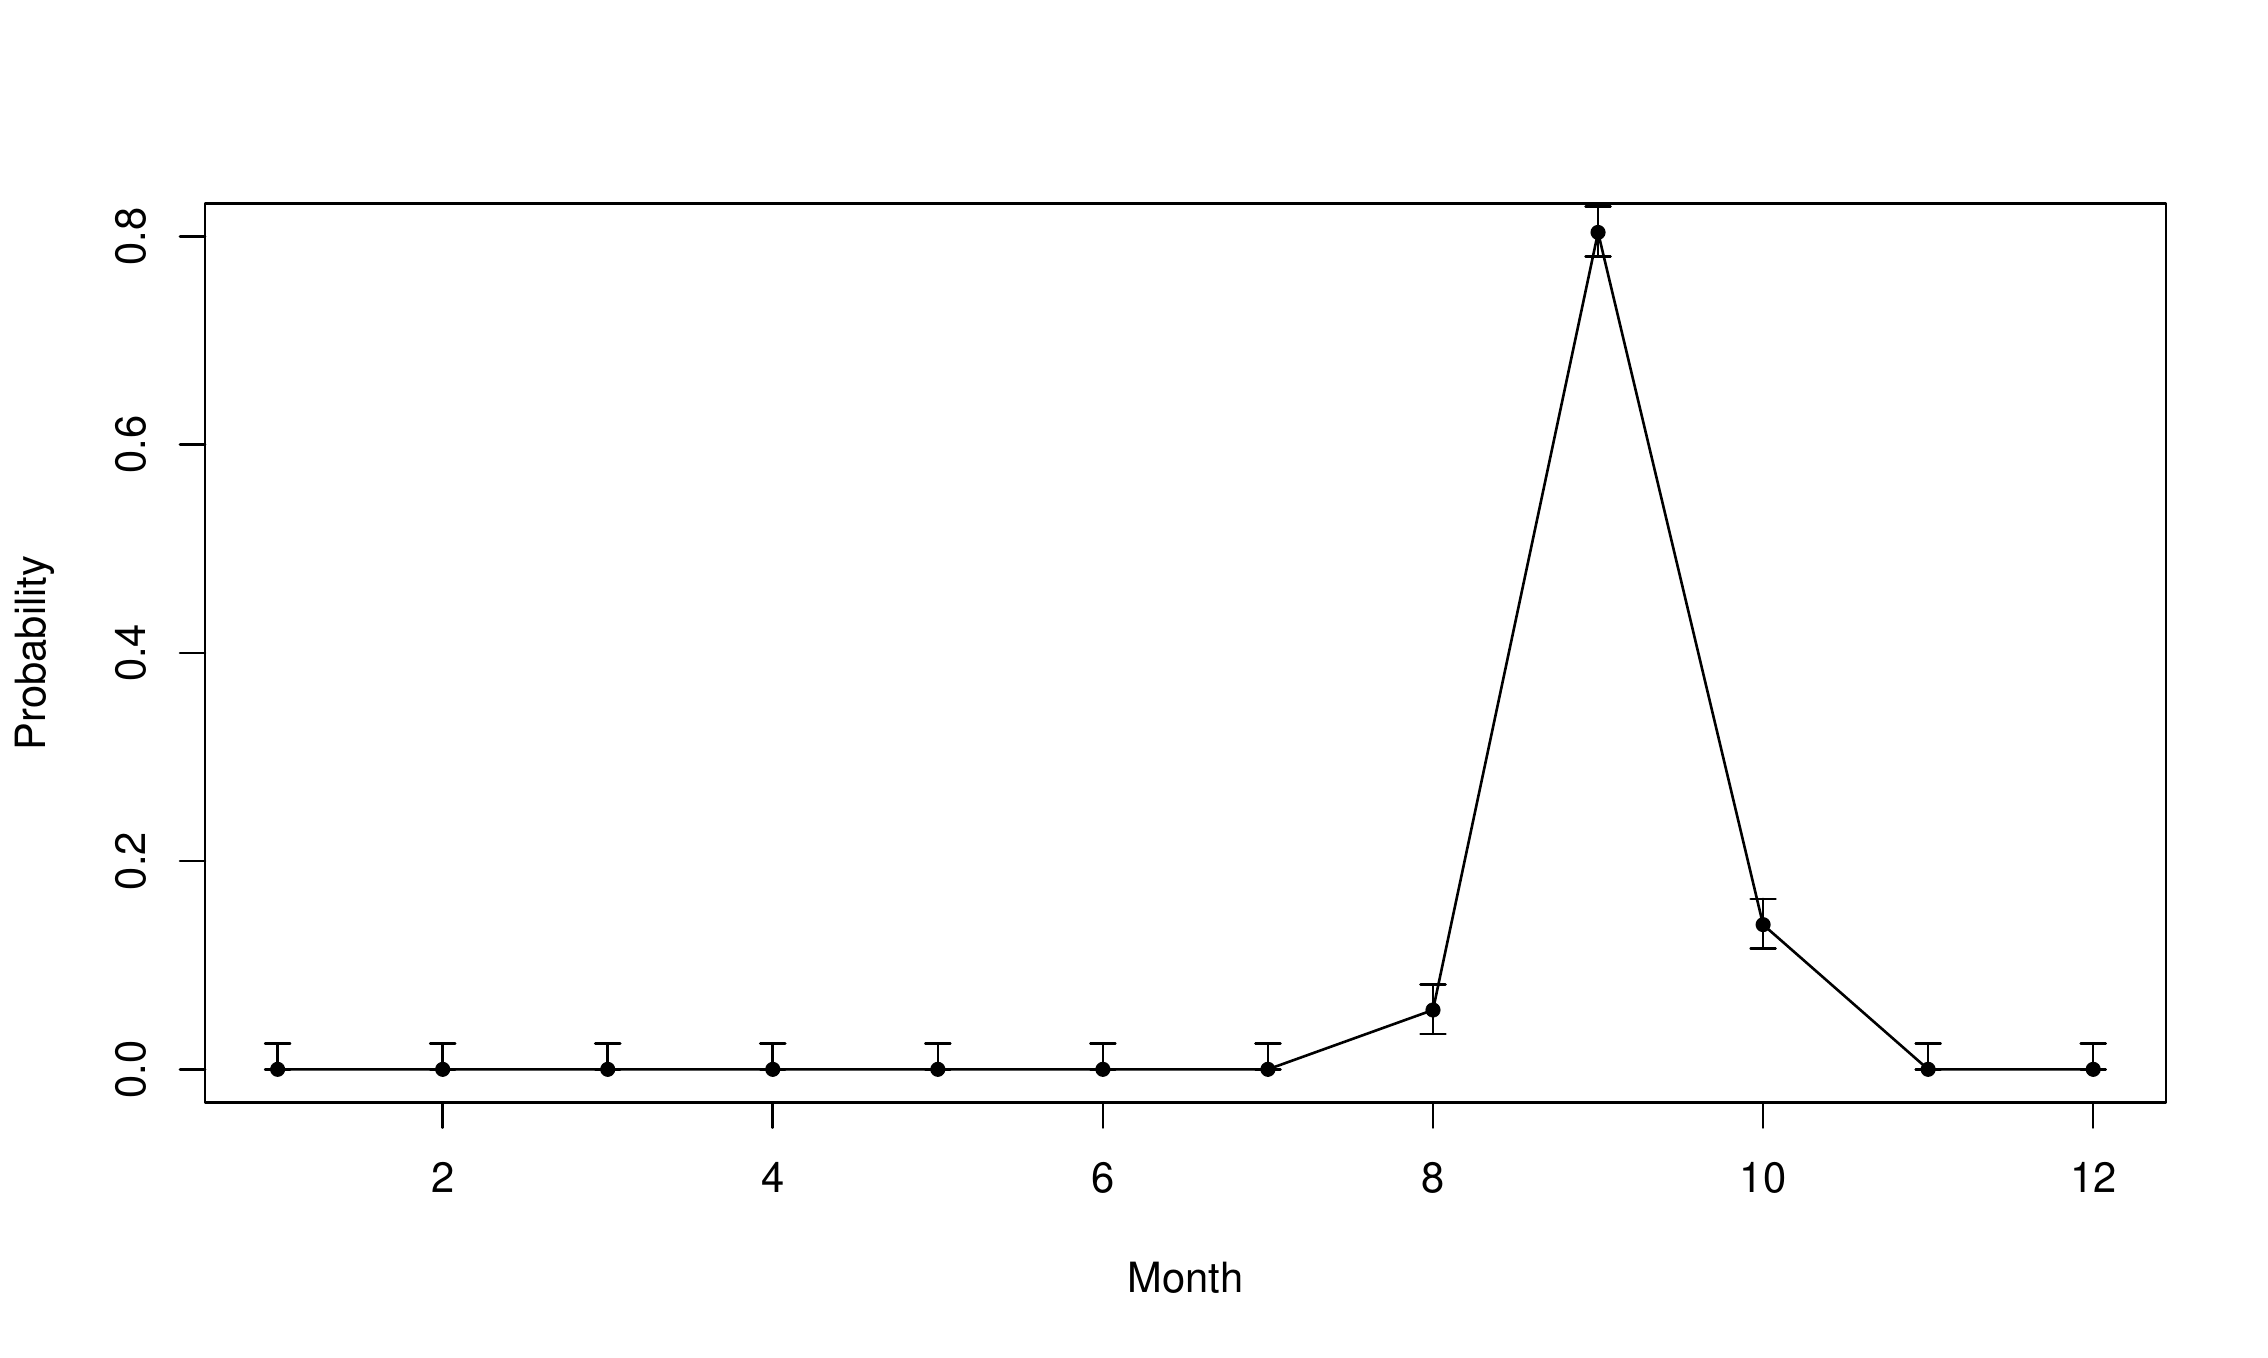}
    \includegraphics[width=0.49\textwidth]{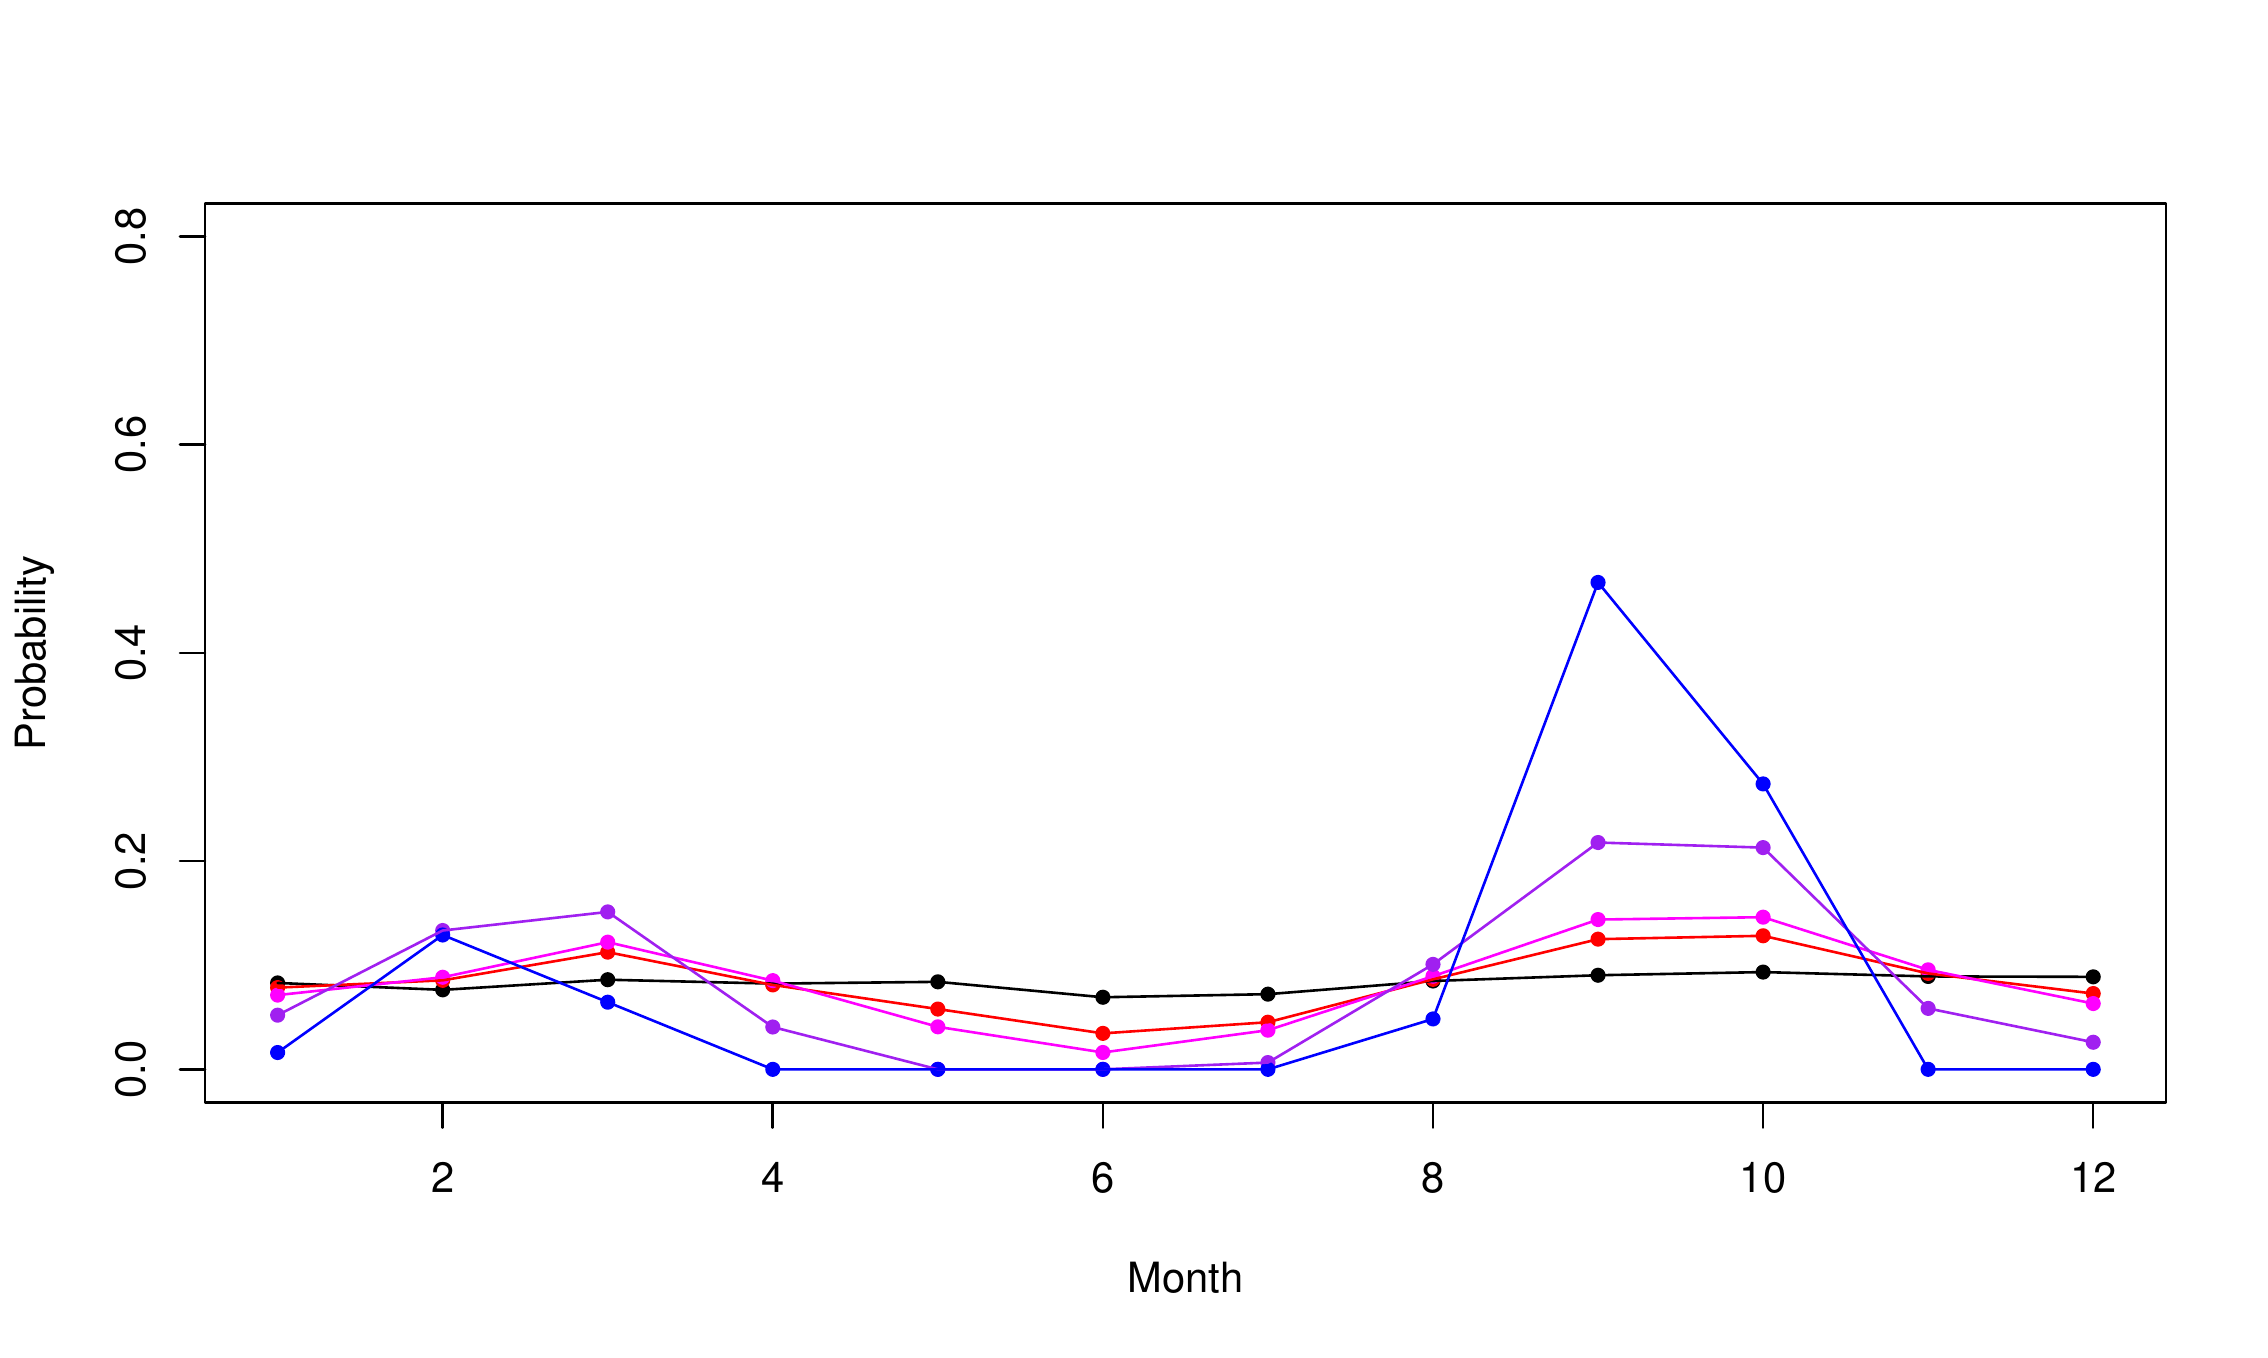}
    \includegraphics[width=0.49\textwidth]{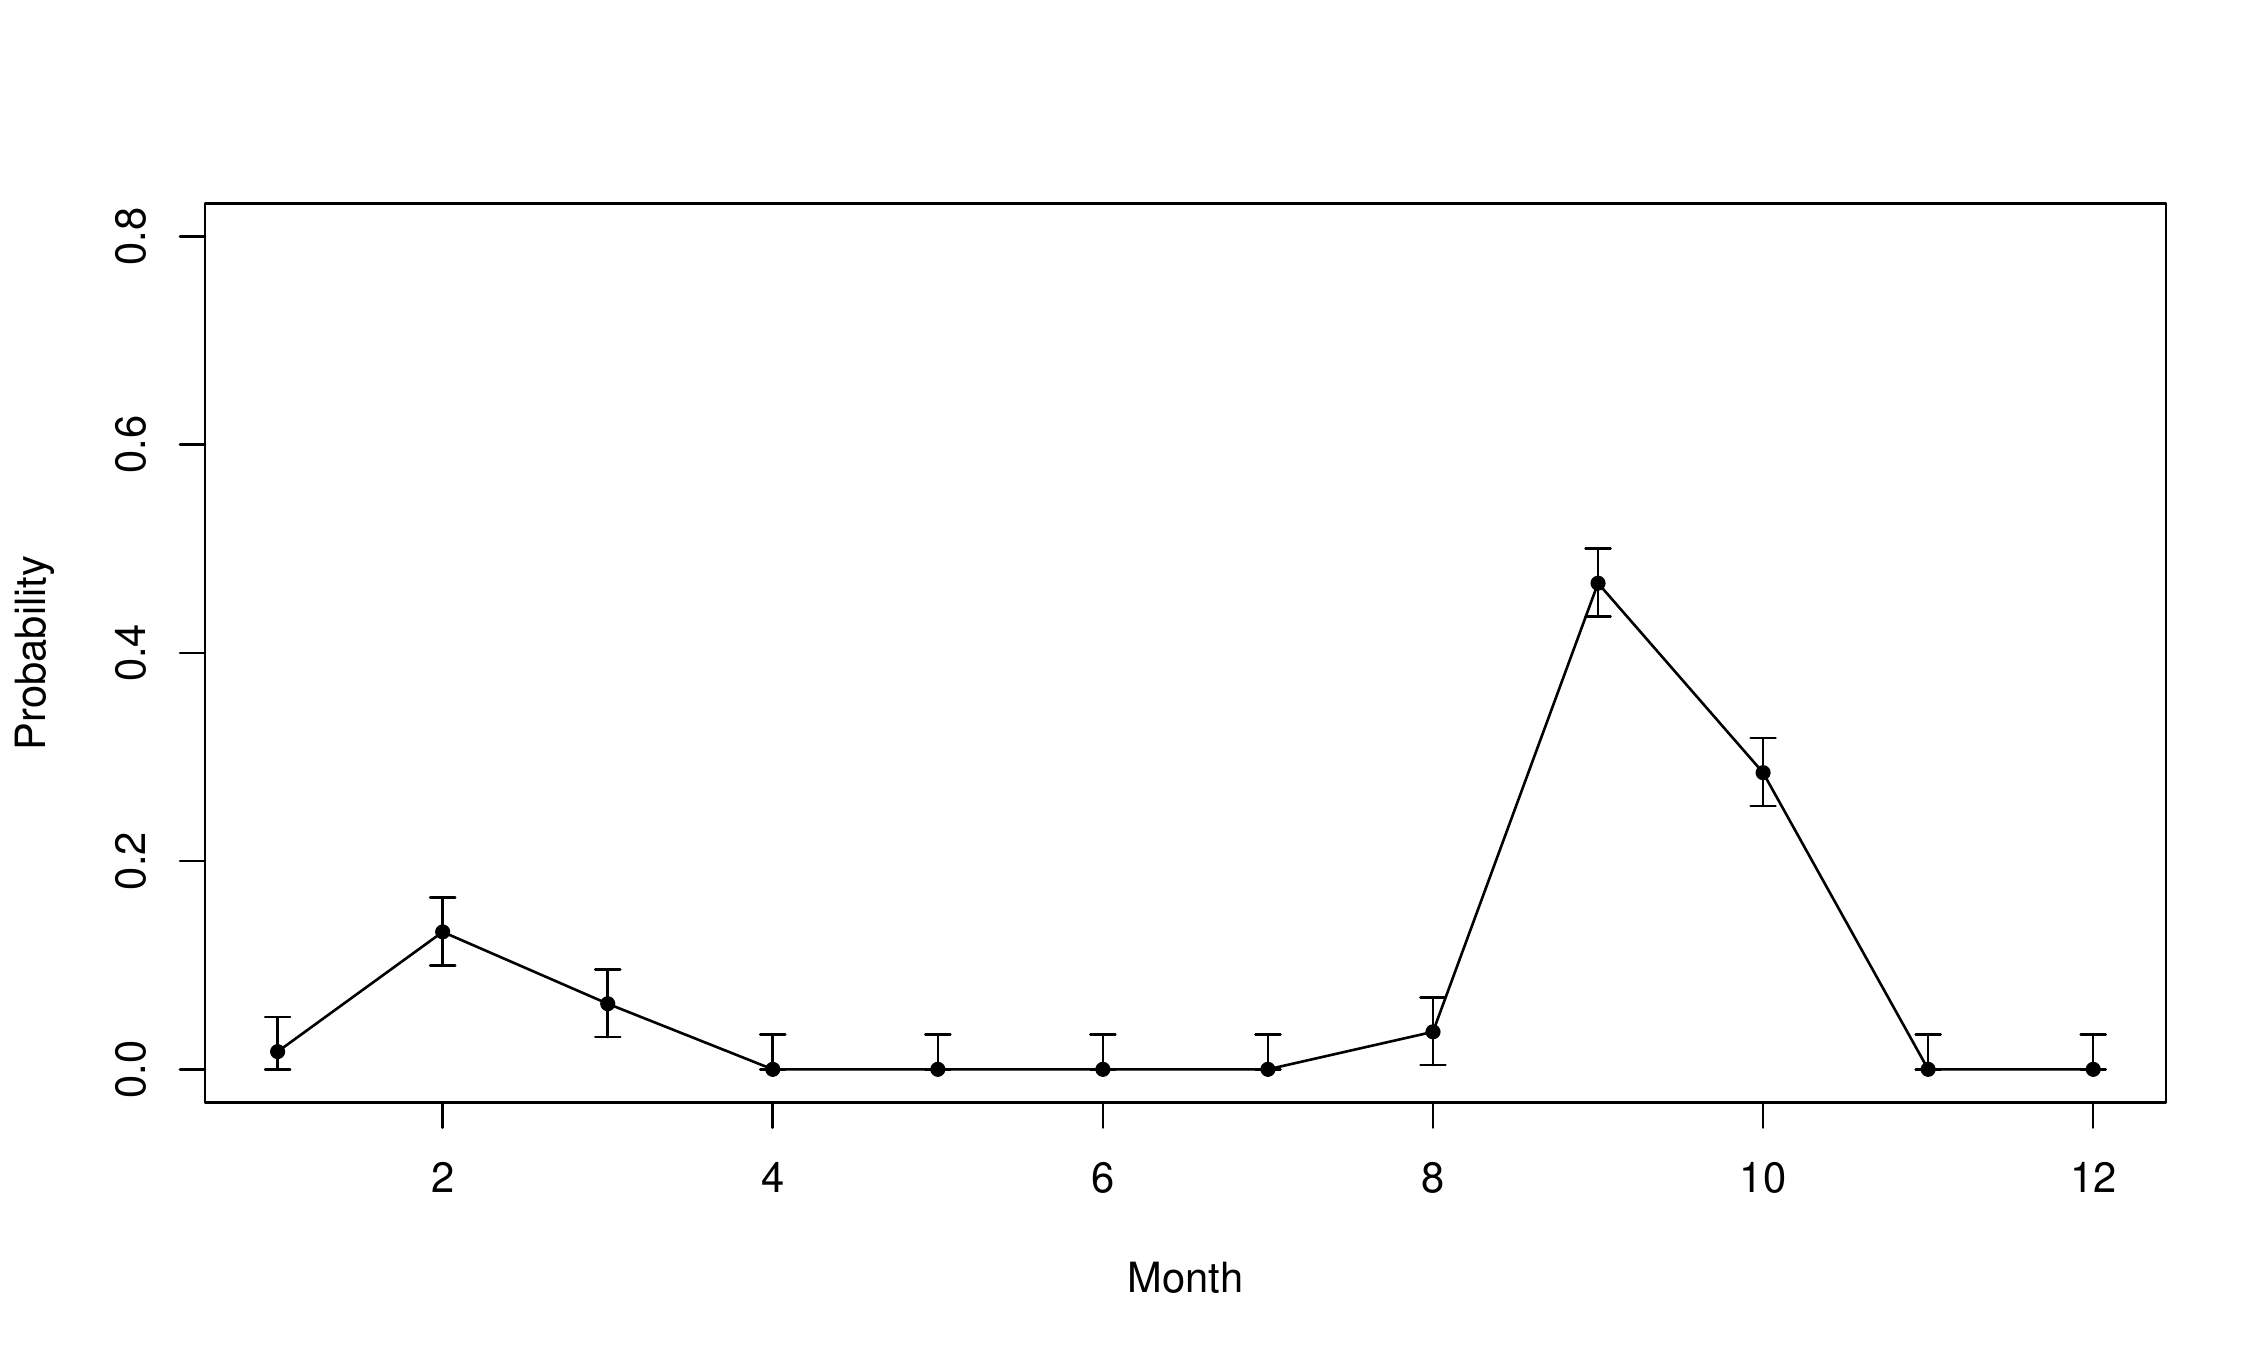}
    \includegraphics[width=0.49\textwidth]{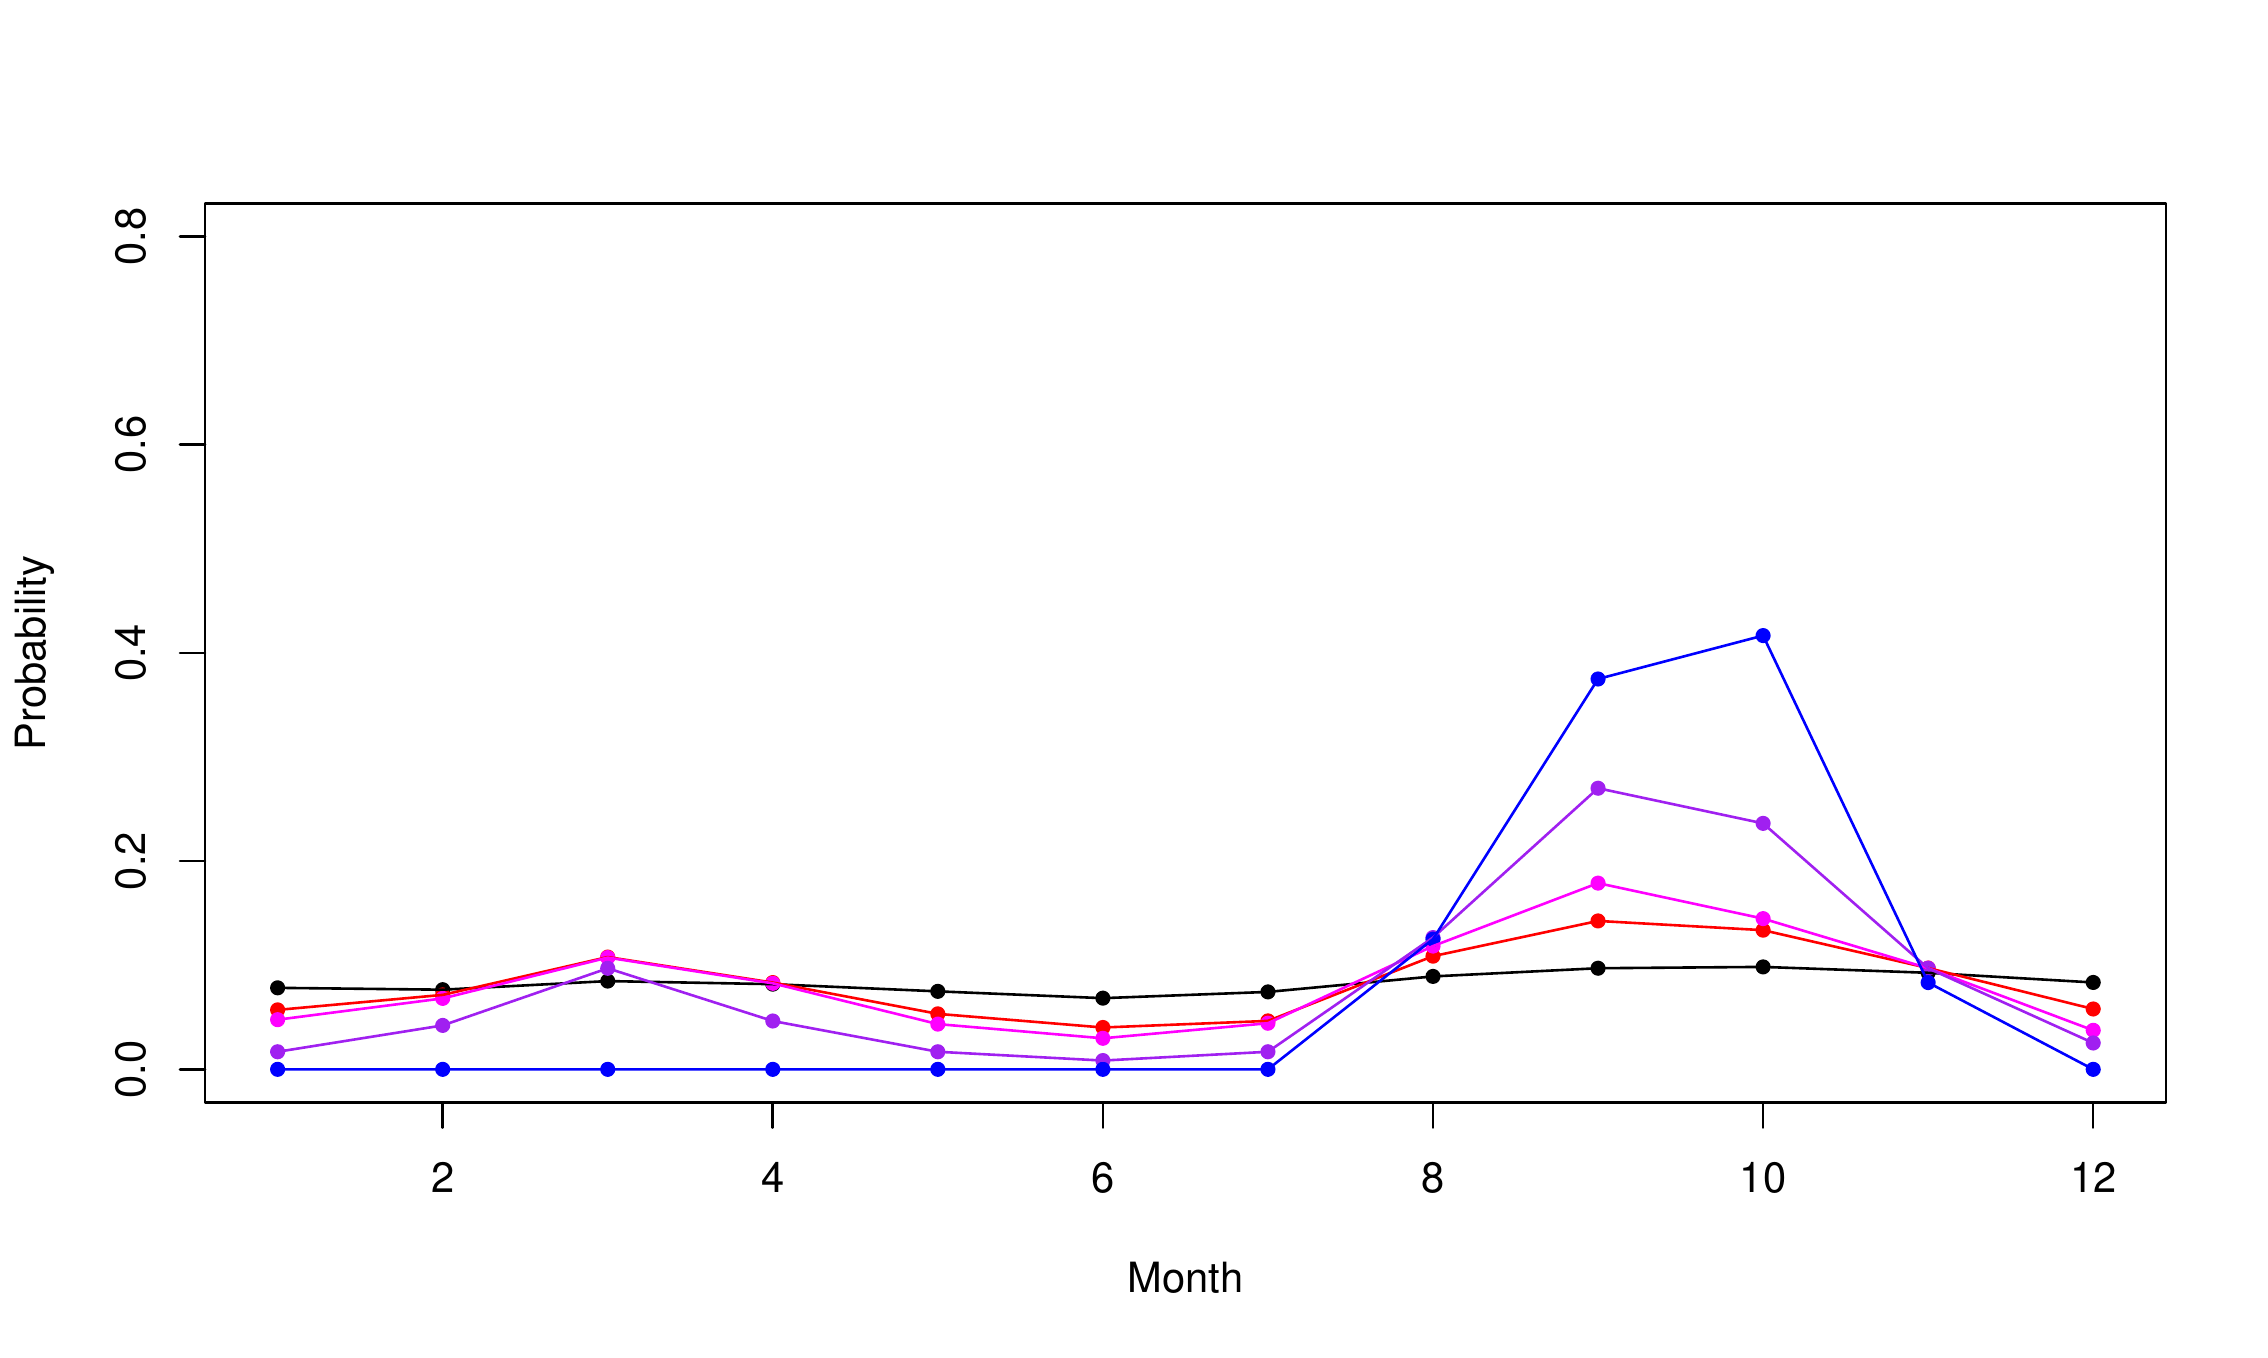}
    \includegraphics[width=0.49\textwidth]{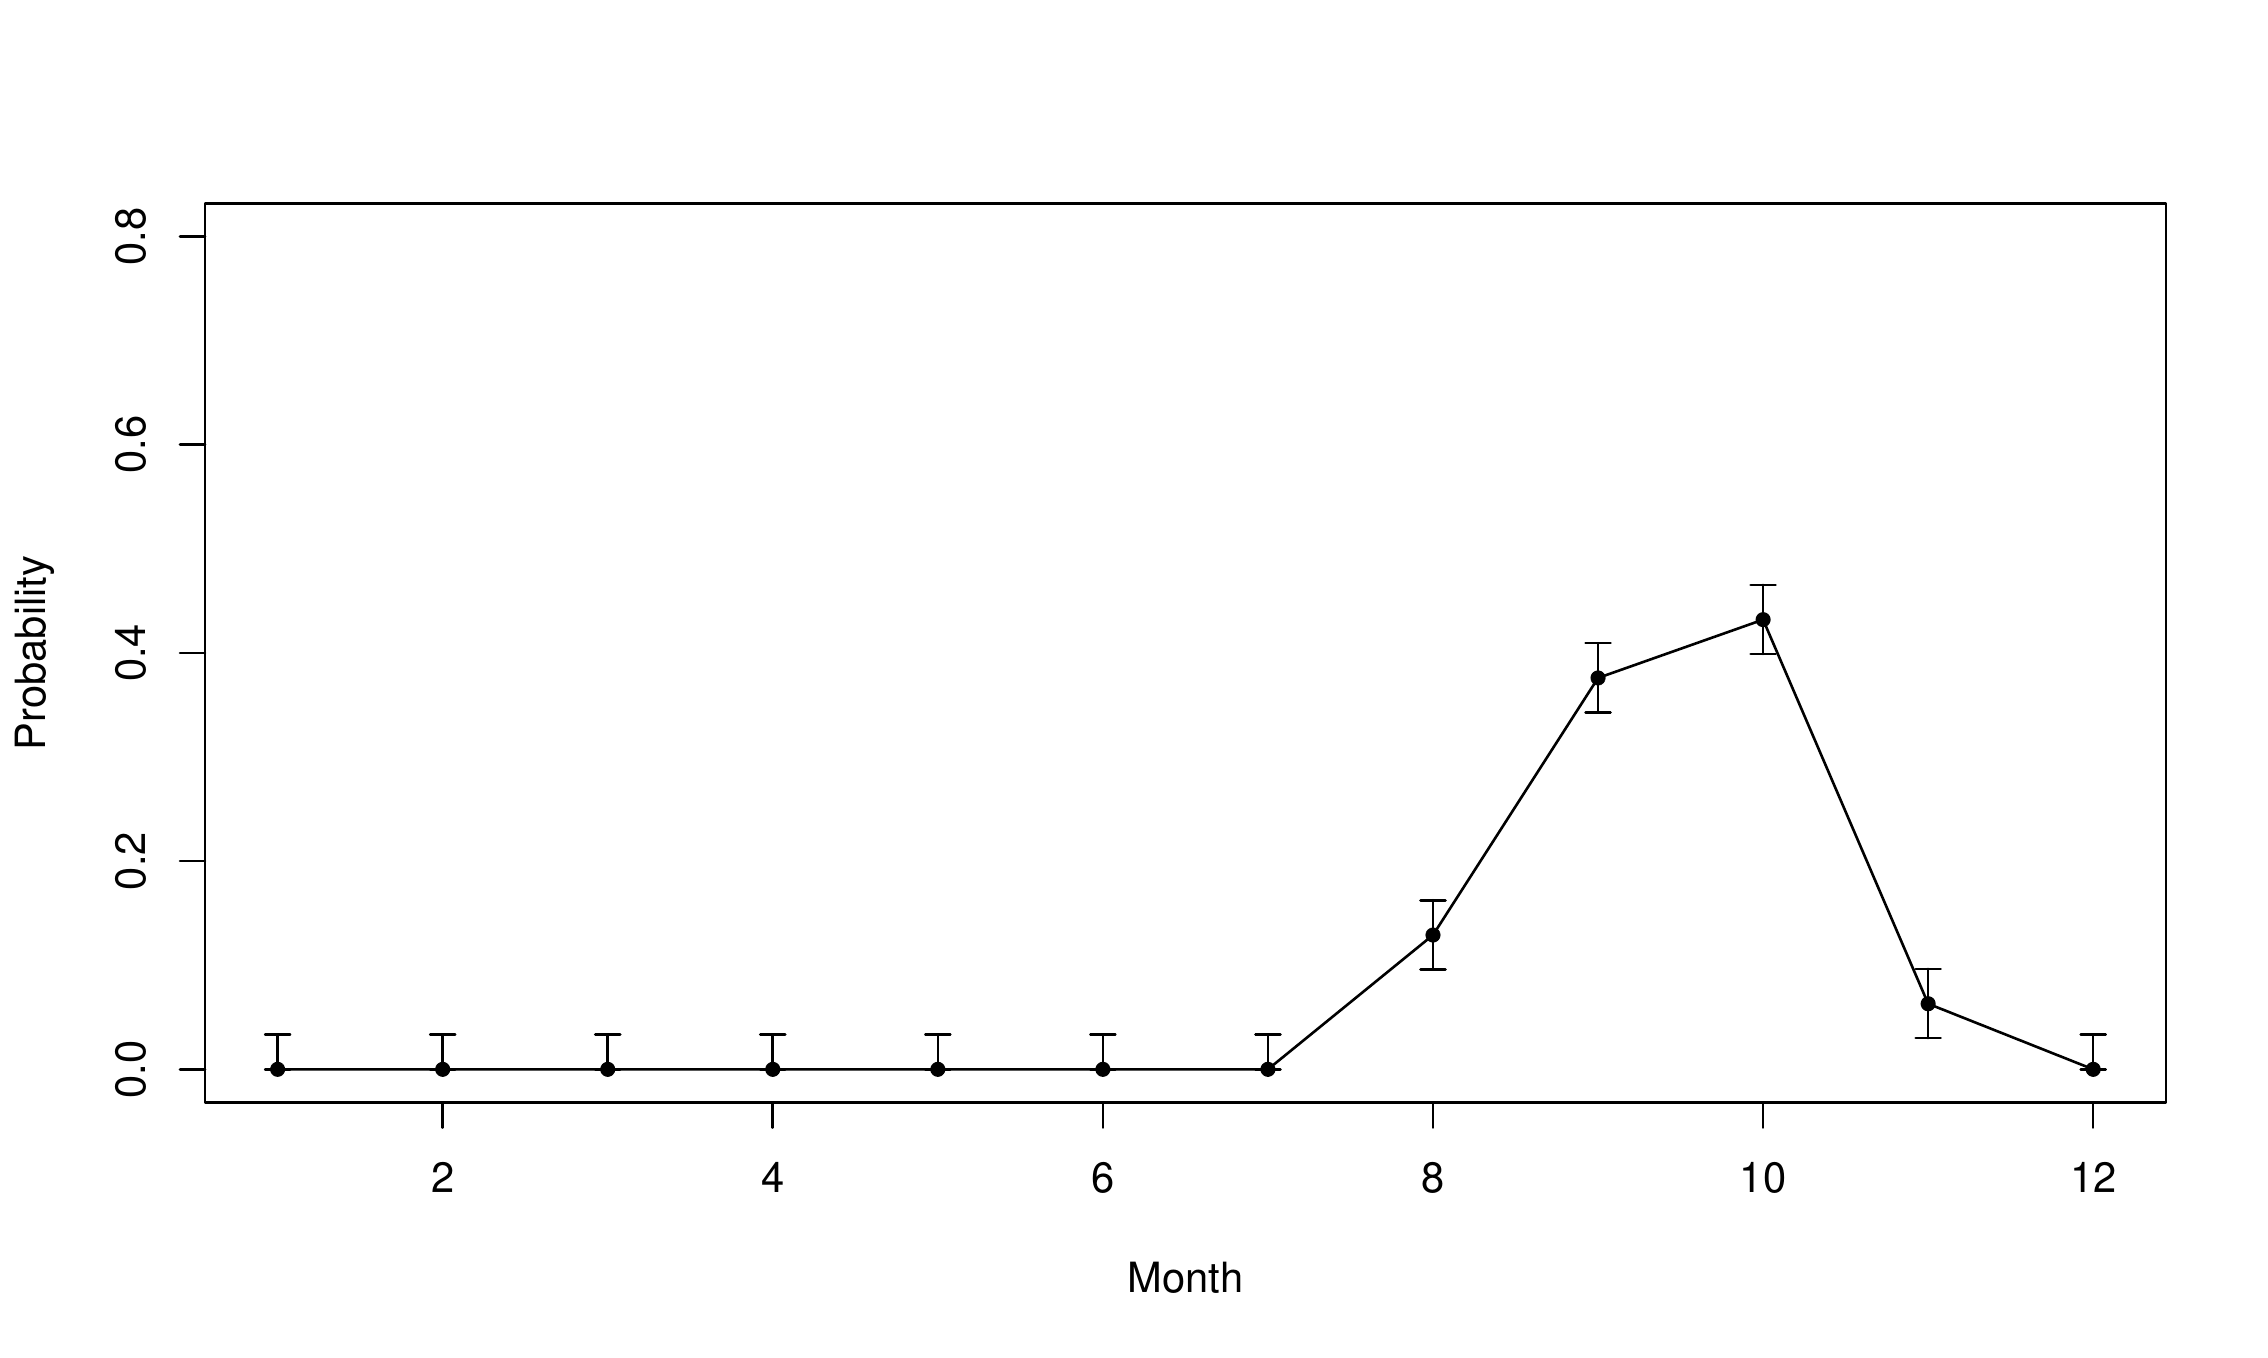}
    \caption{Estimates of $\hat p_j(R;q)$ (see expression~\eqref{prob}) for months $j=1,\ldots,12$ at $q=0.5$ (black), 0.9 (pink), 0.95 (magenta), 0.99 (purple) and 0.999 (blue) for Lowestoft (top), Newlyn (middle) and Sheerness (bottom) in the left column. We also show the 95\% confidence intervals for $\hat p_j(R;0.999)$ estimates at each site (right column).}
    \label{mt_seasonality_plot}
\end{figure}

%\subsection{Skew Surge and Peak Tide Dependence}
%Figure \ref{ss_mt_scatter} shows extreme skew surge (defined as exceedances of the 0.95 quantile) against their associated ranked peak tide (over all peak tides) at each site. The tides are ranked so that 1 corresponds to the smallest peak tide observation. If the two components are independent, ranked peak tides associated with extreme skew surges will be uniformly distributed. We test this formally using a Kolmogorov-Smirnov test for uniformity~\citep{kolmogorov1933} and discuss the results in Section \ref{ss_mt_indep} and Section \ref{ss_mt_indep_supp}.

\begin{table}[]
    \centering\resizebox{\textwidth}{!}{
    \begin{tabular}{c|c||c|c|c|c}
         & Block size & 0.9 & 0.95 & 0.975 & 0.99\\ \hline
        %HEY & 10 & 0.00288 & 0.0336 & 0.1313 & 0.095 \\
        HEY & 19 &  & 0.044 (0.082) &  &   \\
        LOW & 5 & 0.63 (0.17) & 0.72 (0.22) & 0.78 (0.27) & 0.33 (0.23) \\
        NEW & 20 & 0.070 (0.075) & 0.091 (0.087) & 0.15 (0.17) & 0.12 (0.11)  \\
        SHE & 6 & 1.5$\times 10^{-8}$ (4.1$\times{10^{-8}}$) & 1.1$\times 10^{-4}$ (2.9 $\times 10^{-4}$) & 9.9 $\times{10^-4}$ (-0.0011) & 0.0013 (7.0$\times{10^{-4}}$) \\
    \end{tabular}
    }
    \caption{K-S test $p$ values uniformity of ranked peak tides associated with extreme skew surges, defined as exceedances of different quantiles of the data. Average $p$ values after repeated bootstrapping are shown in parentheses.}
    %%%%% Needs updating for NEW
    \label{KStest_threshold}
\end{table}

\begin{figure}
    \centering
    \includegraphics[width=0.48\textwidth]{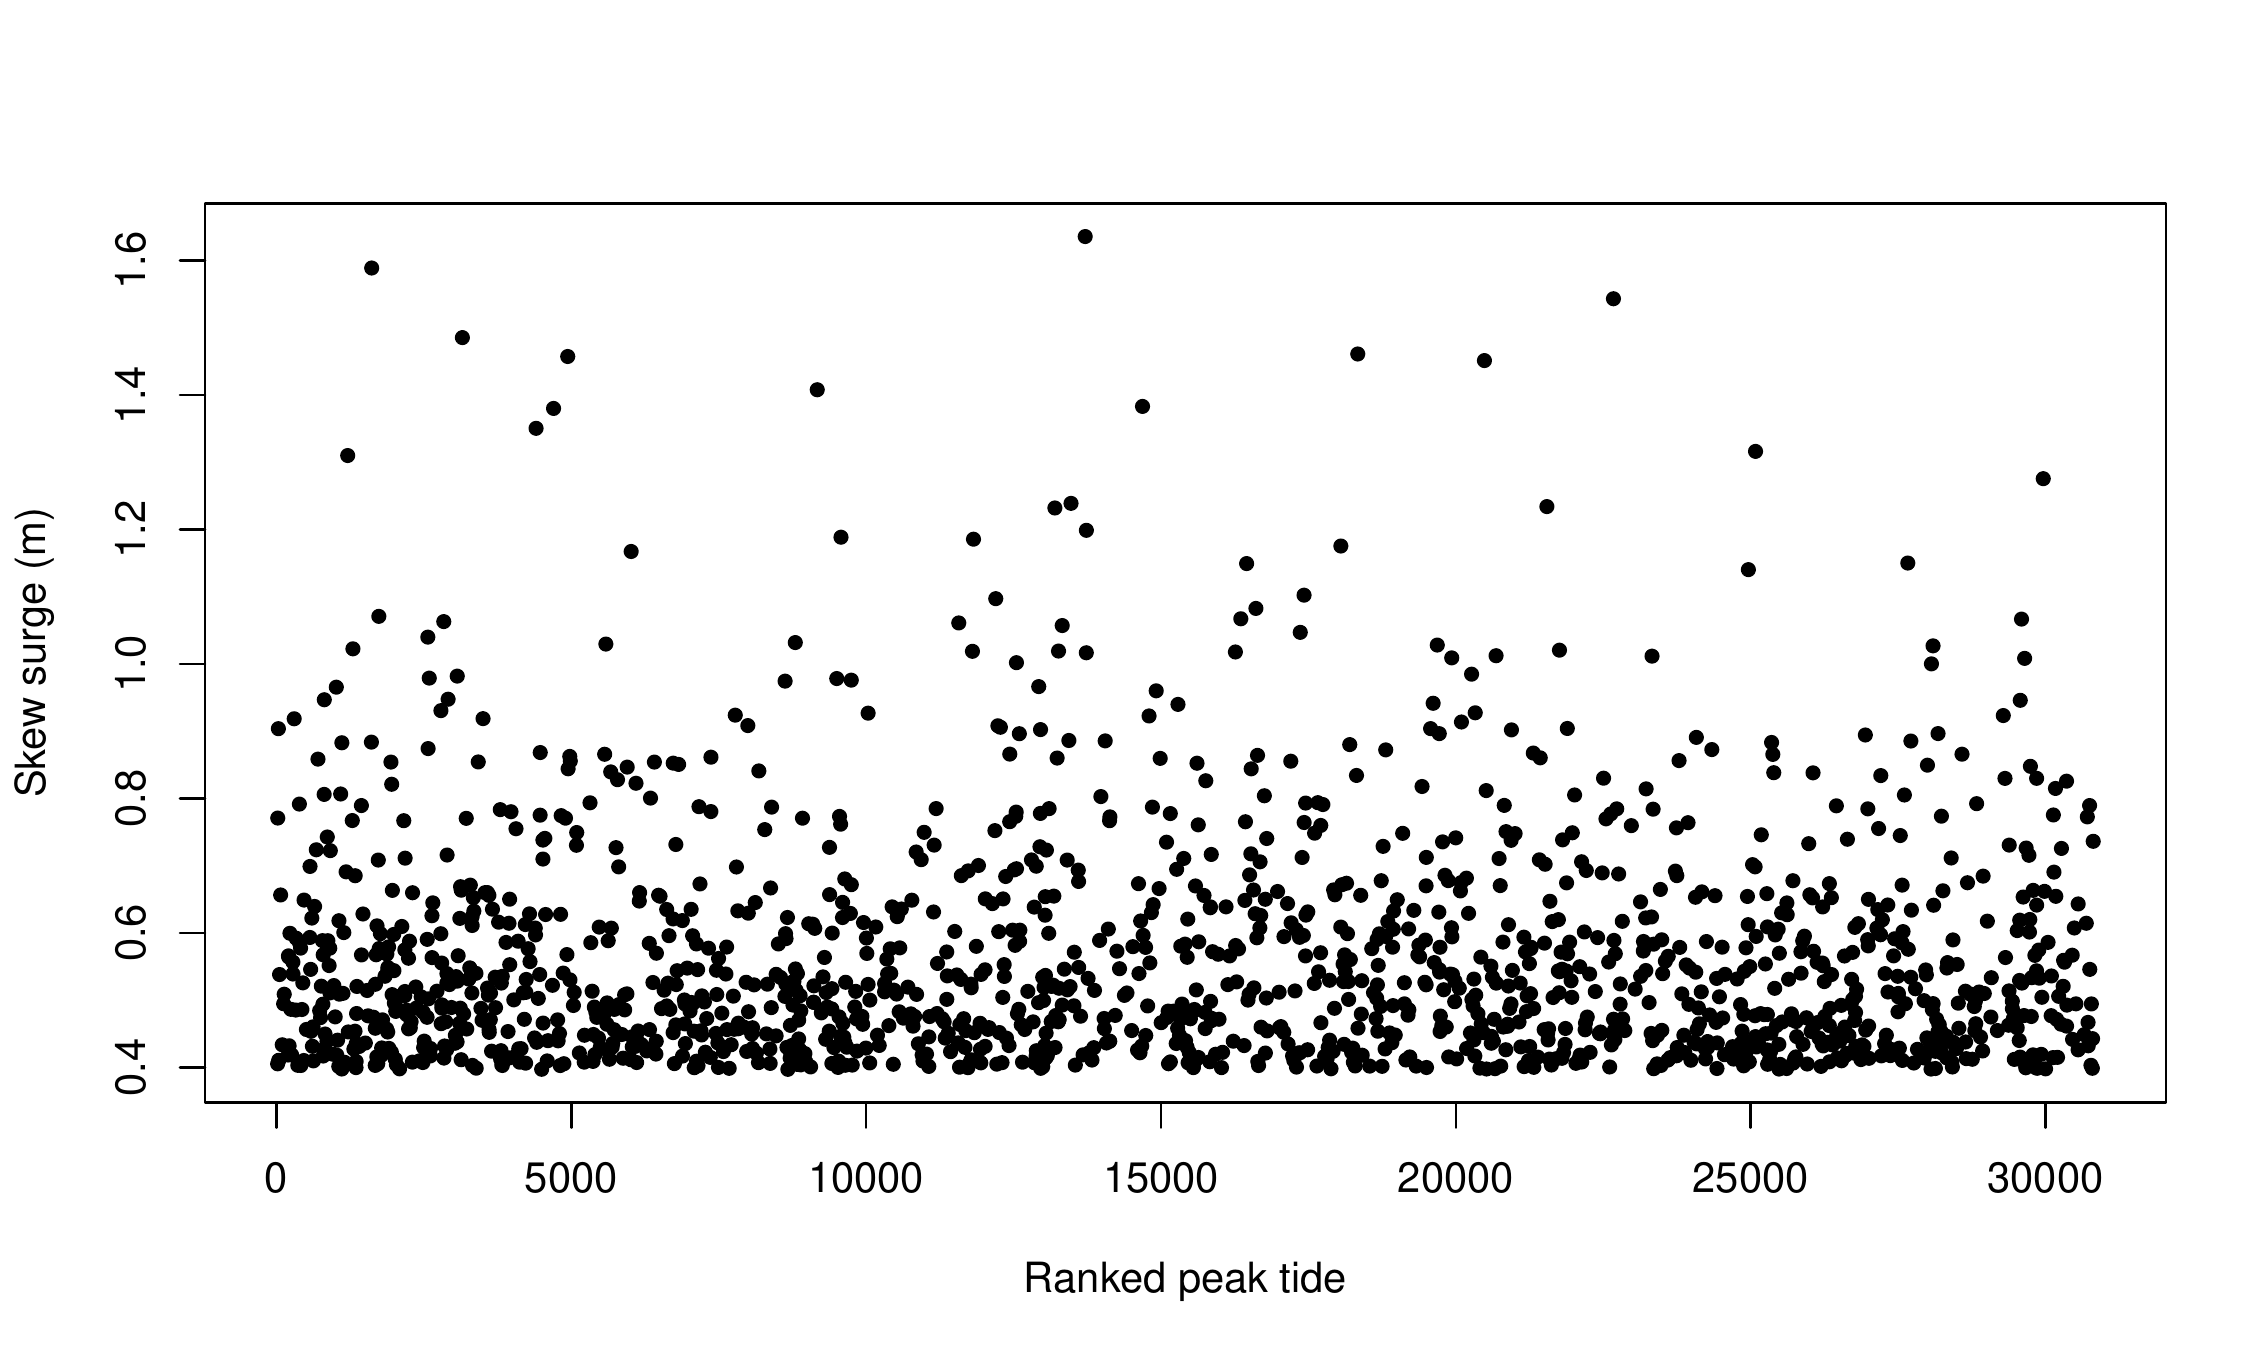}
    \includegraphics[width=0.48\textwidth]{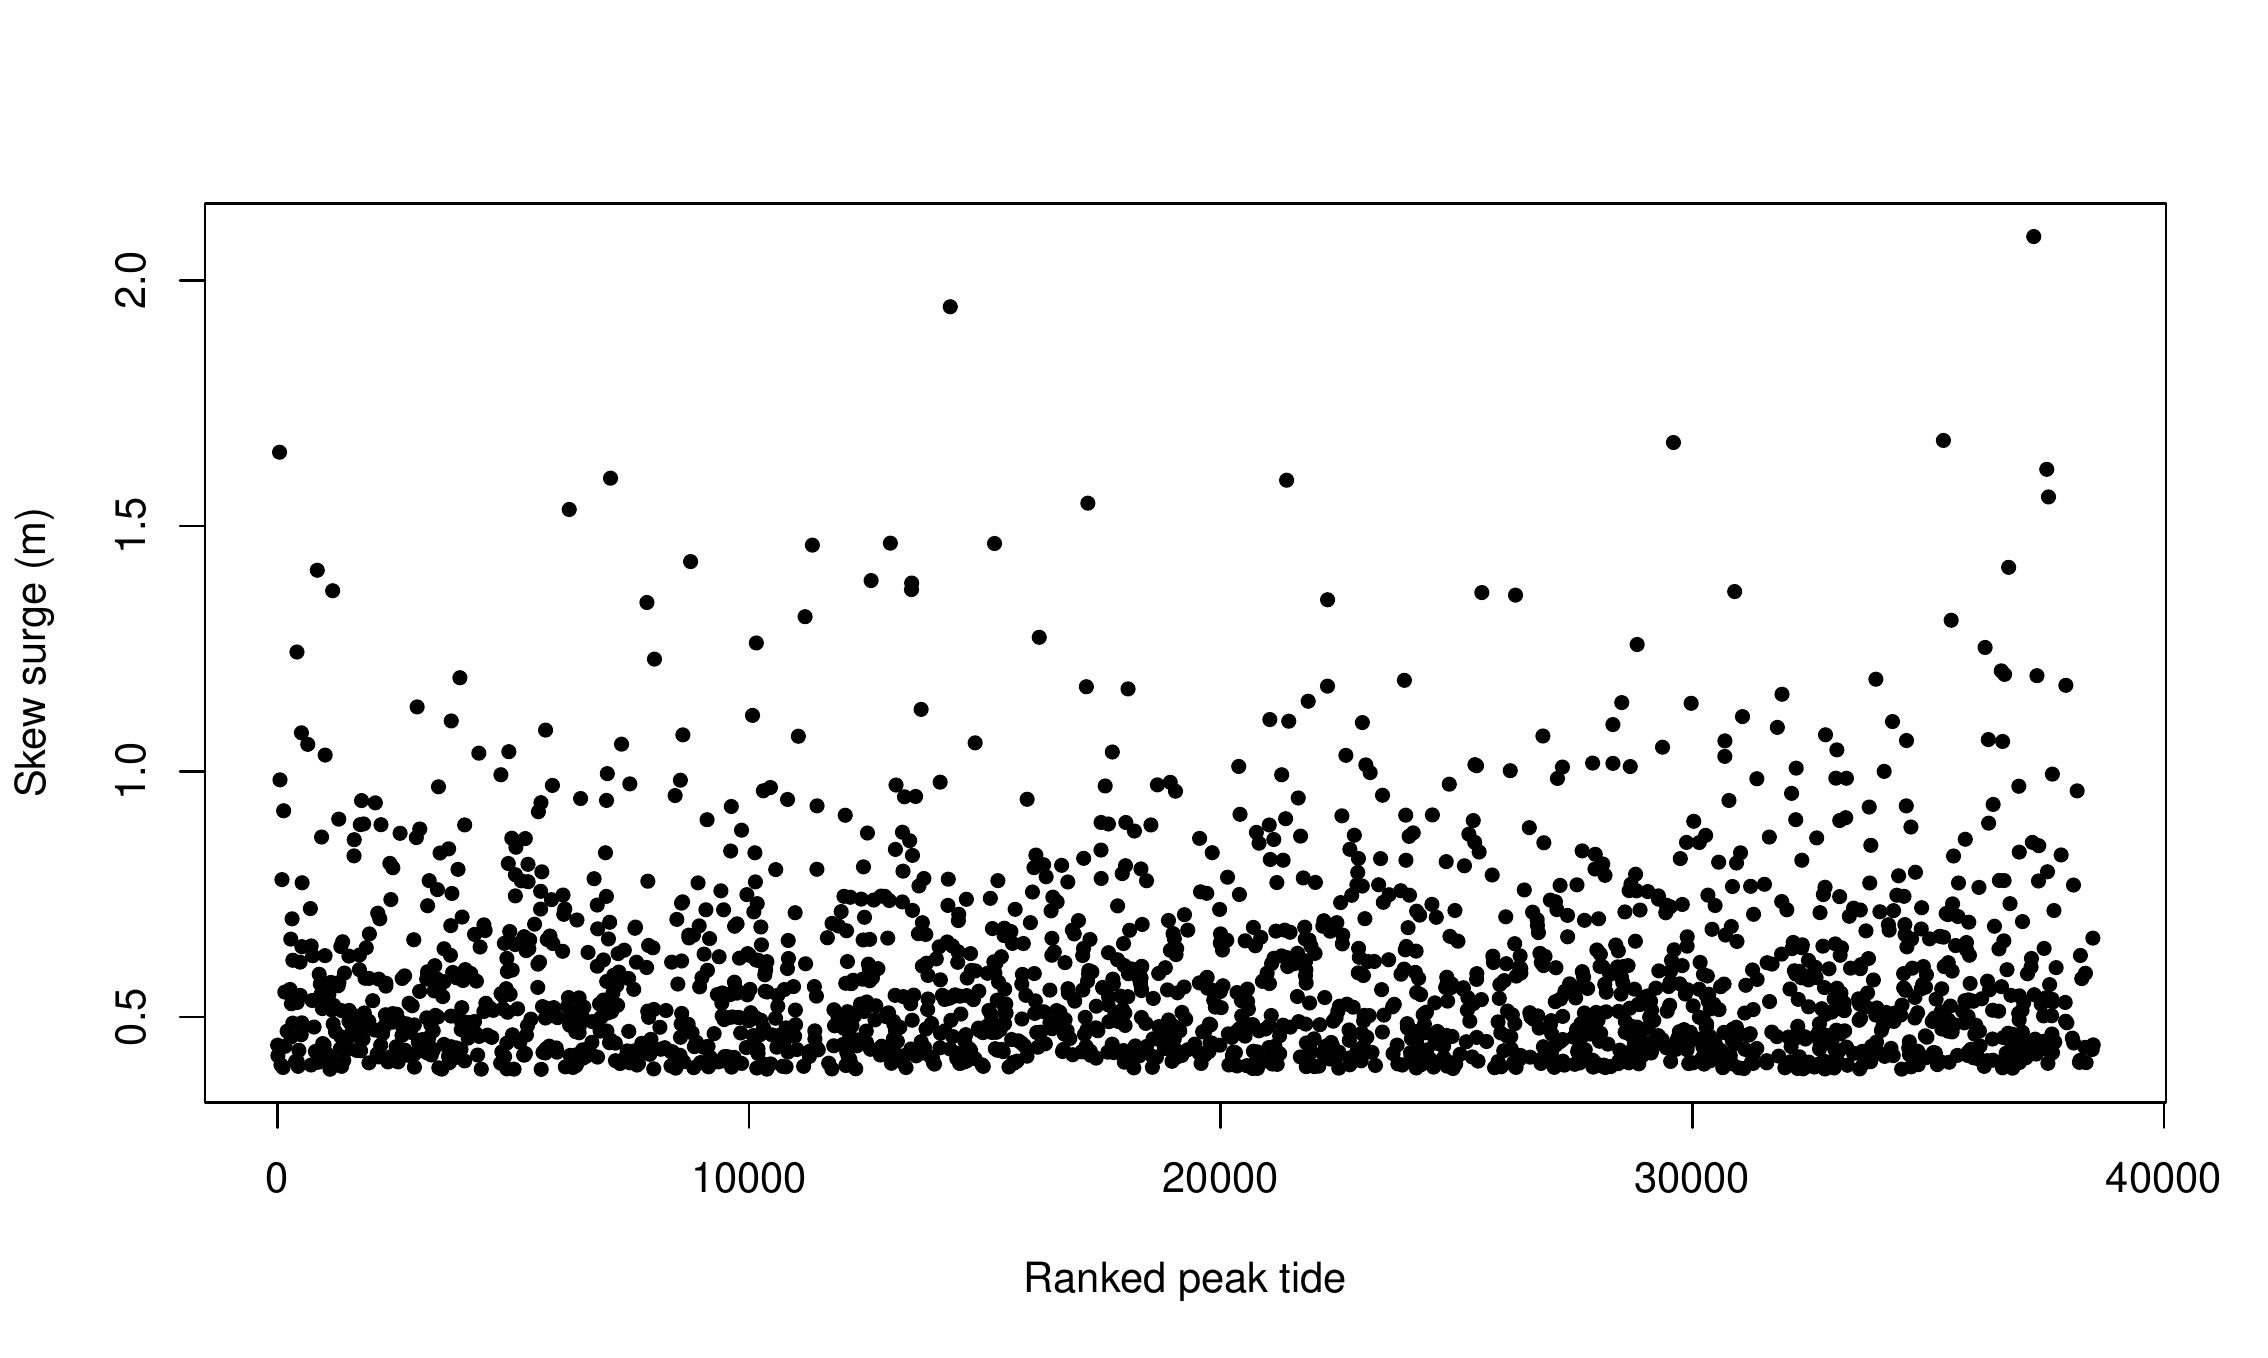}\\
    \includegraphics[width=0.48\textwidth]{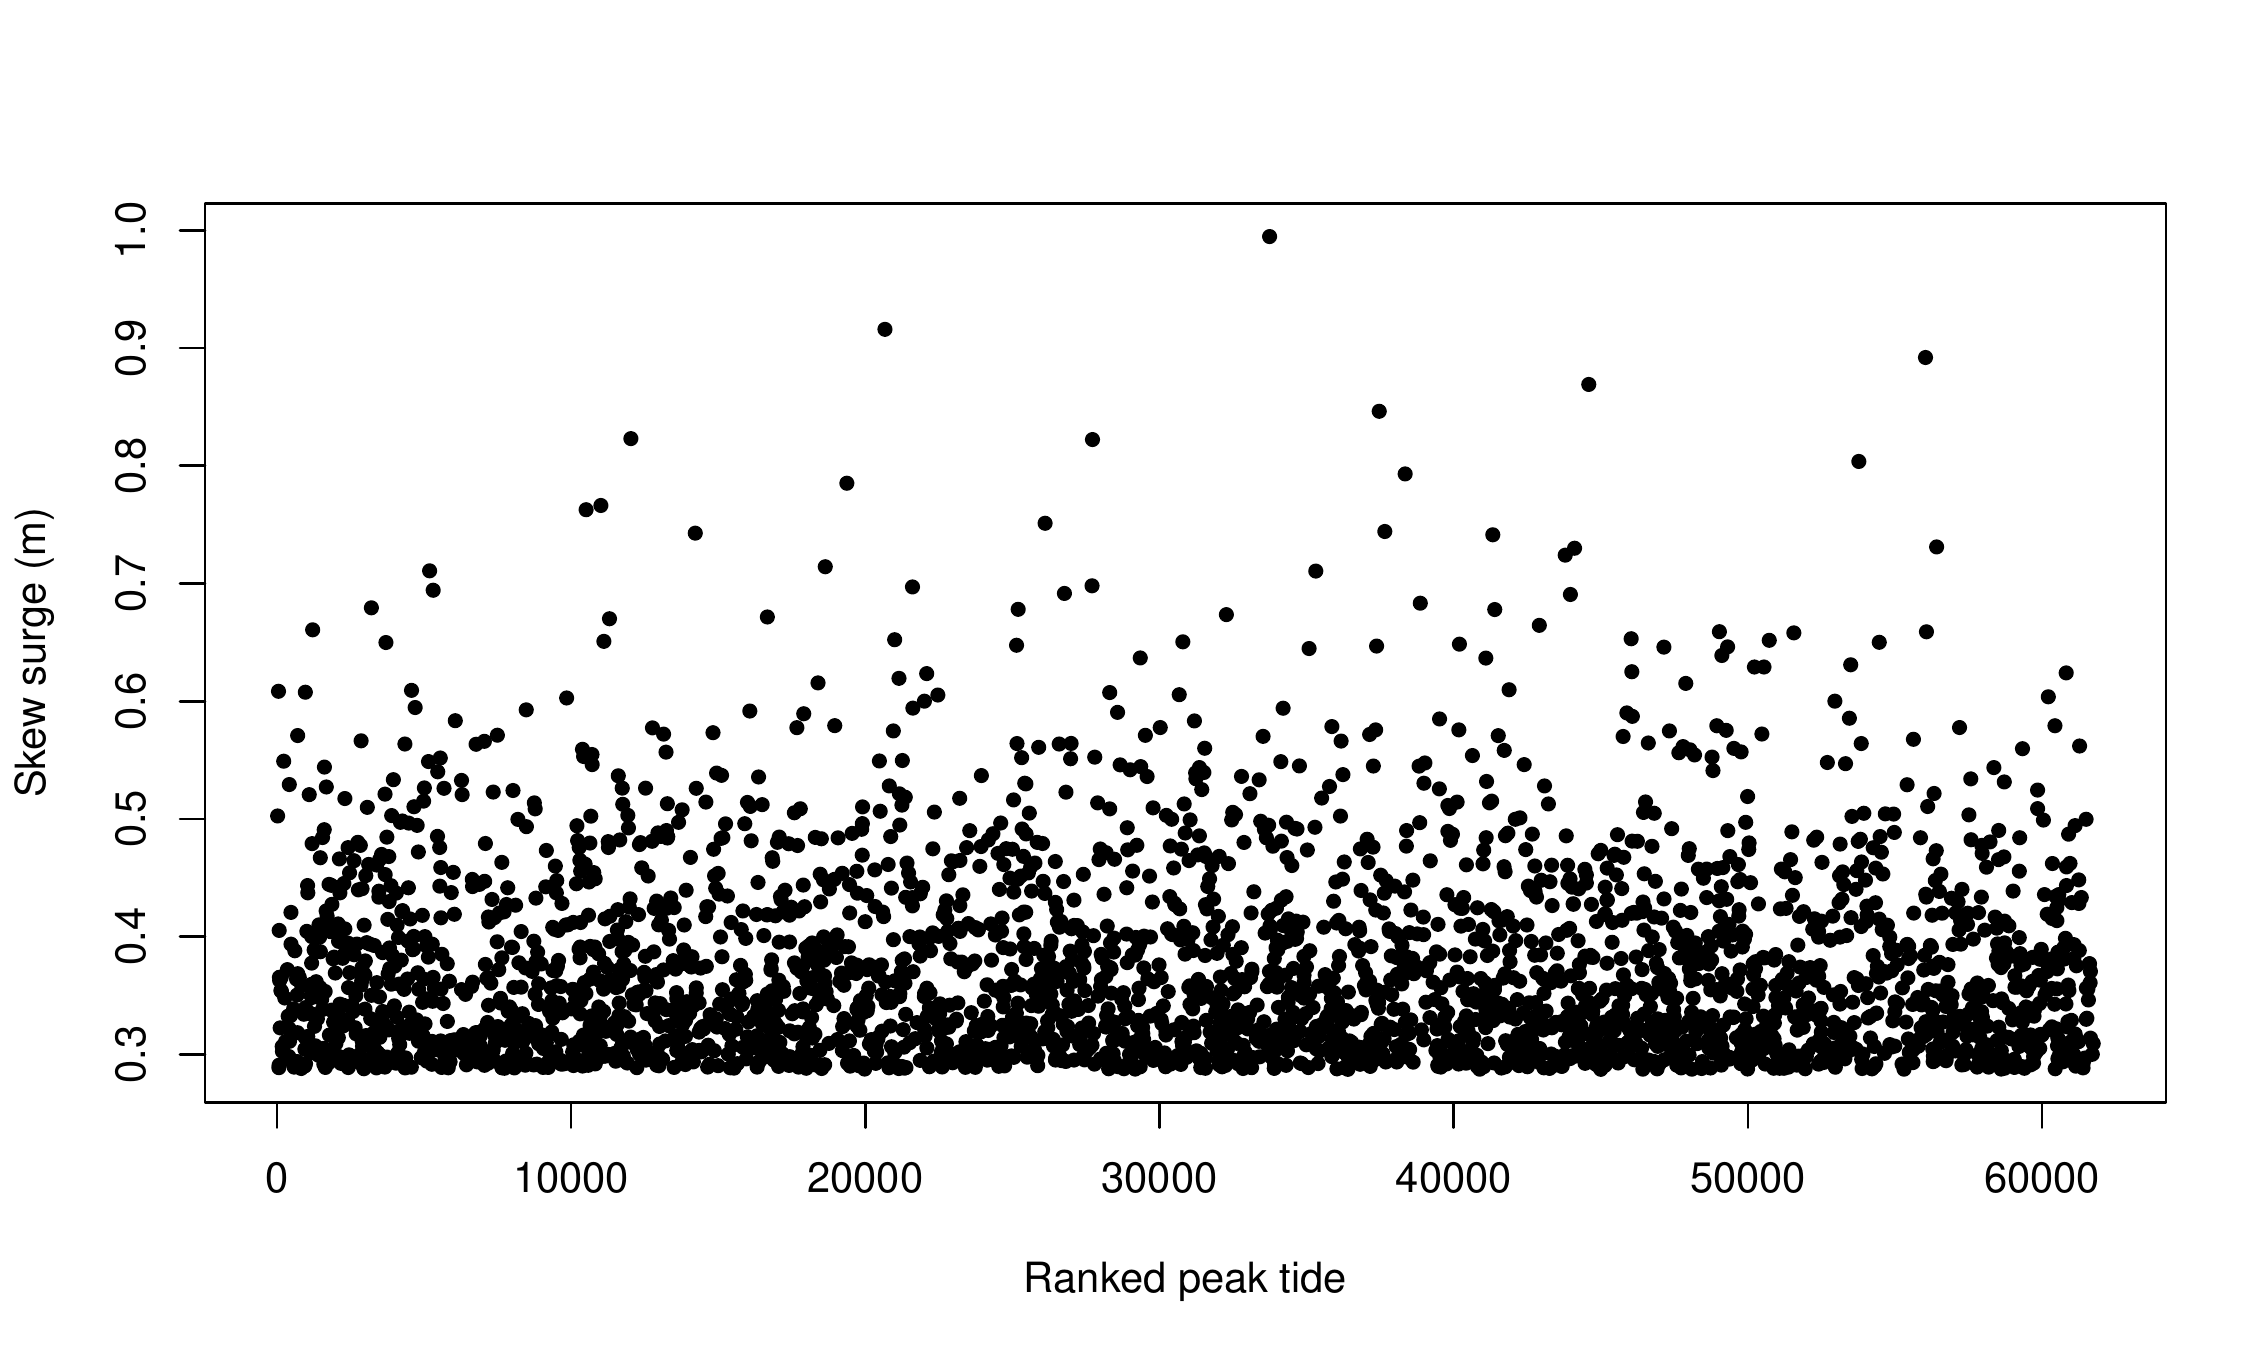}
    \includegraphics[width=0.48\textwidth]{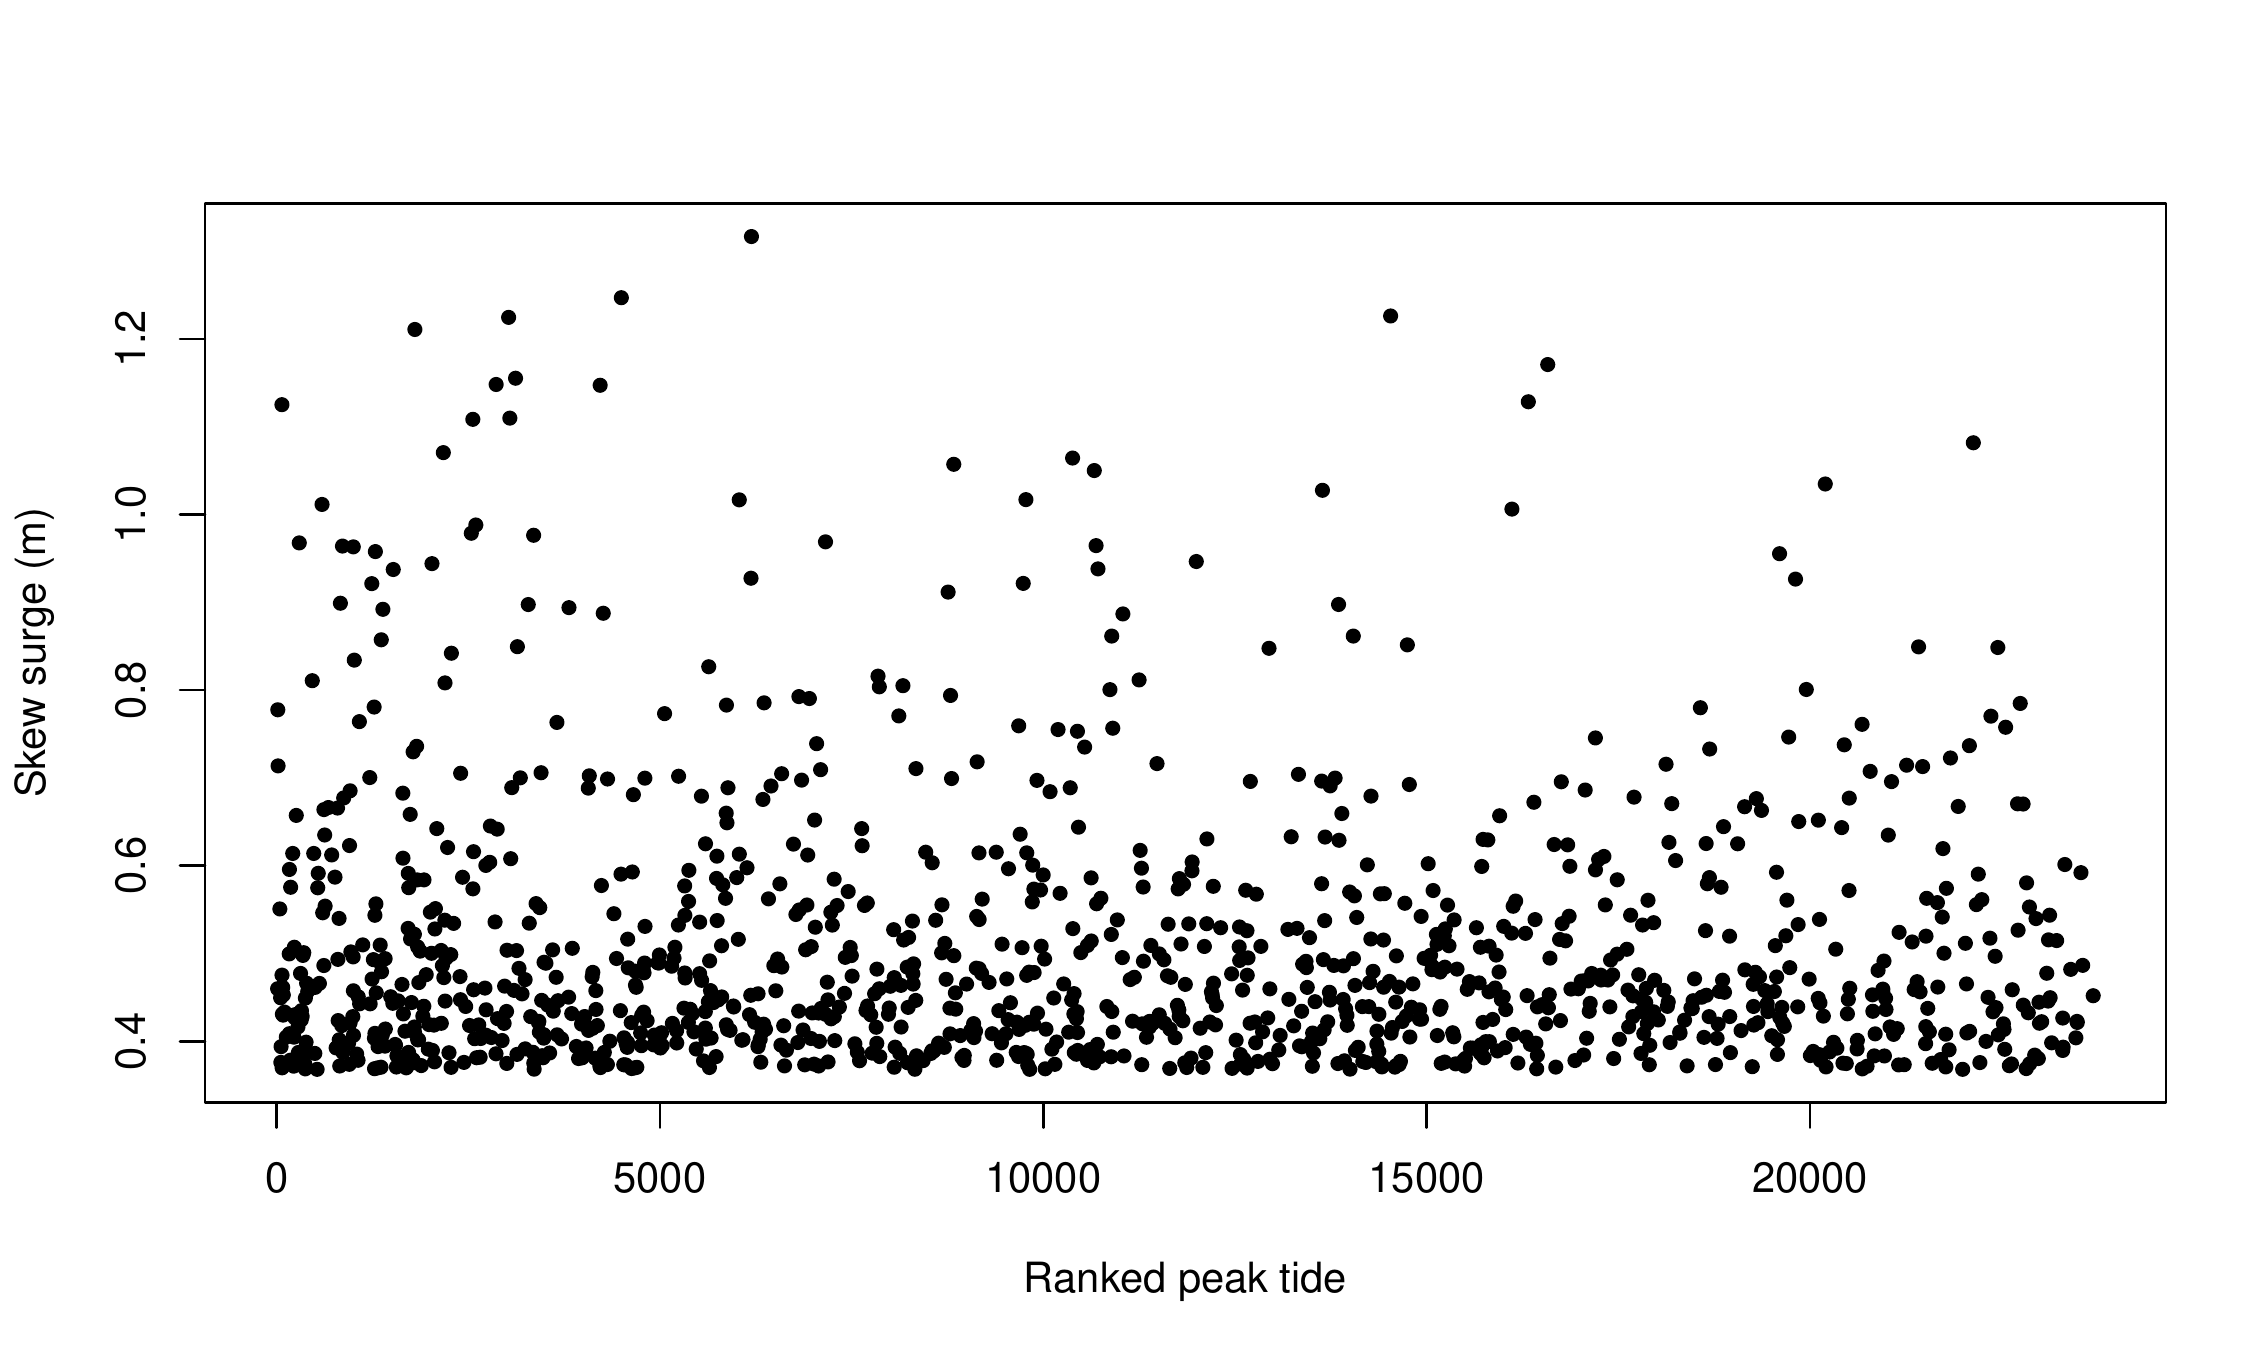}
    \caption{Extreme skew surge observations against associated rank peak tides at Heysham (top right), Lowestoft (top left), Newlyn (bottom left) and Sheerness (bottom right)}
    \label{ss_mt_scatter}
\end{figure}

\begin{figure}
    \centering
    \includegraphics[width=0.4\textwidth]{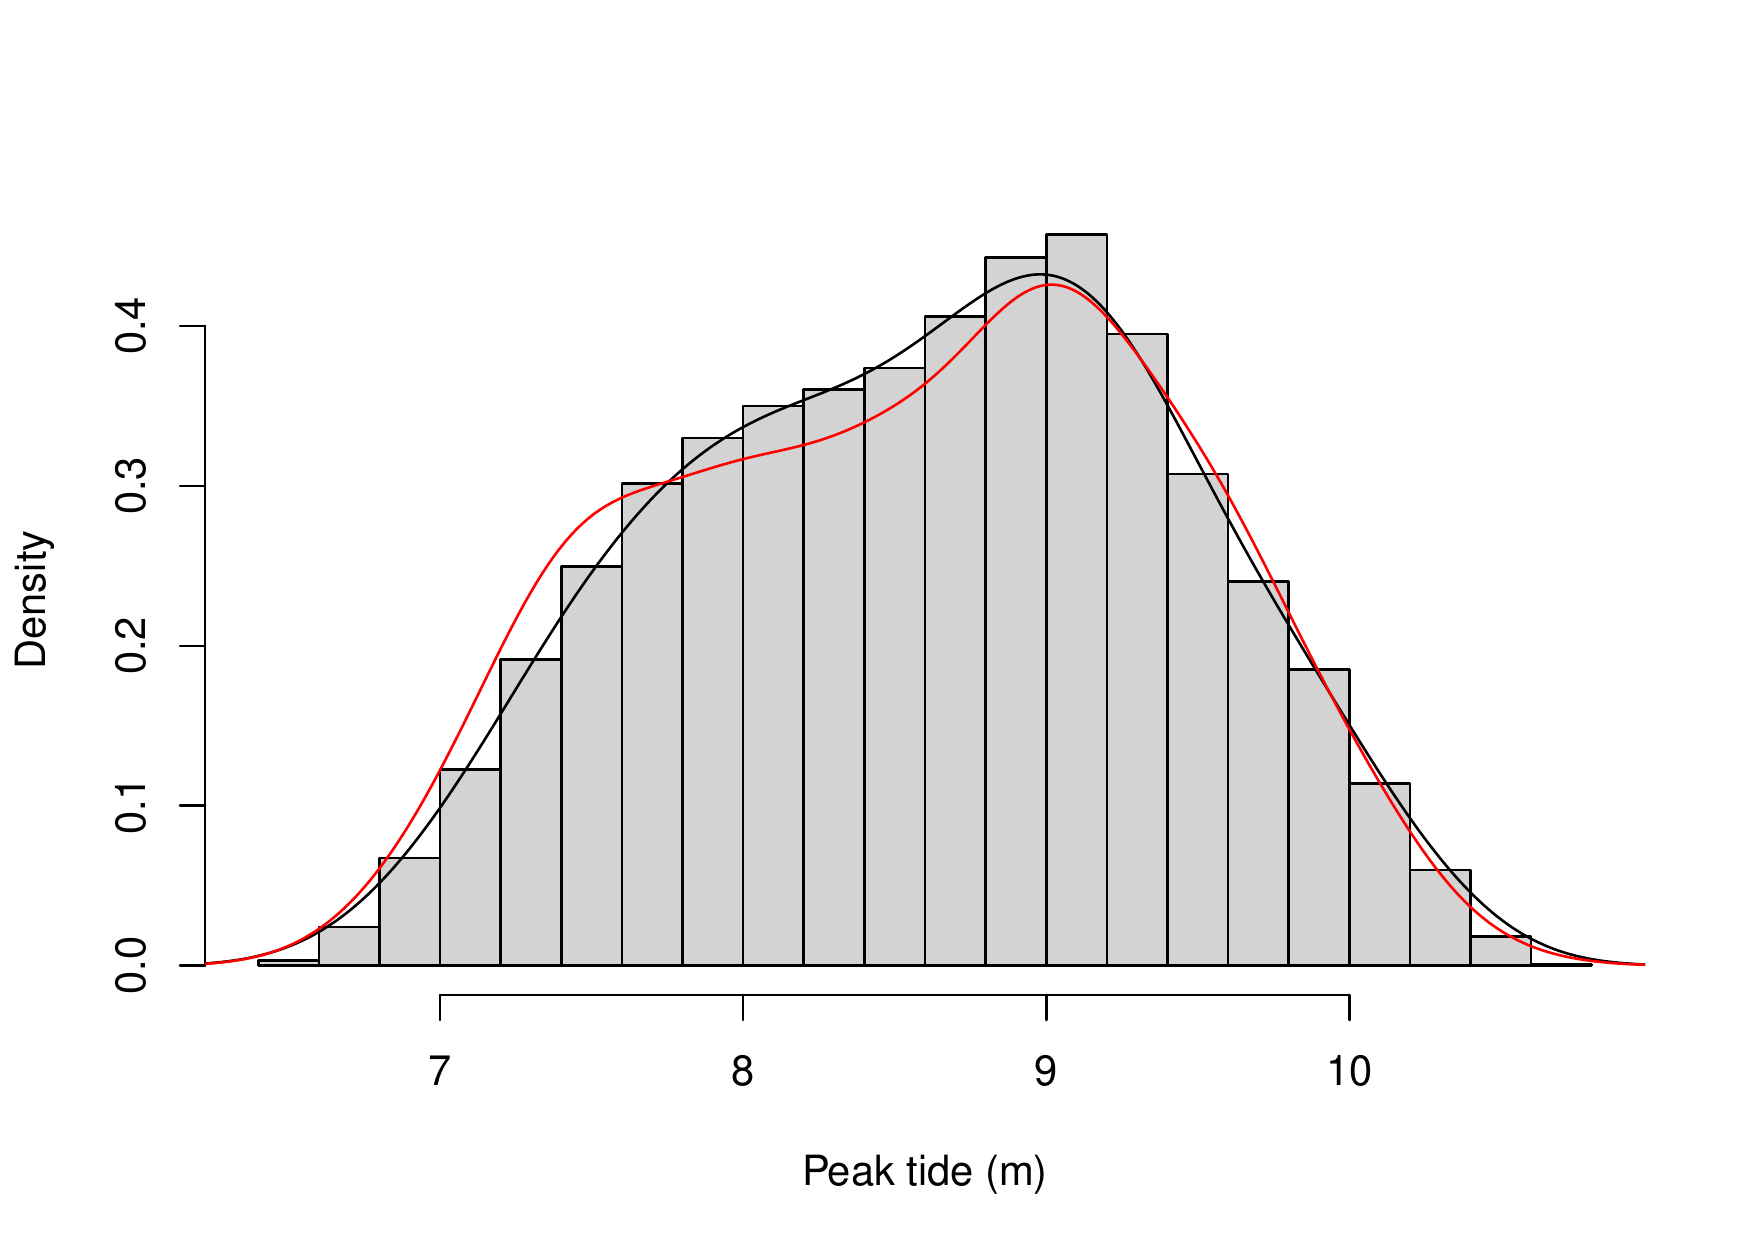}\includegraphics[width=0.4\textwidth]{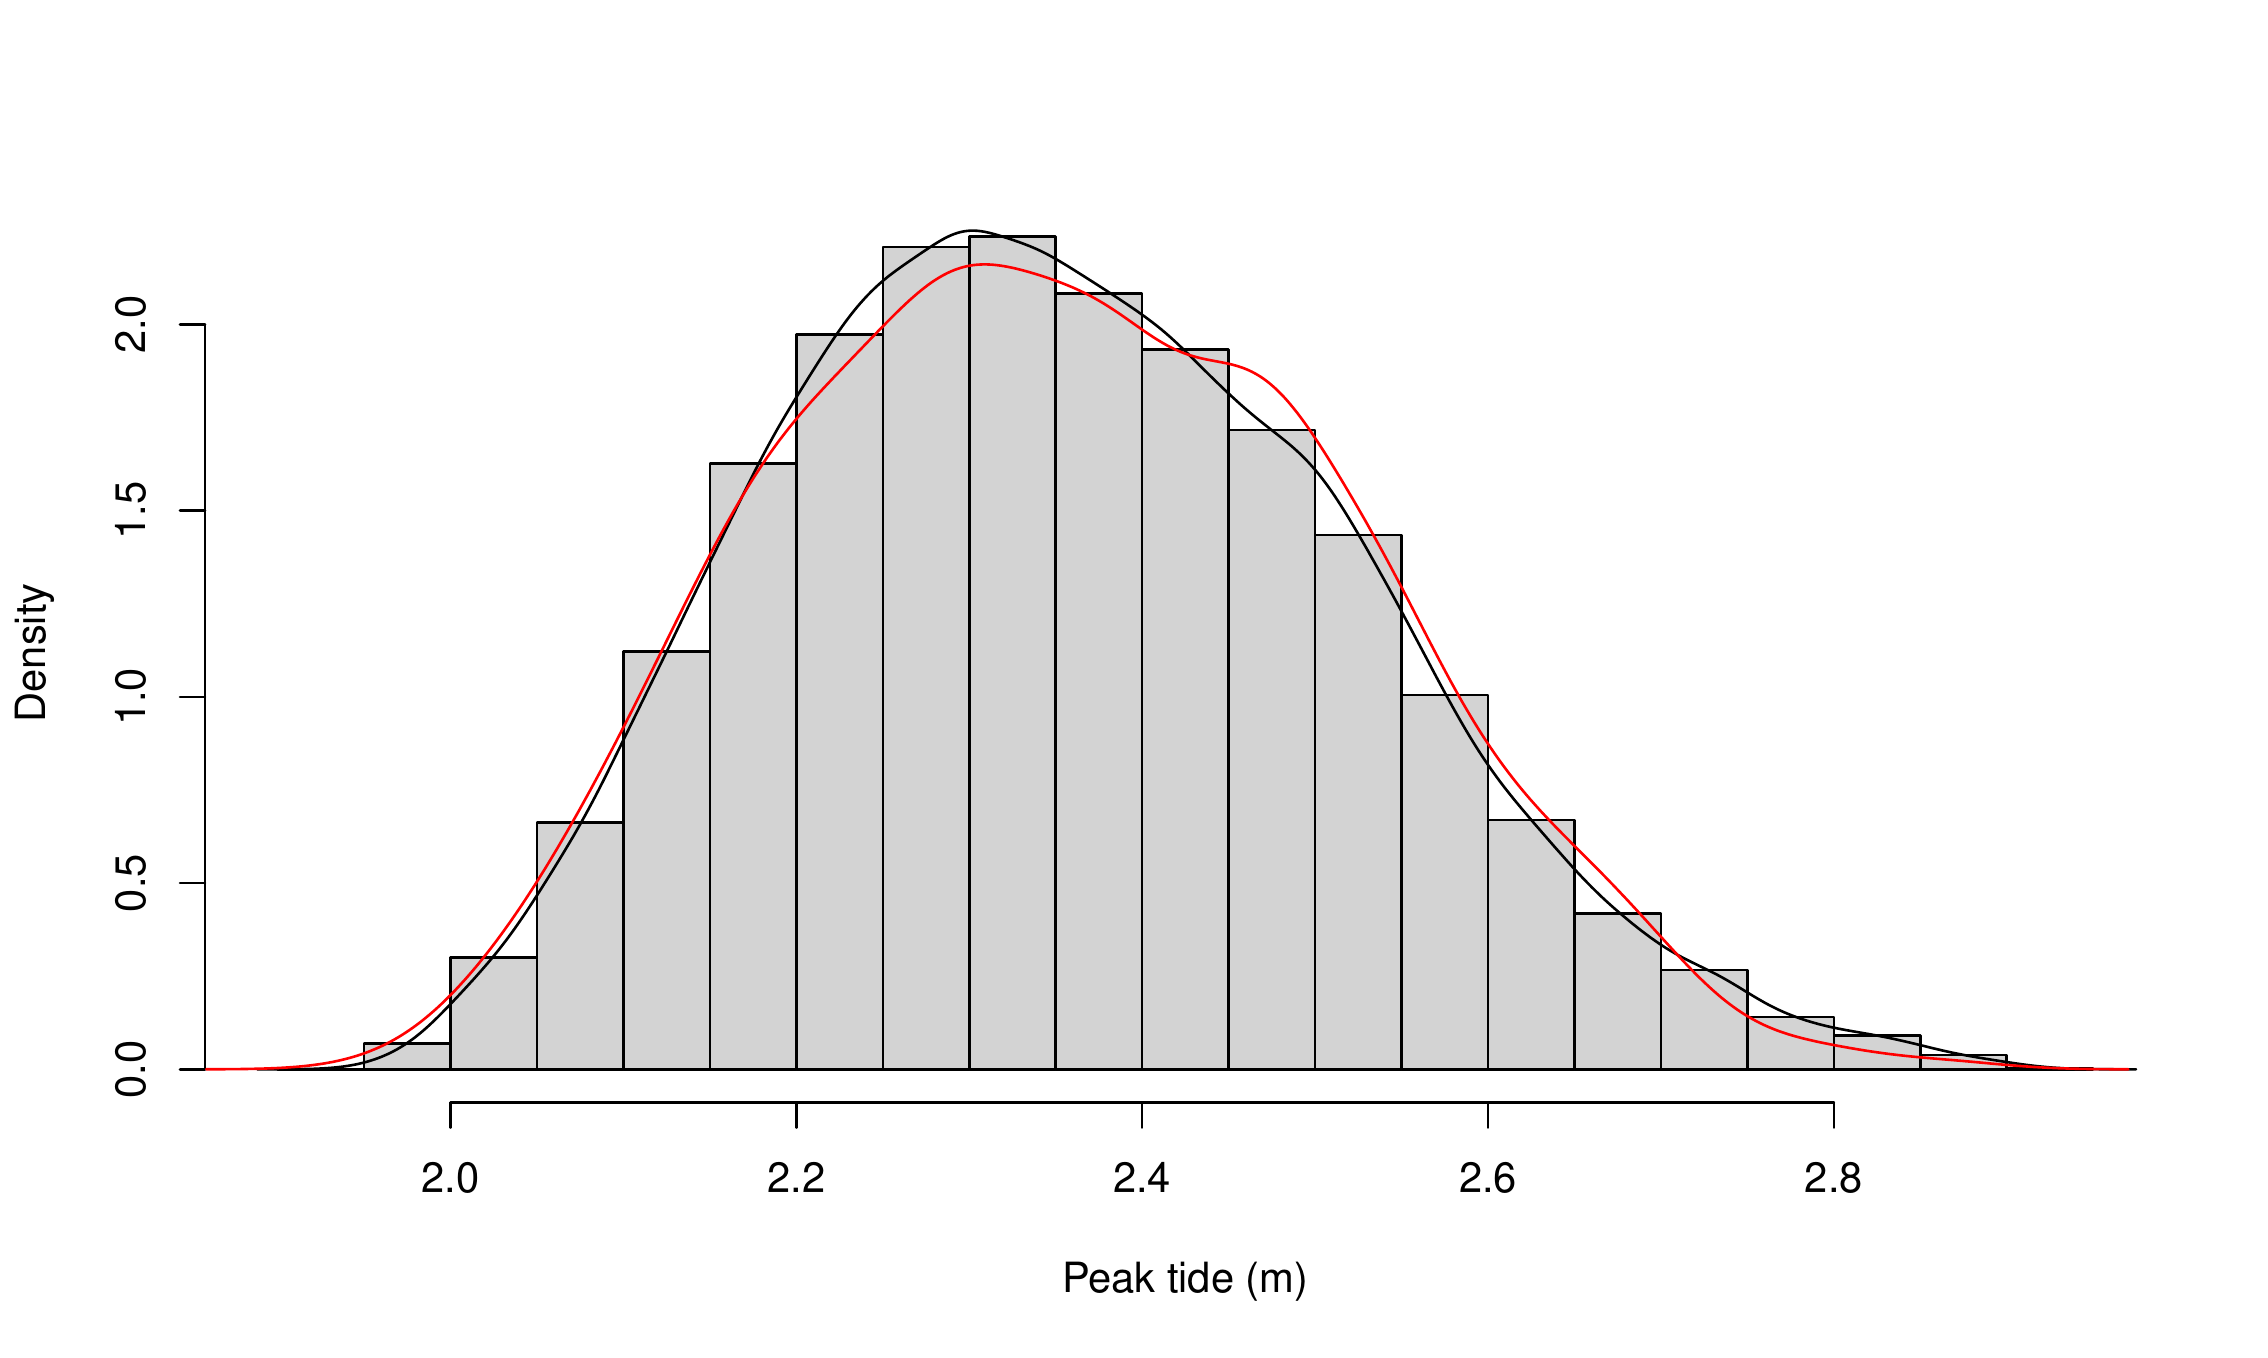}\\
    \includegraphics[width=0.4\textwidth]{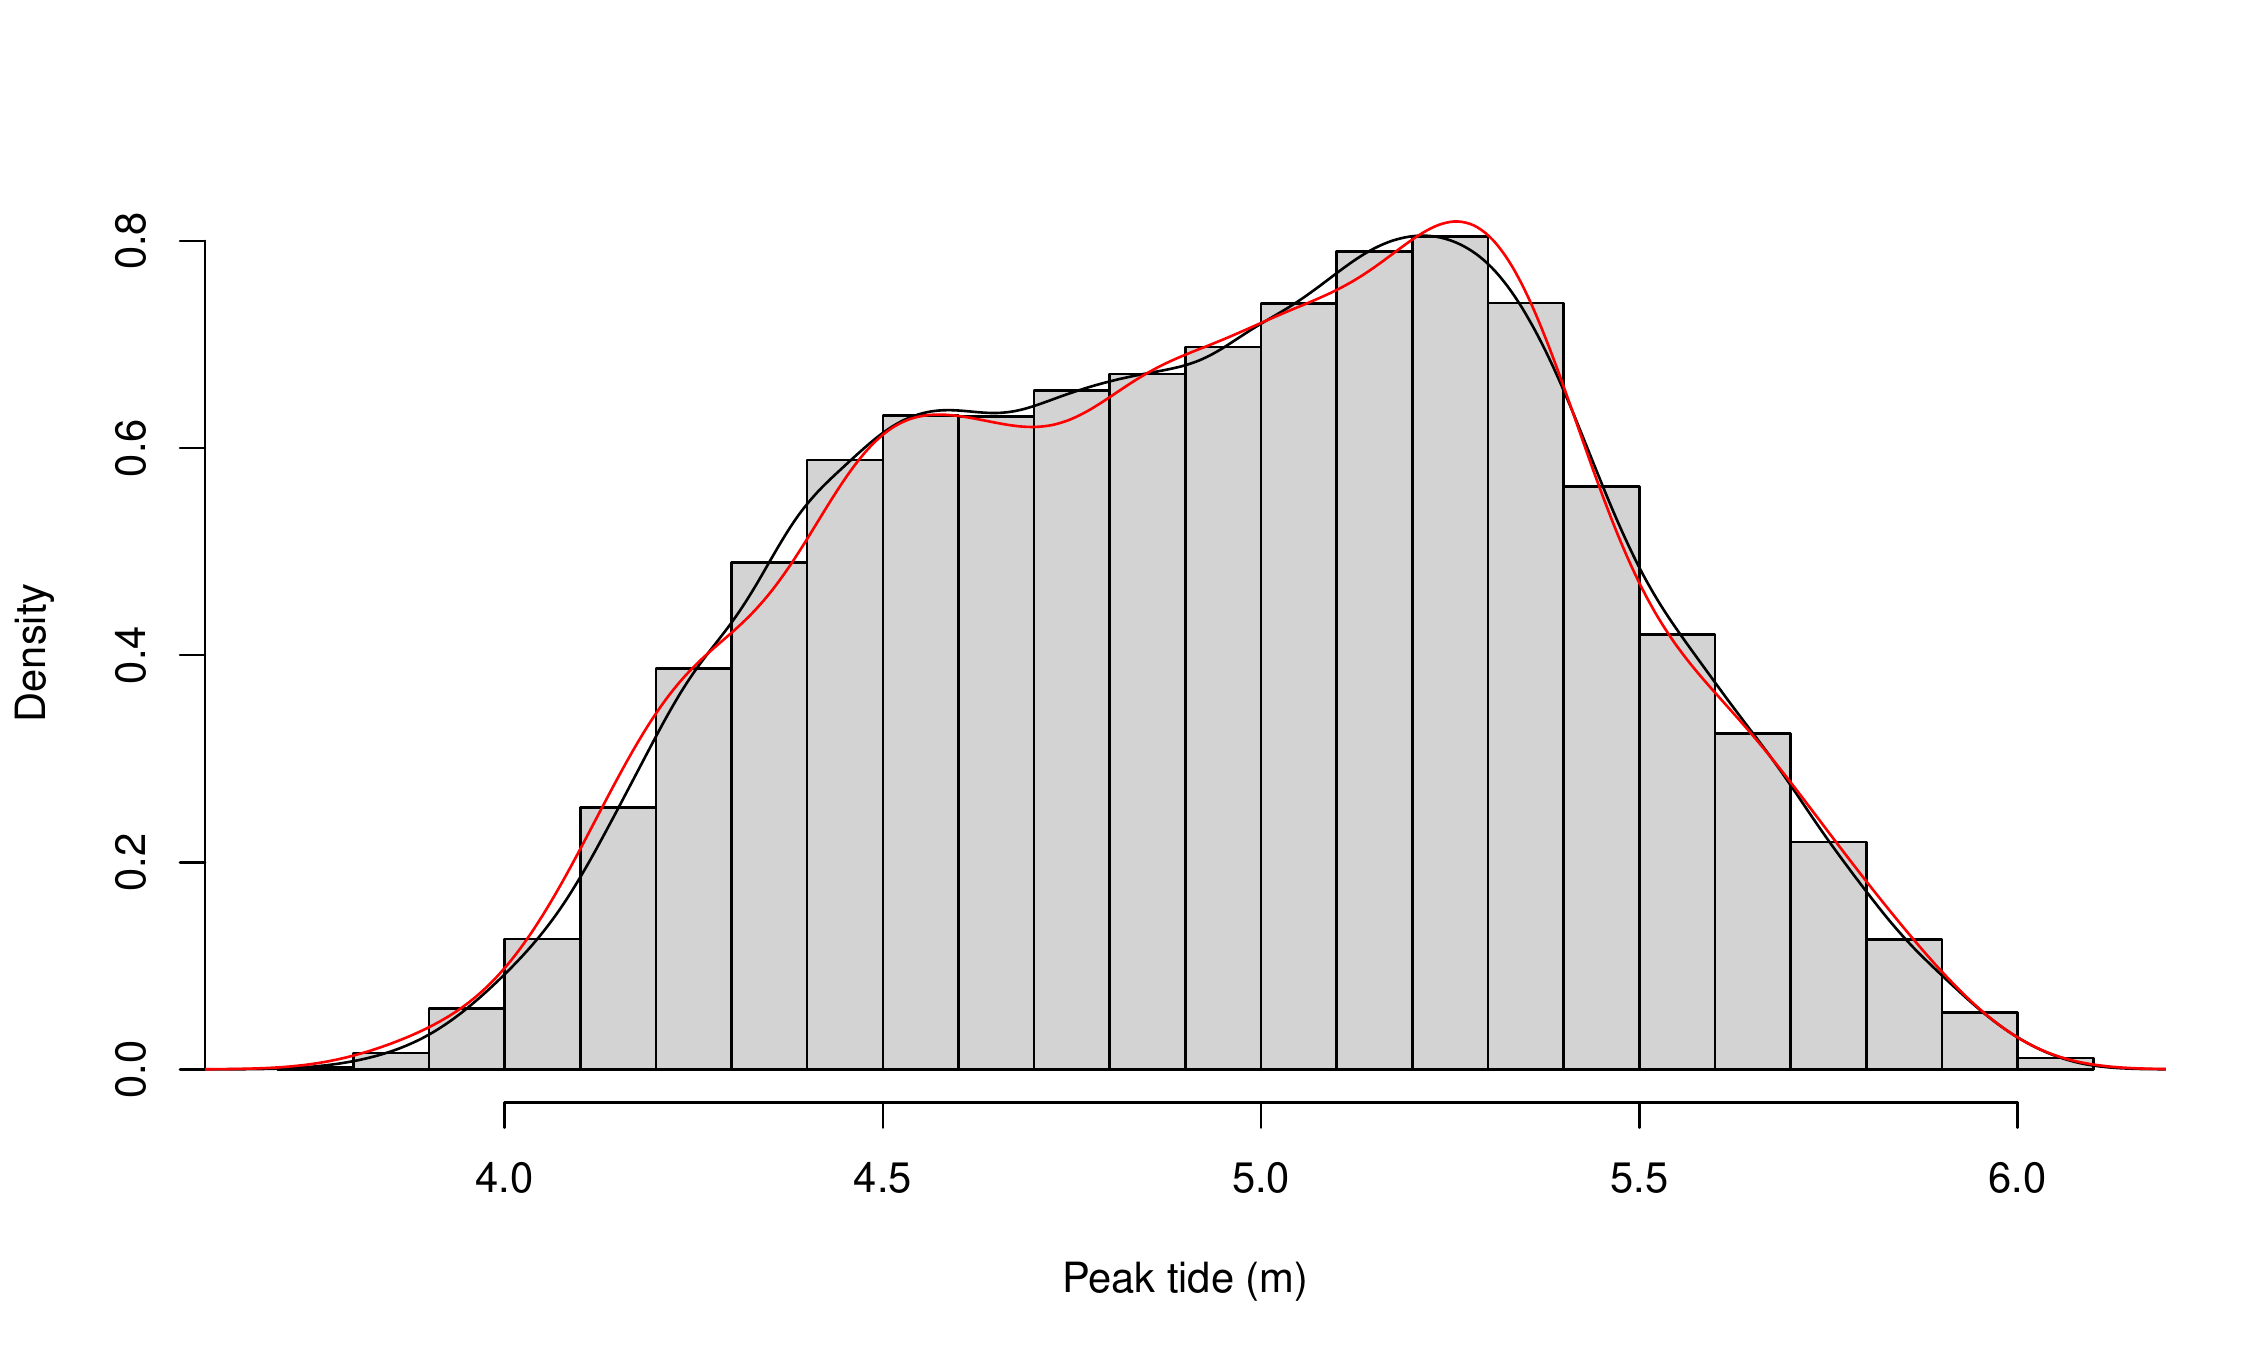}\includegraphics[width=0.4\textwidth]{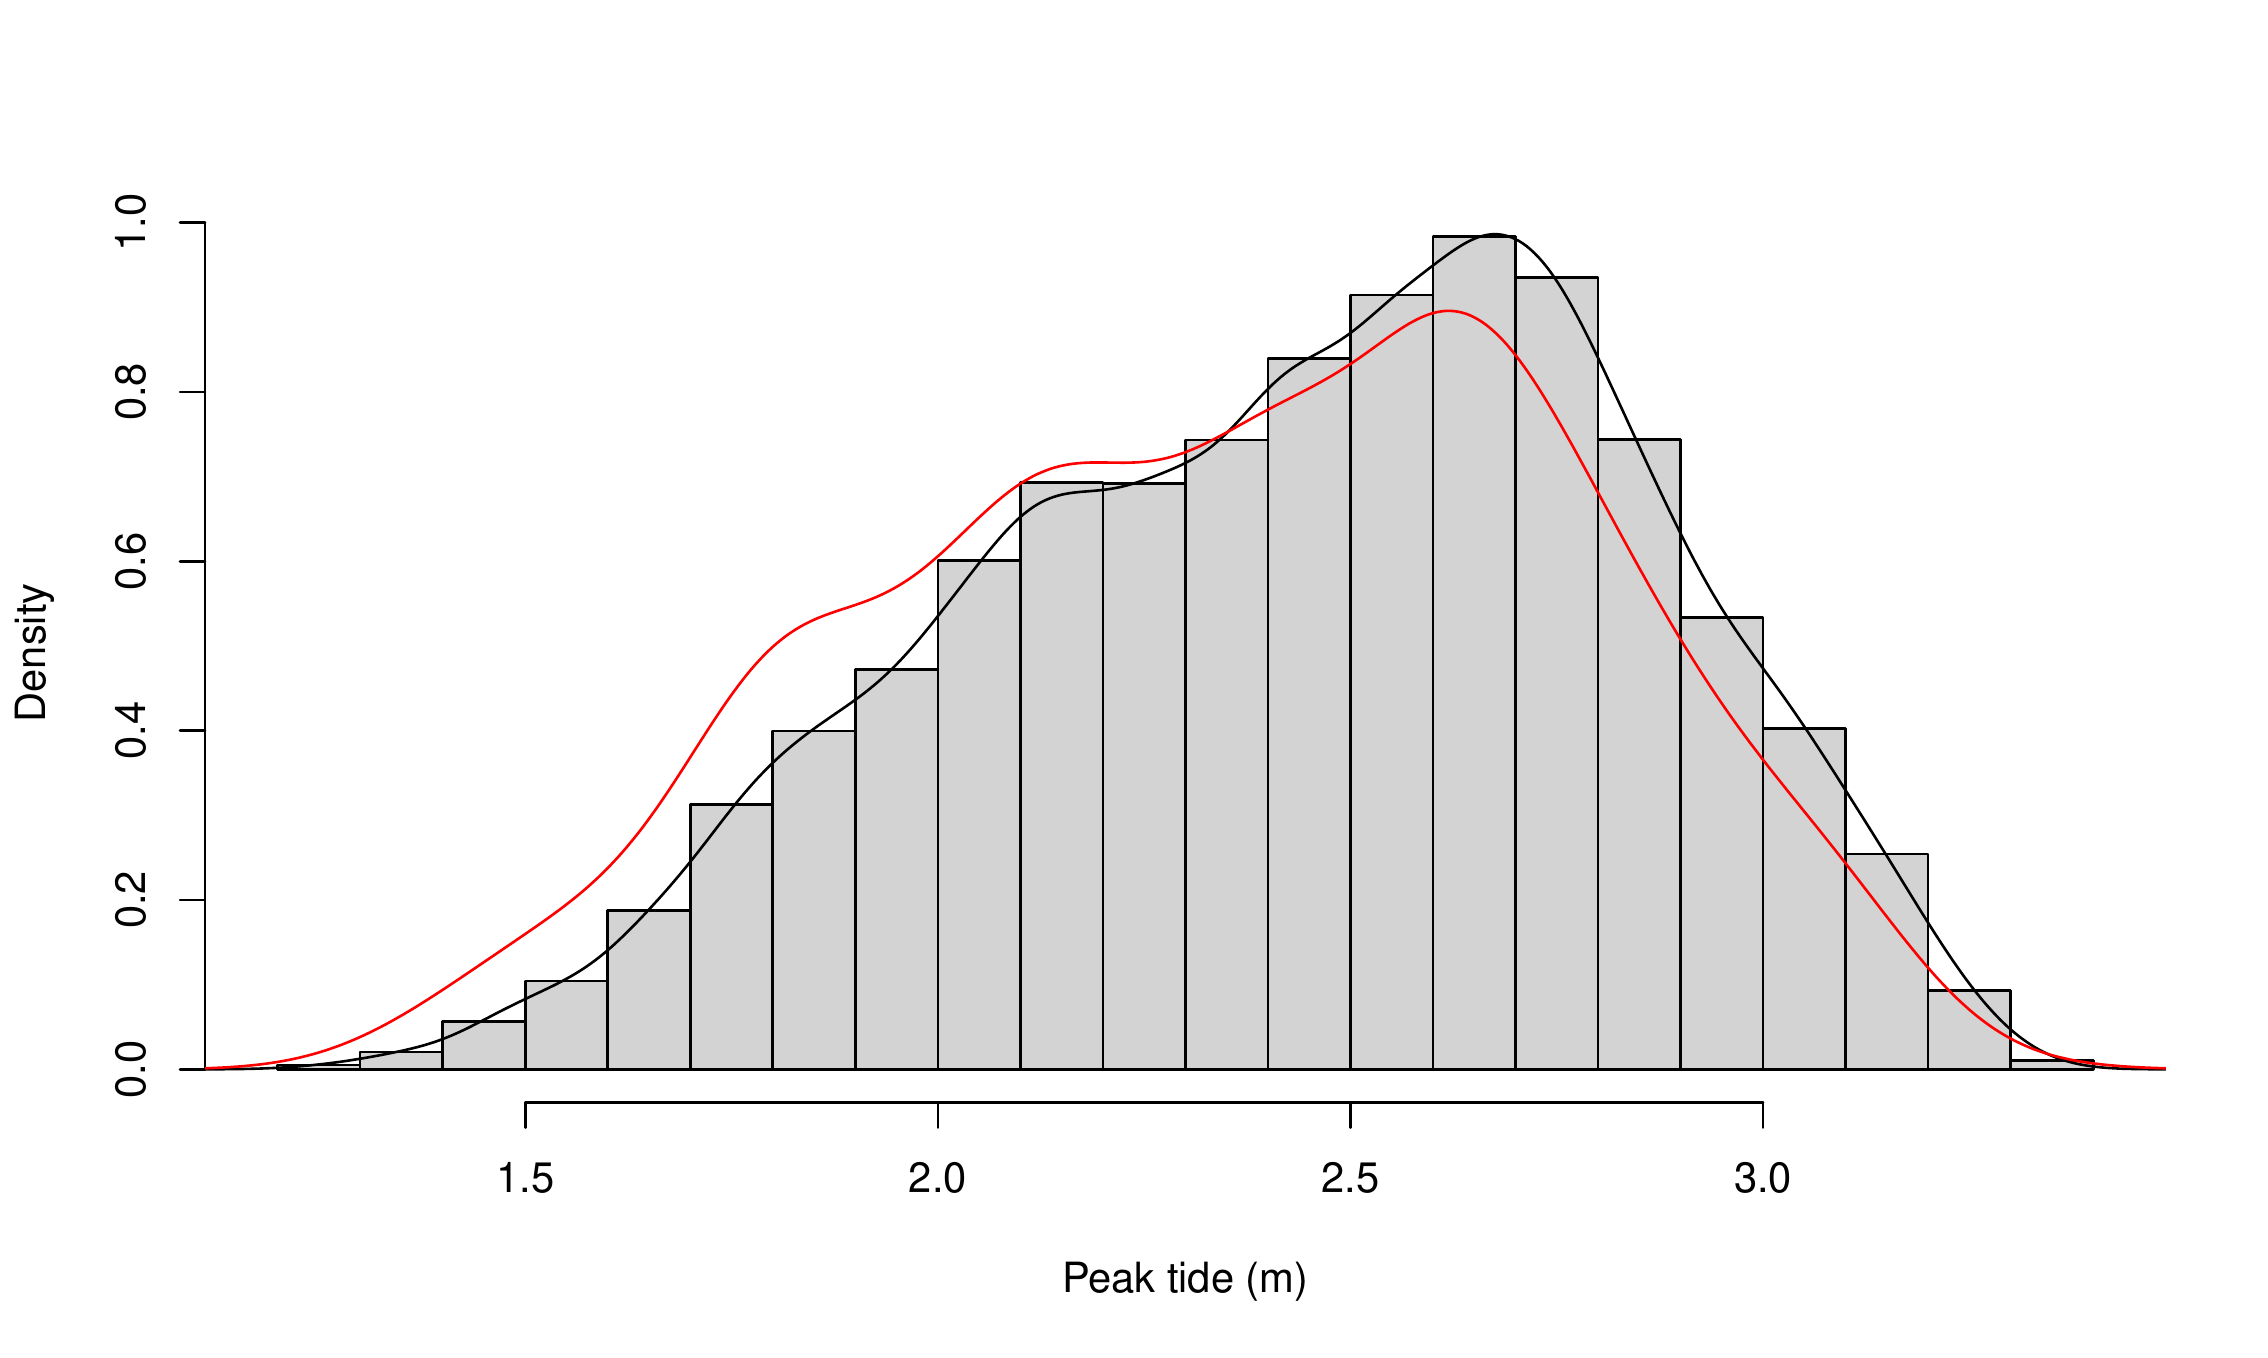}
    \caption{Distribution of peak tides at Heysham (top left), Lowestoft (top right), Newlyn (bottom left) and Sheerness (bottom right). Probability density function of all peak tides (black) and probability density function peak tides associated with extreme skew surges (red) are interpolated onto each distribution.}
    \label{pdf_mt}
\end{figure}

\begin{figure}
    \centering
    \includegraphics[width=0.45\textwidth]{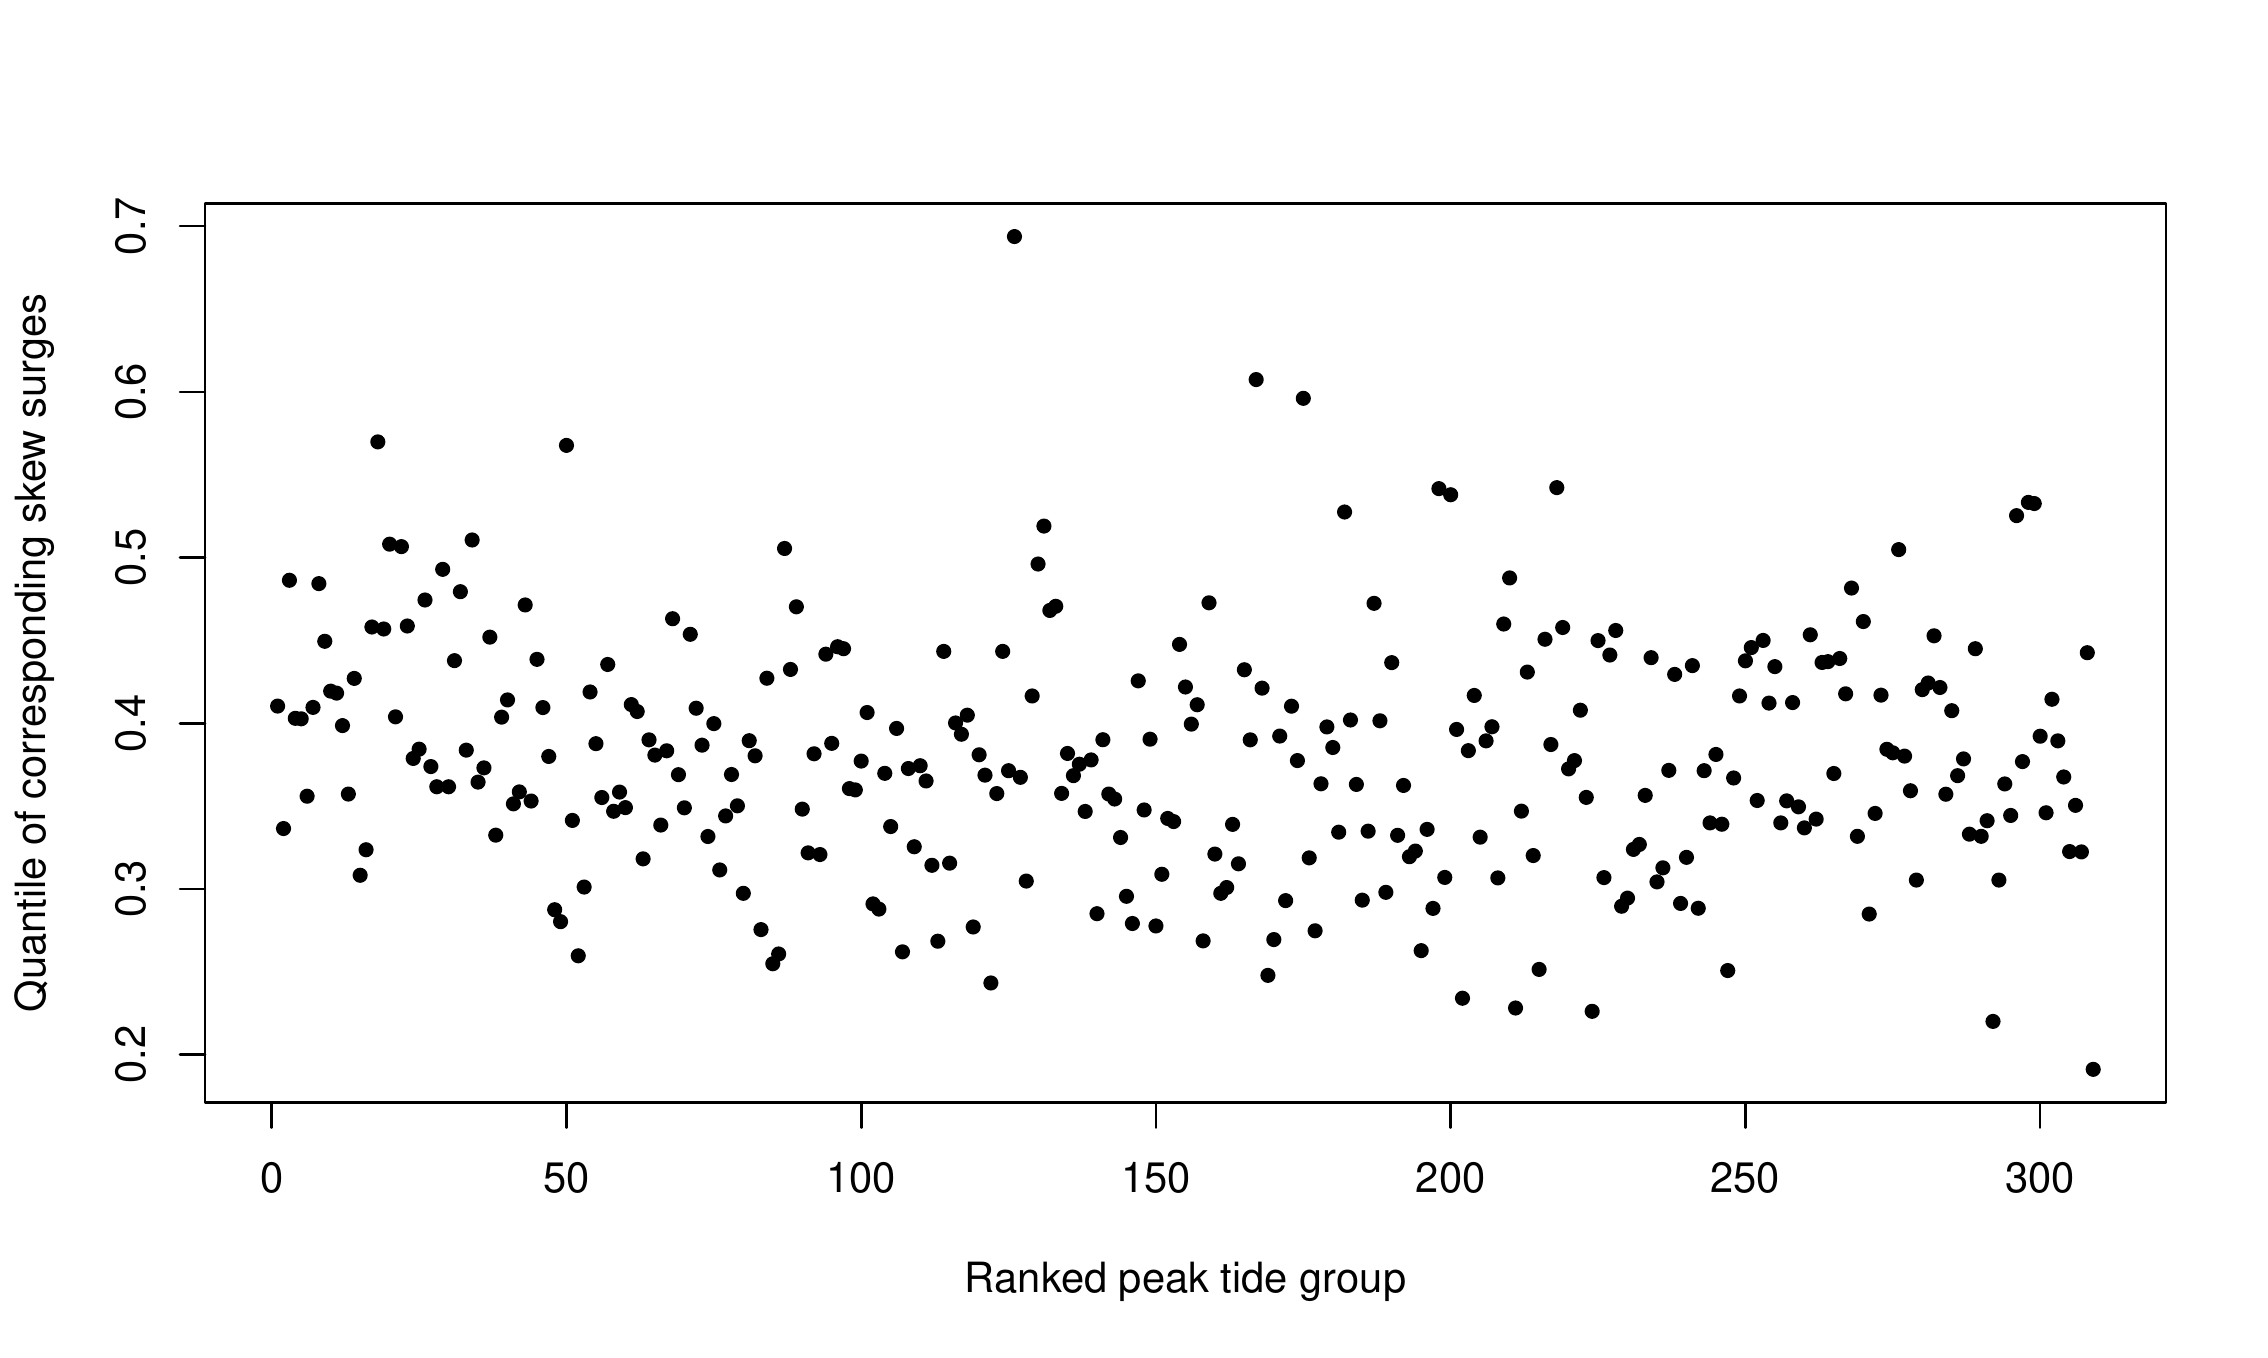}\includegraphics[width=0.45\textwidth]{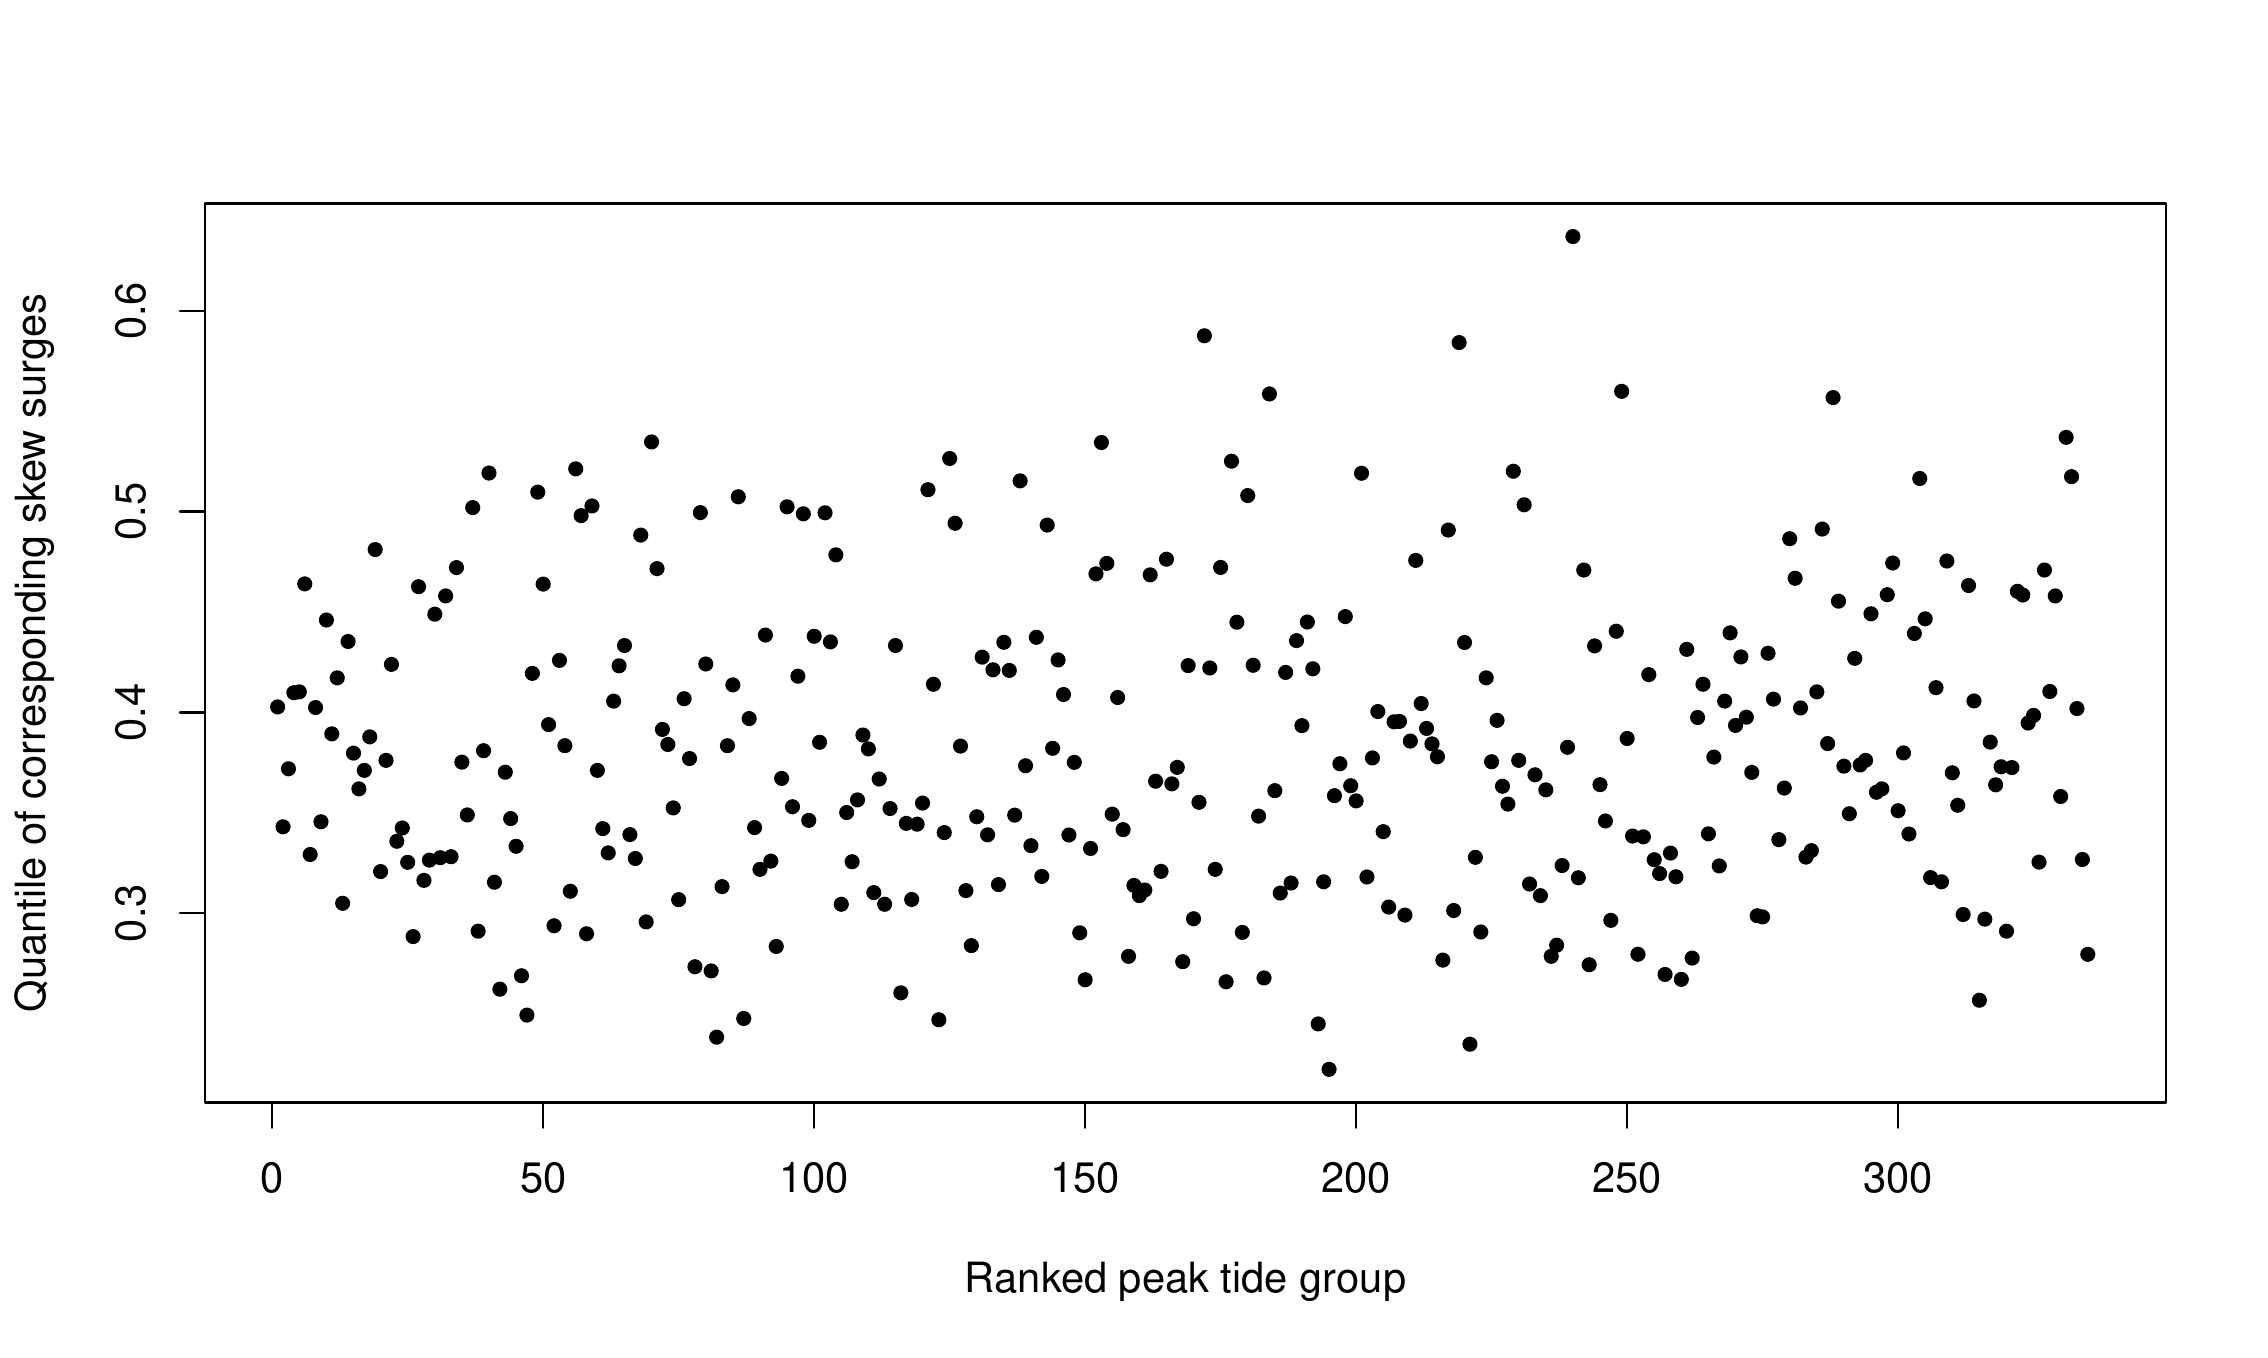}\\
    \includegraphics[width=0.45\textwidth]{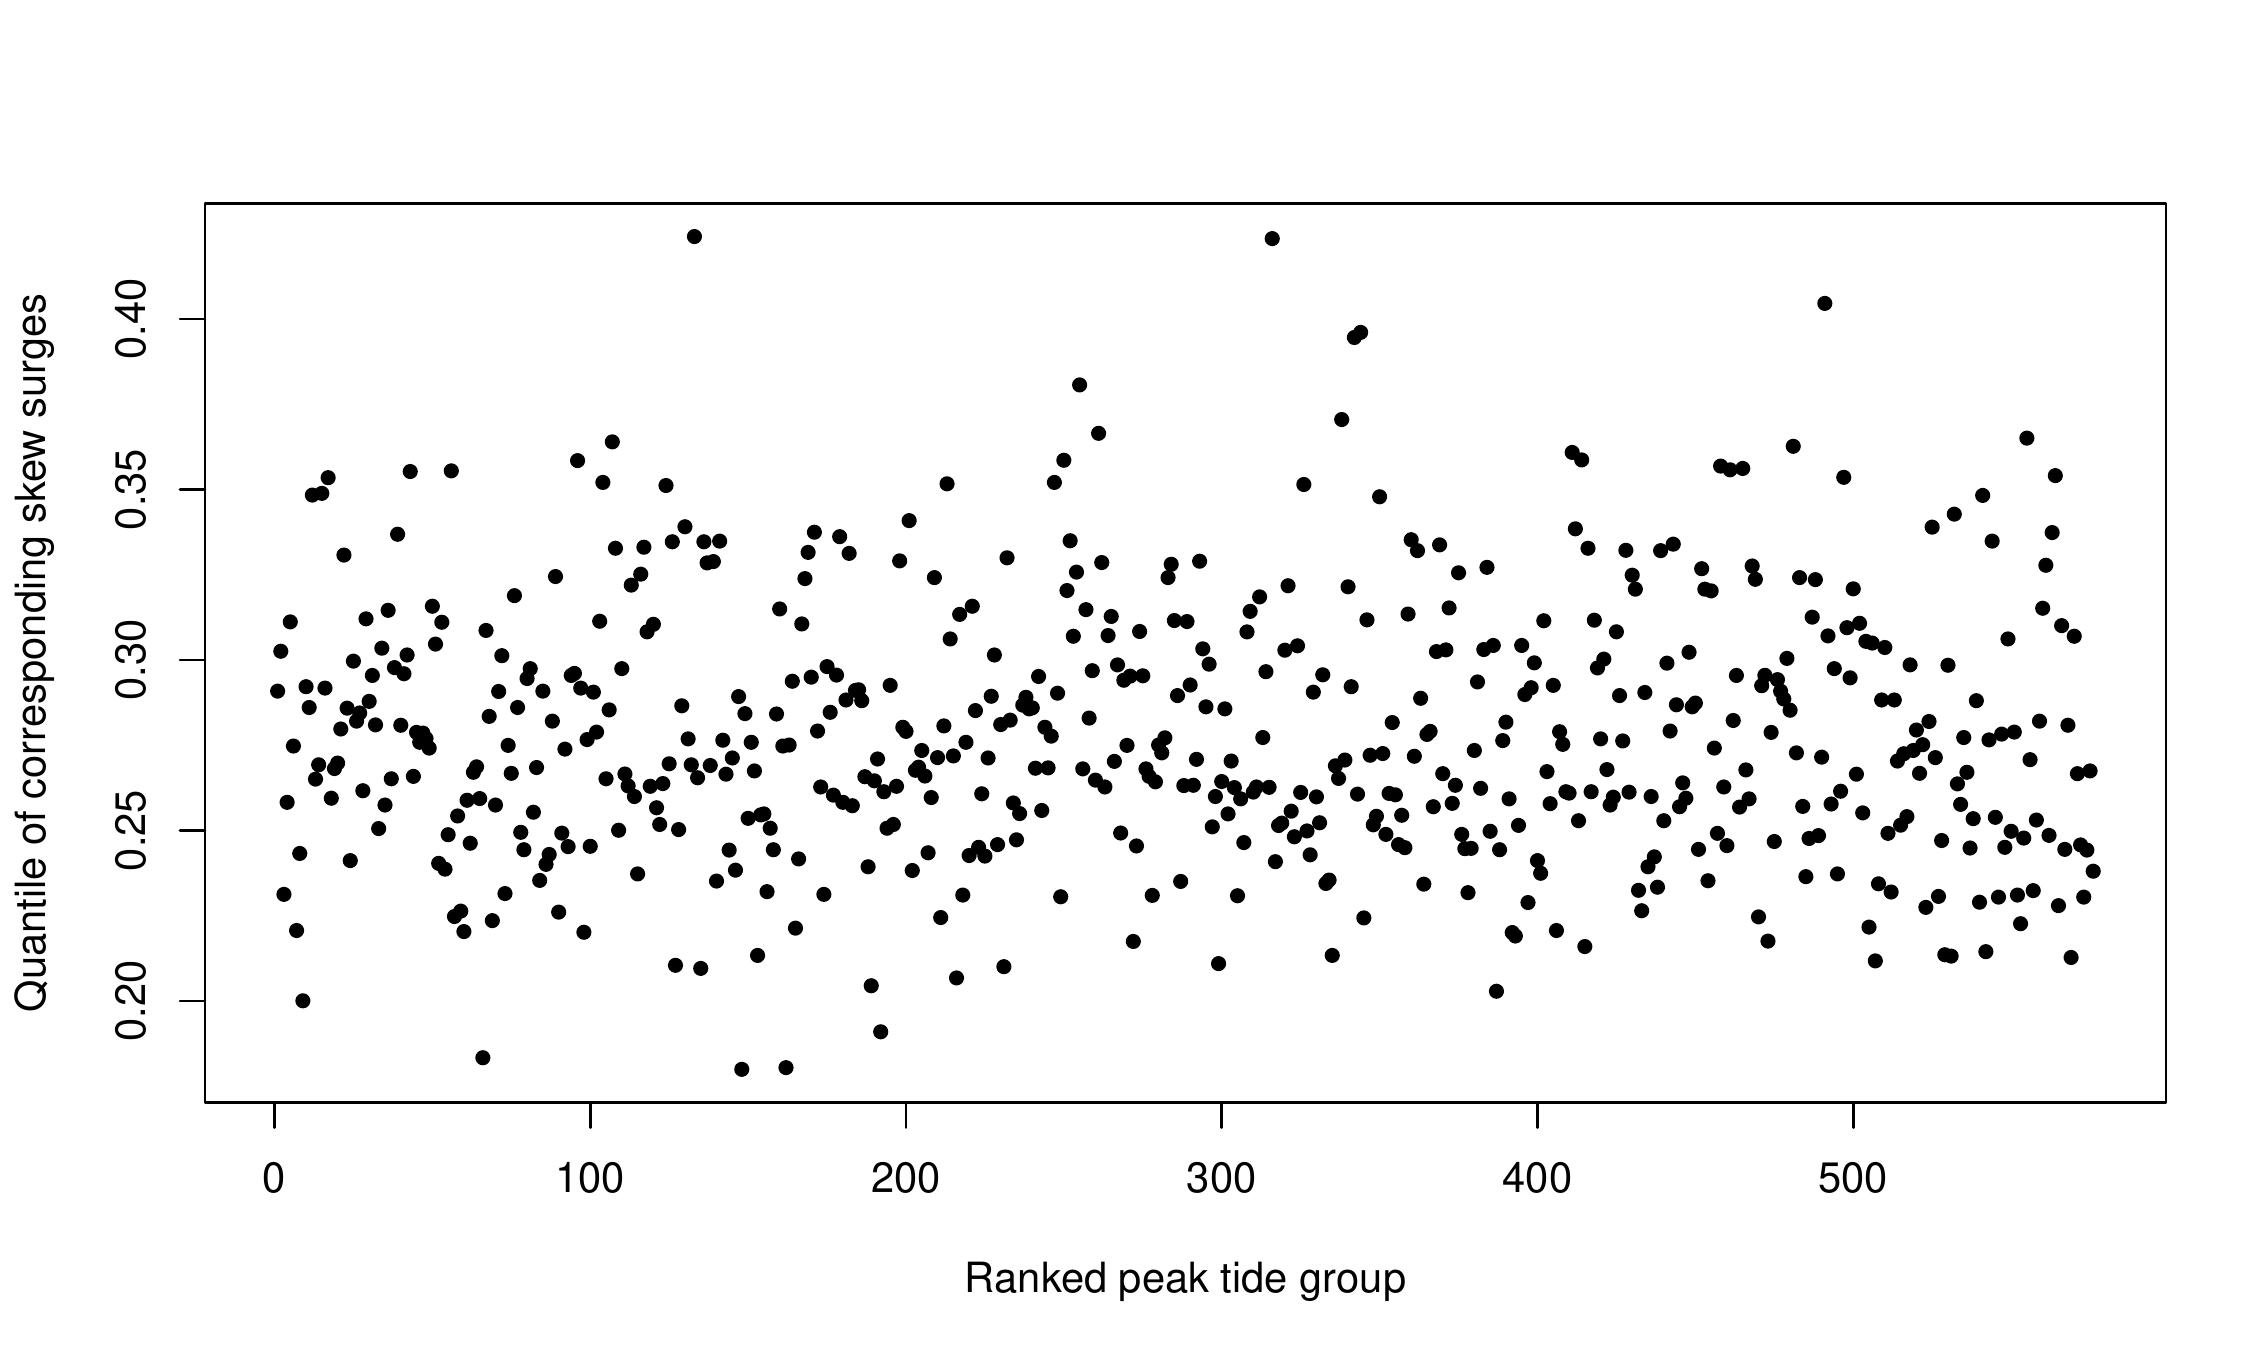}\includegraphics[width=0.45\textwidth]{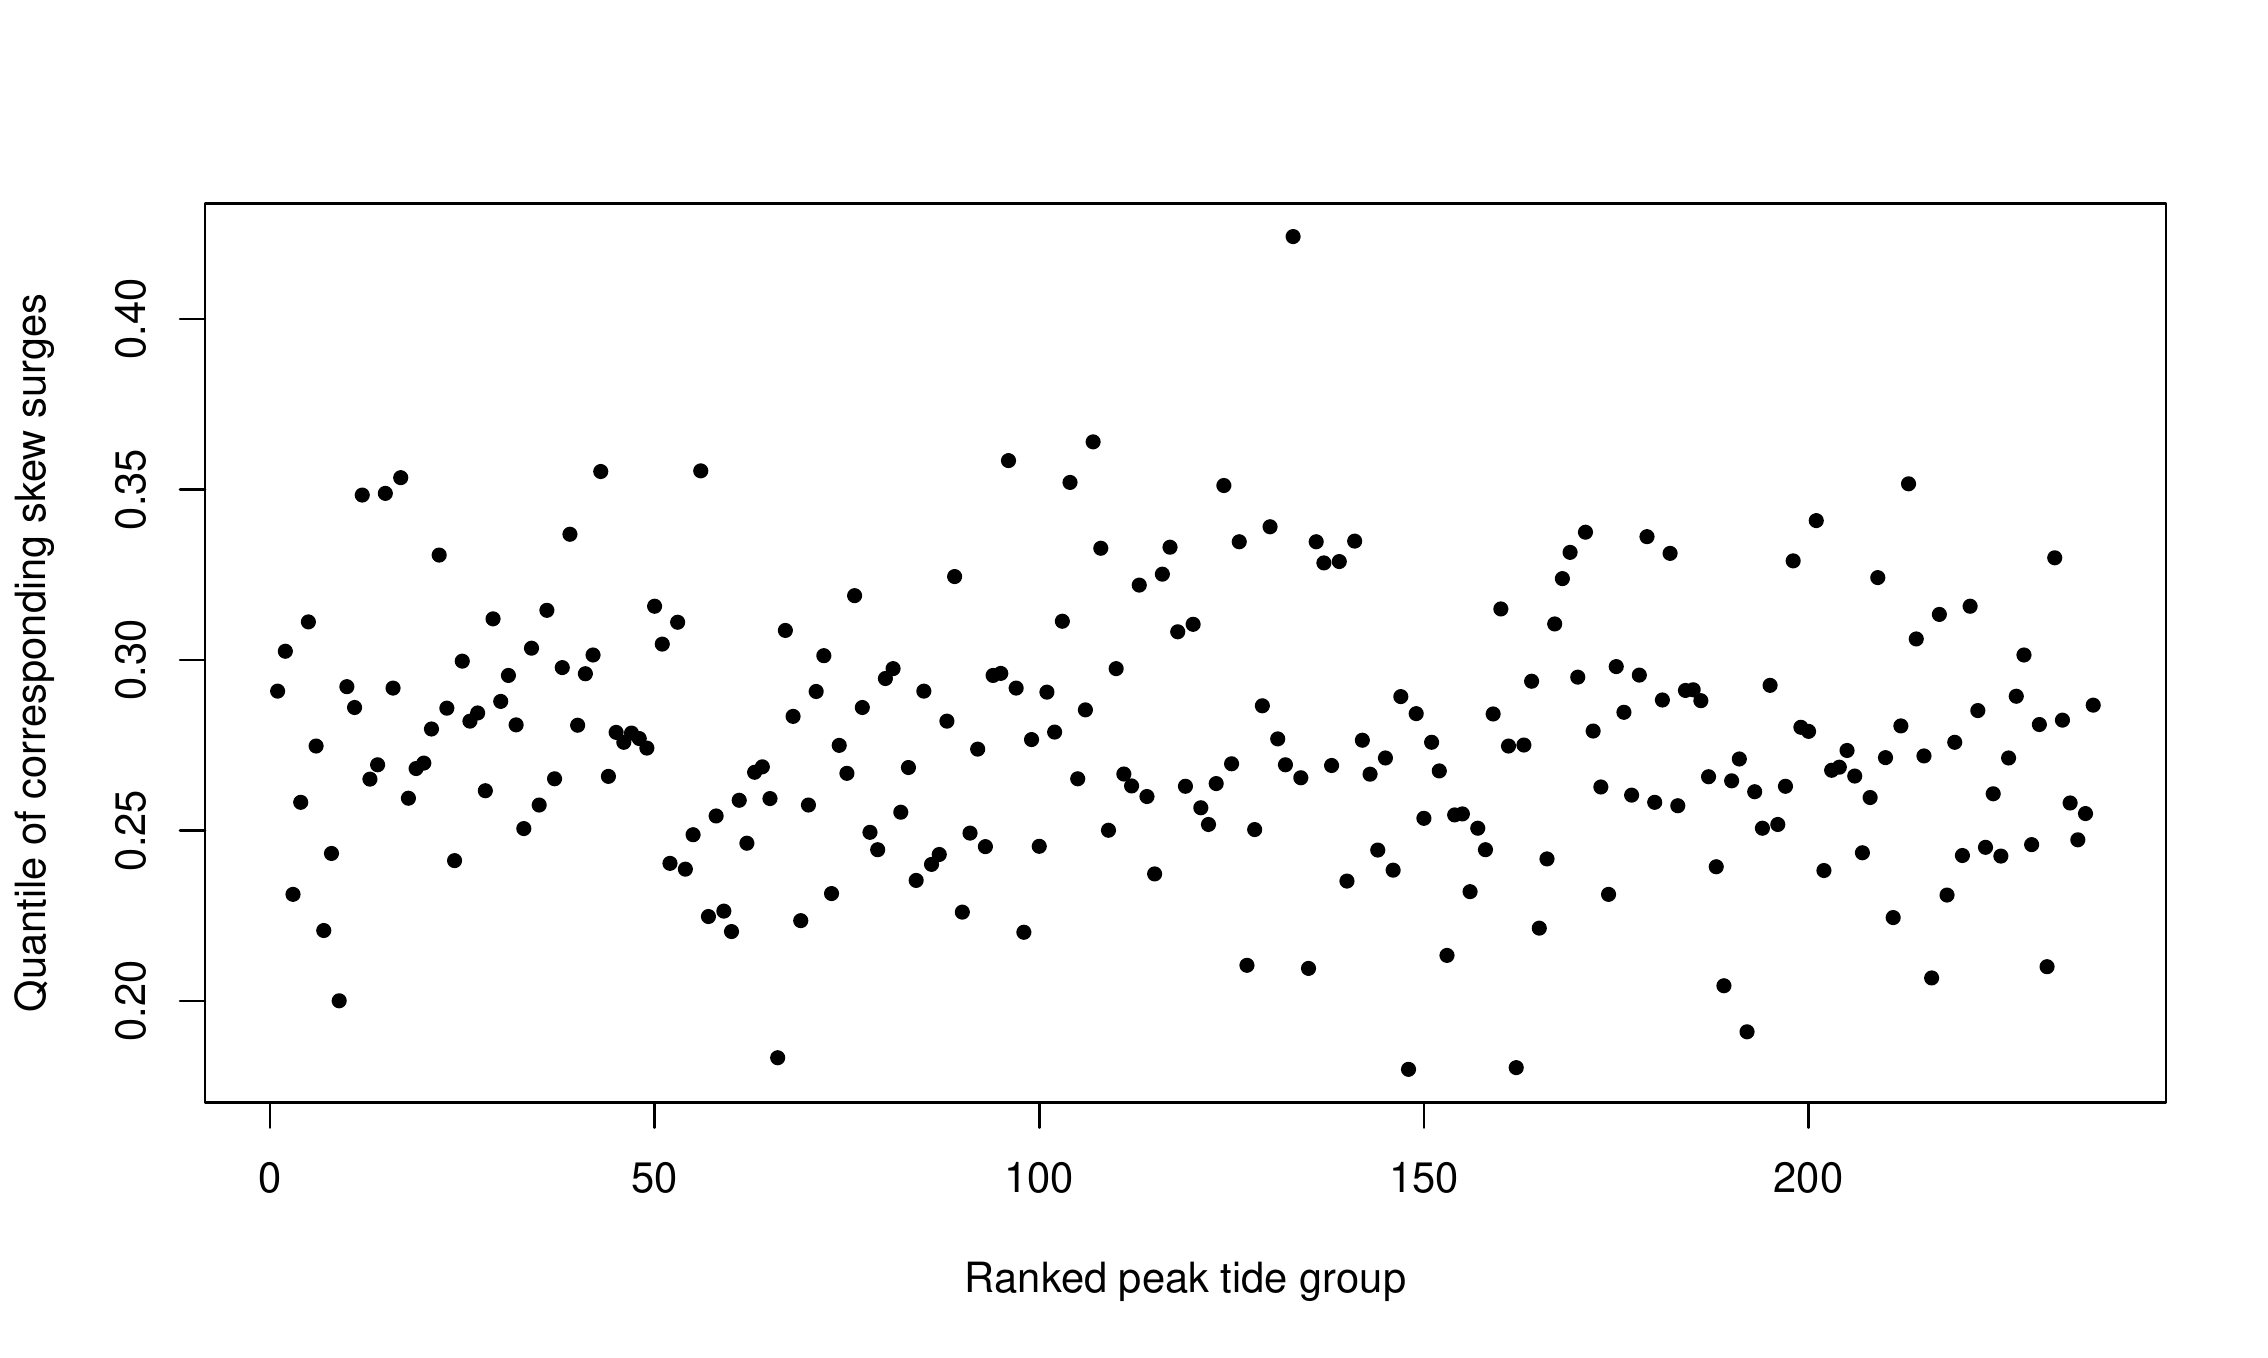}
    \caption{0.95 quantile estimates of skew surges associated with groups of ordered peak tides of size 100, at Heysham (top left), Lowestoft (top right), Newlyn (bottom left) and Sheerness (bottom right).}
    \label{quantile_reg}
\end{figure}

%\subsection{Parameter Estimates for Extreme Skew Surges}
%Figure \ref{ss_param_ests_fig_all} shows the GPD model parameter estimates for Lowestoft, Newlyn and Sheerness for the monthly model discussed in Section \ref{acc_ss_seasonality} and Model $B$, with scale parameter defined by equation \ref{sinescale}. Each site shows the same pattern in scale parameter as Heysham, in Figure \ref{ss_param_ests_fig_HEY}, where values are higher in Winter than Summer. Whereas, the monthly model shape parameter estimates remain relatively constant across months, except for May at Lowestoft. However, fixing the shape parameter across still yields the best model fit (see Table \ref{AICBIC_ss}). Notice that the 95\% confidence intervals on parameter estimates are much narrower at Newlyn due to the amount of data available. 

\begin{figure}[h]
    \entering
    \includegraphics[width=0.5\textwidth]{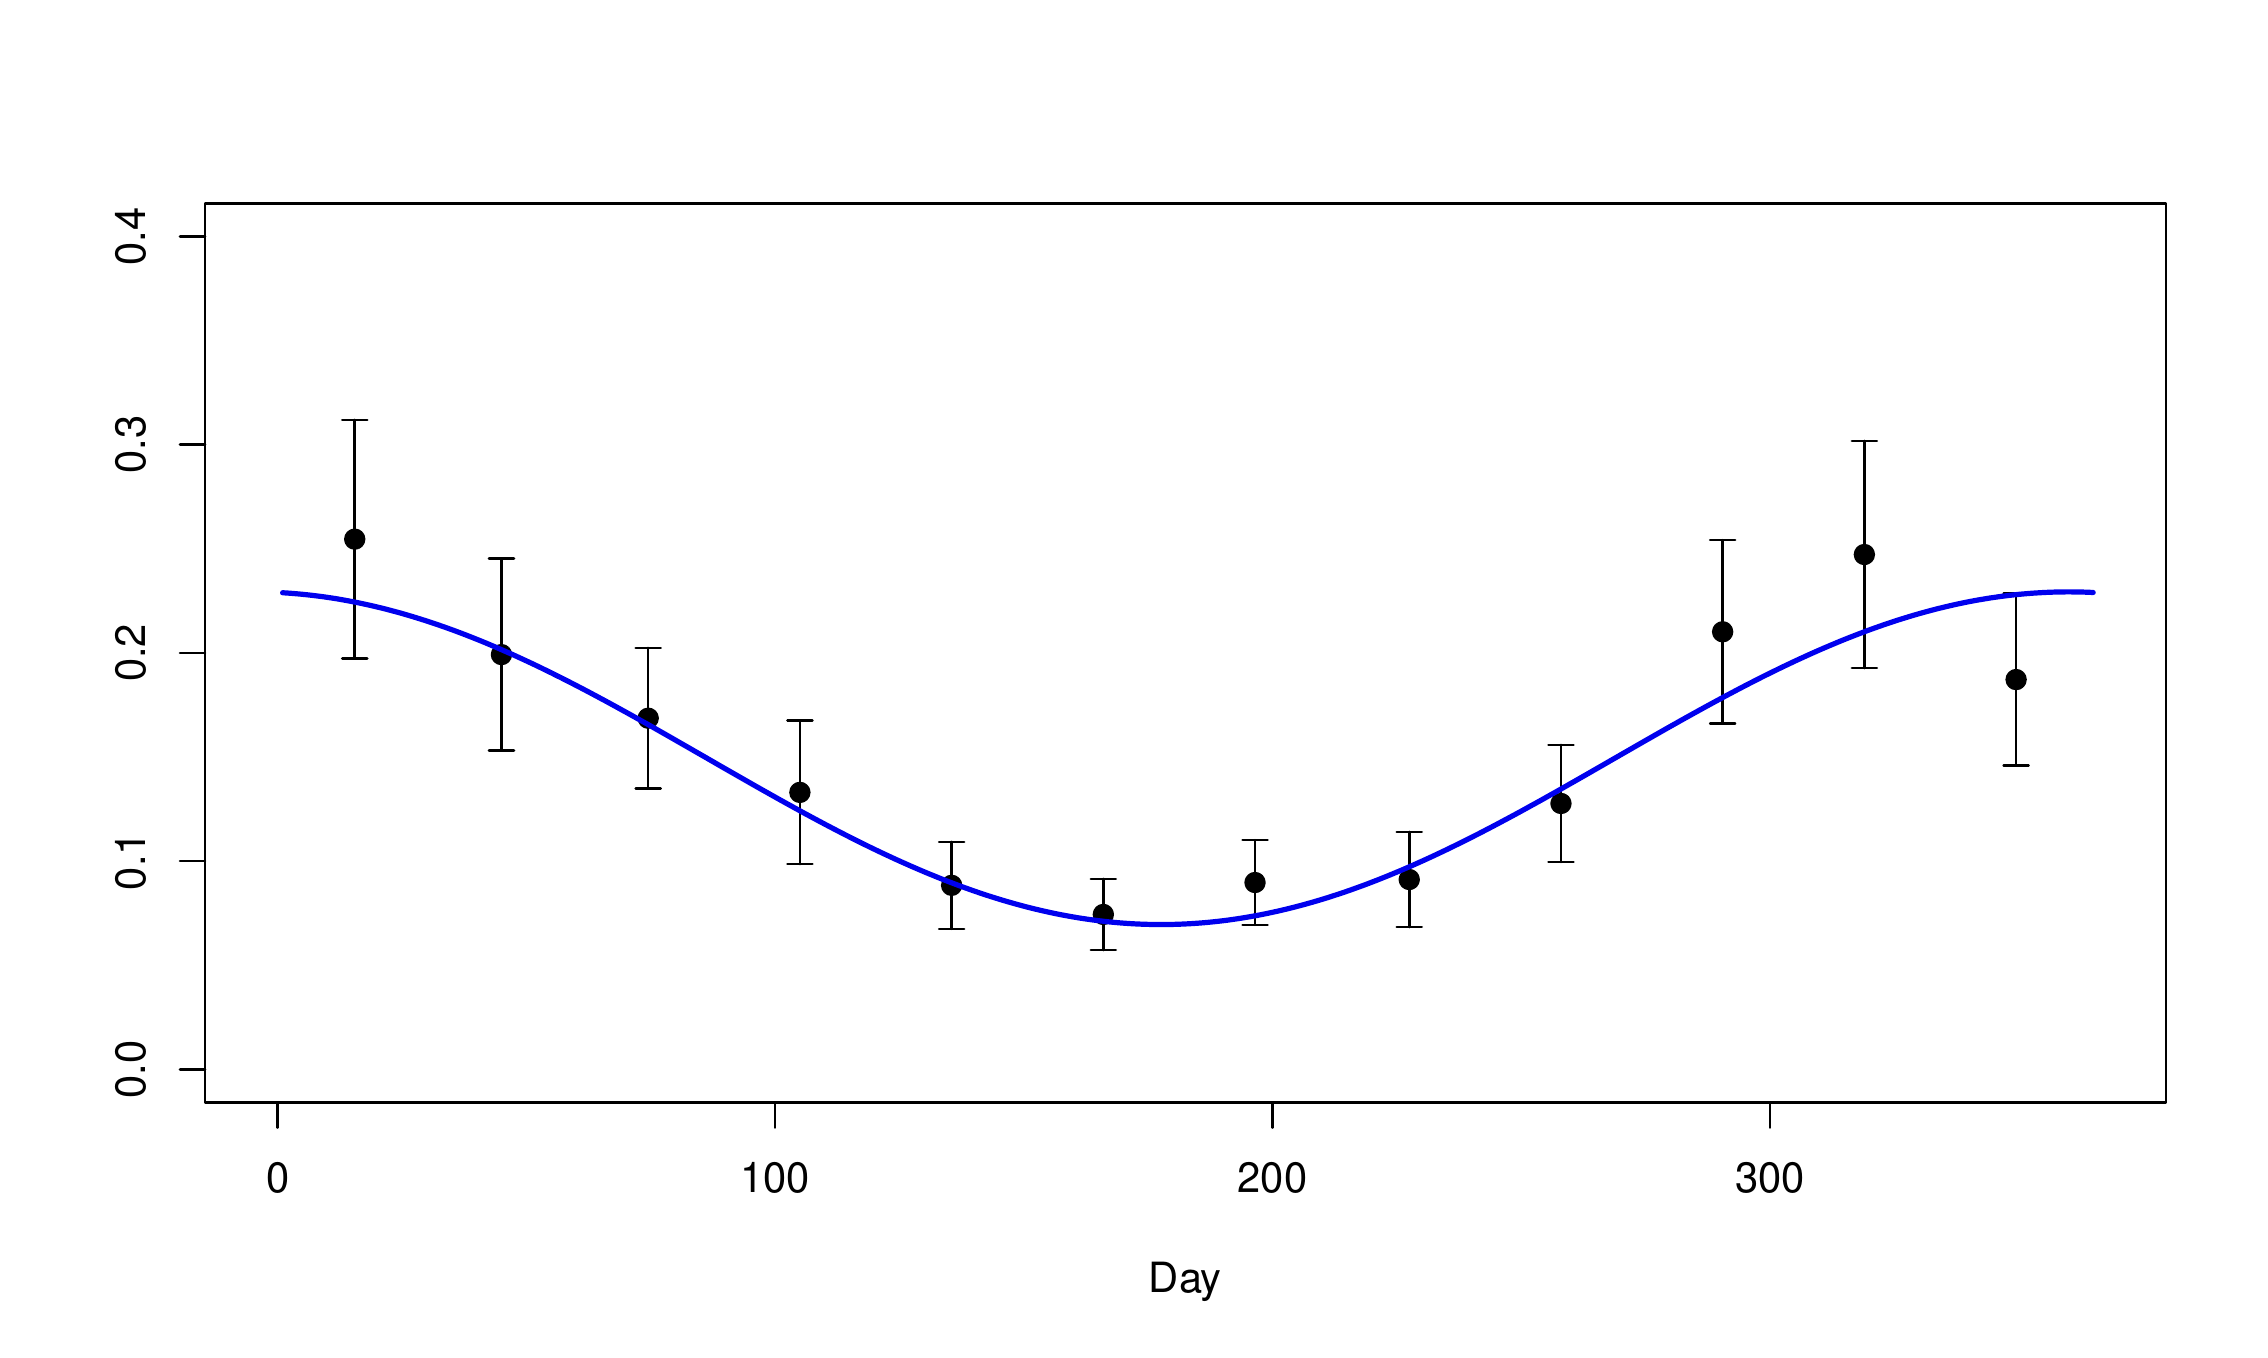}\includegraphics[width=0.5\textwidth]{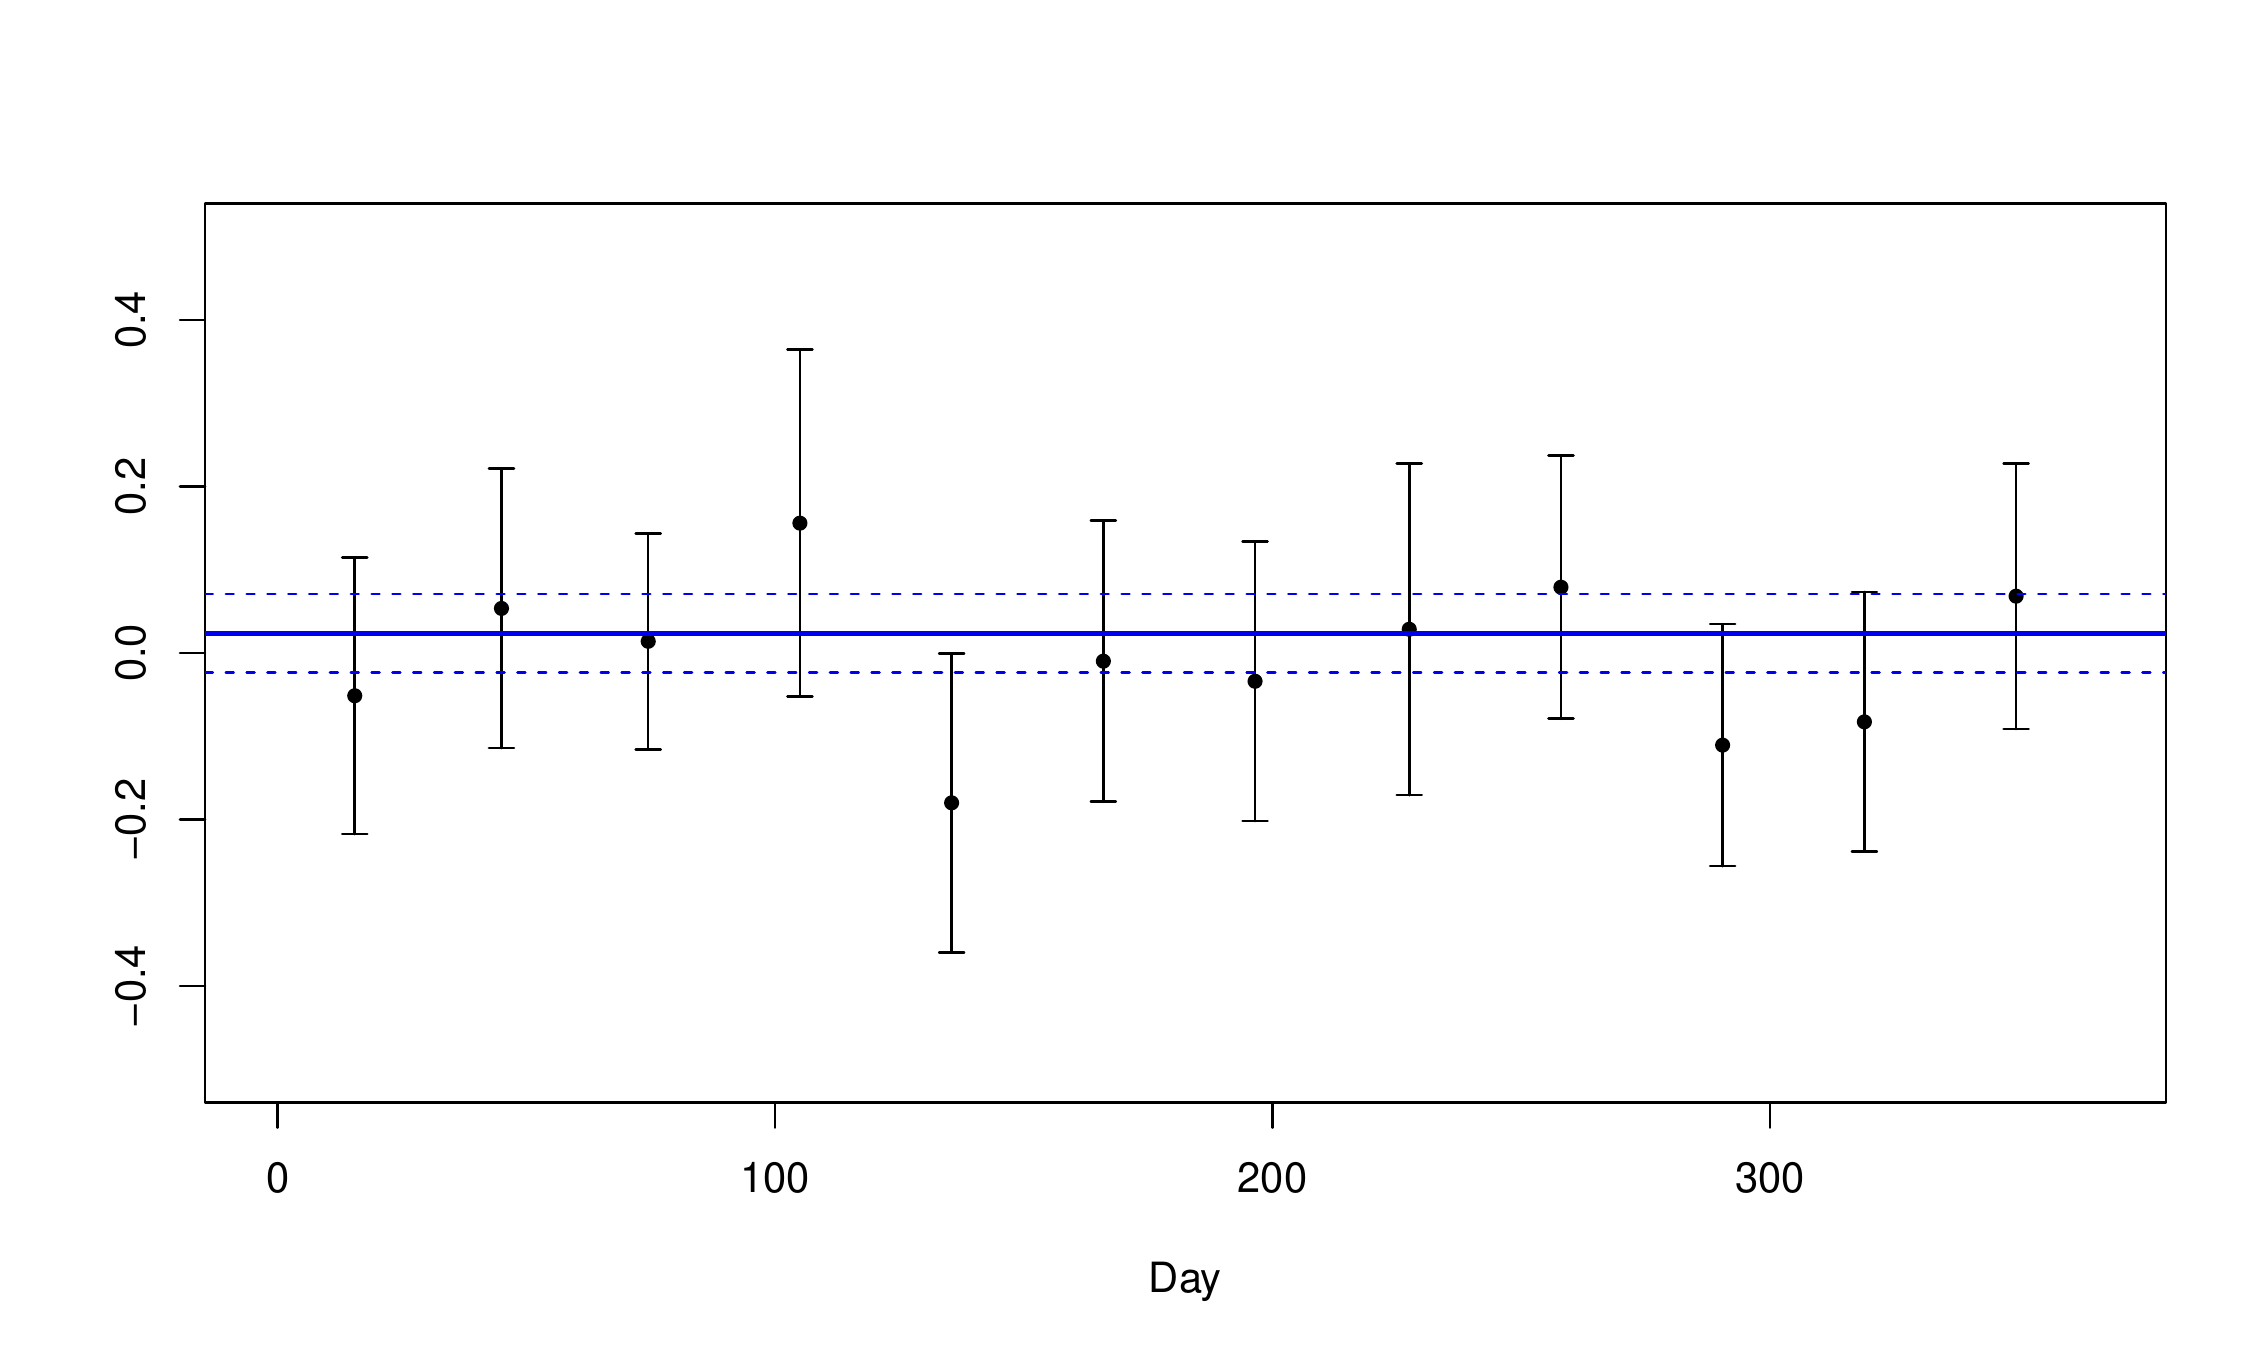}
    \includegraphics[width=0.5\textwidth]{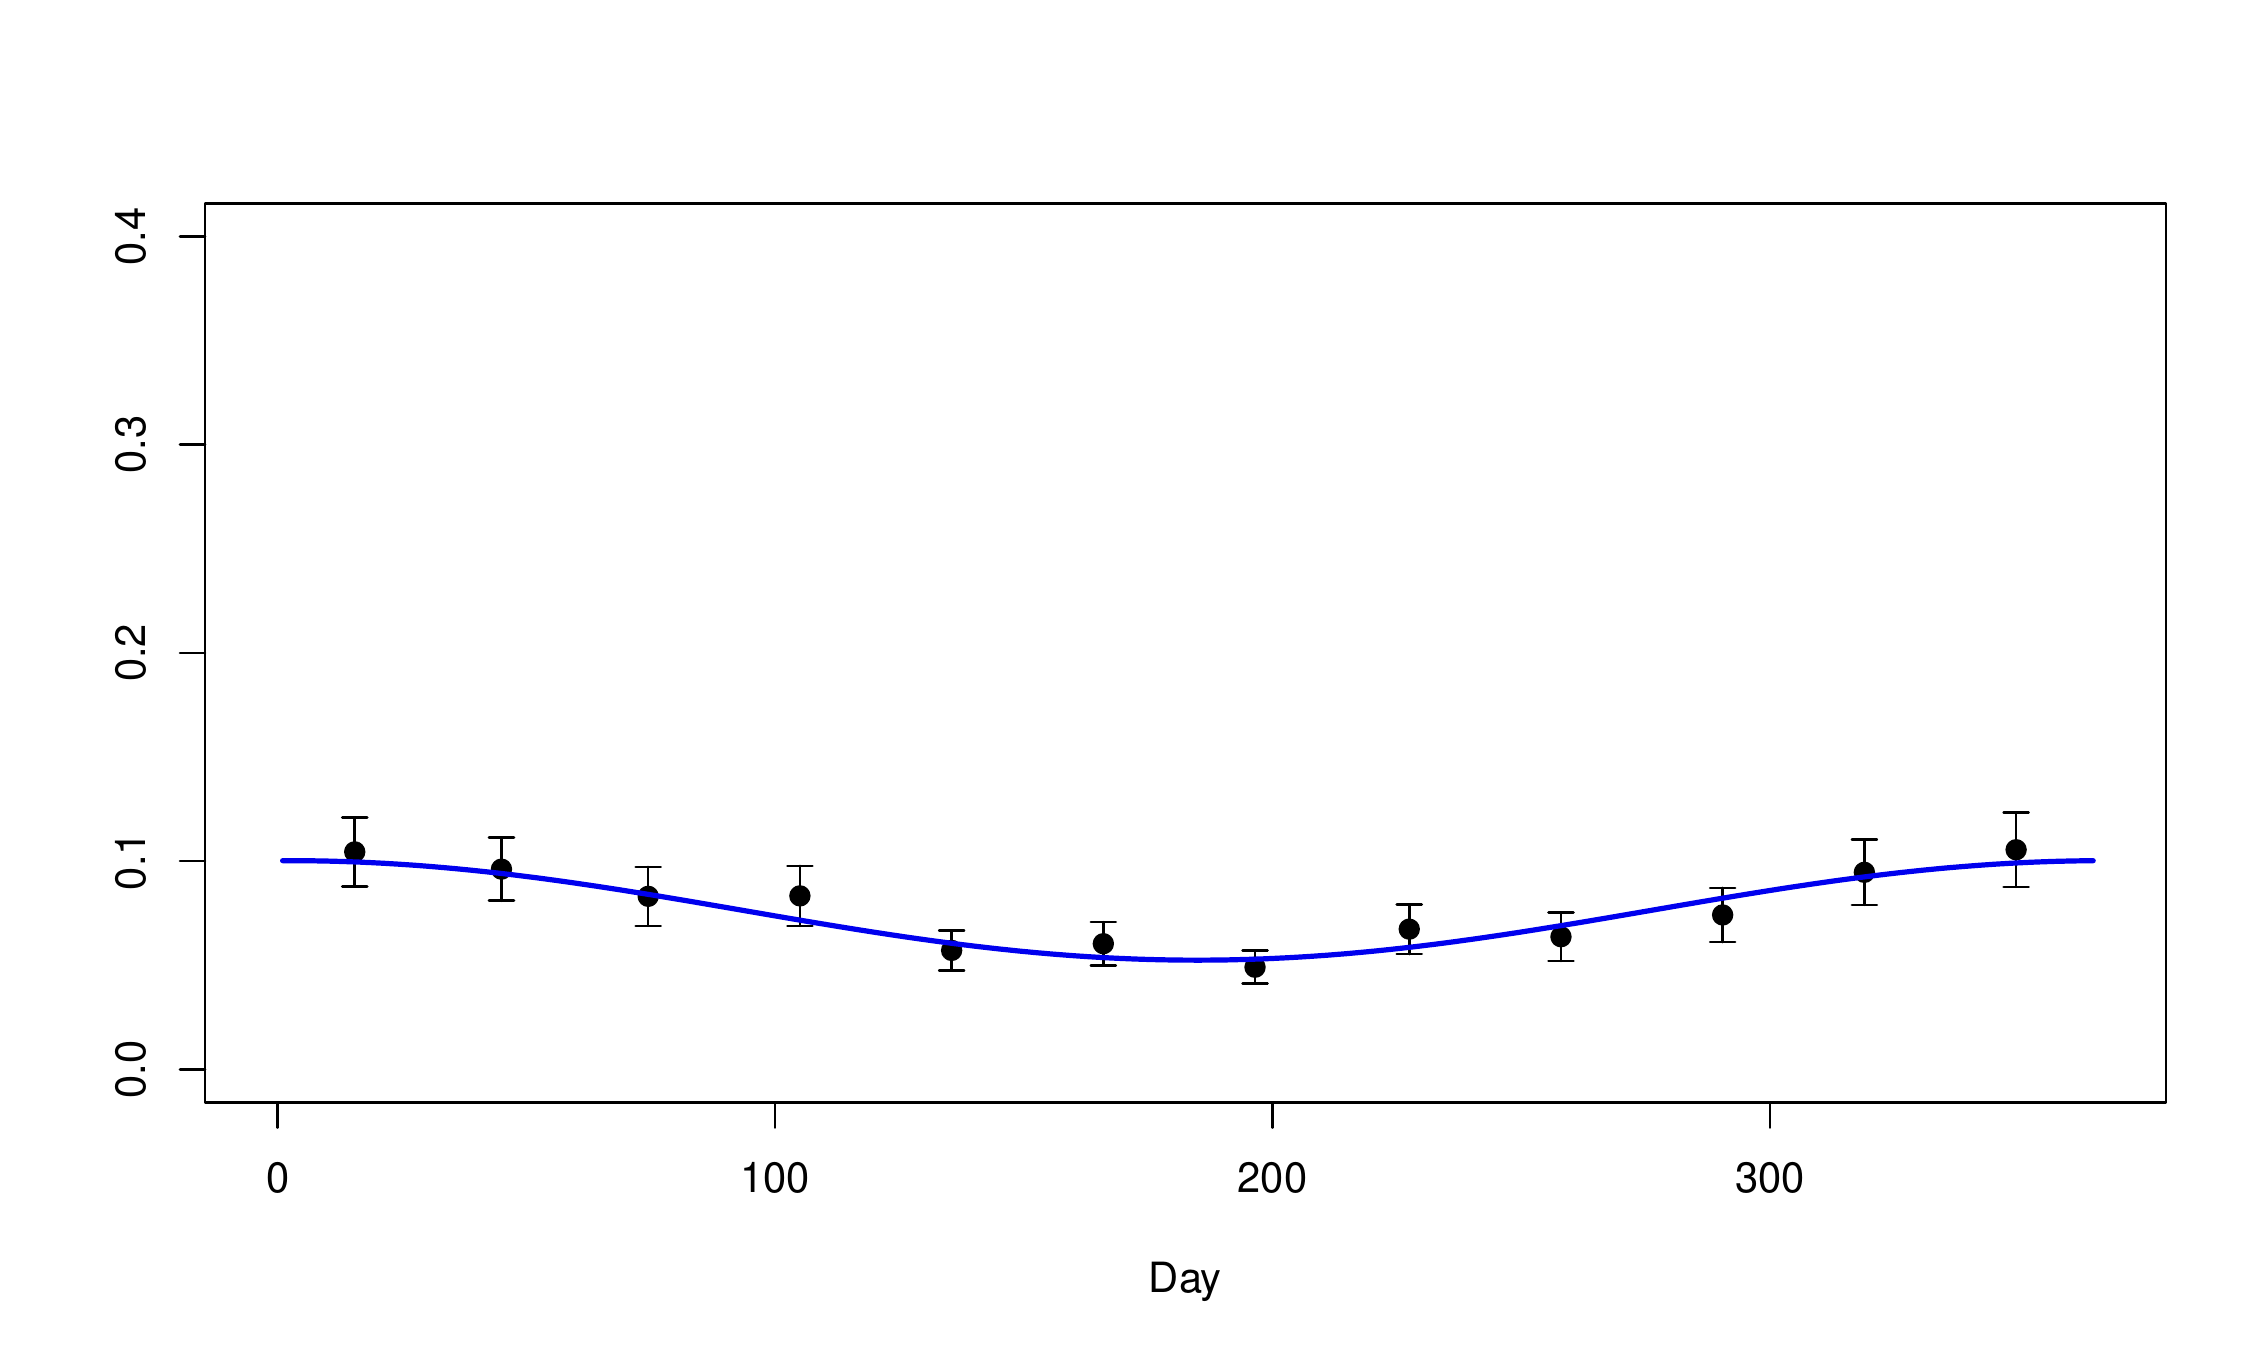}\includegraphics[width=0.5\textwidth]{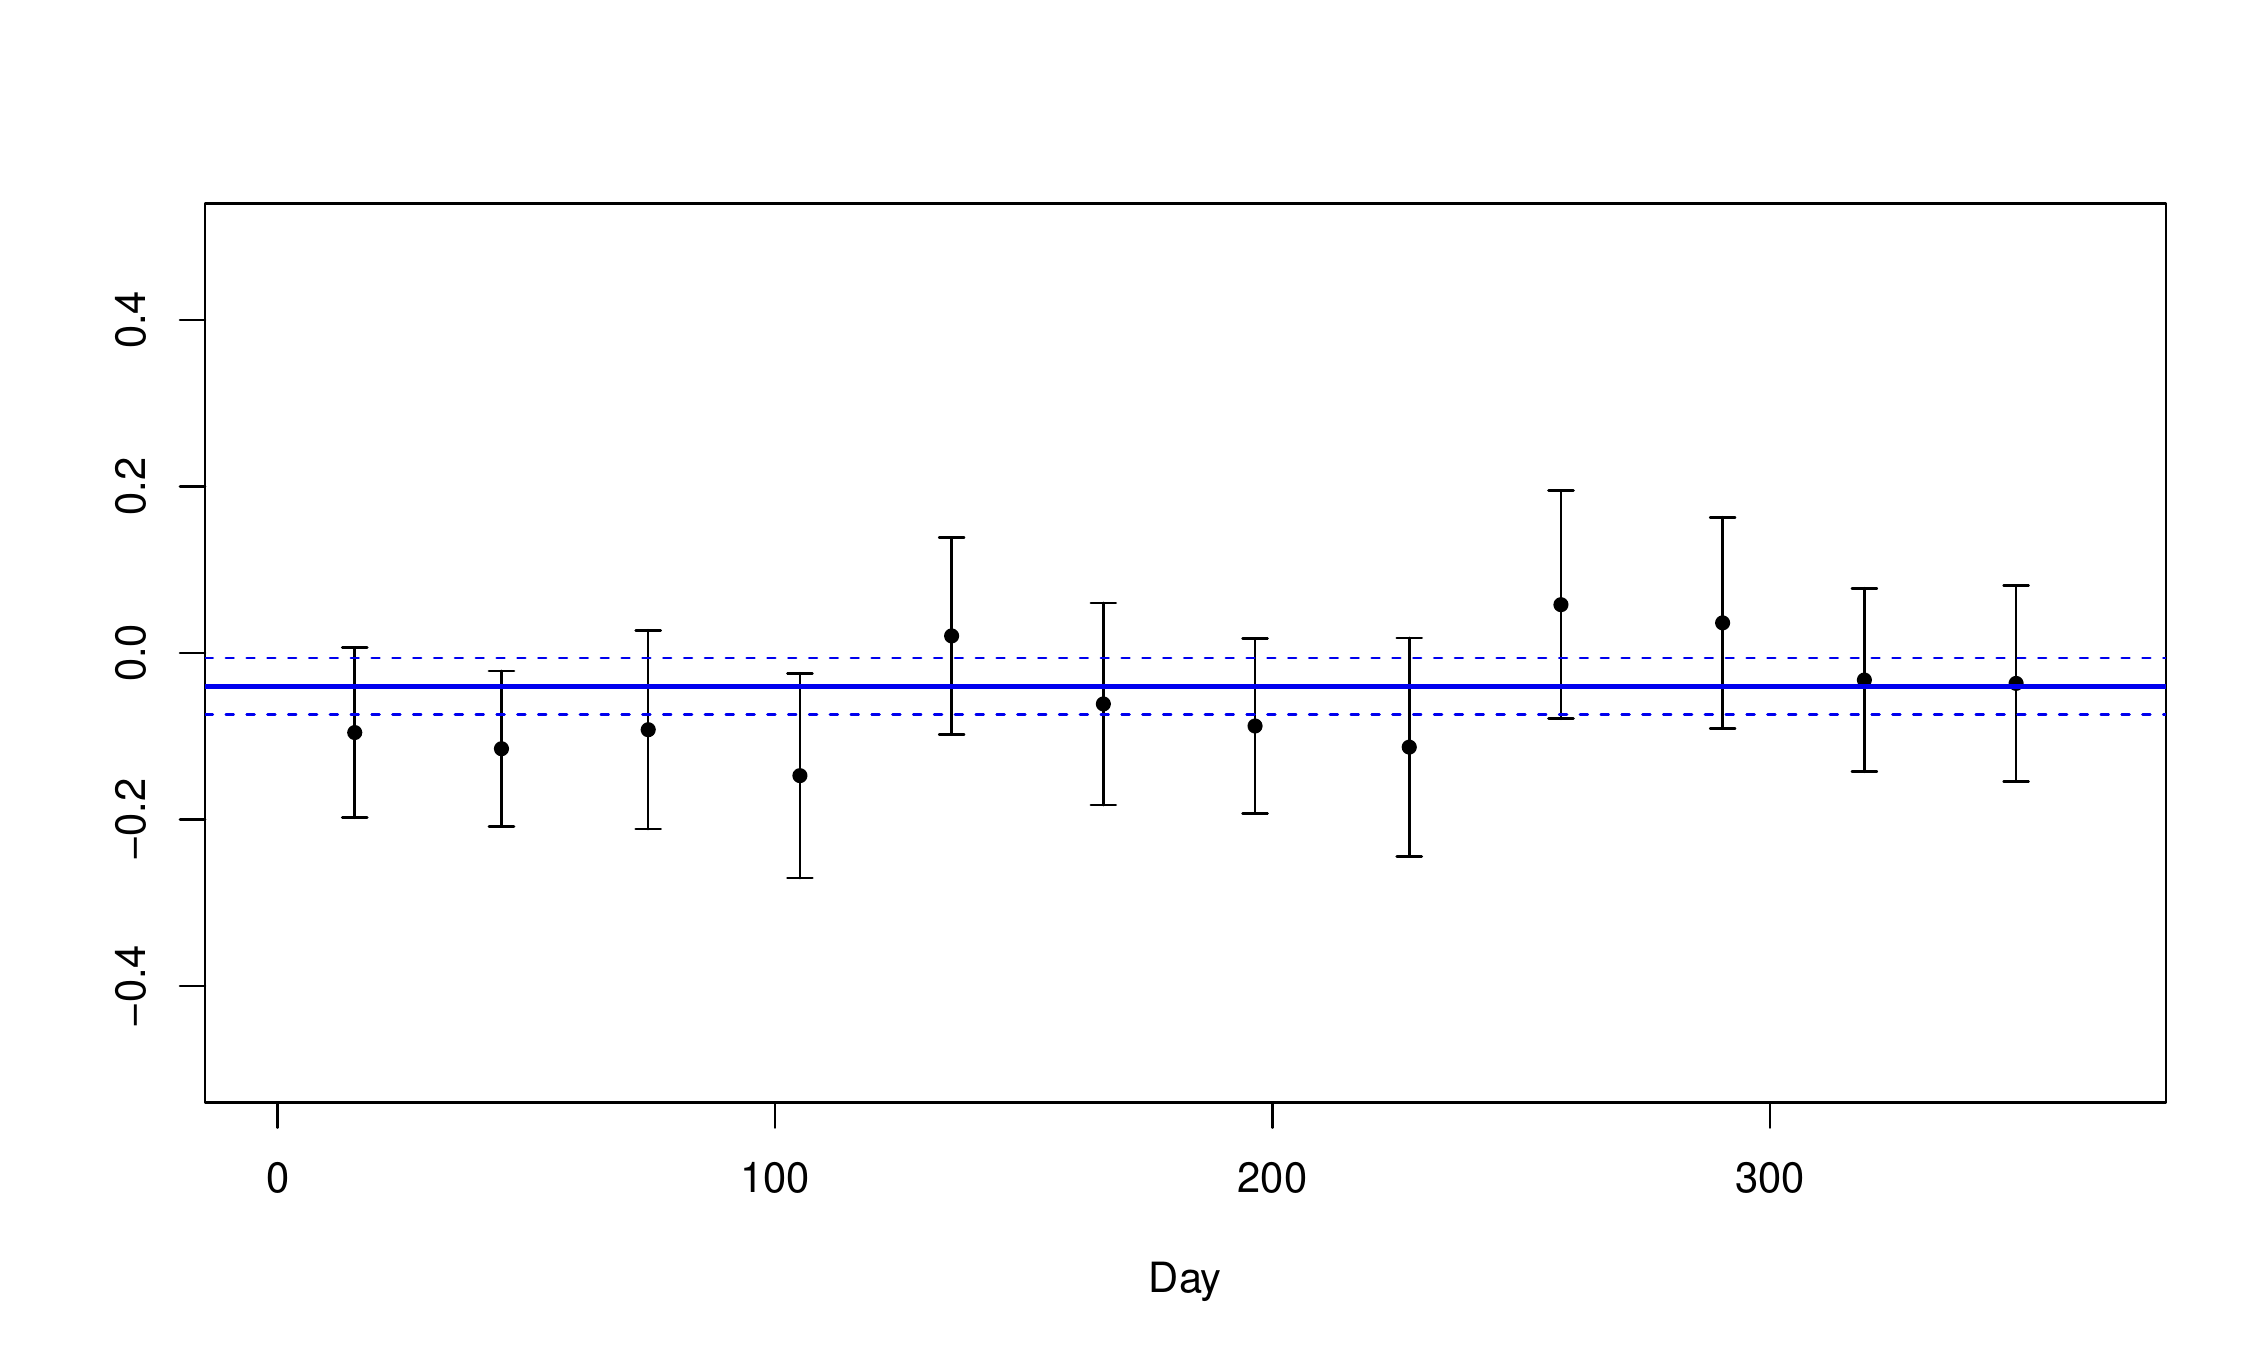}
    \includegraphics[width=0.5\textwidth]{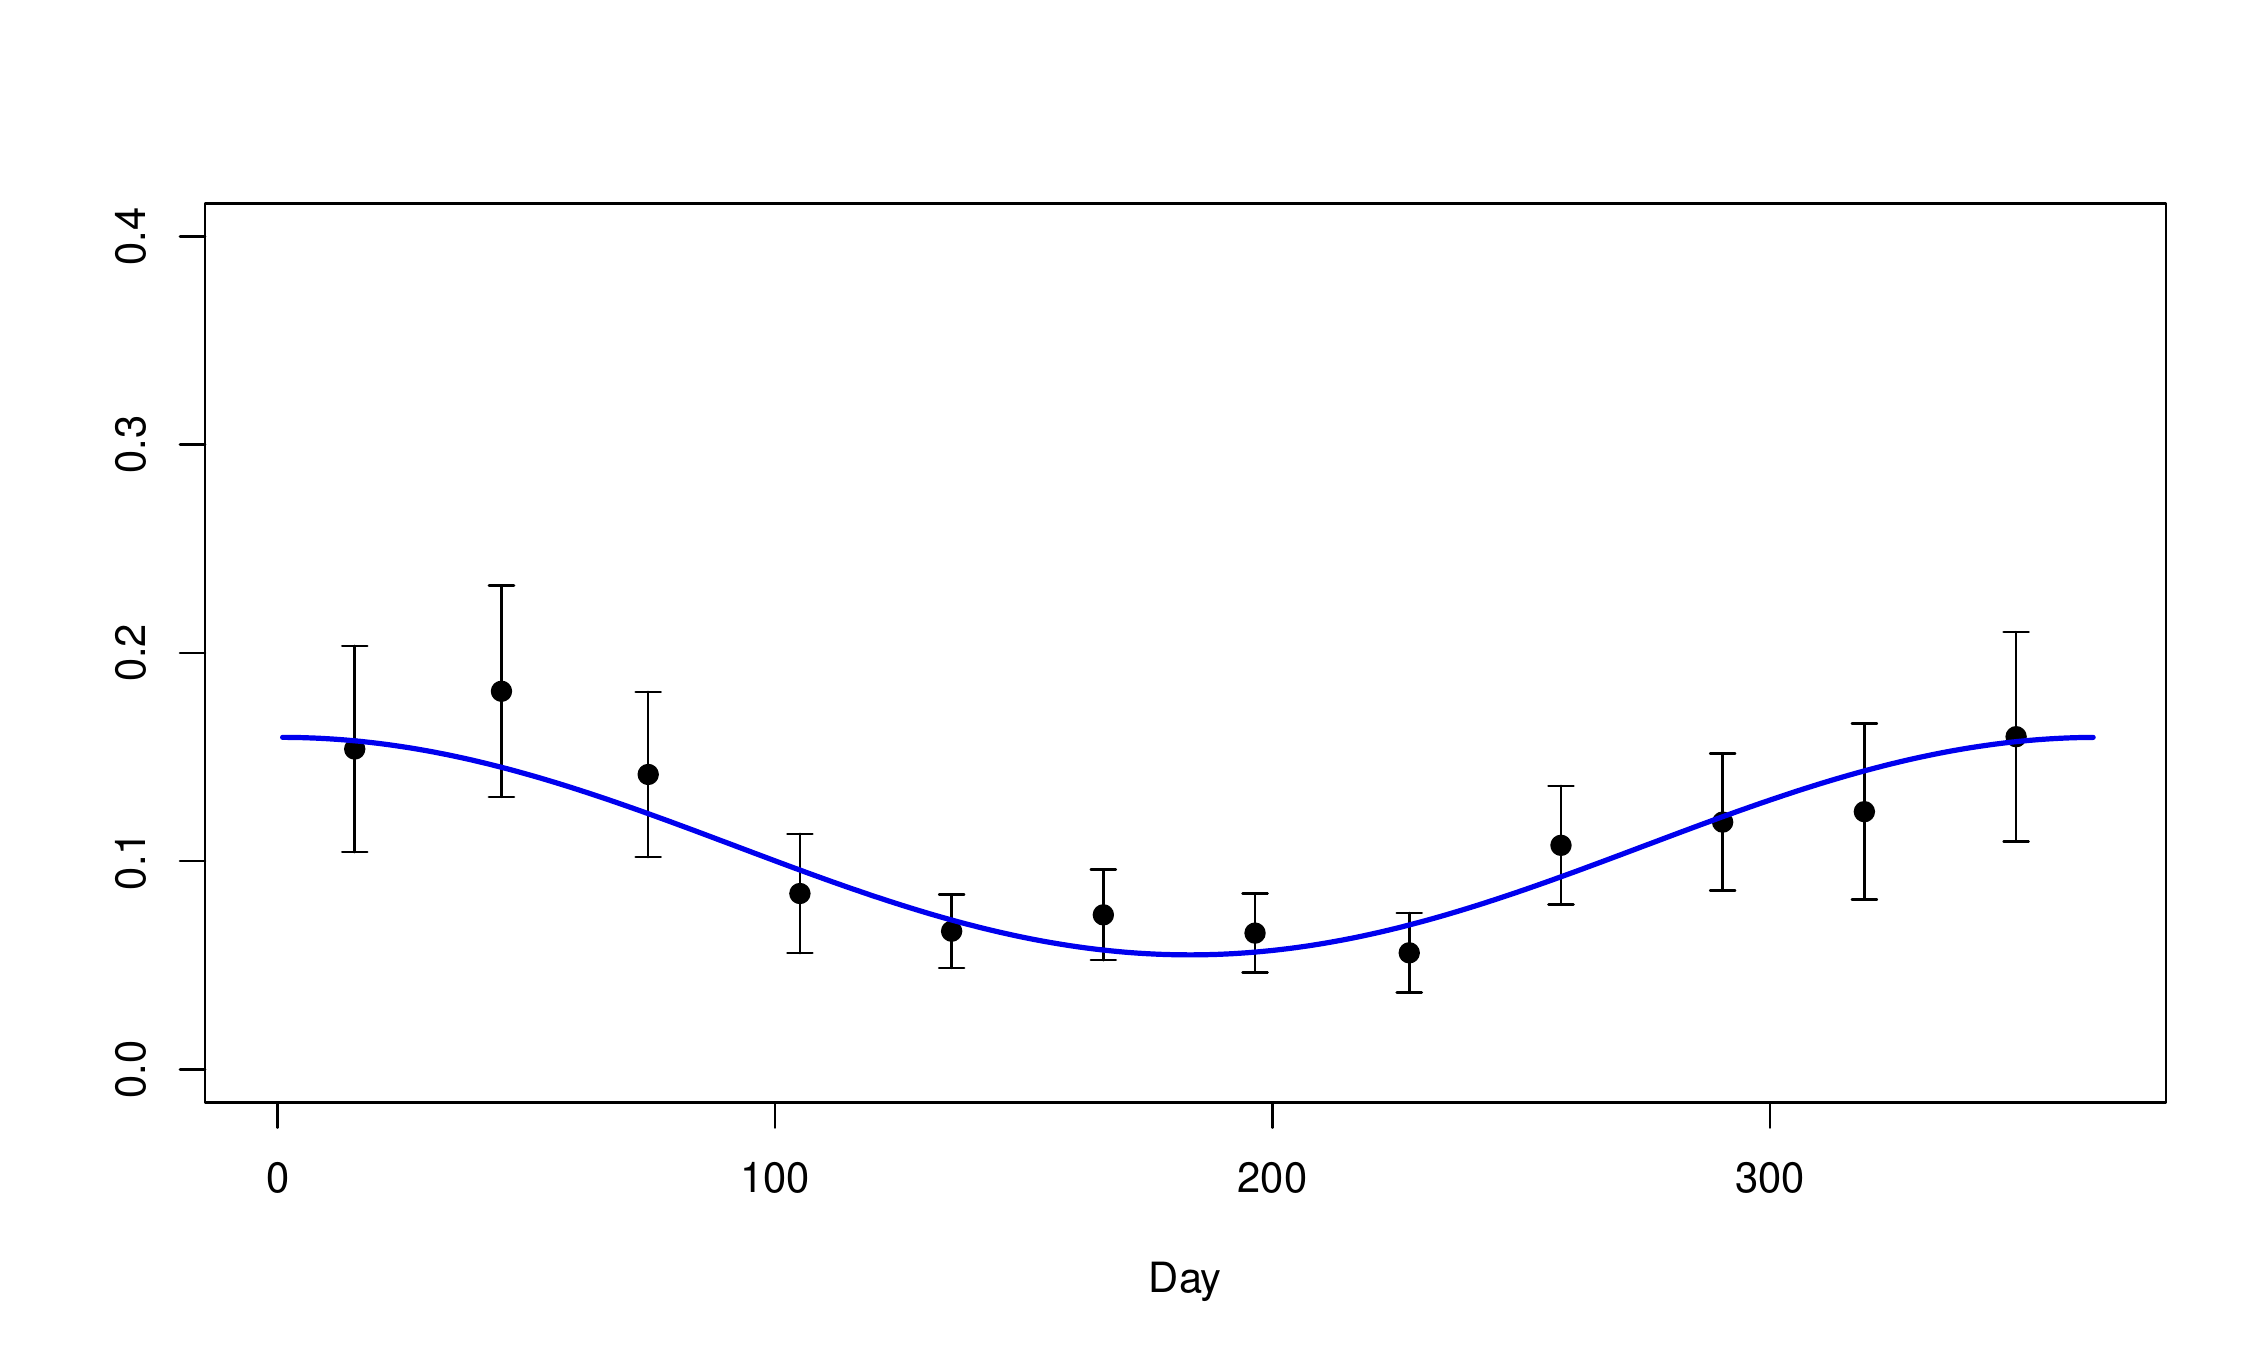}\includegraphics[width=0.5\textwidth]{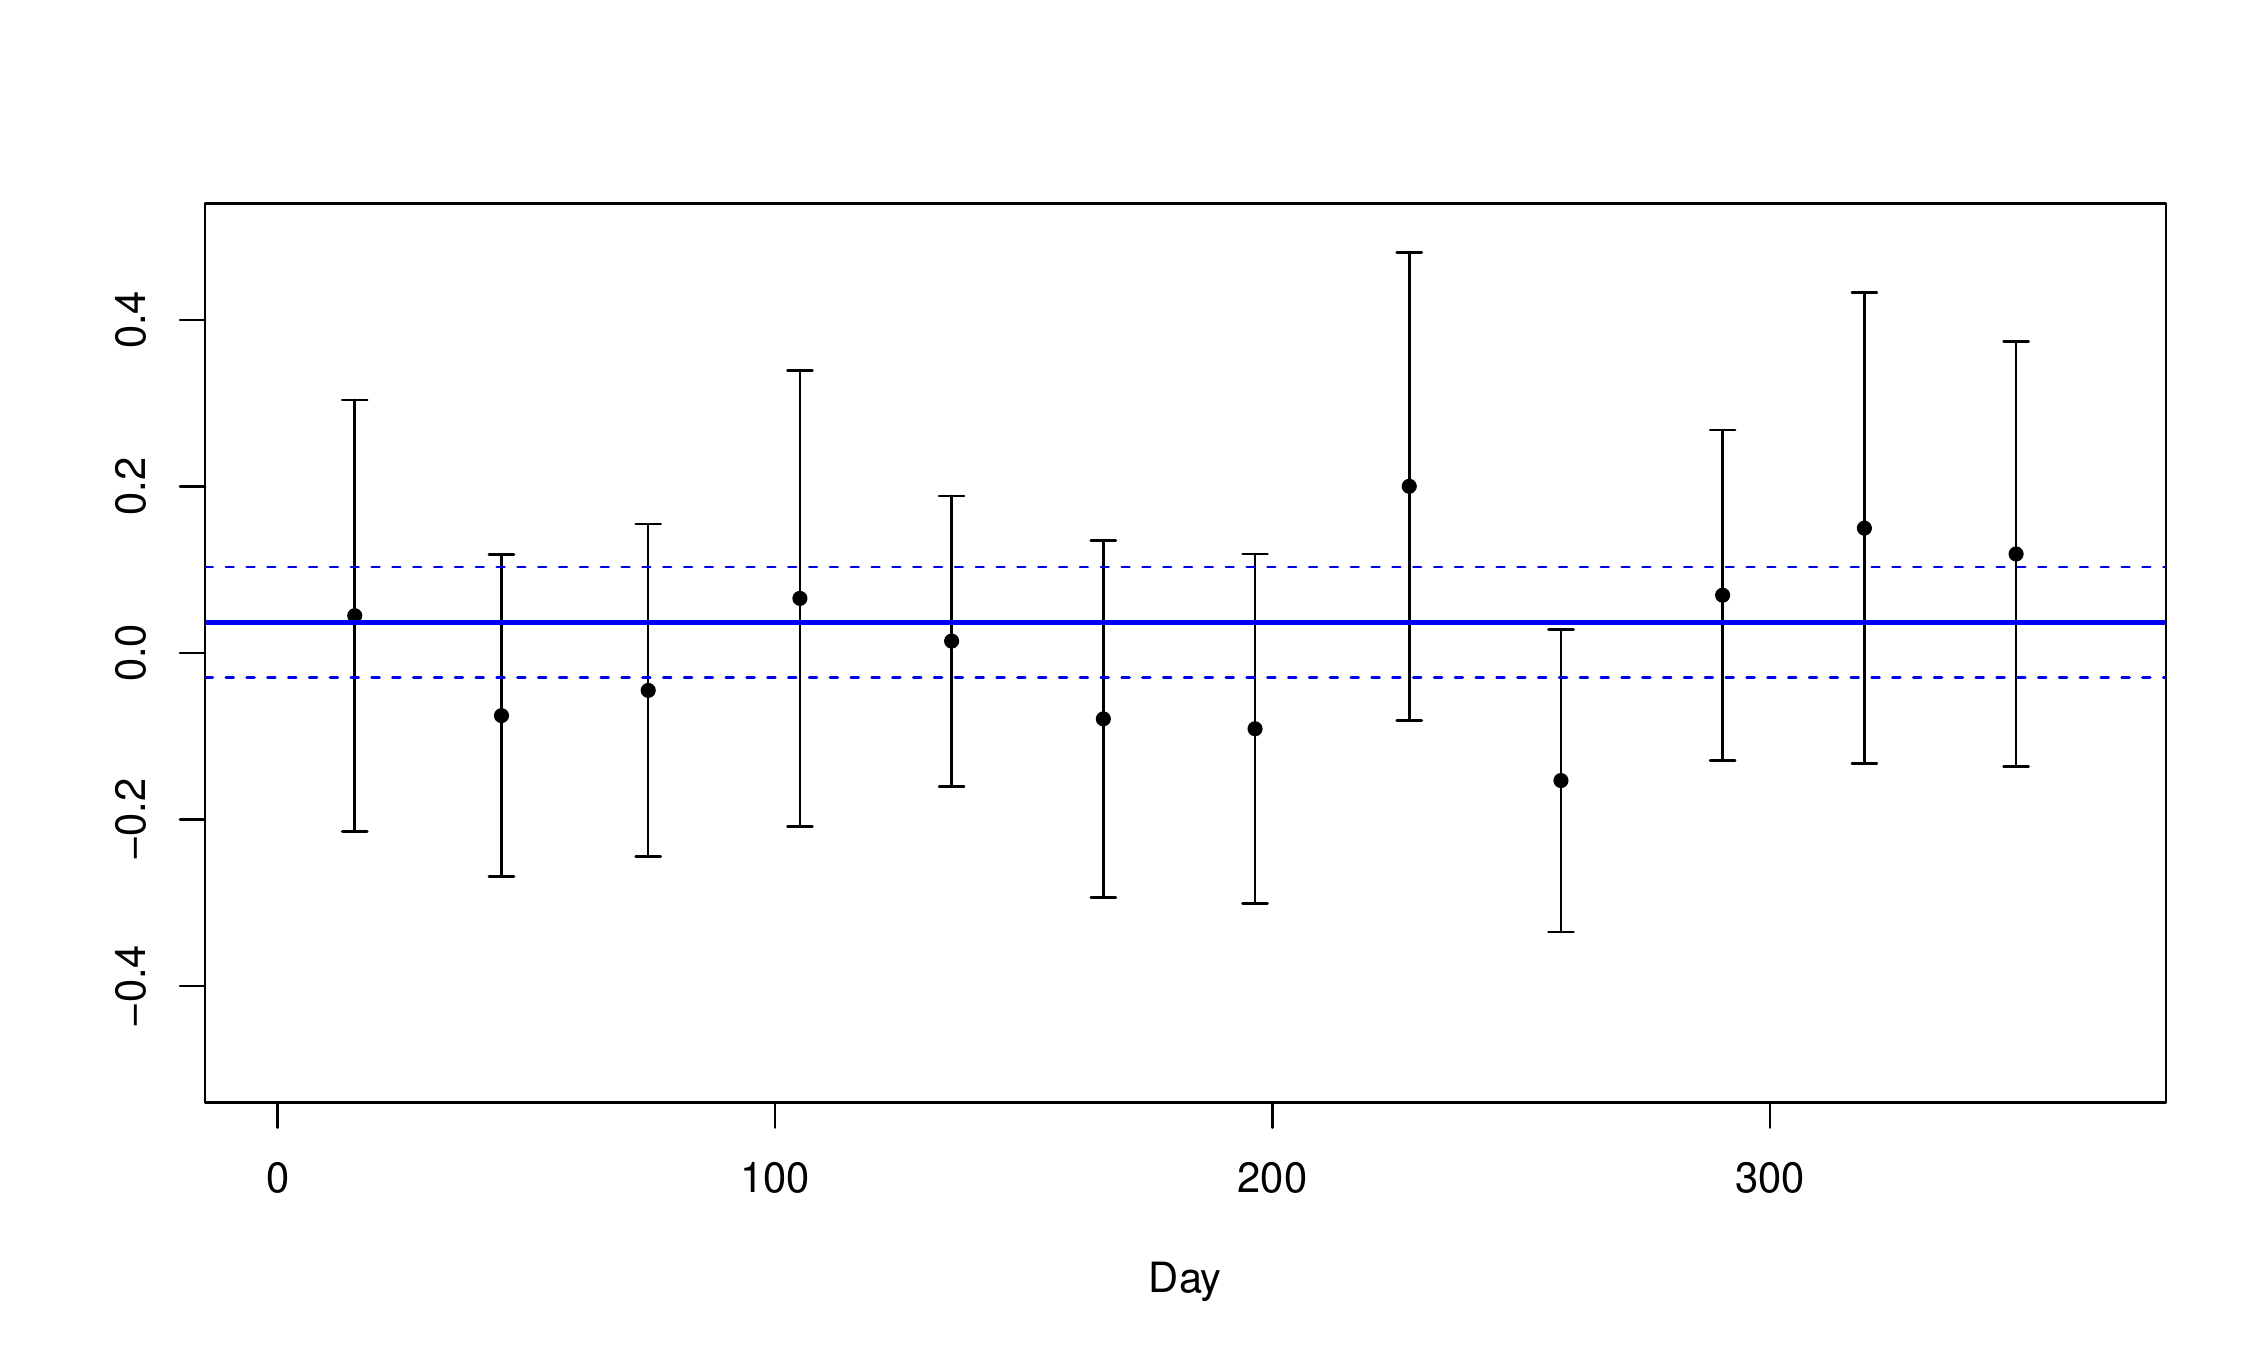}
    \caption{Scale (left) and shape (right) parameter estimates for Model $S2$ (blue) and the monthly model (black) at Lowestoft (top), Newlyn (middle) and Sheerness (bottom).}
    \label{ss_param_ests_fig_all}
\end{figure}

%\subsection{Accounting for Skew Surge Temporal Dependence}
%Figure \ref{fig::acf_ss} shows the autocorrelation function (acf) plot for each site. These aid with choosing a block size for the non-stationary bootstrap procedure in Section \ref{ss_mt_indep} and Section \ref{ss_mt_indep_supp}, and with run length for the runs estimate in Section \ref{ss_dep}. Figure \ref{fig::exi_vartrl} shows estimates of the extremal index using the runs estimate, for various run lengths and threshold at each location. Figures \ref{fig::chi} and \ref{fig::chibar} show plots of the extremal dependence measures $\chi$ and $\bar\chi$ (see Section \ref{sec::suppmat_exi}) for various high quantiles and for each site. %The extremal index is higher for higher thresholds, as expected since exceedances of higher thresholds are less likely to be dependent and cluster. As run length increases, the extremal index decreases 

\begin{figure}[h]
    \centering
    \includegraphics[width=0.45\textwidth]{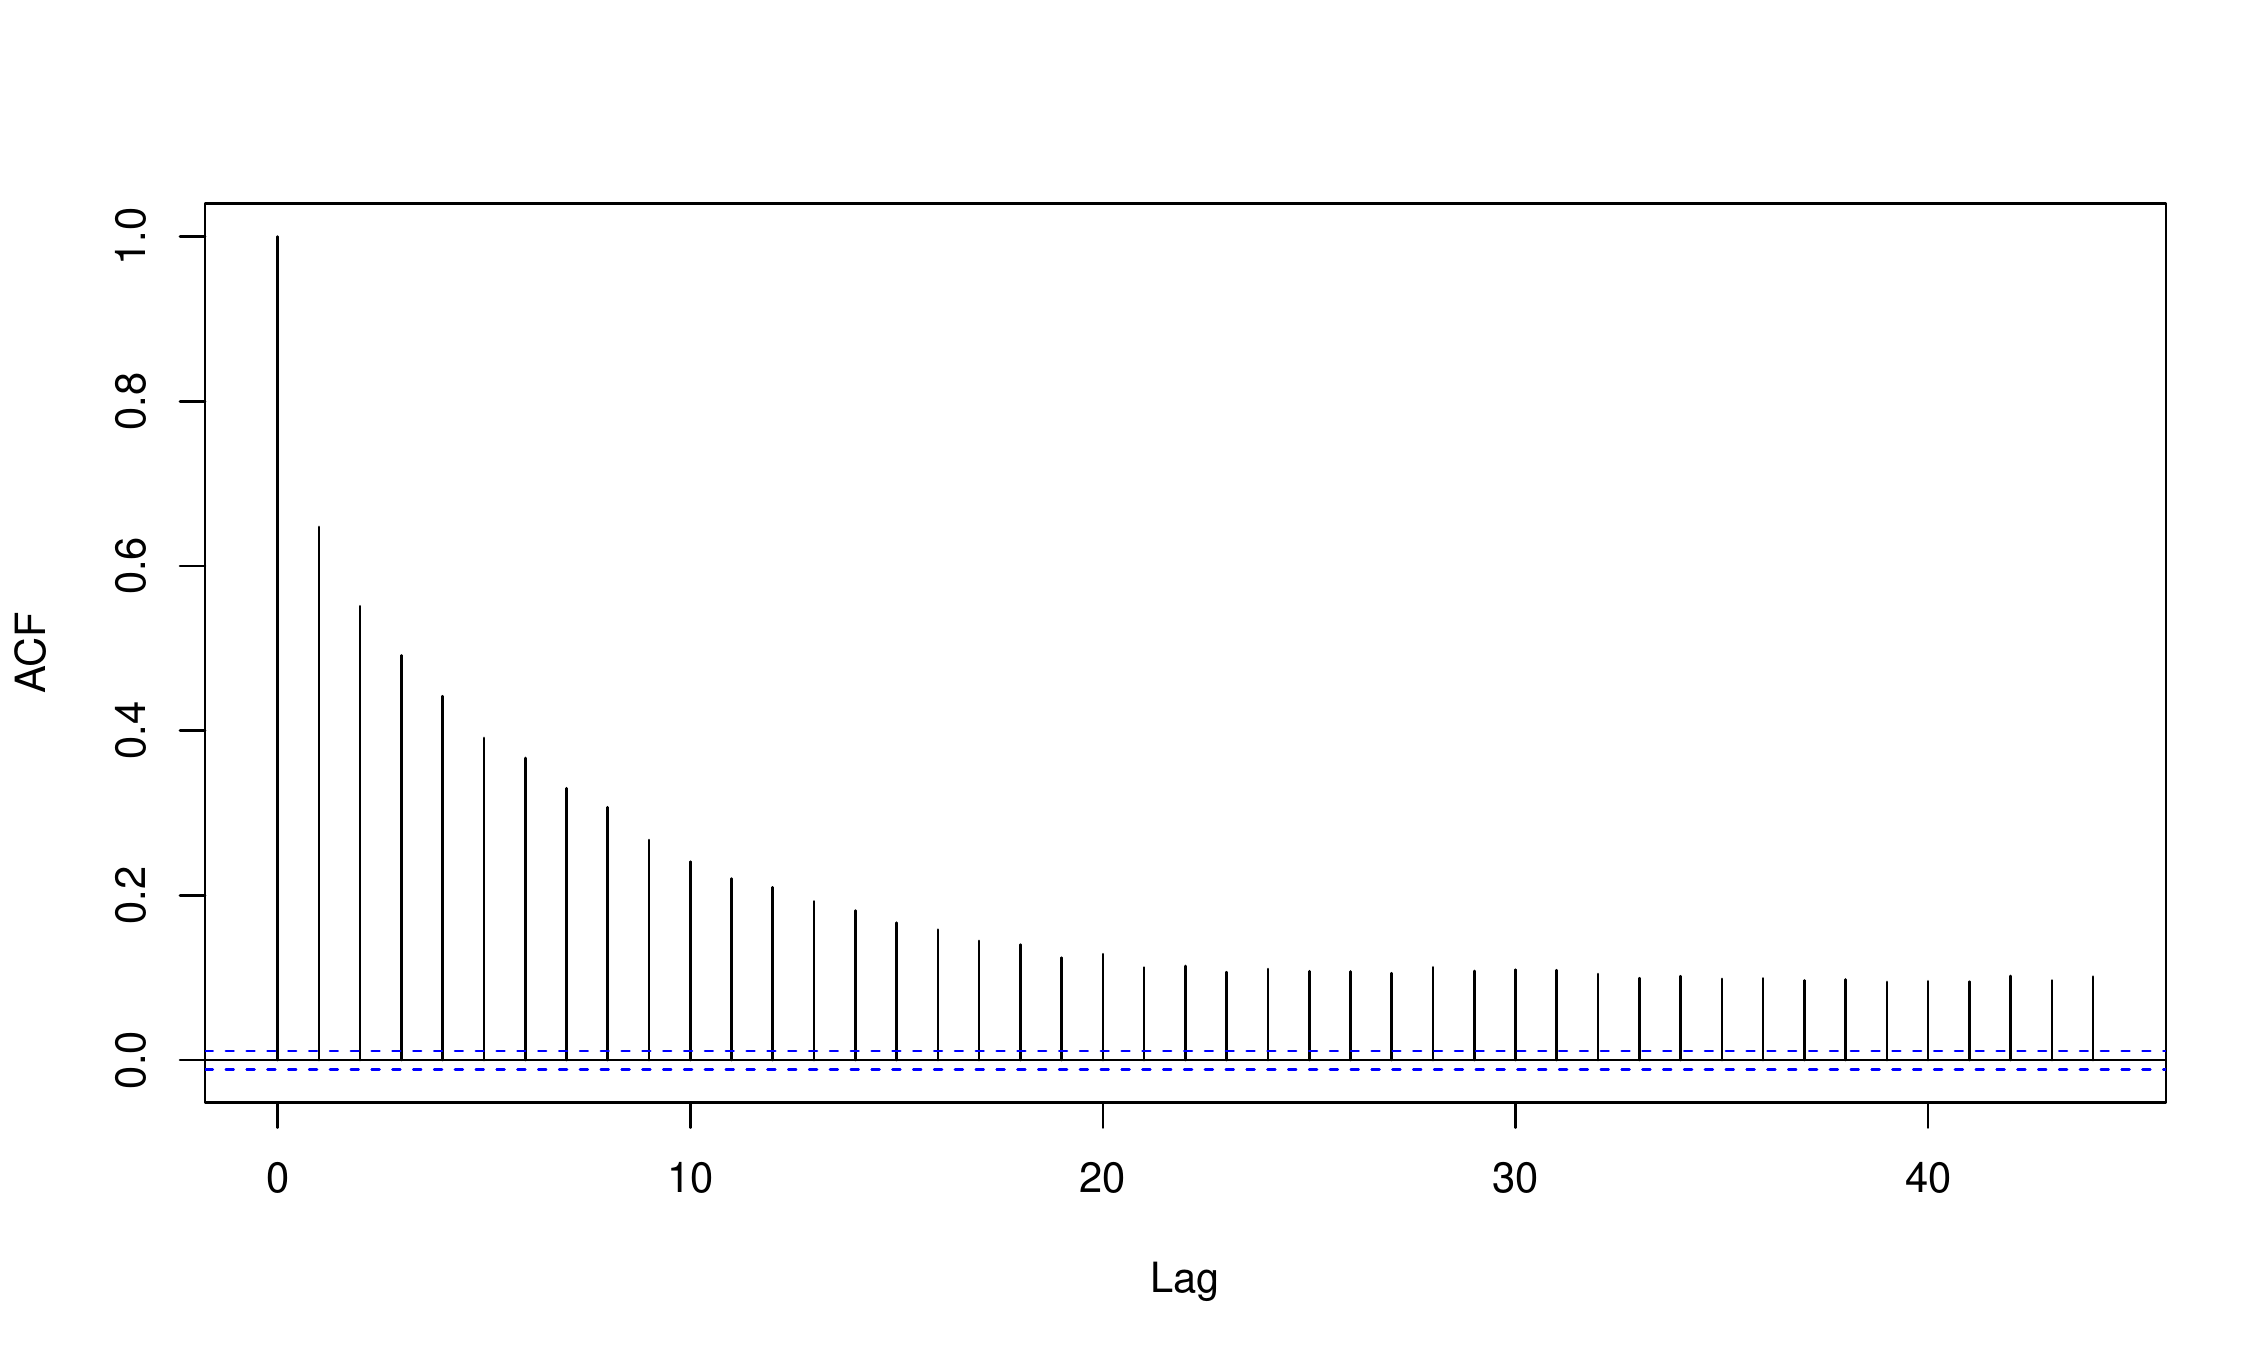}\includegraphics[width=0.45\textwidth]{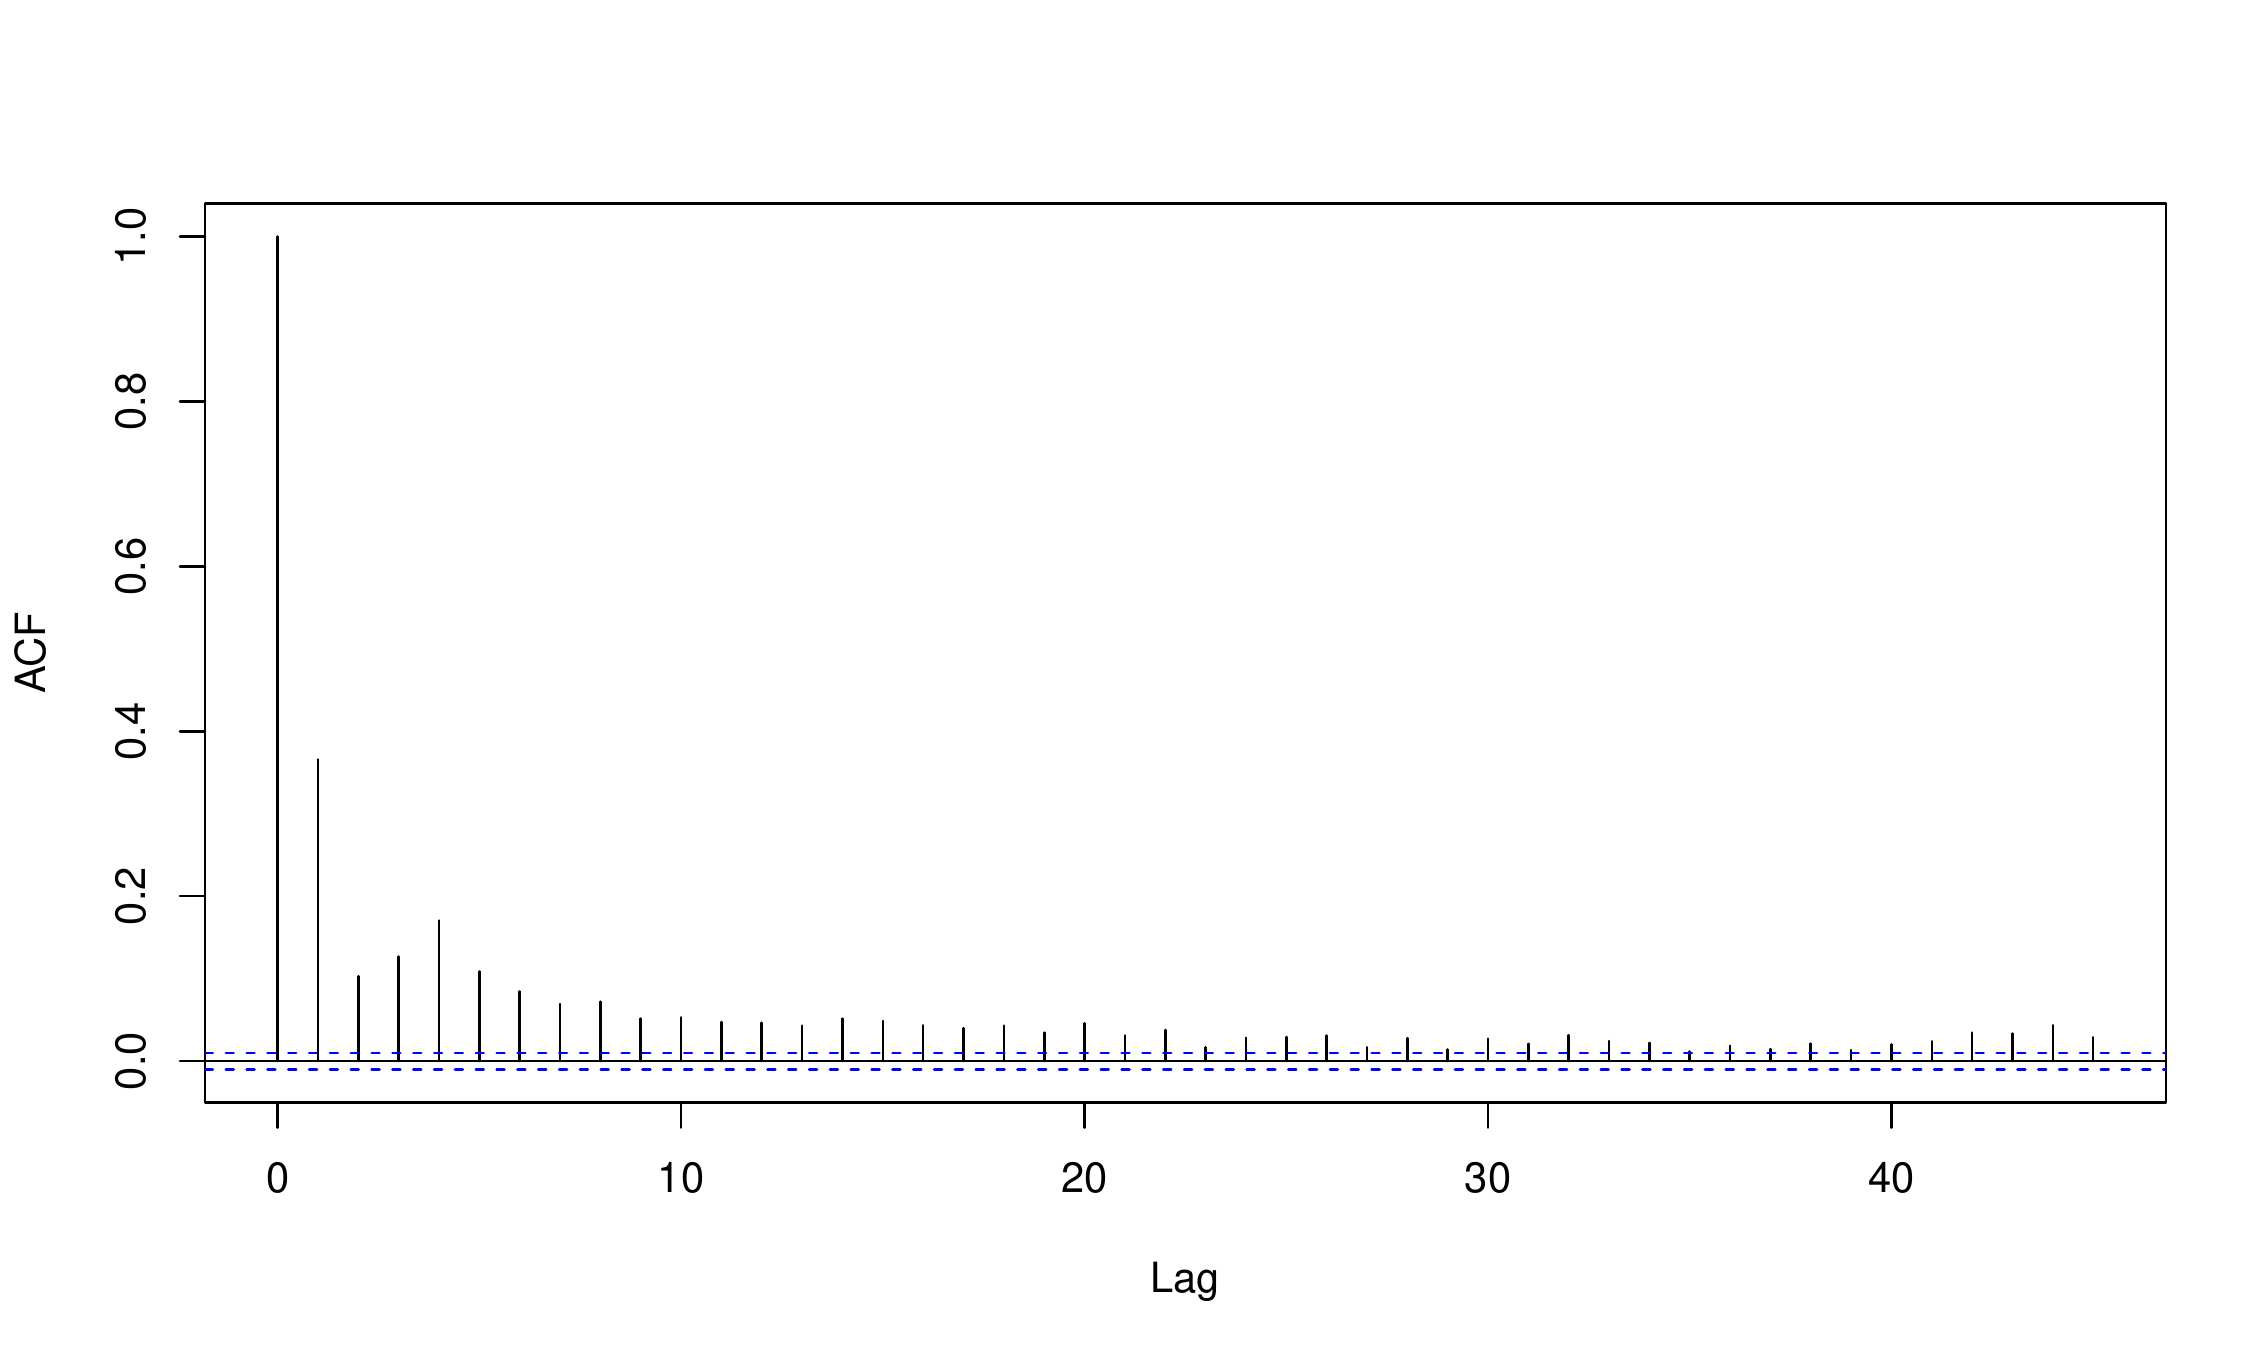} \\
    \includegraphics[width=0.45\textwidth]{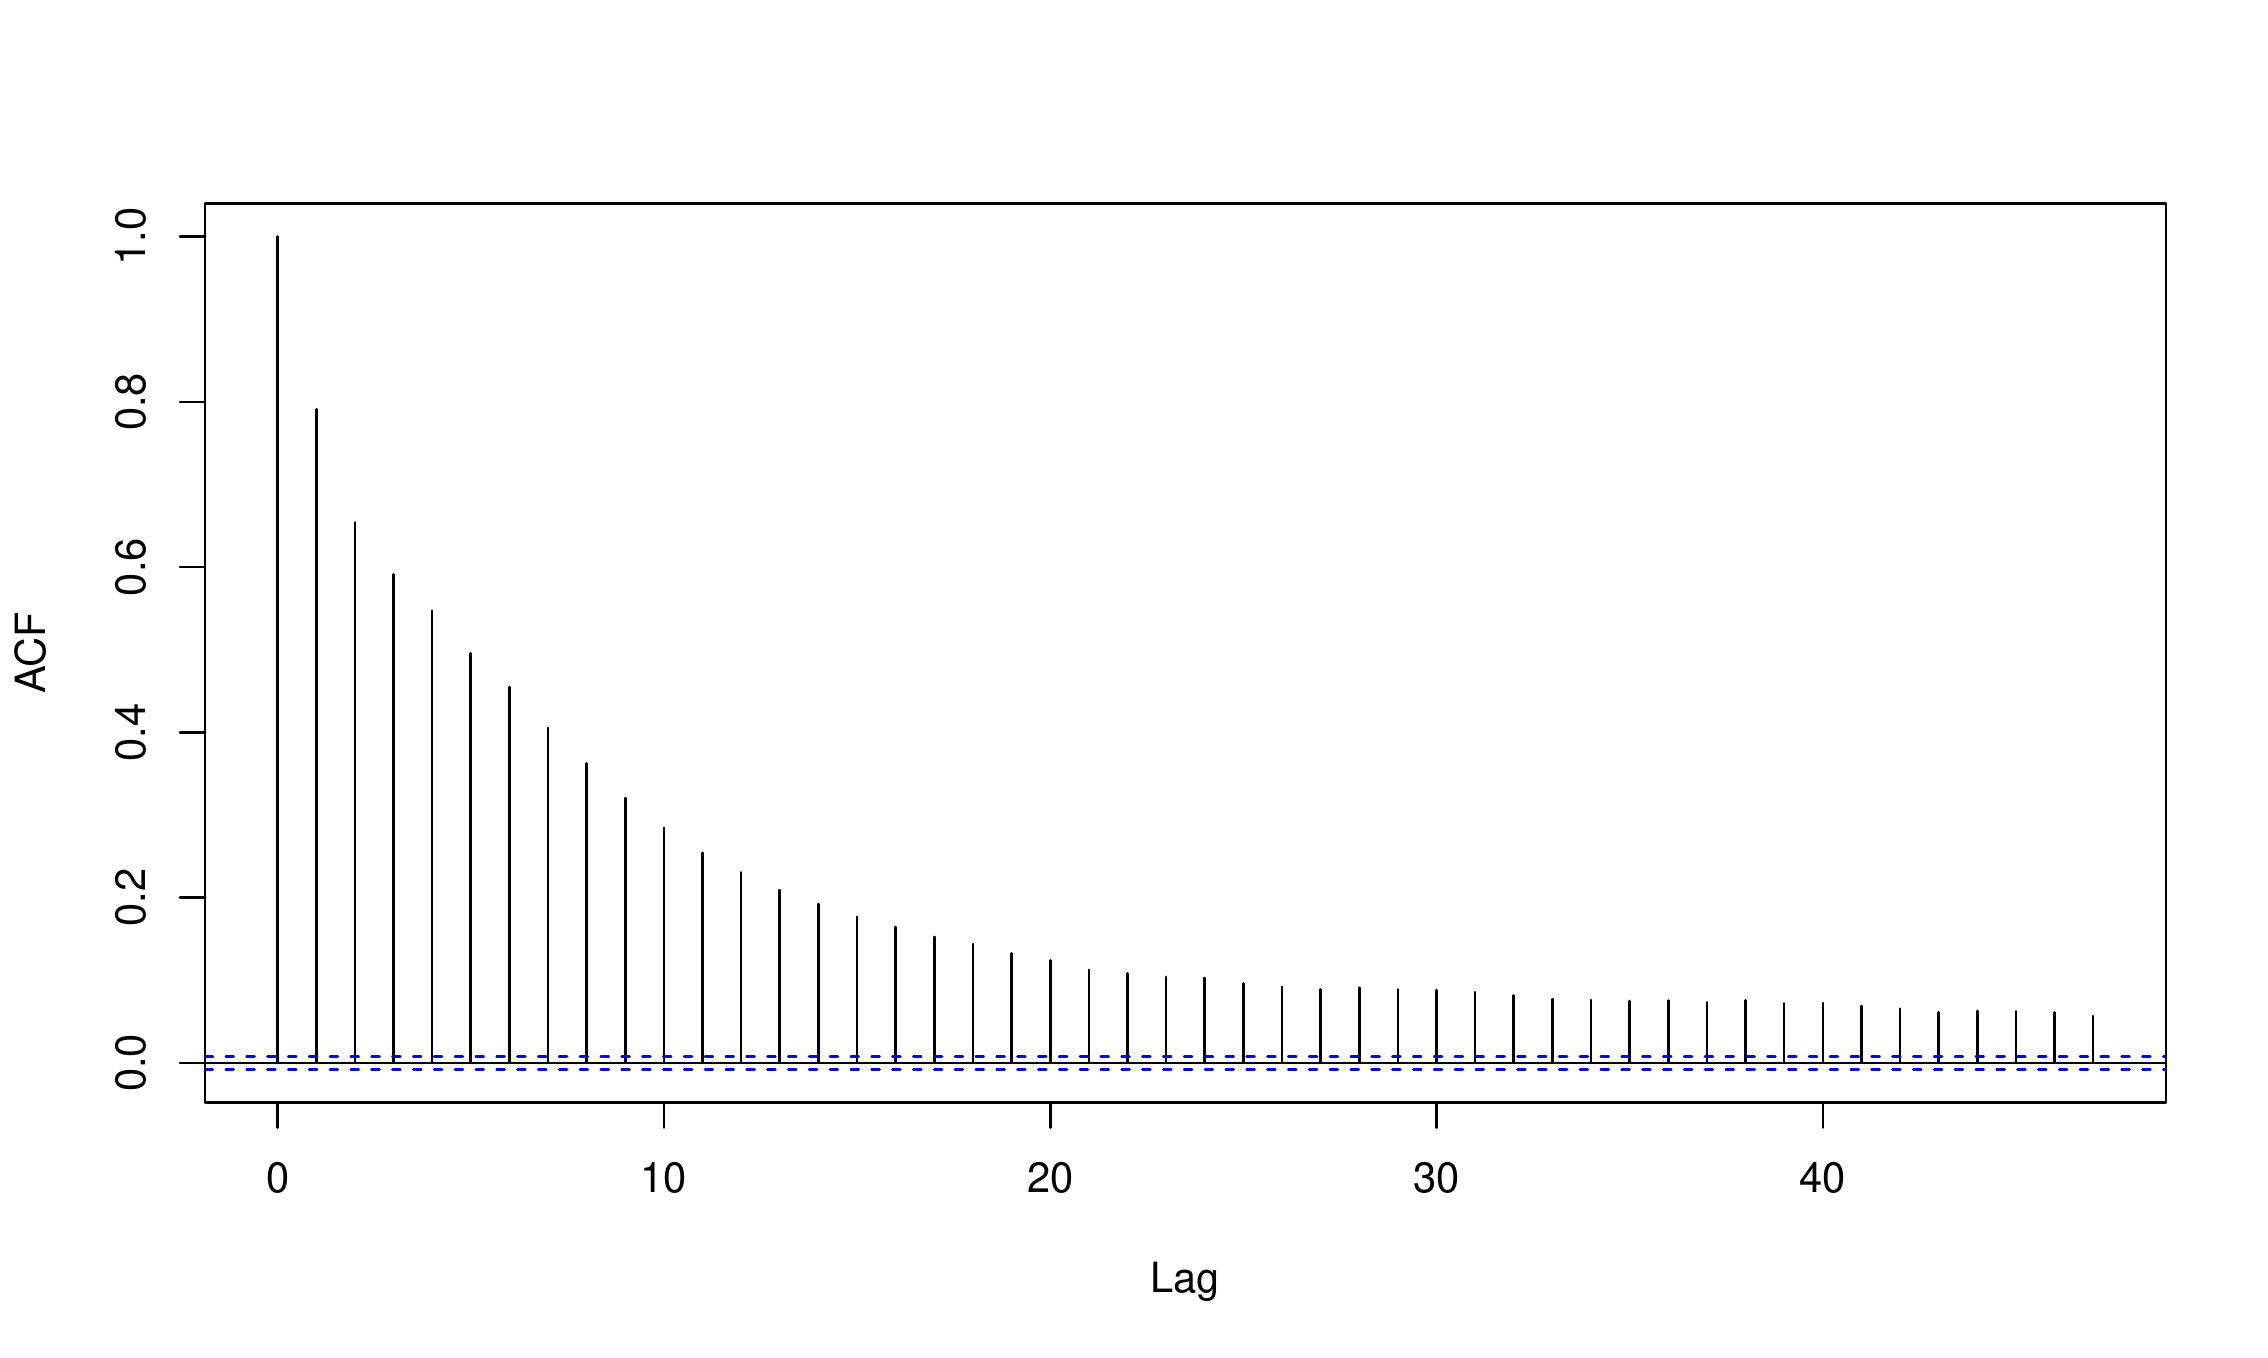}\includegraphics[width=0.45\textwidth]{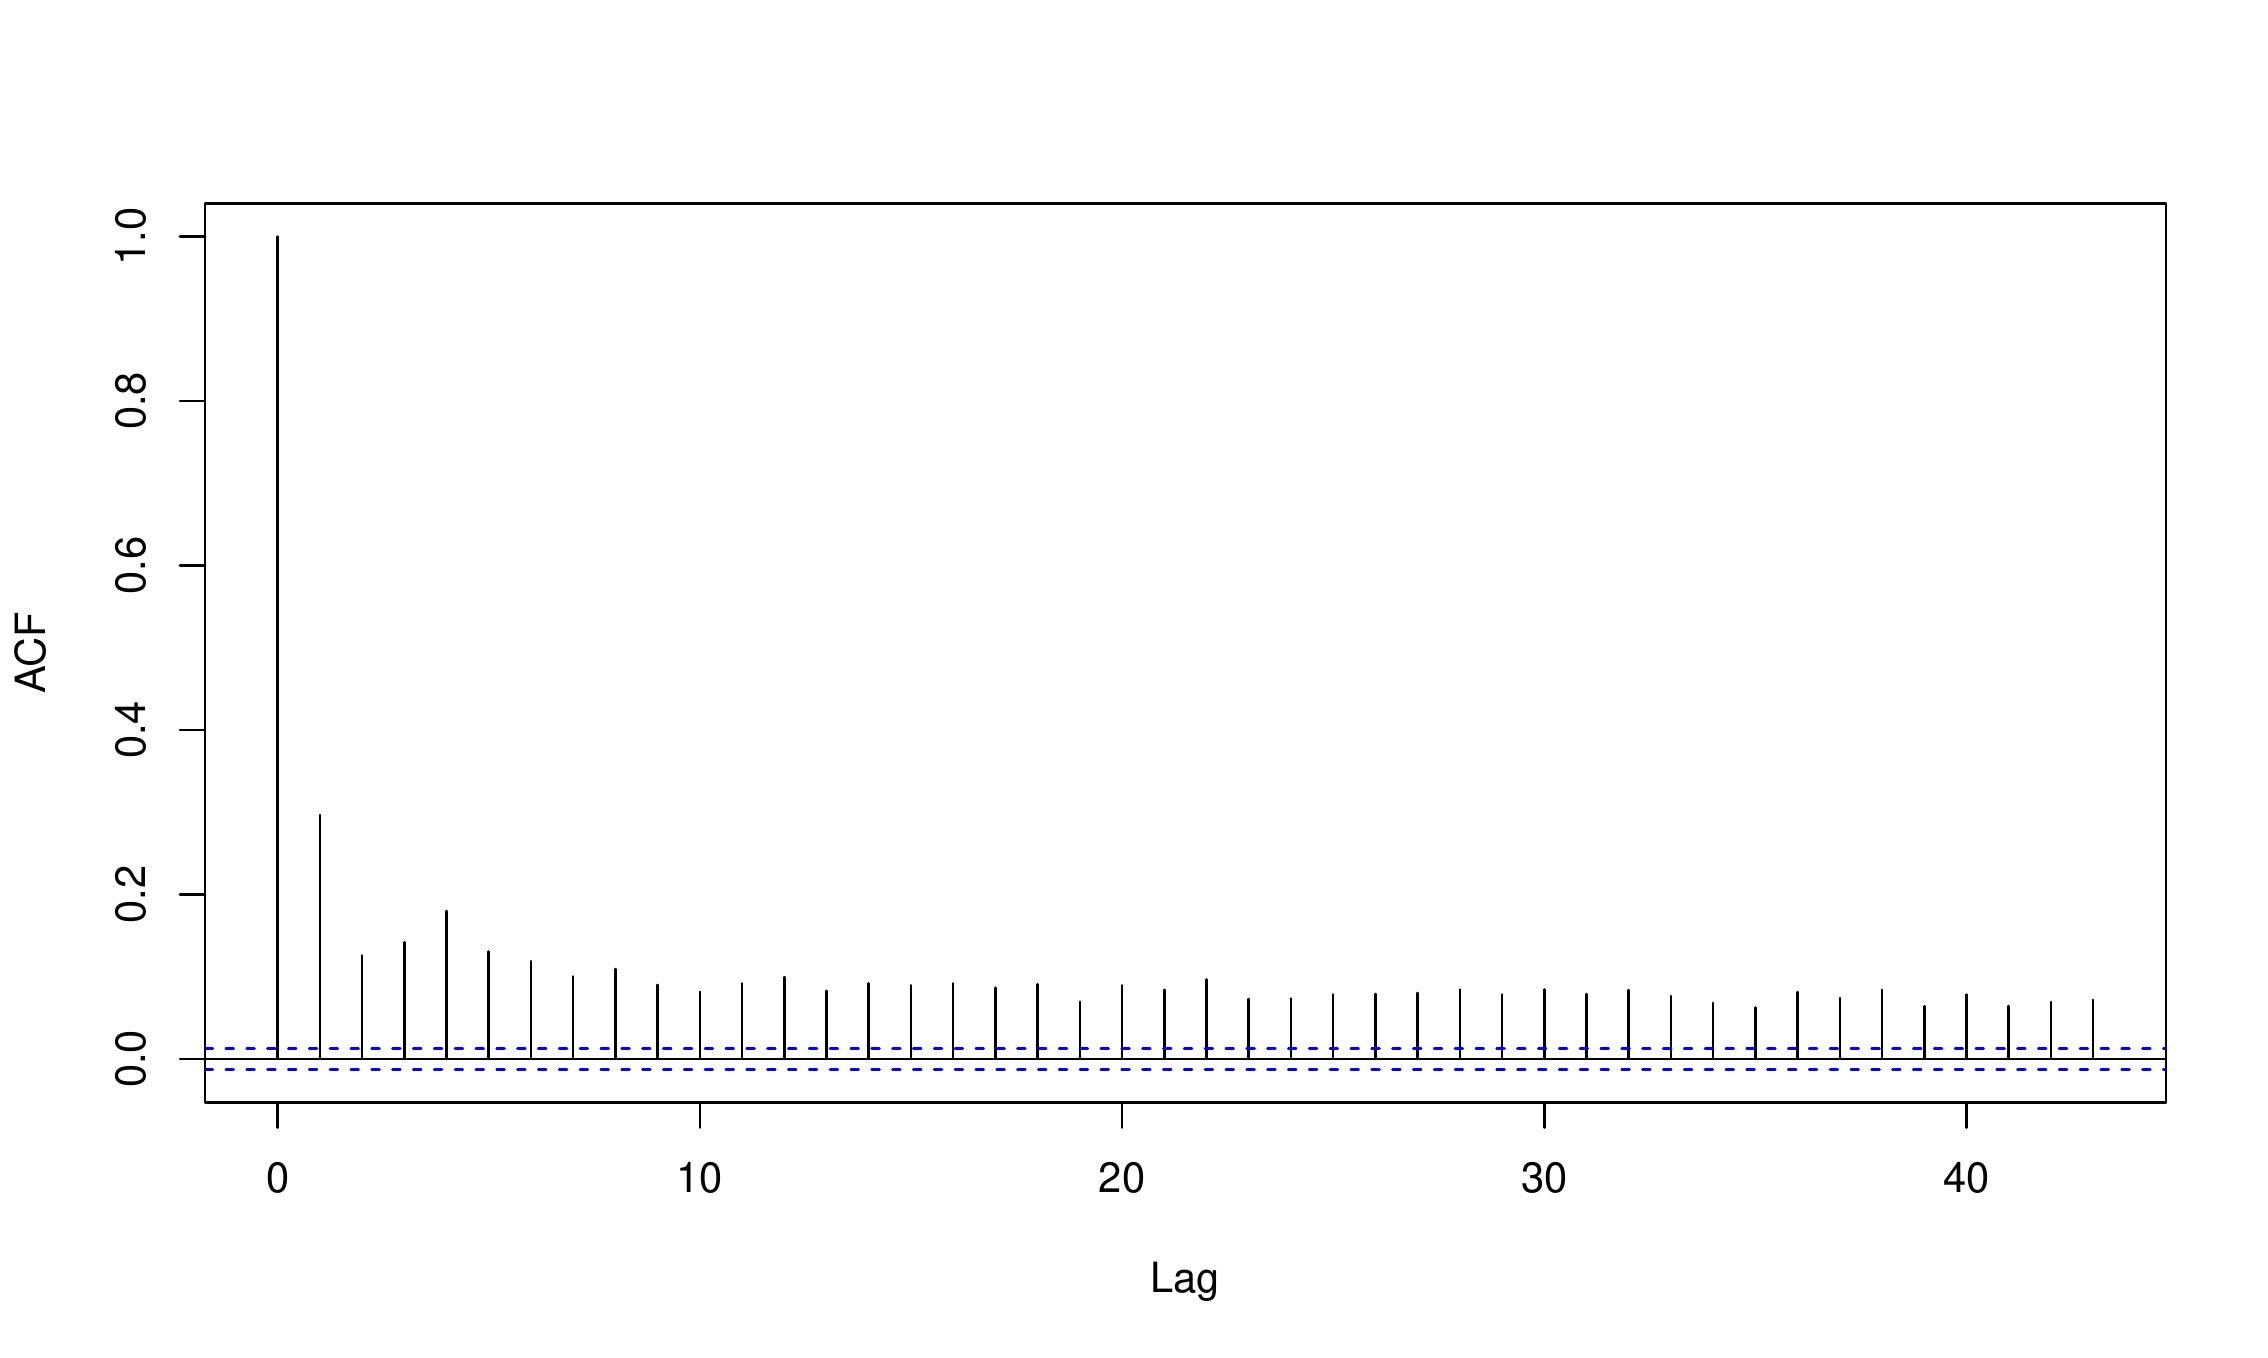}
    \caption{Autocorrelation function plots for Heysham (top right), Lowestoft (top left), Newlyn (bottom right) and Sheerness (bottom left).}
    \label{fig::acf_ss}
\end{figure}

\begin{figure}[h]
    \centering
    \includegraphics[width=0.45\textwidth]{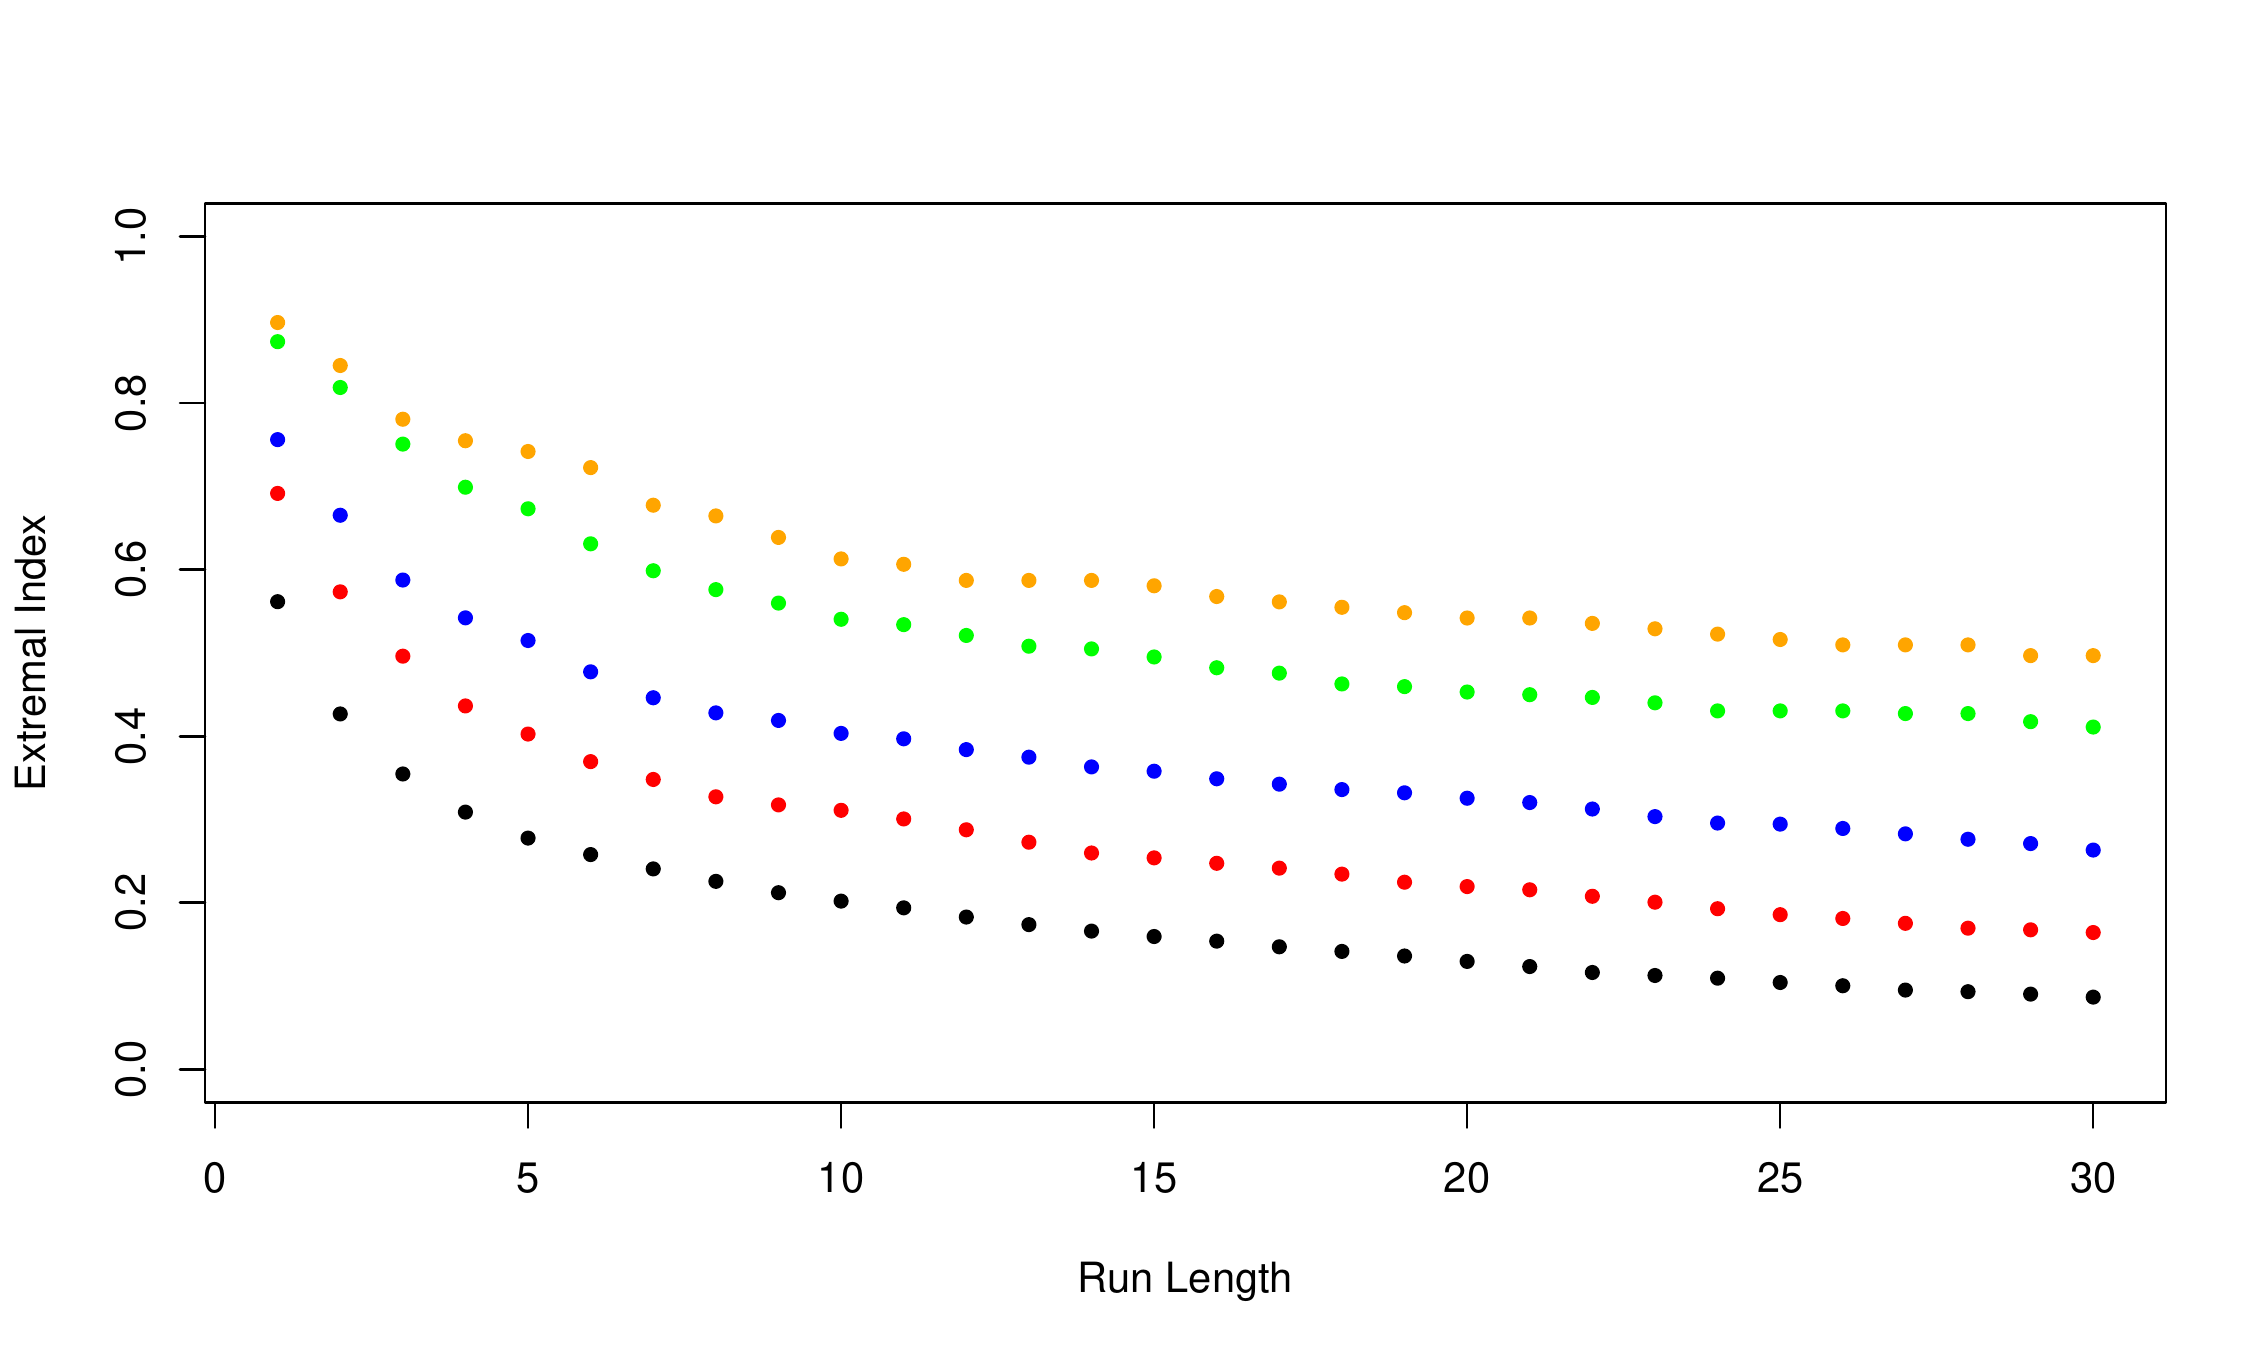}    \includegraphics[width=0.45\textwidth]{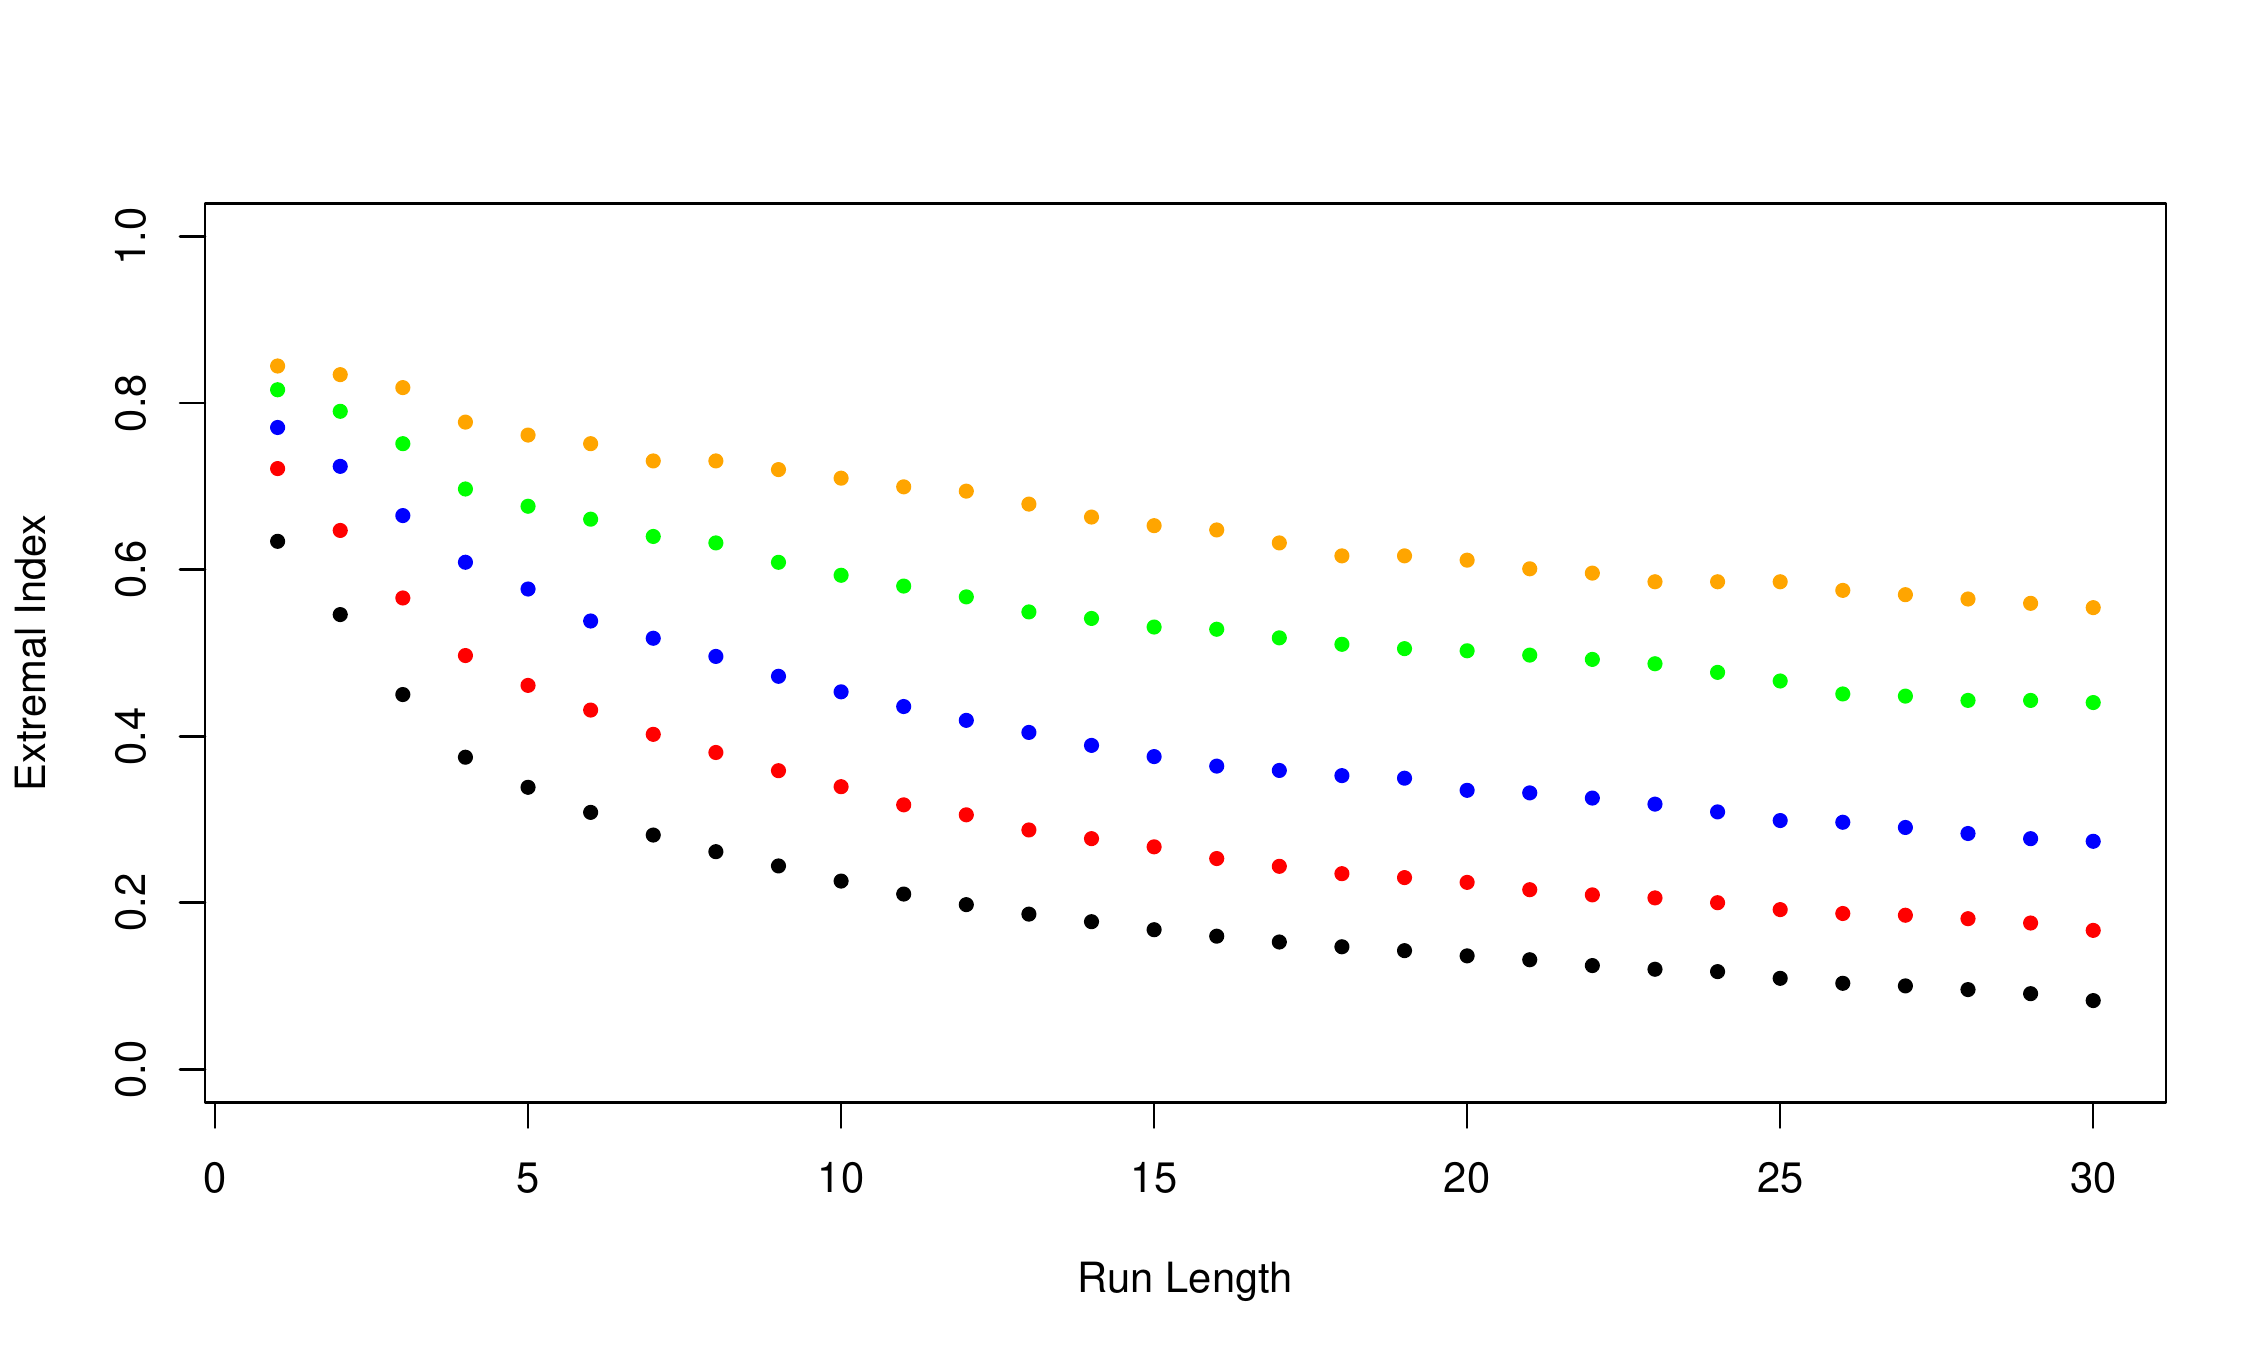}\\
    \includegraphics[width=0.45\textwidth]{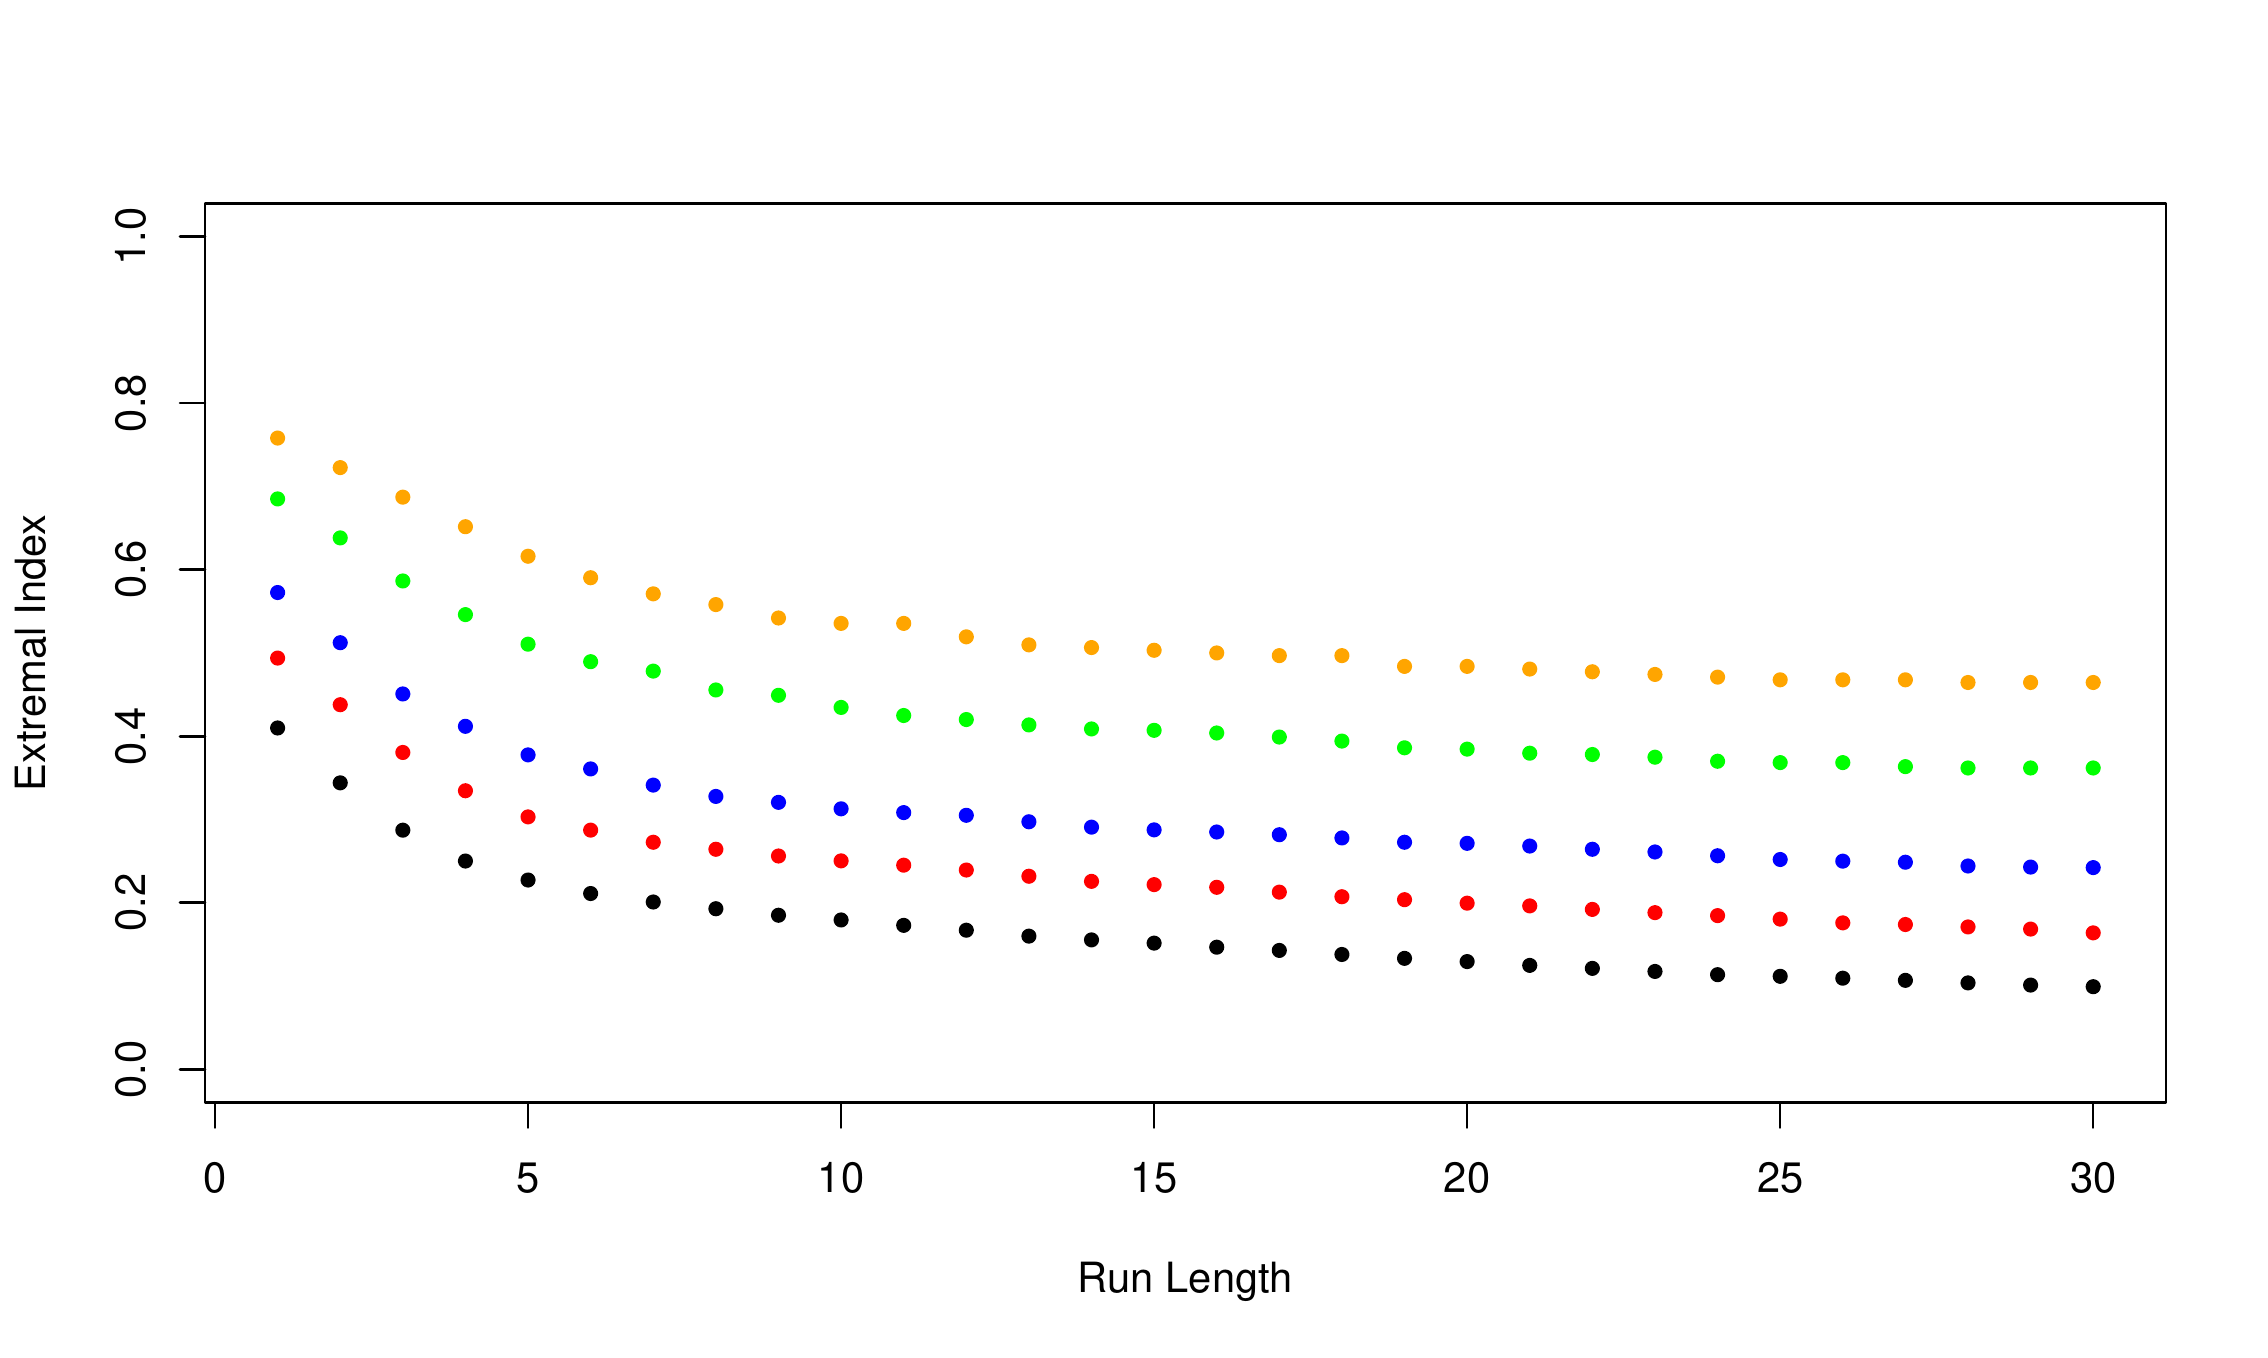}
    \includegraphics[width=0.45\textwidth]{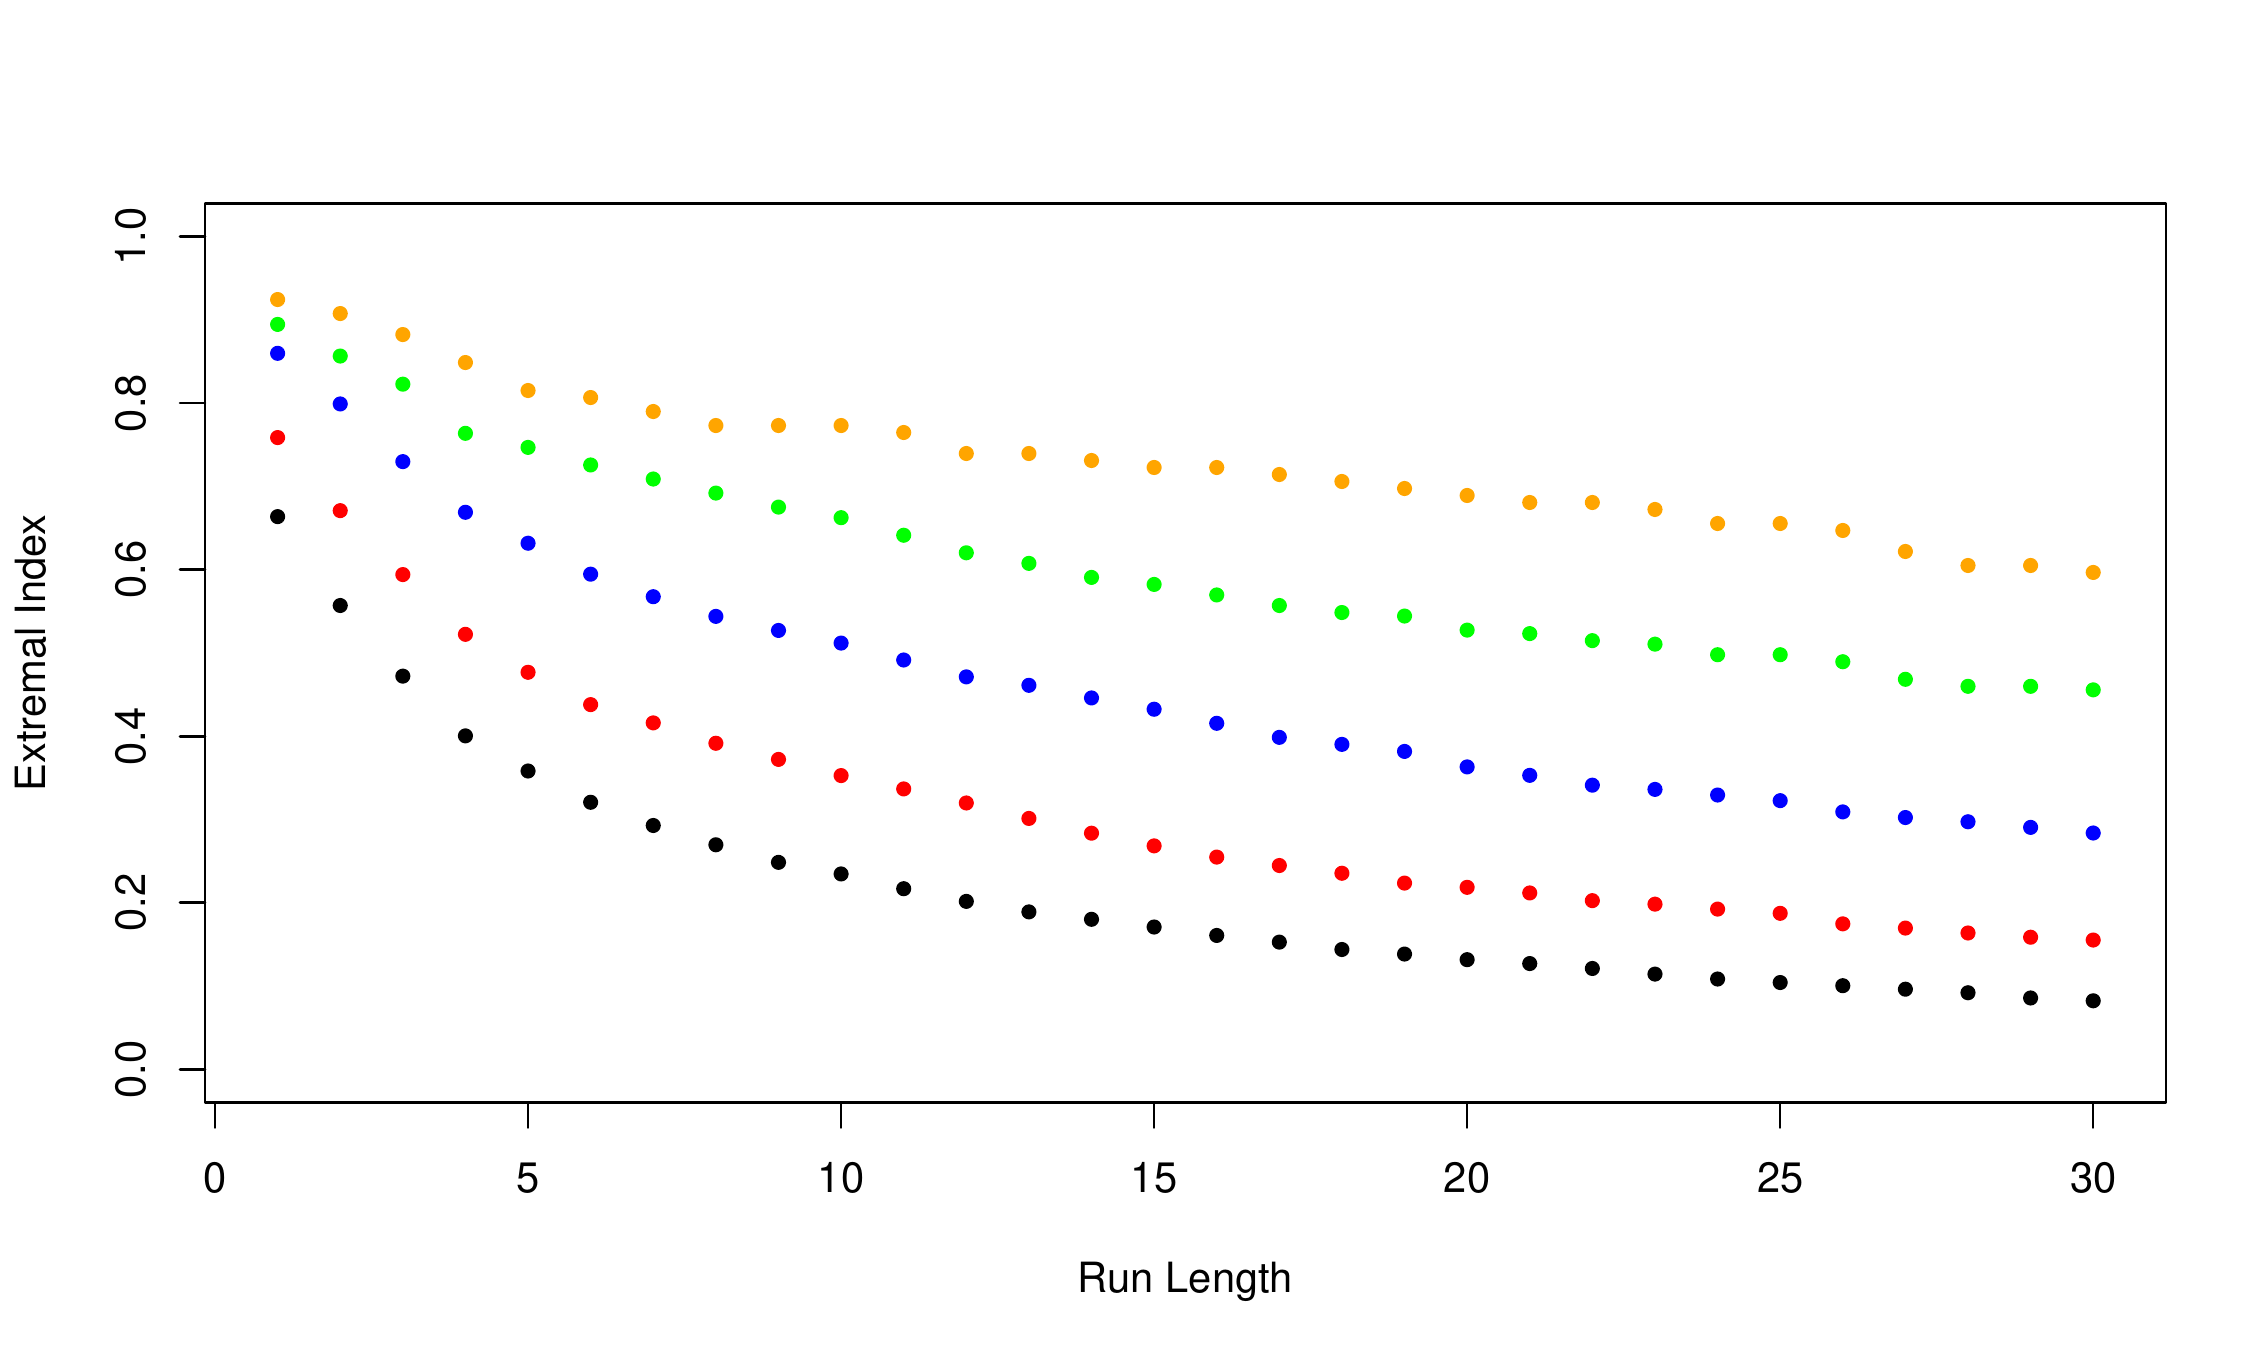}
    \caption{Runs estimate of the extremal index for skew surge, at various quantiles and run lengths. The quantiles are 0.9 (black), 0.95 (red), 0.975 (blue), 0.99 (green) and 0.999 (orange).}
    \label{fig::exi_vartrl}
\end{figure}

\begin{figure}
    \centering
    \includegraphics[width=0.85\textwidth,height=5cm]{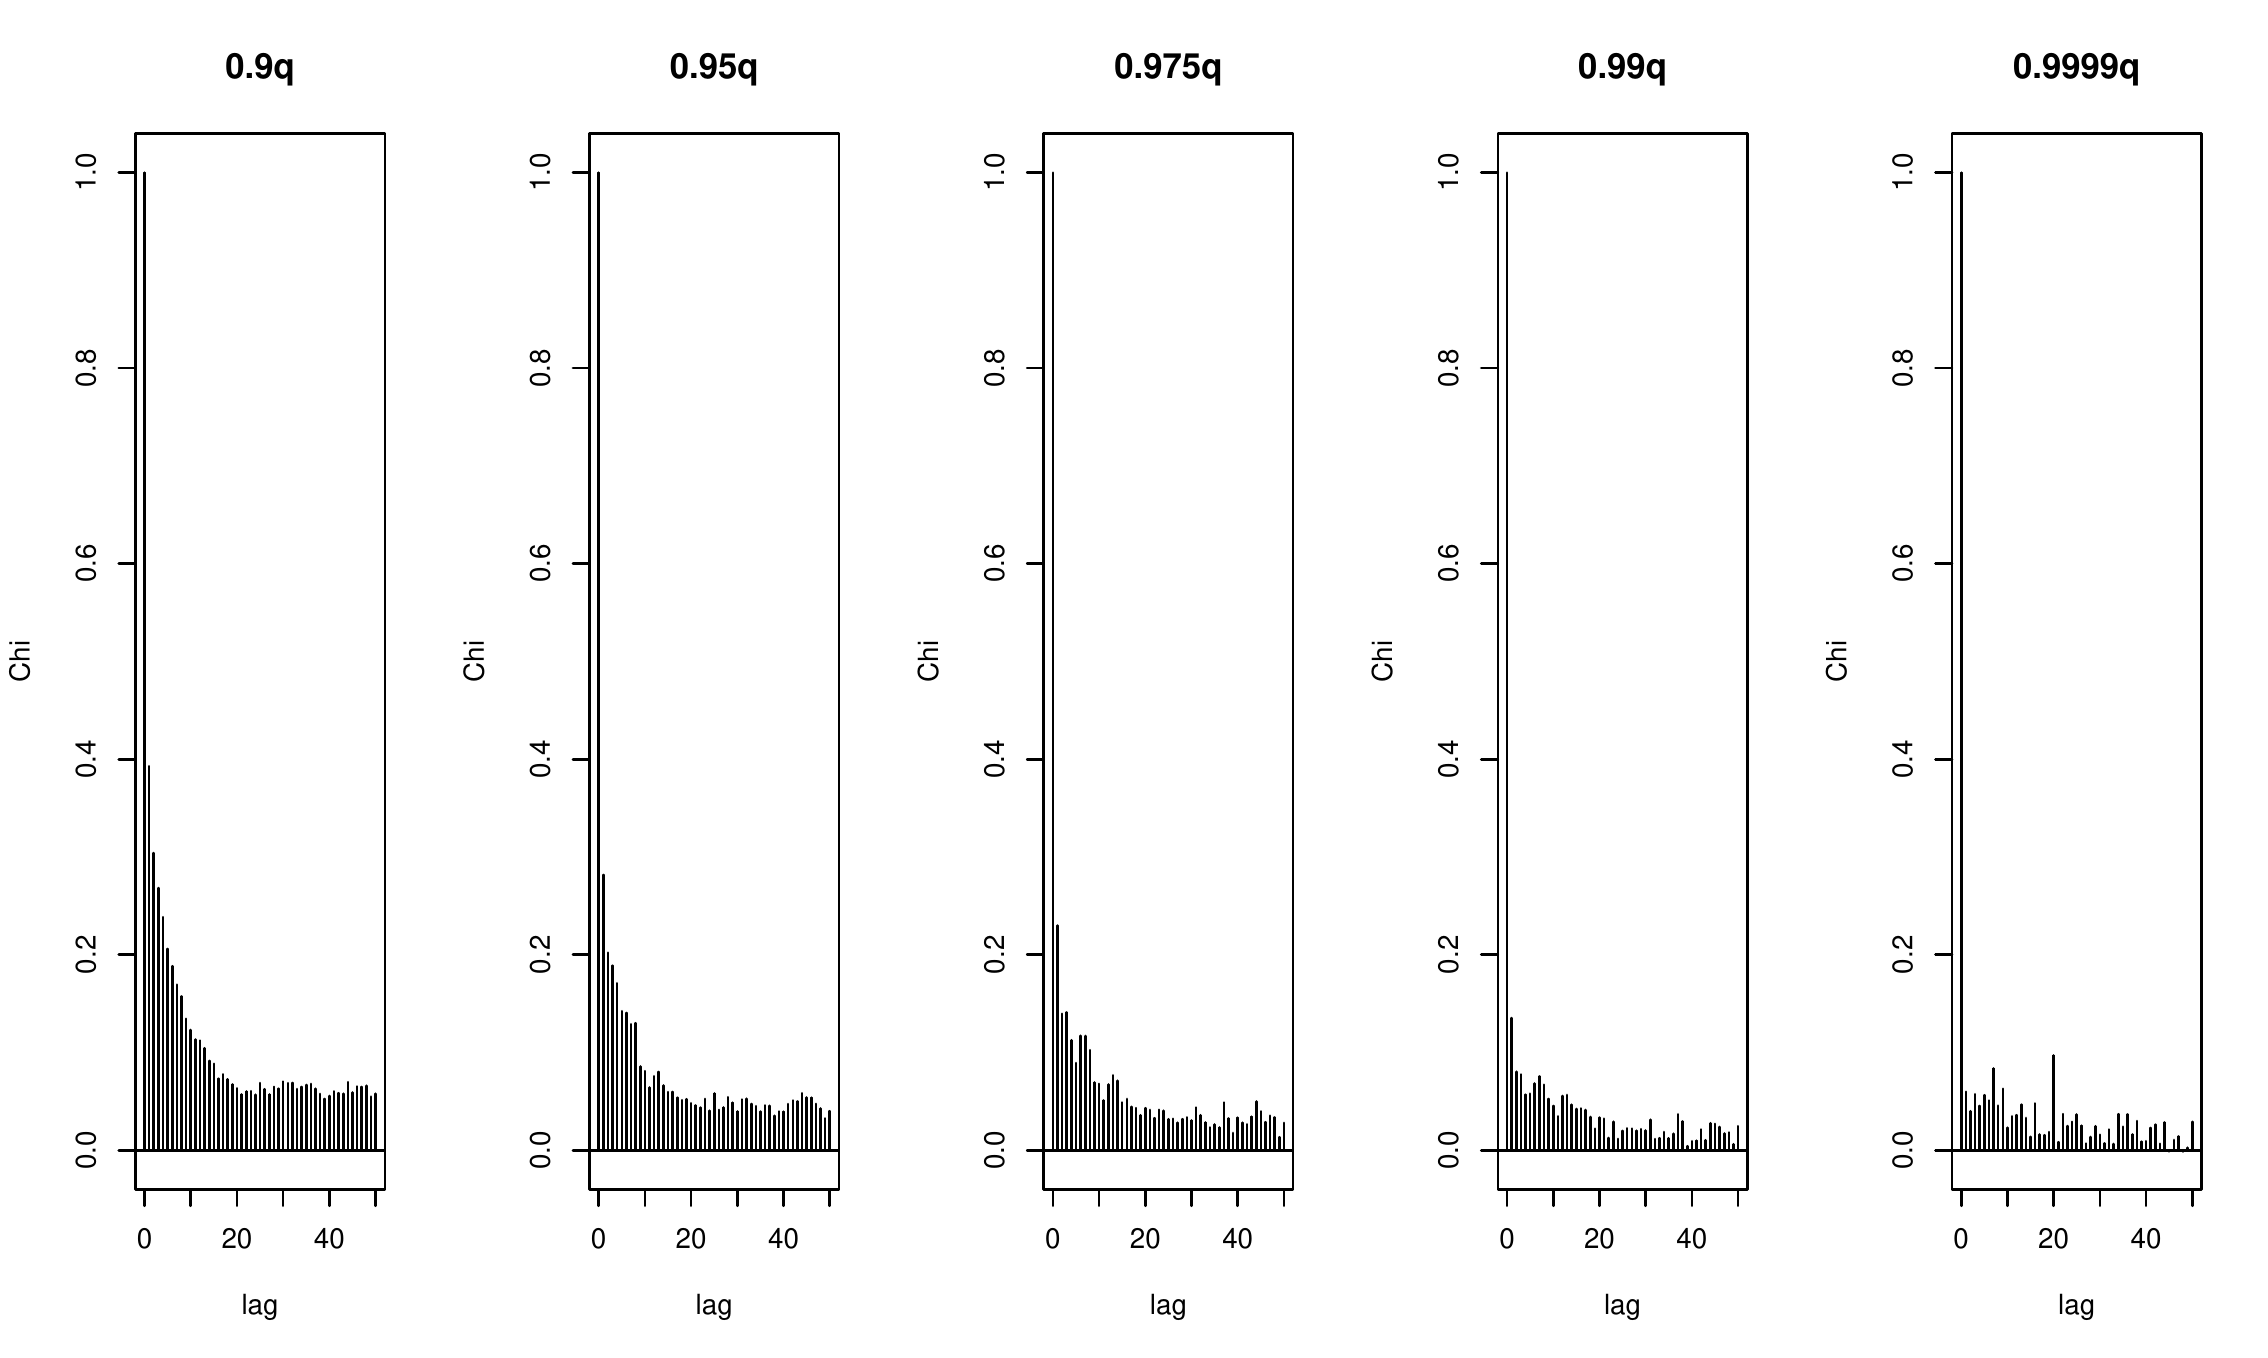} \\
    \includegraphics[width=0.85\textwidth,height=5cm]{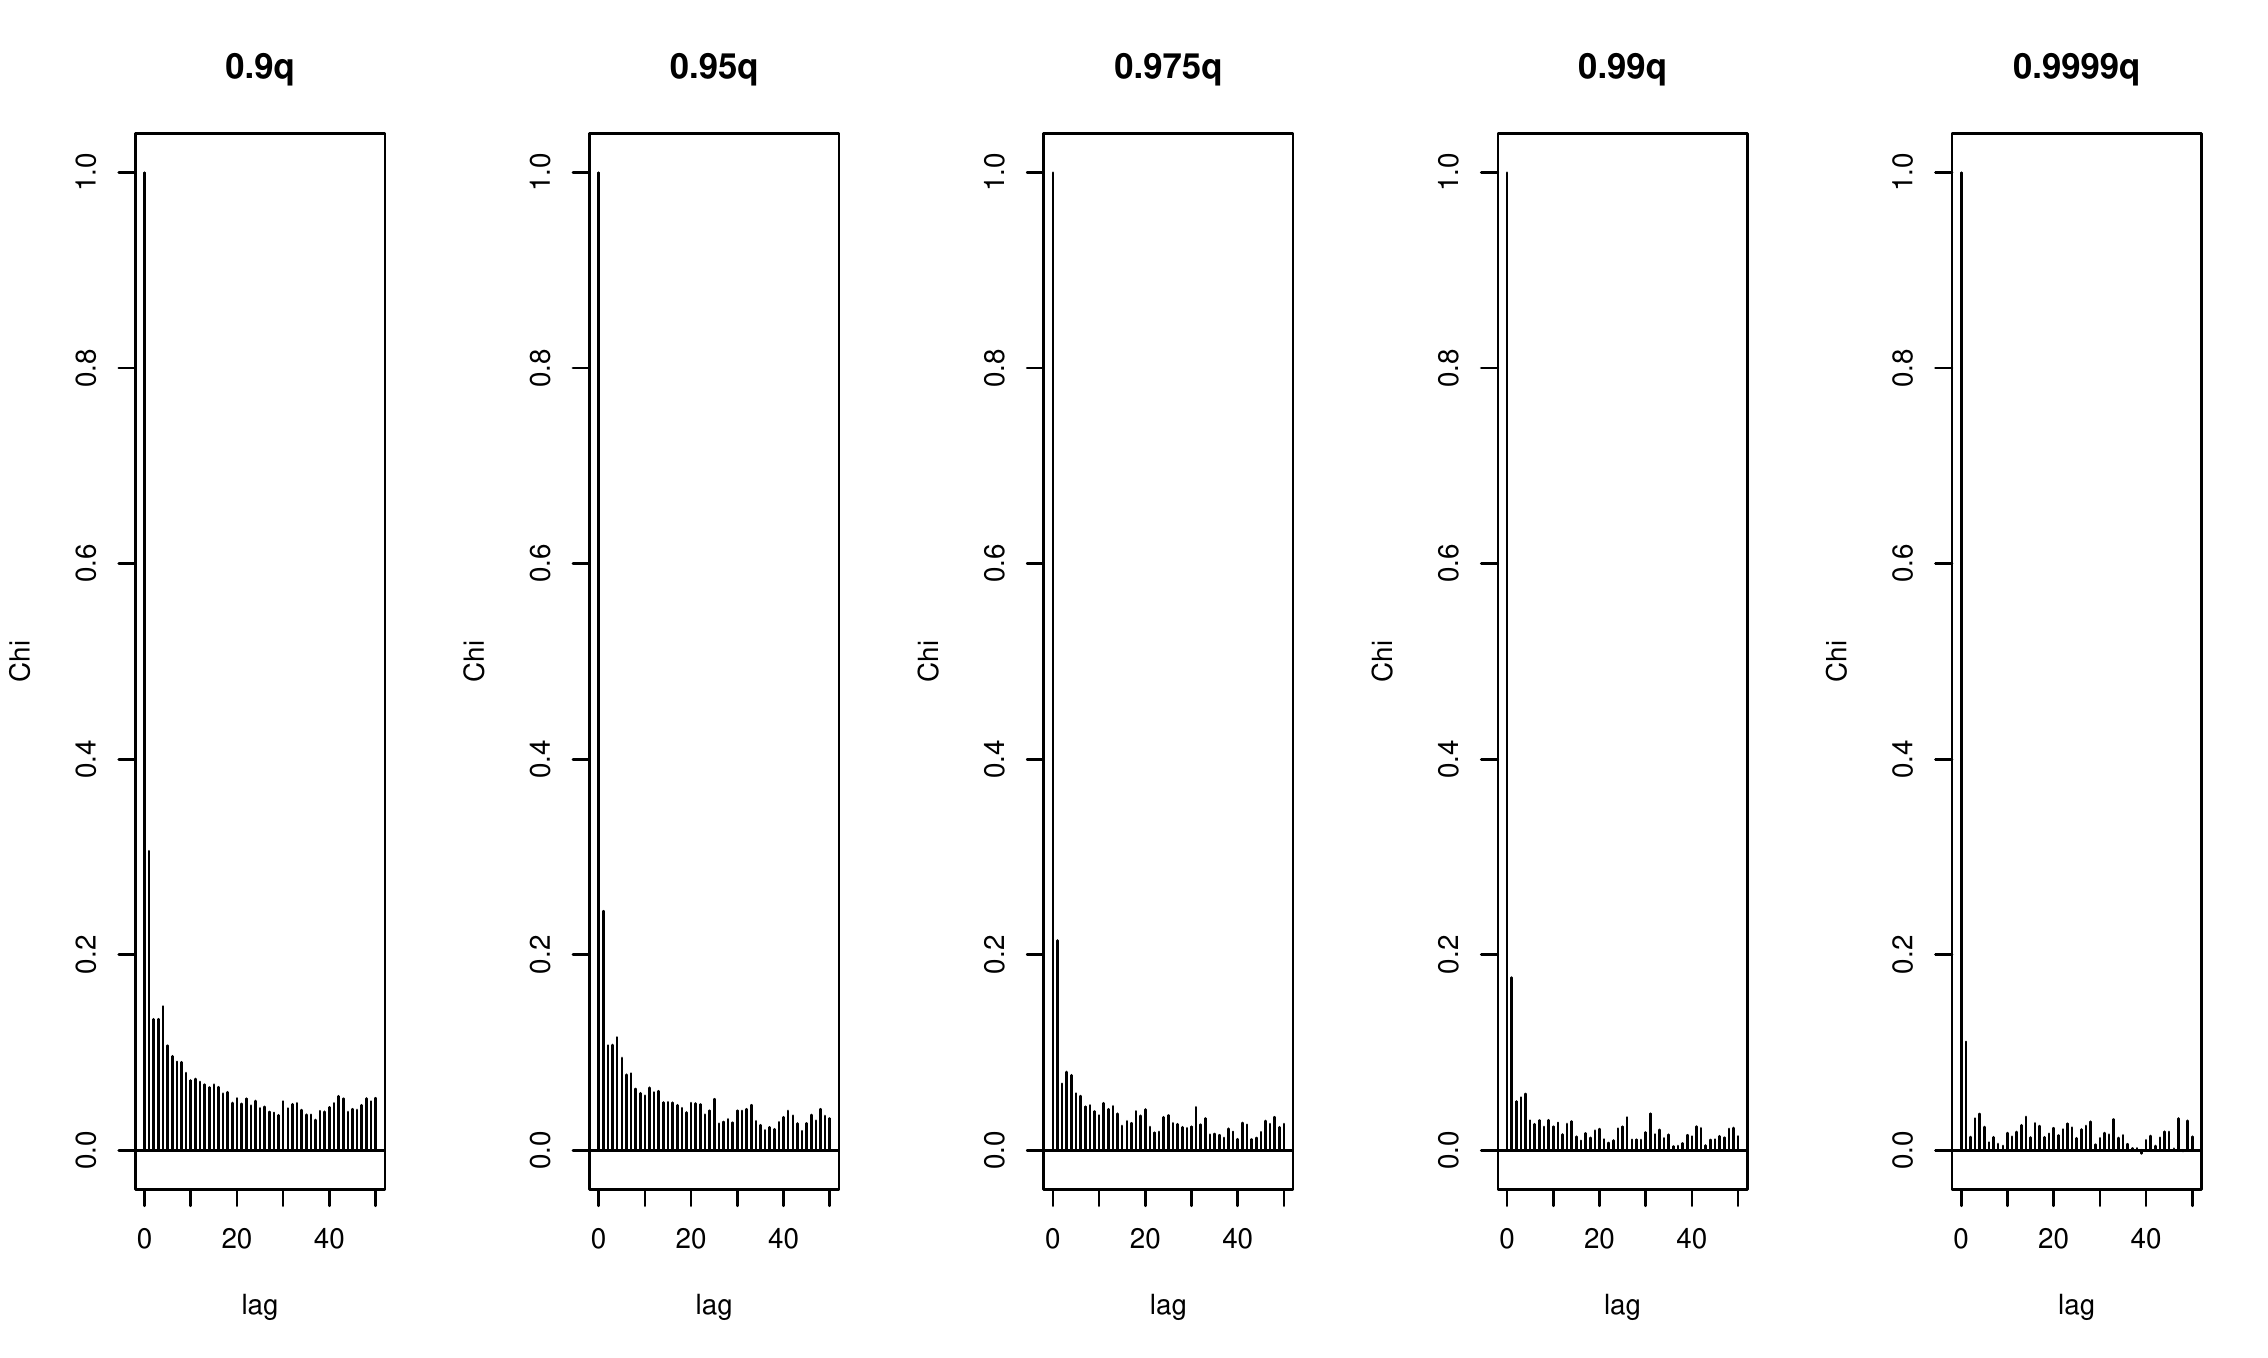} \\
    \includegraphics[width=0.85\textwidth,height=5cm]{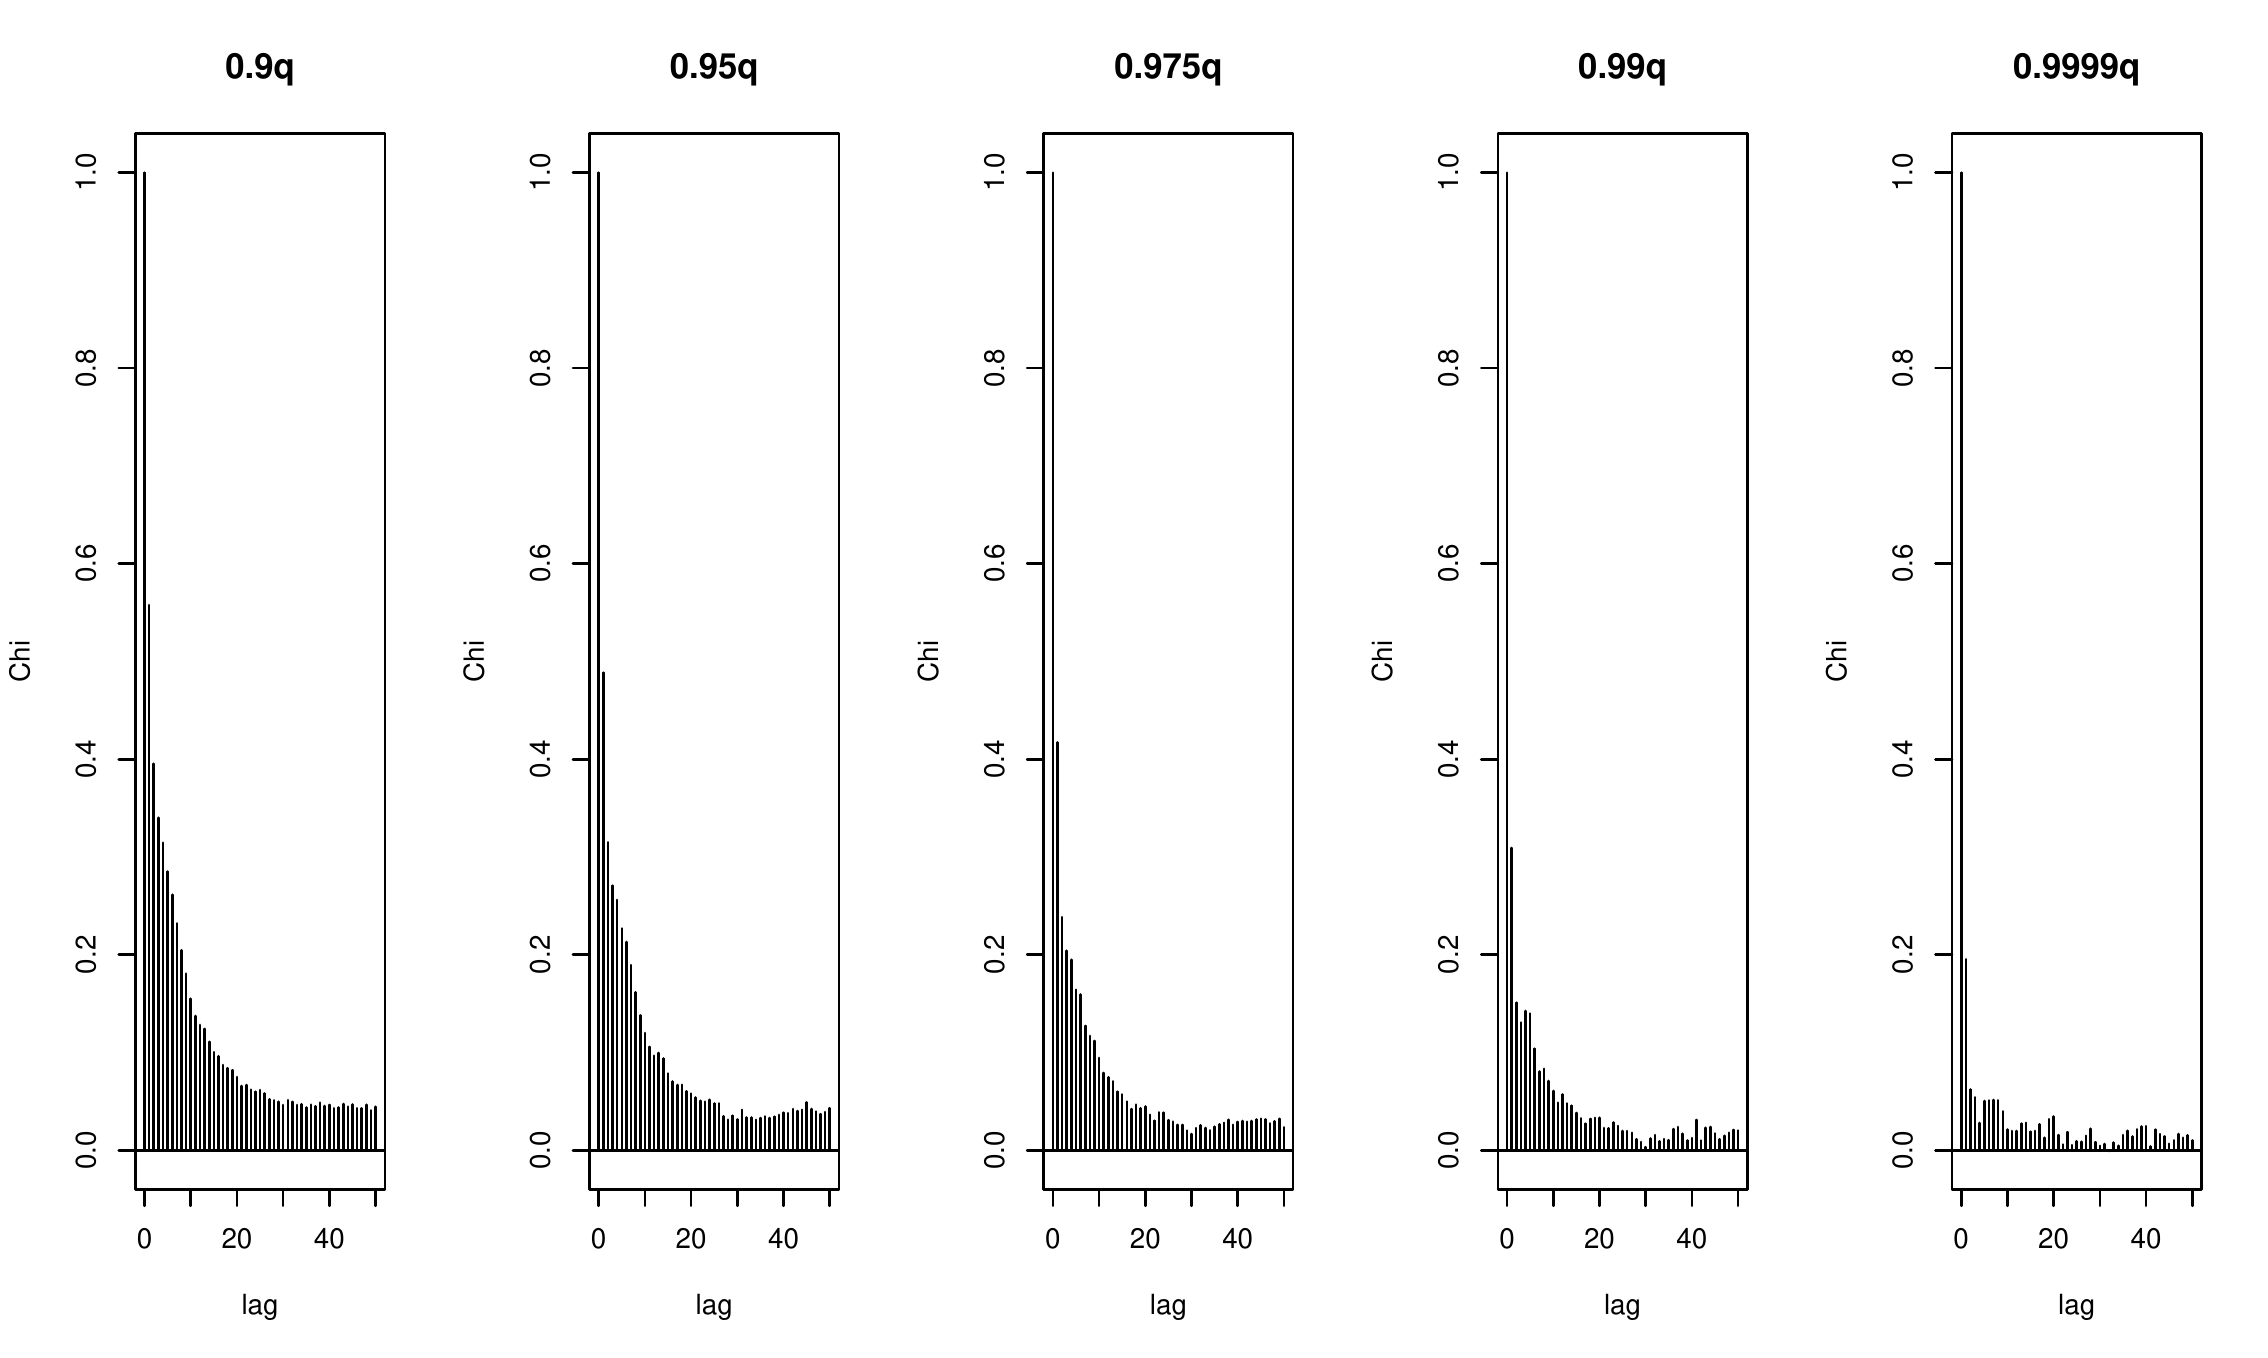} \\
    \includegraphics[width=0.85\textwidth,height=5cm]{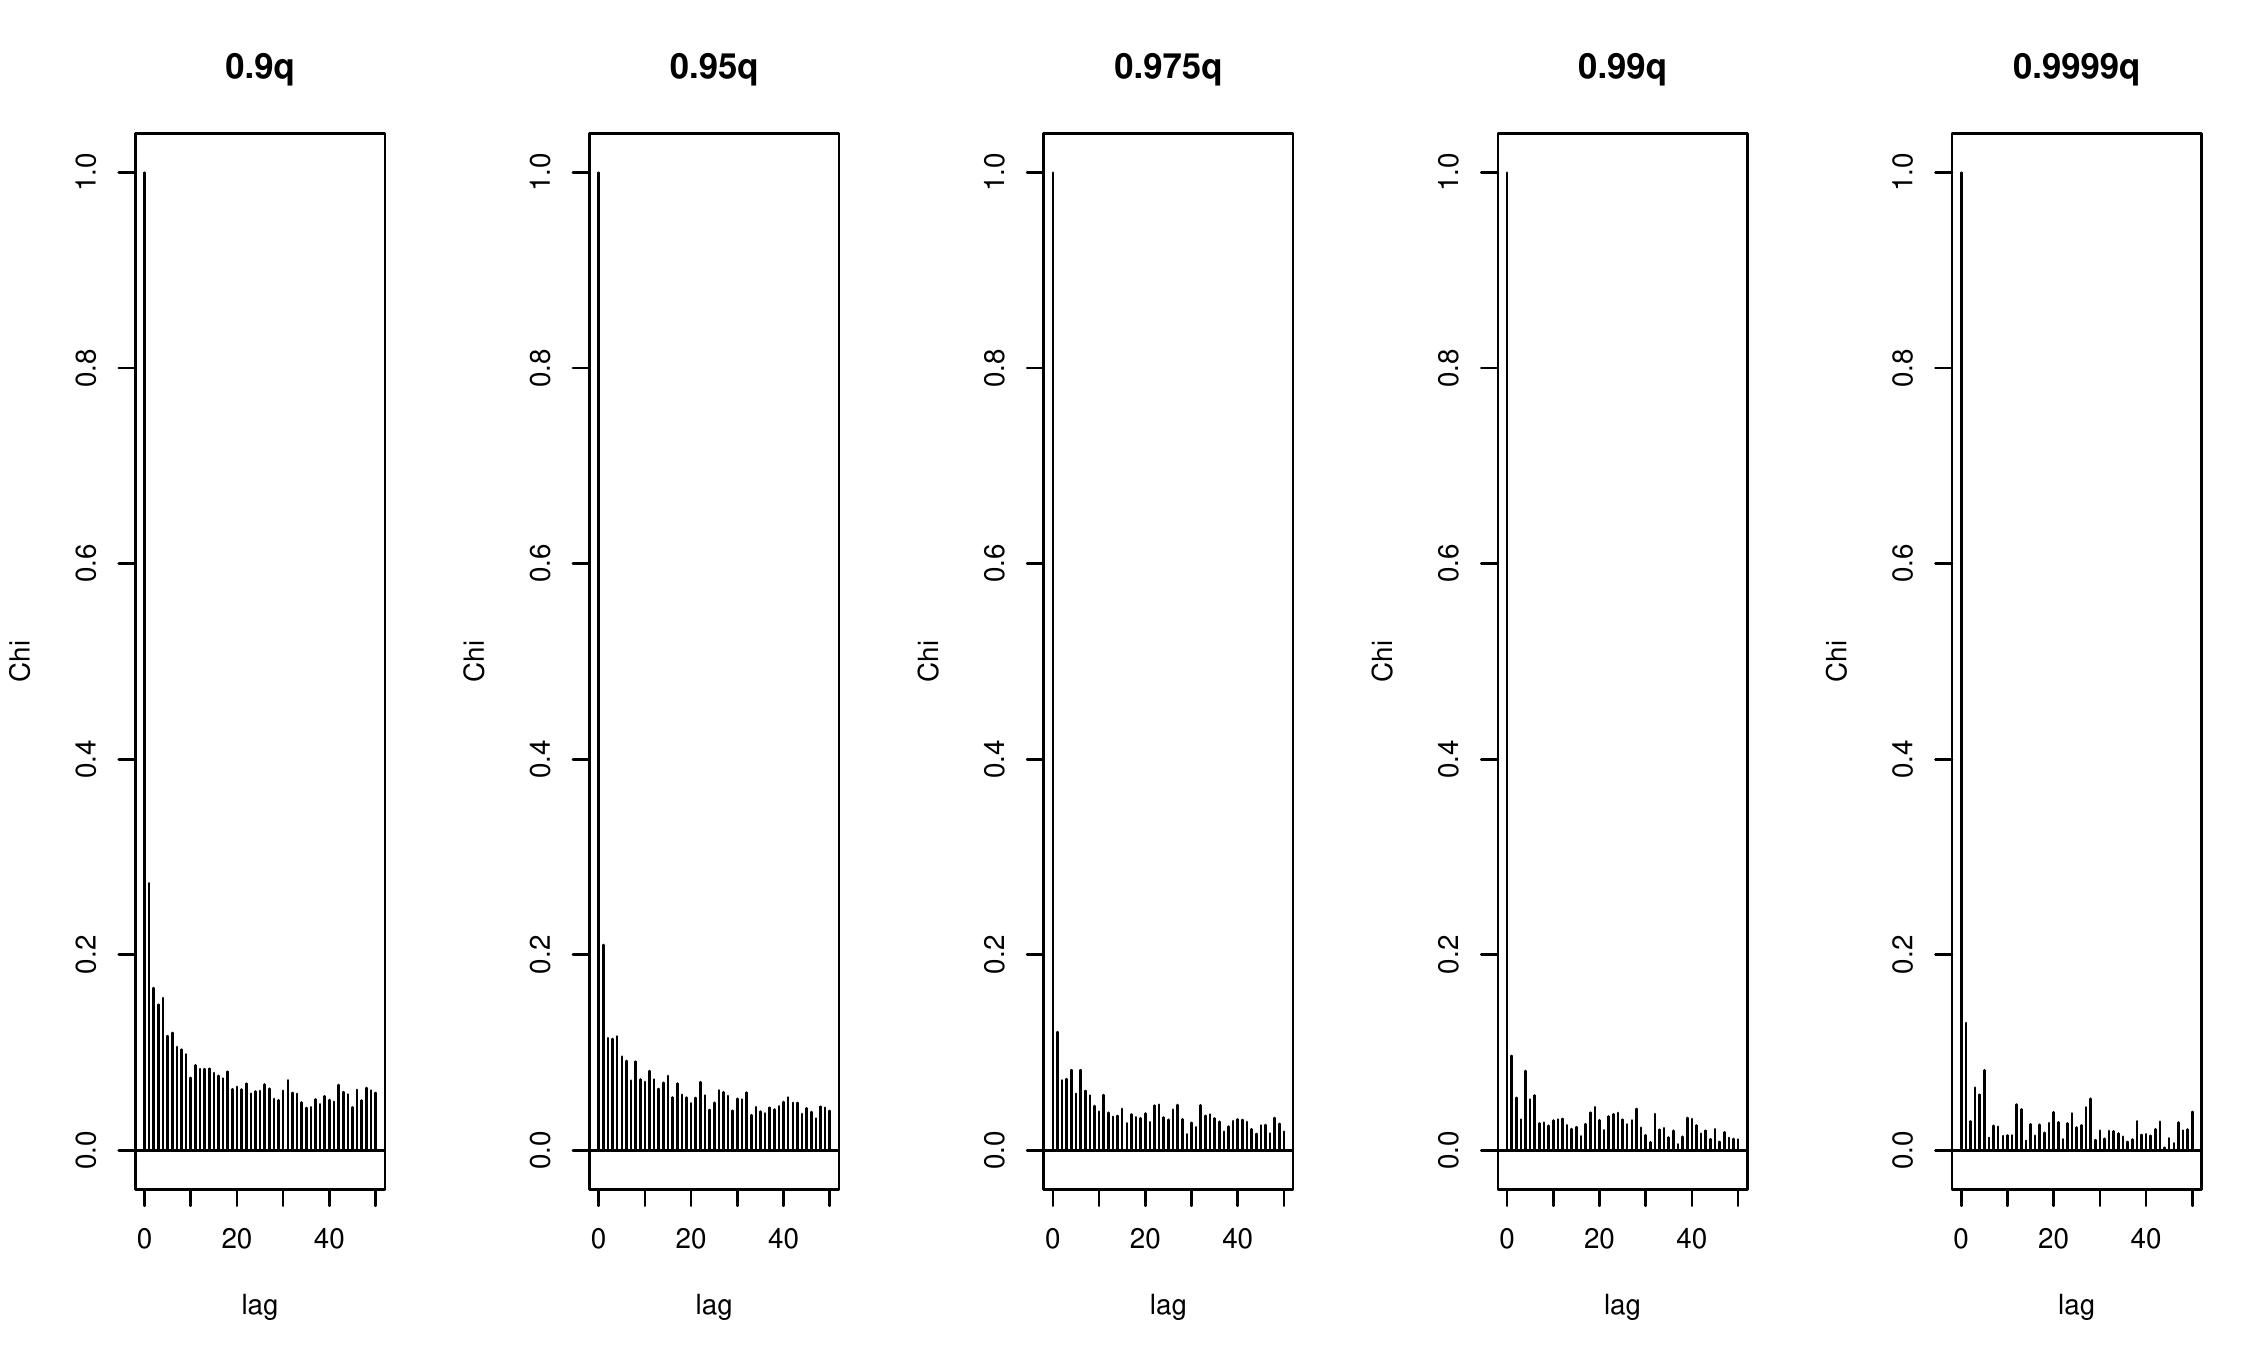}
    \caption{$\chi$ for Heysham, Lowestoft, Newlyn and Sheerness (from top to bottom) for exceedances of the 0.9, 0.95, 0.975, 0.99 and 0.999 quantiles for various lags.}
    \label{fig::chi}
\end{figure}

\begin{figure}
    \centering
    \includegraphics[width=0.49\textwidth]{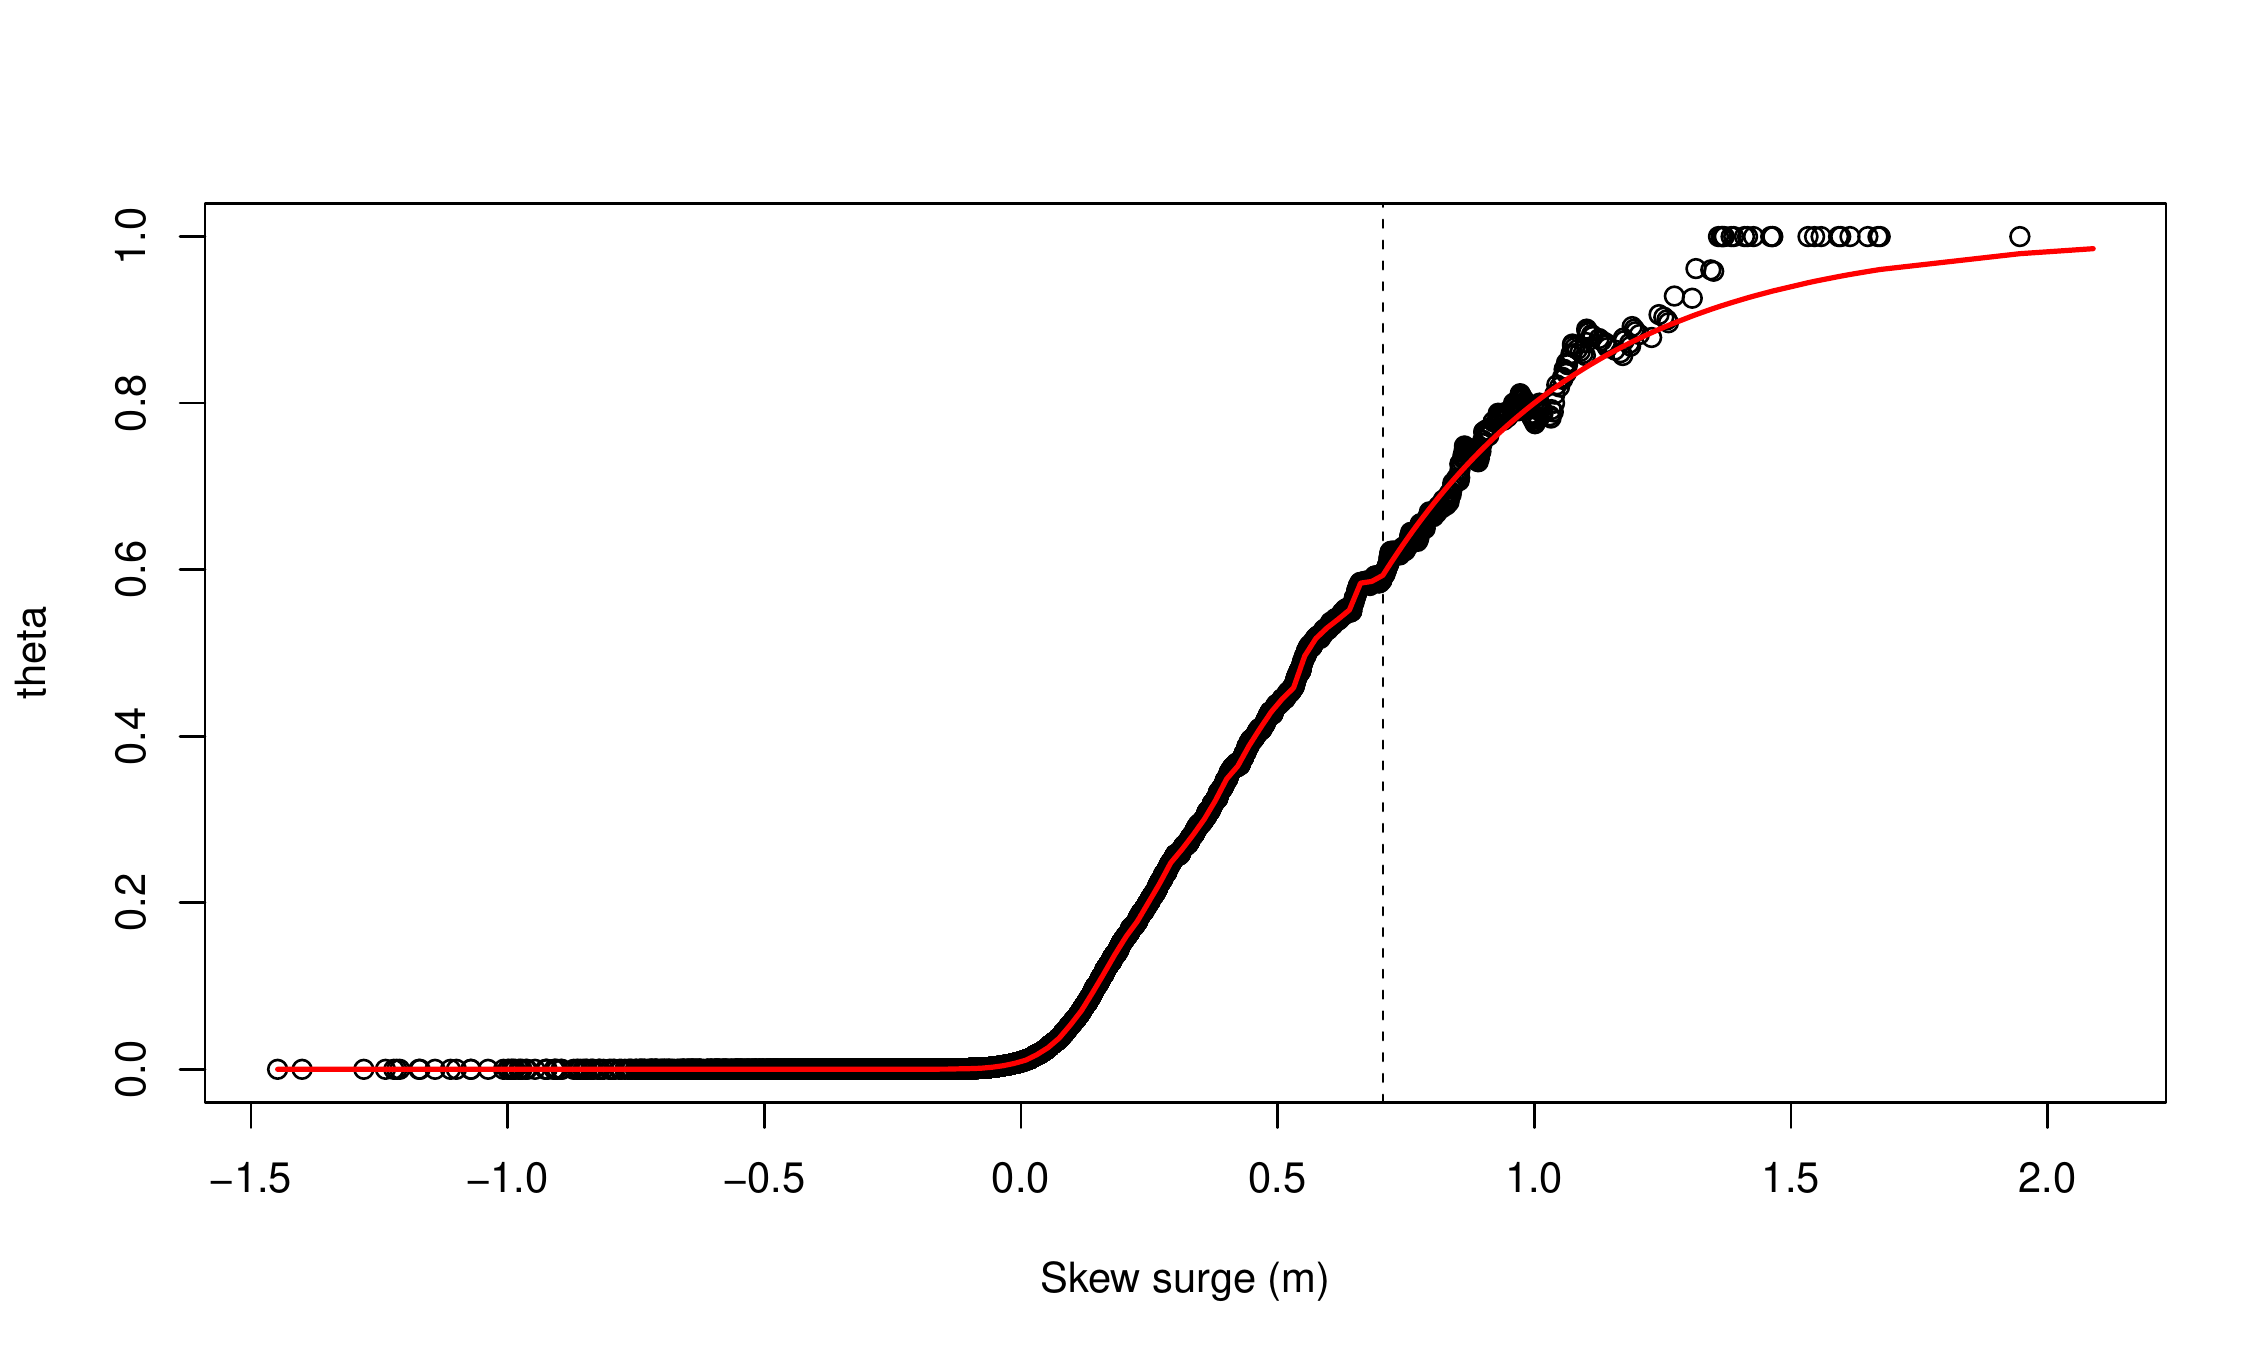}
    \includegraphics[width=0.49\textwidth]{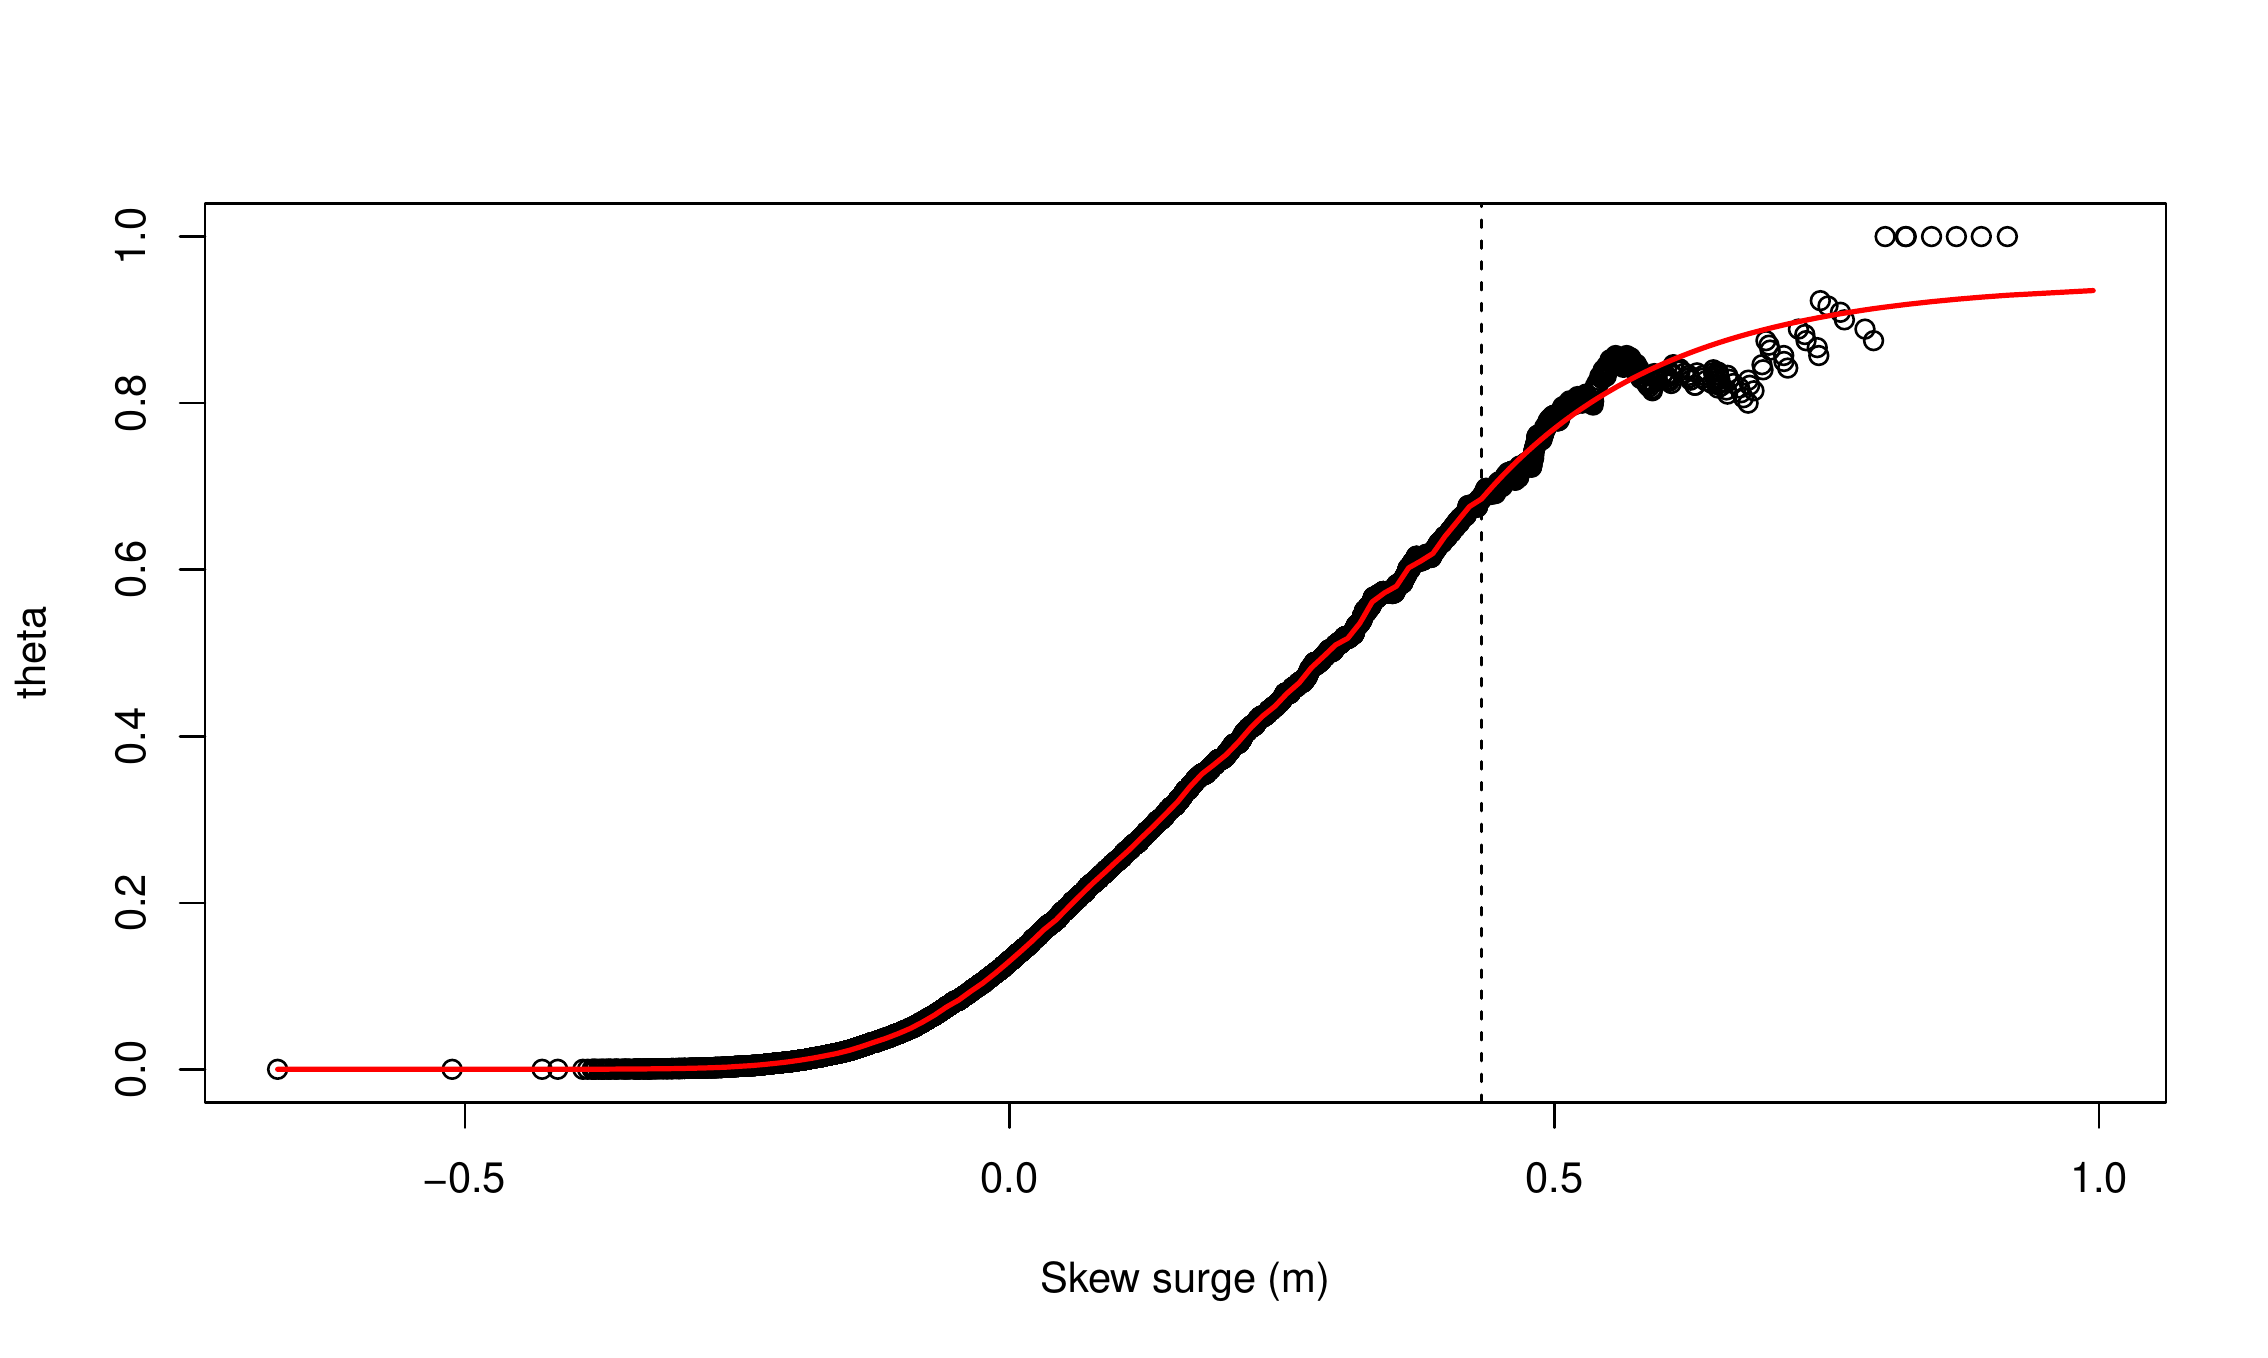}
    \includegraphics[width=0.49\textwidth]{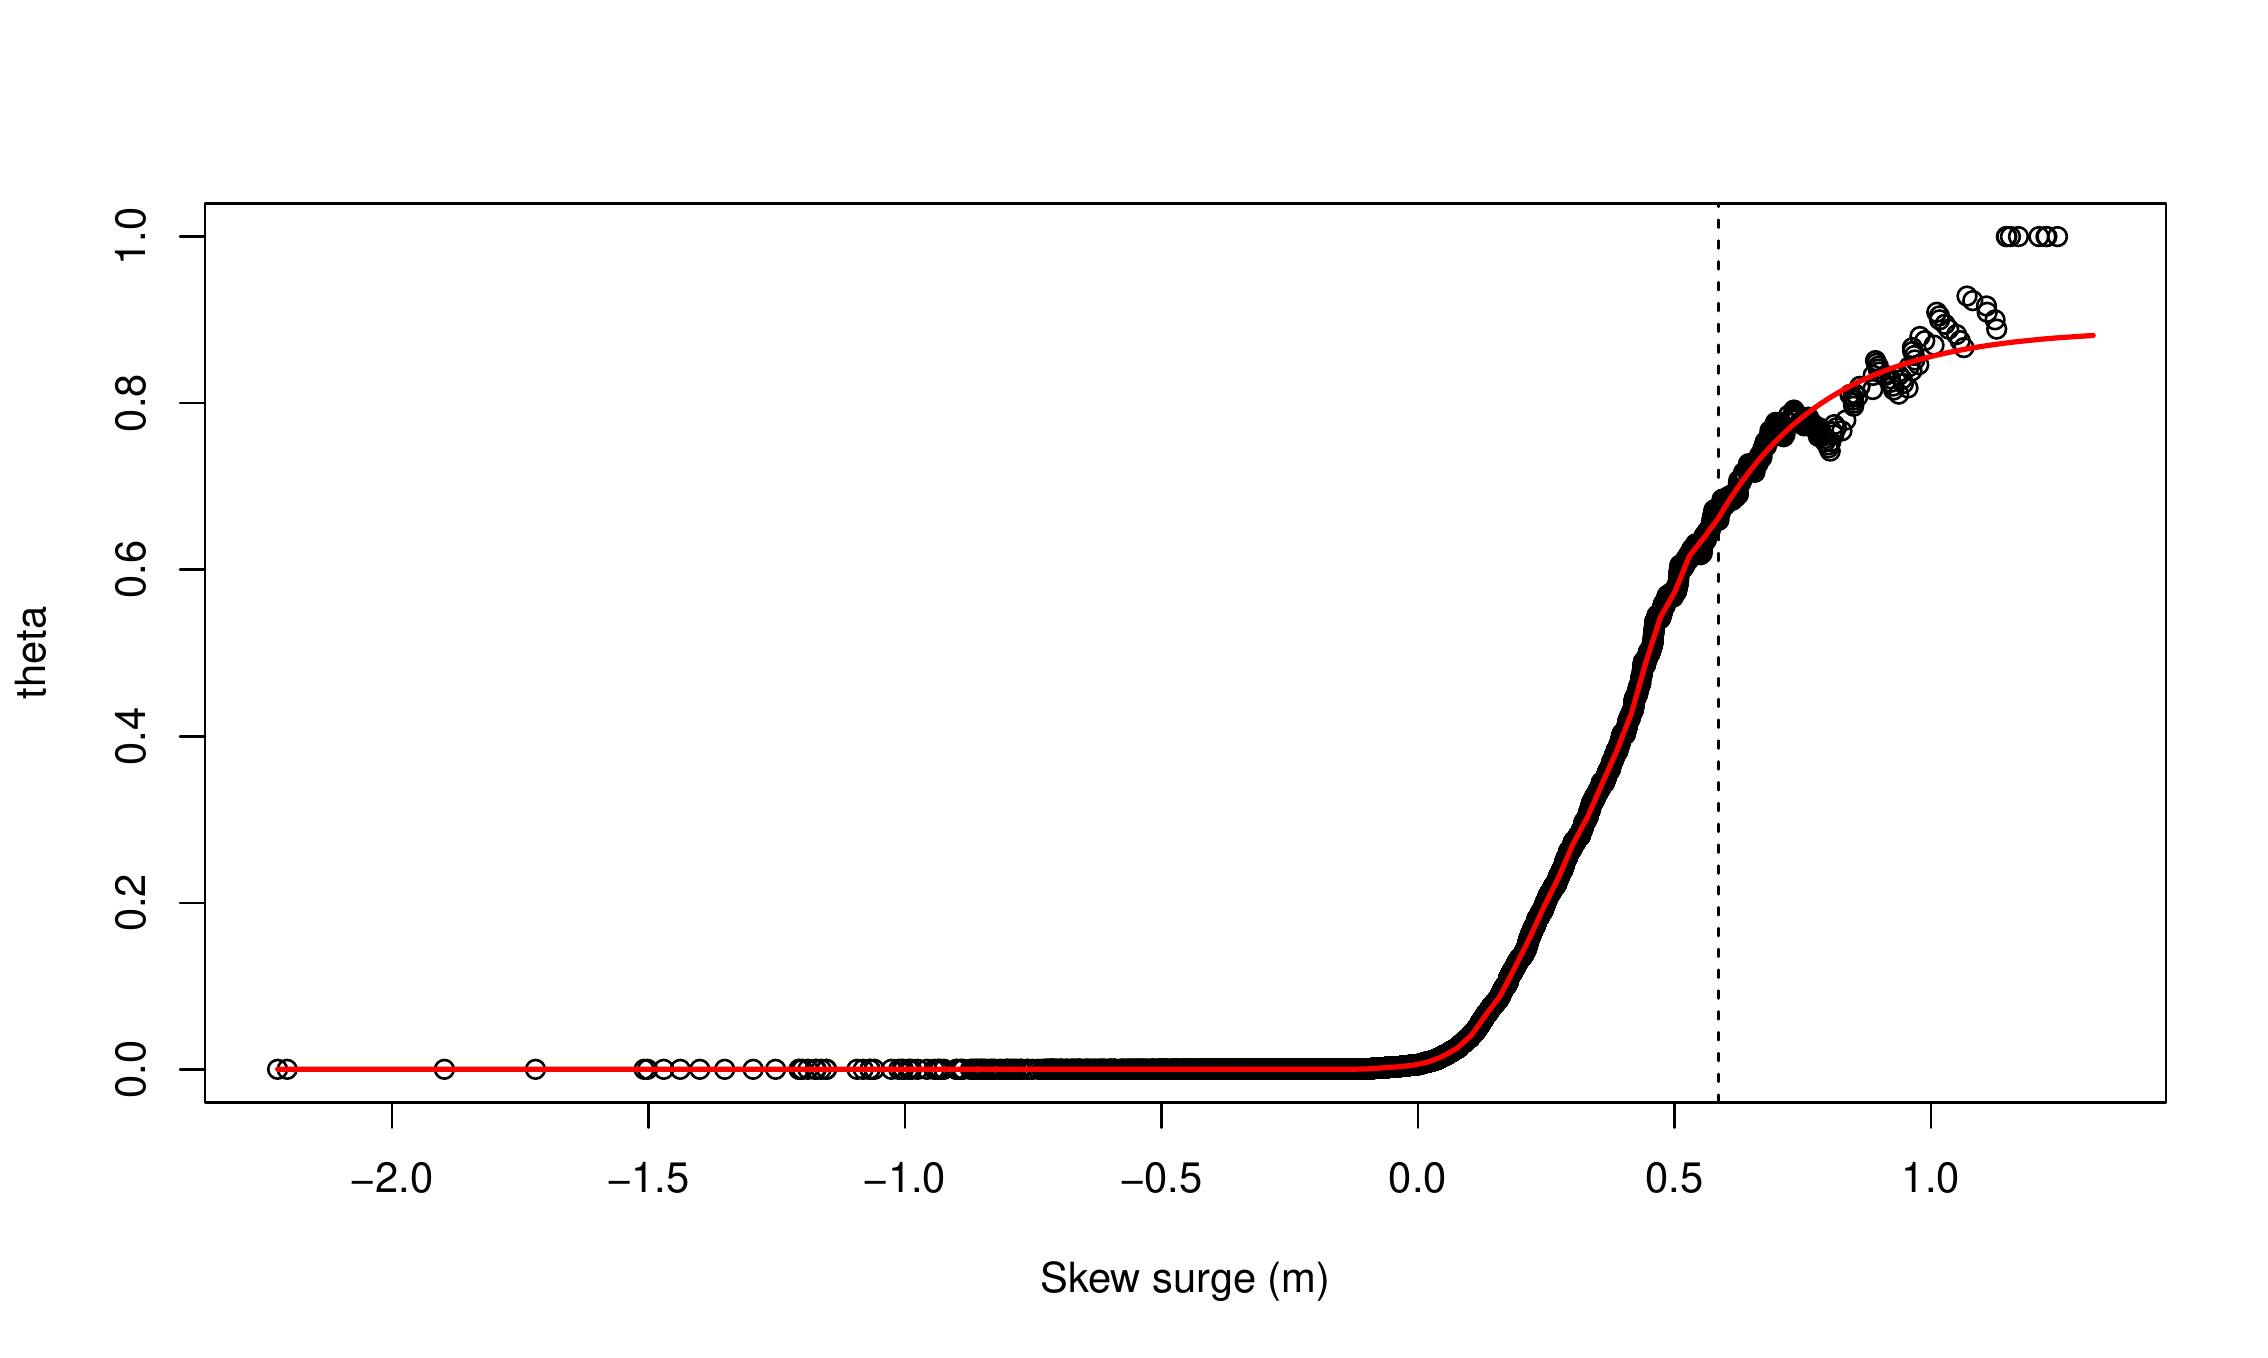}
    \caption{Estimates of the subasymptotic extremal index $\theta(y,r)$ for different skew surge levels using the runs estimate (black) and our model estimate (red) of expression~\eqref{eqn::exi_model} at Lowestoft (top left), Newlyn (middle) and Sheerness (bottom). Run lengths are chosen as 10, 2 and 10, respectively. And the threshold $v$ is chosen as the 0.99 skew surge quantile at all sites.}
    \label{fig::exifun_all}
\end{figure}

\begin{figure}
    \centering
    \includegraphics[width=0.85\textwidth,height=5cm]{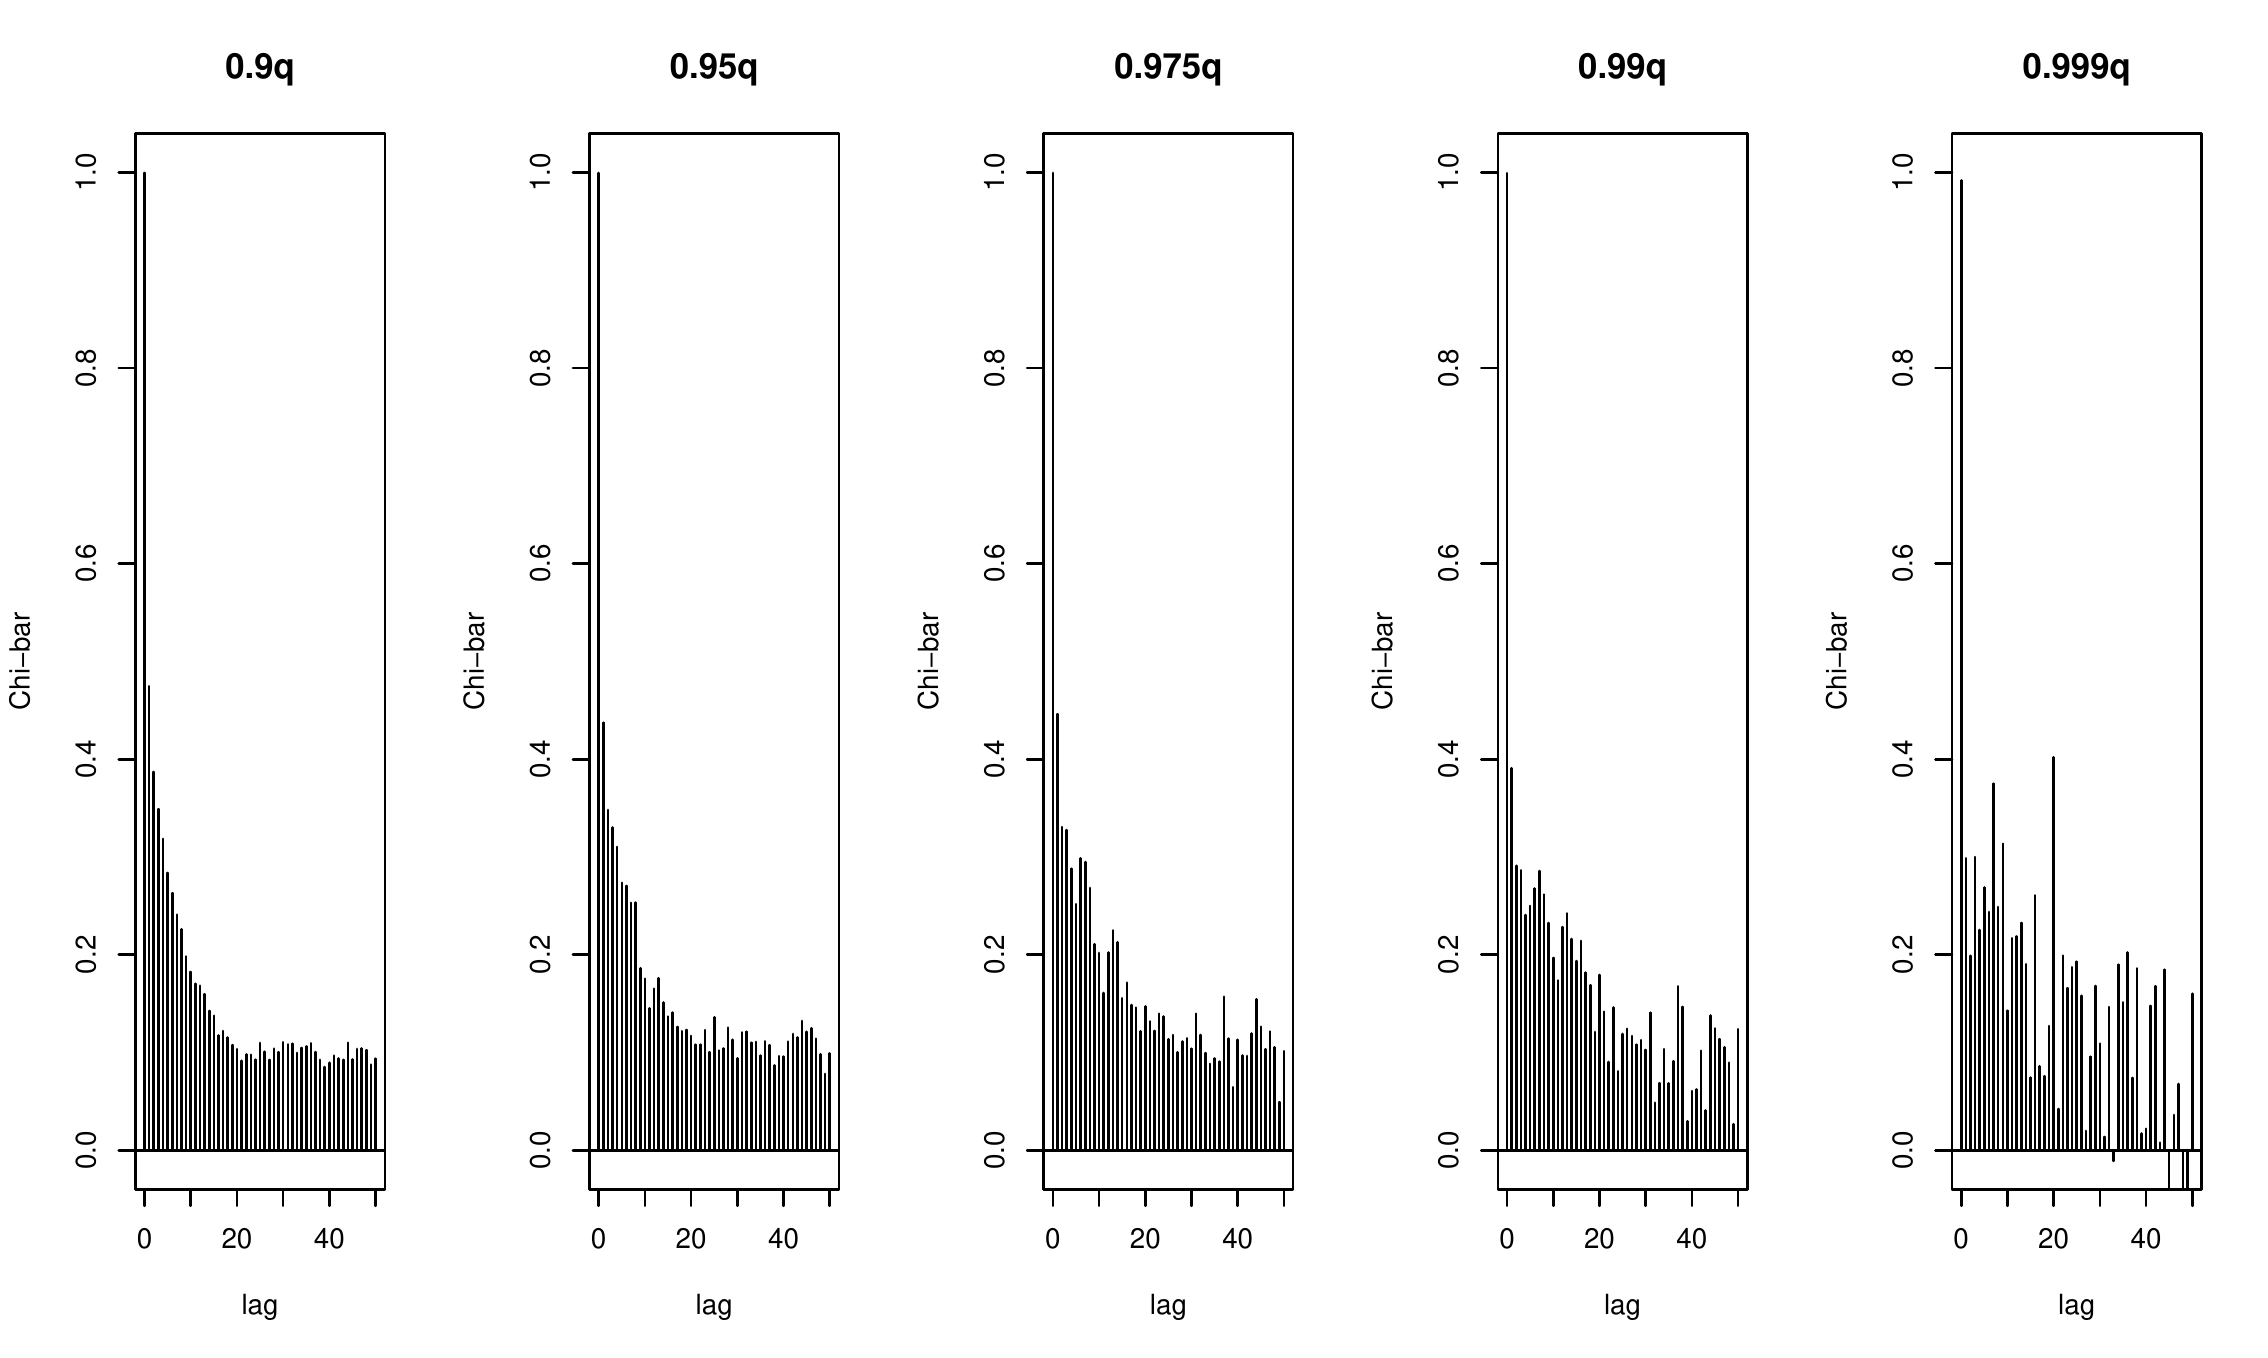} \\
    \includegraphics[width=0.85\textwidth,height=5cm]{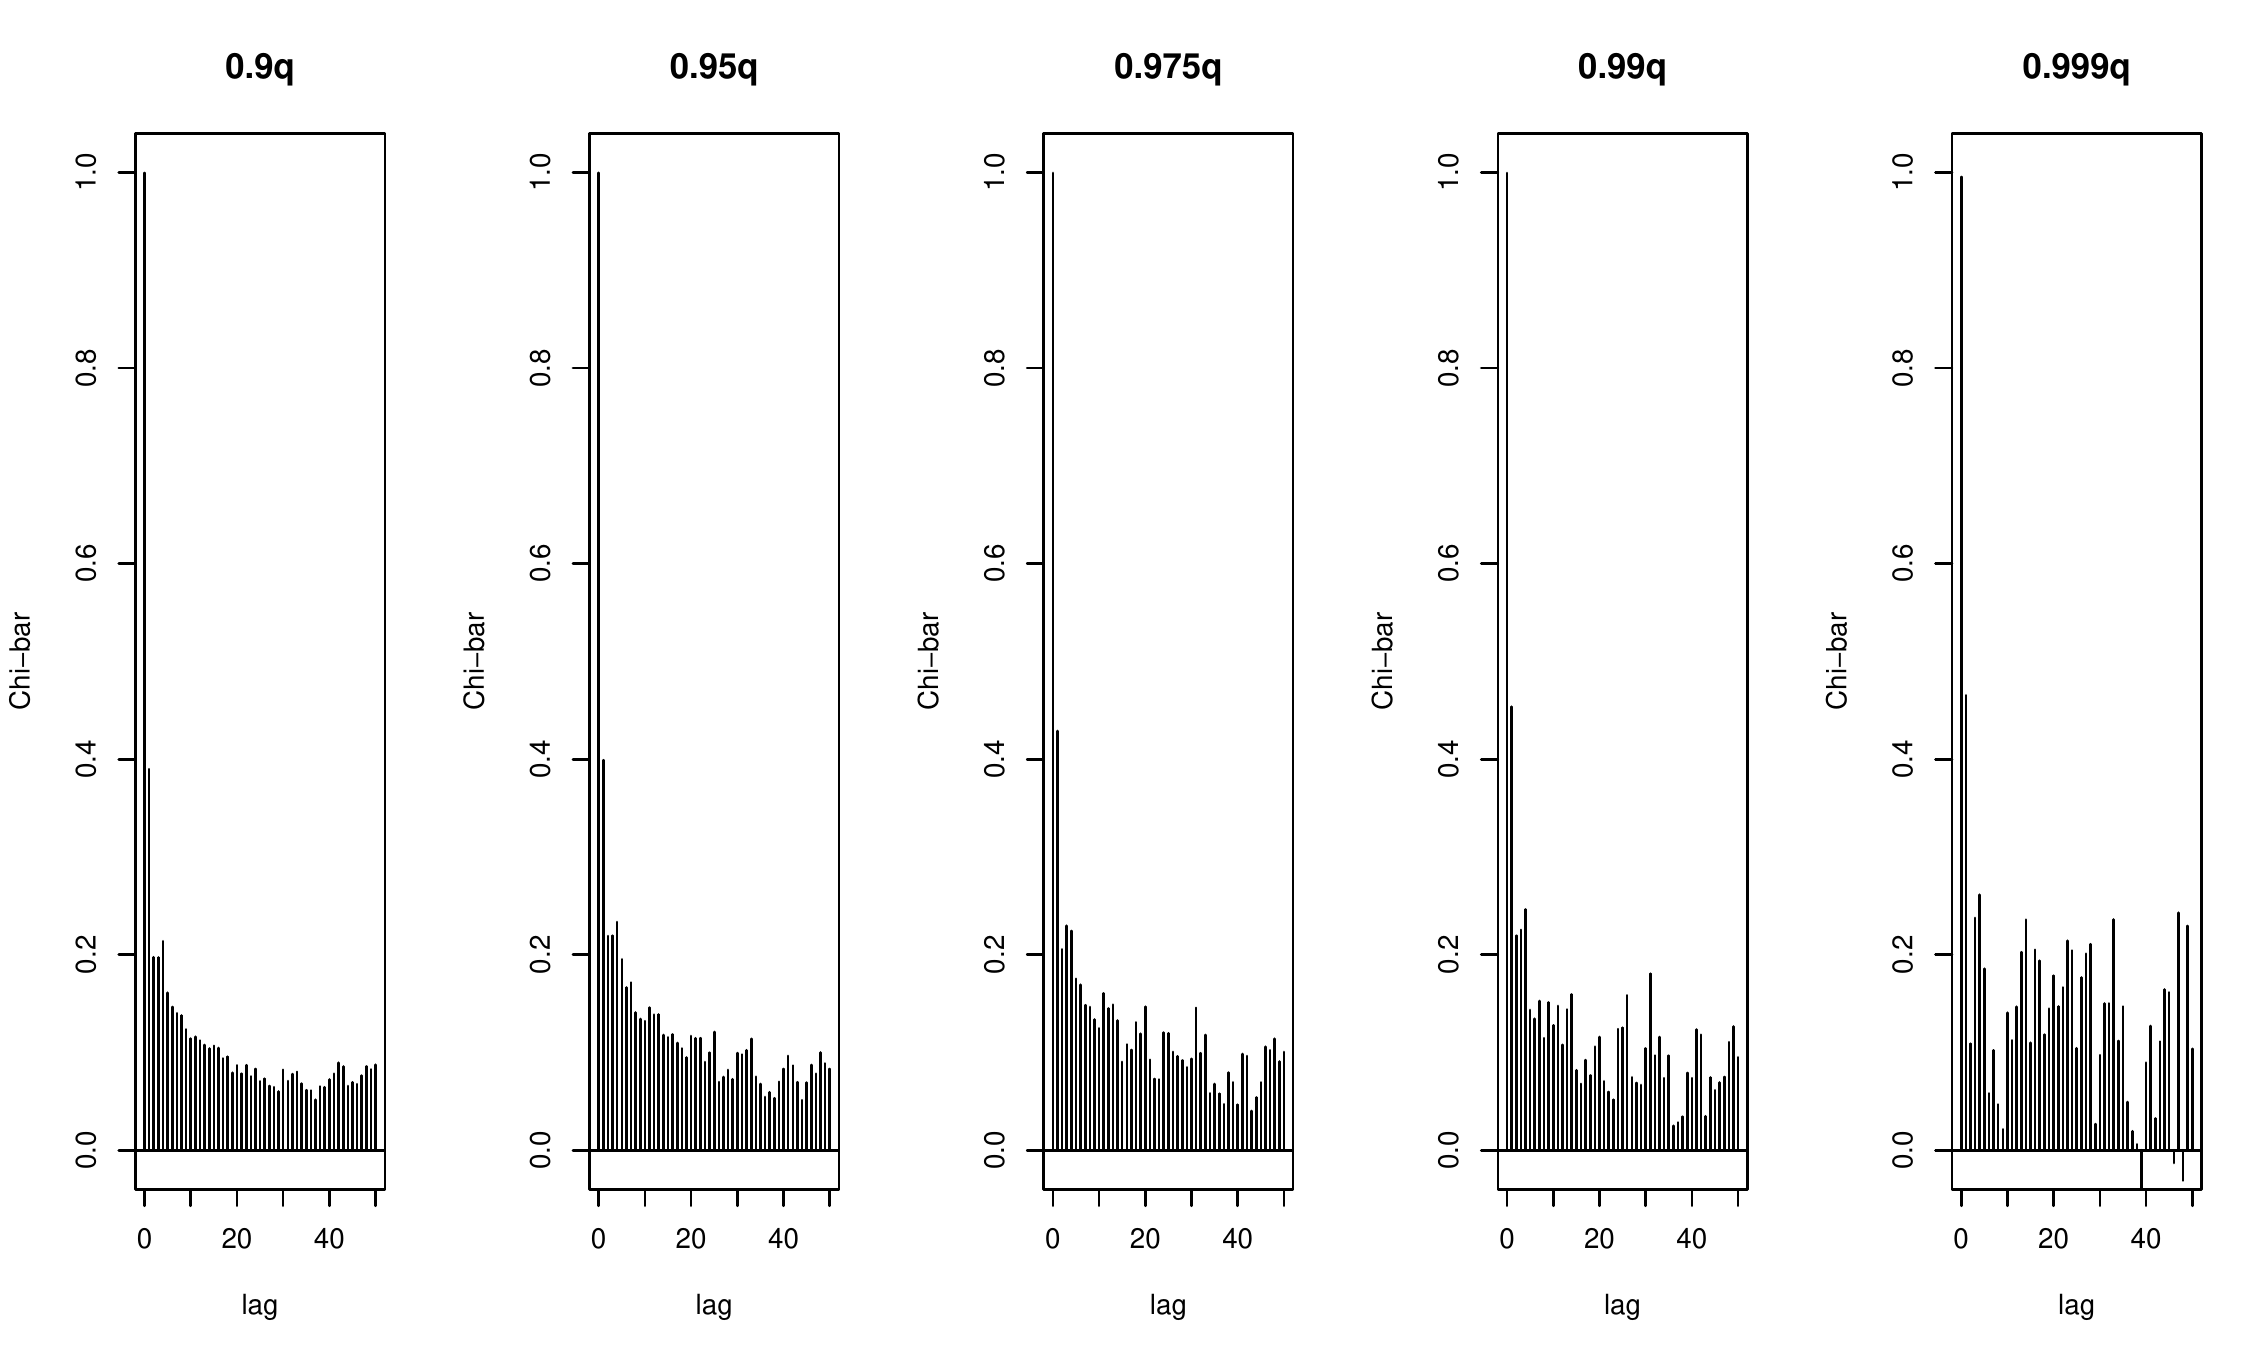} \\
    \includegraphics[width=0.85\textwidth,height=5cm]{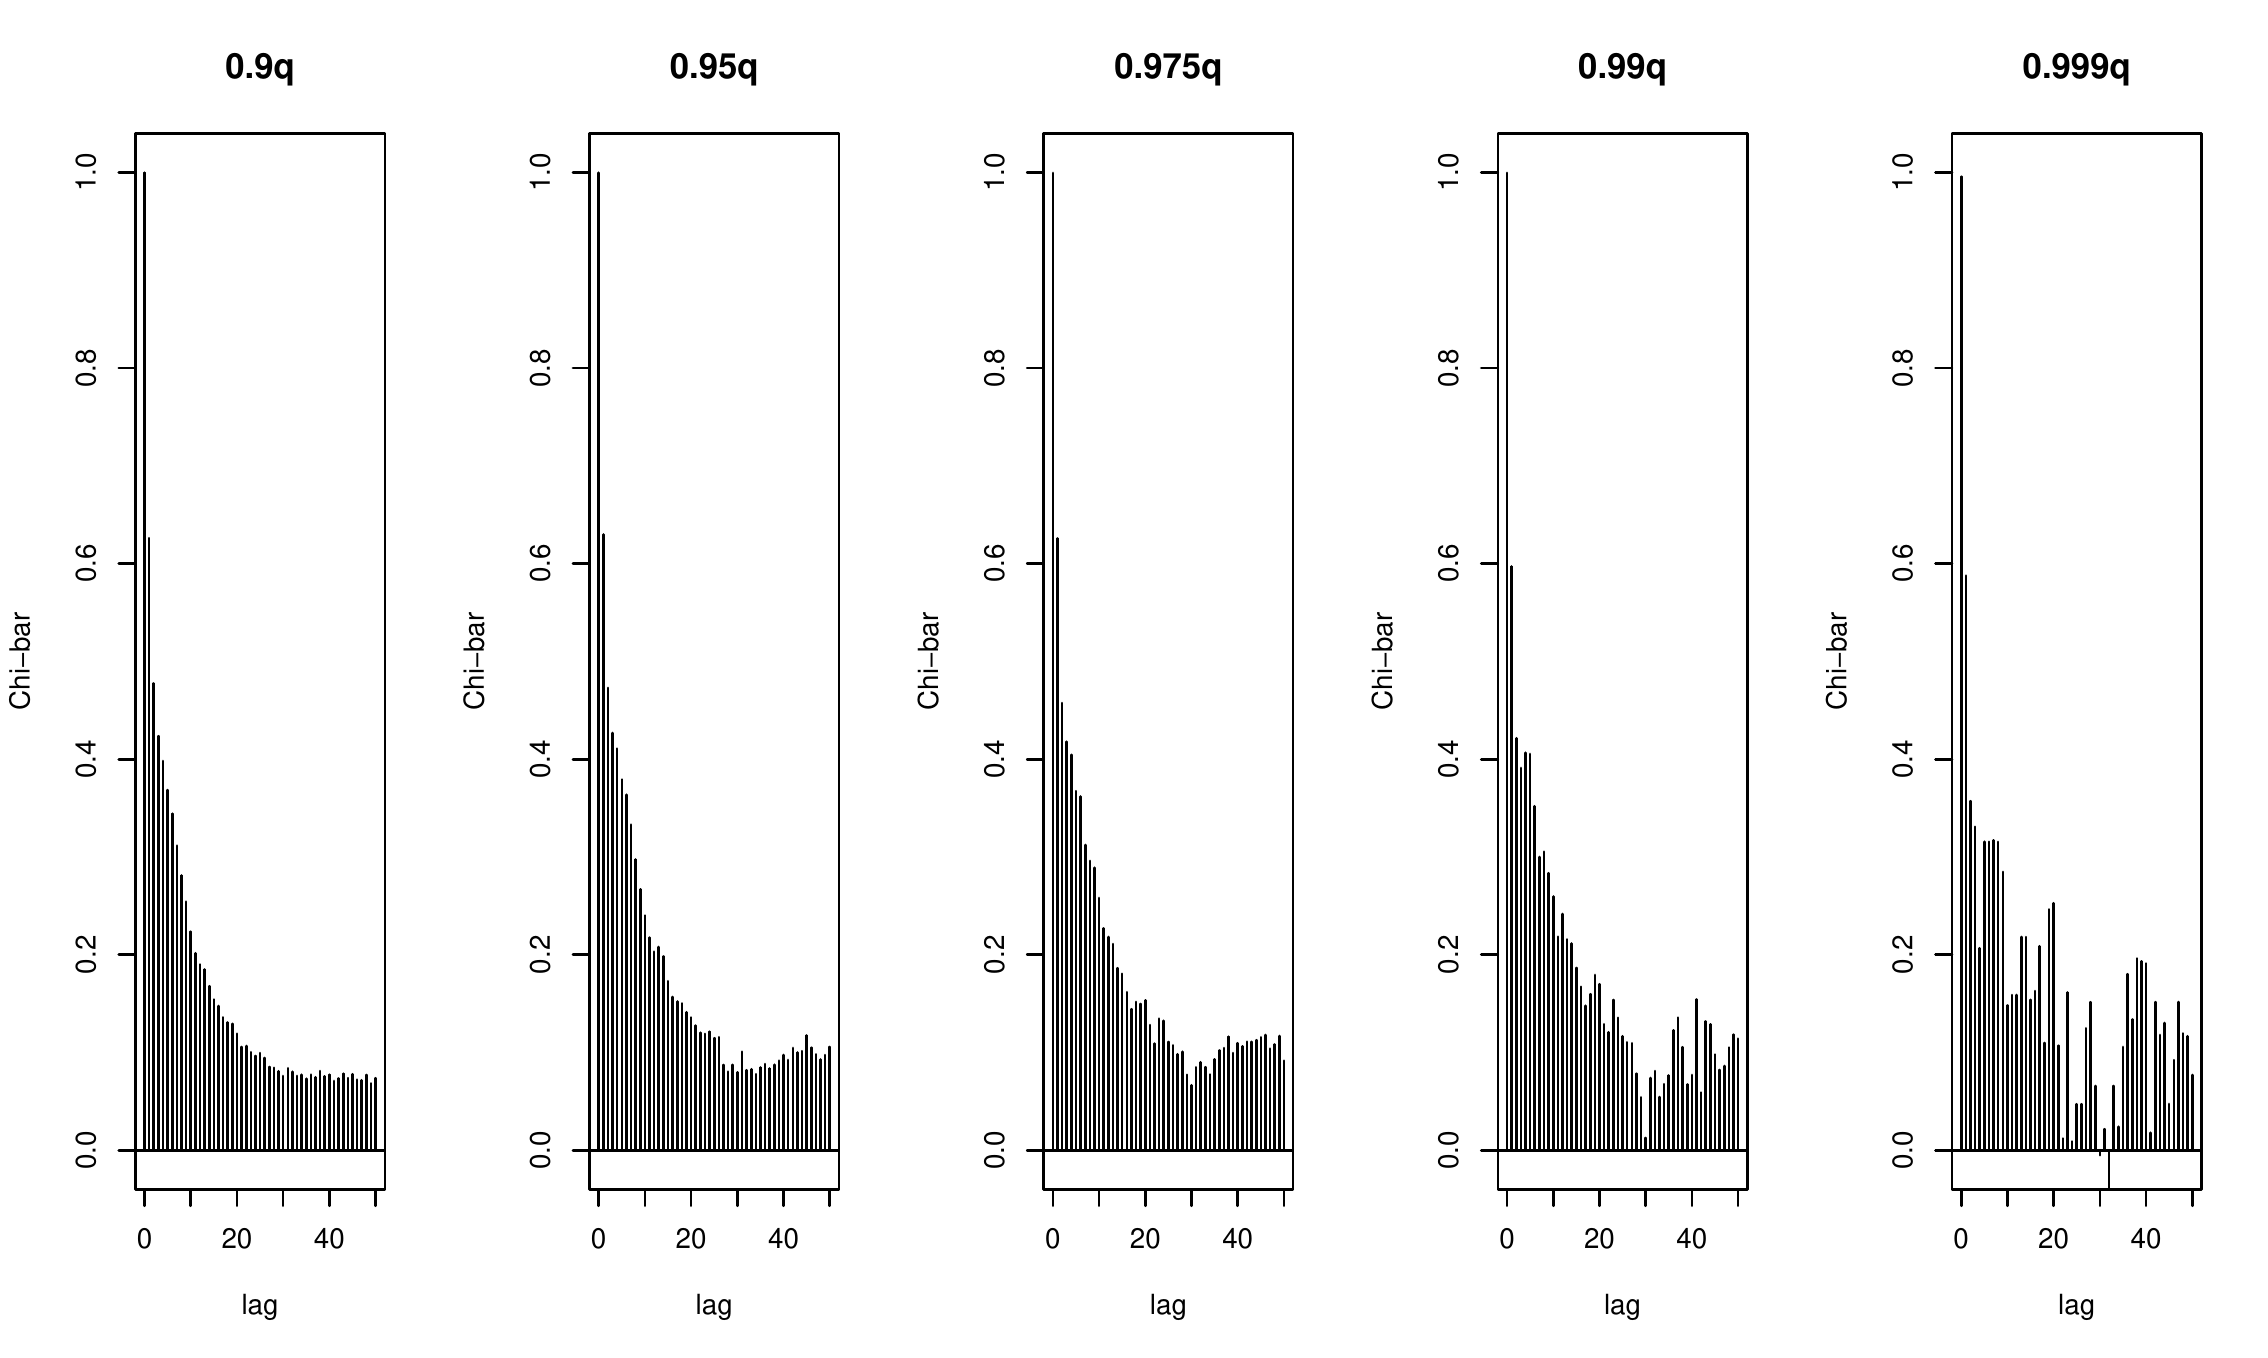} \\
    \includegraphics[width=0.85\textwidth,height=5cm]{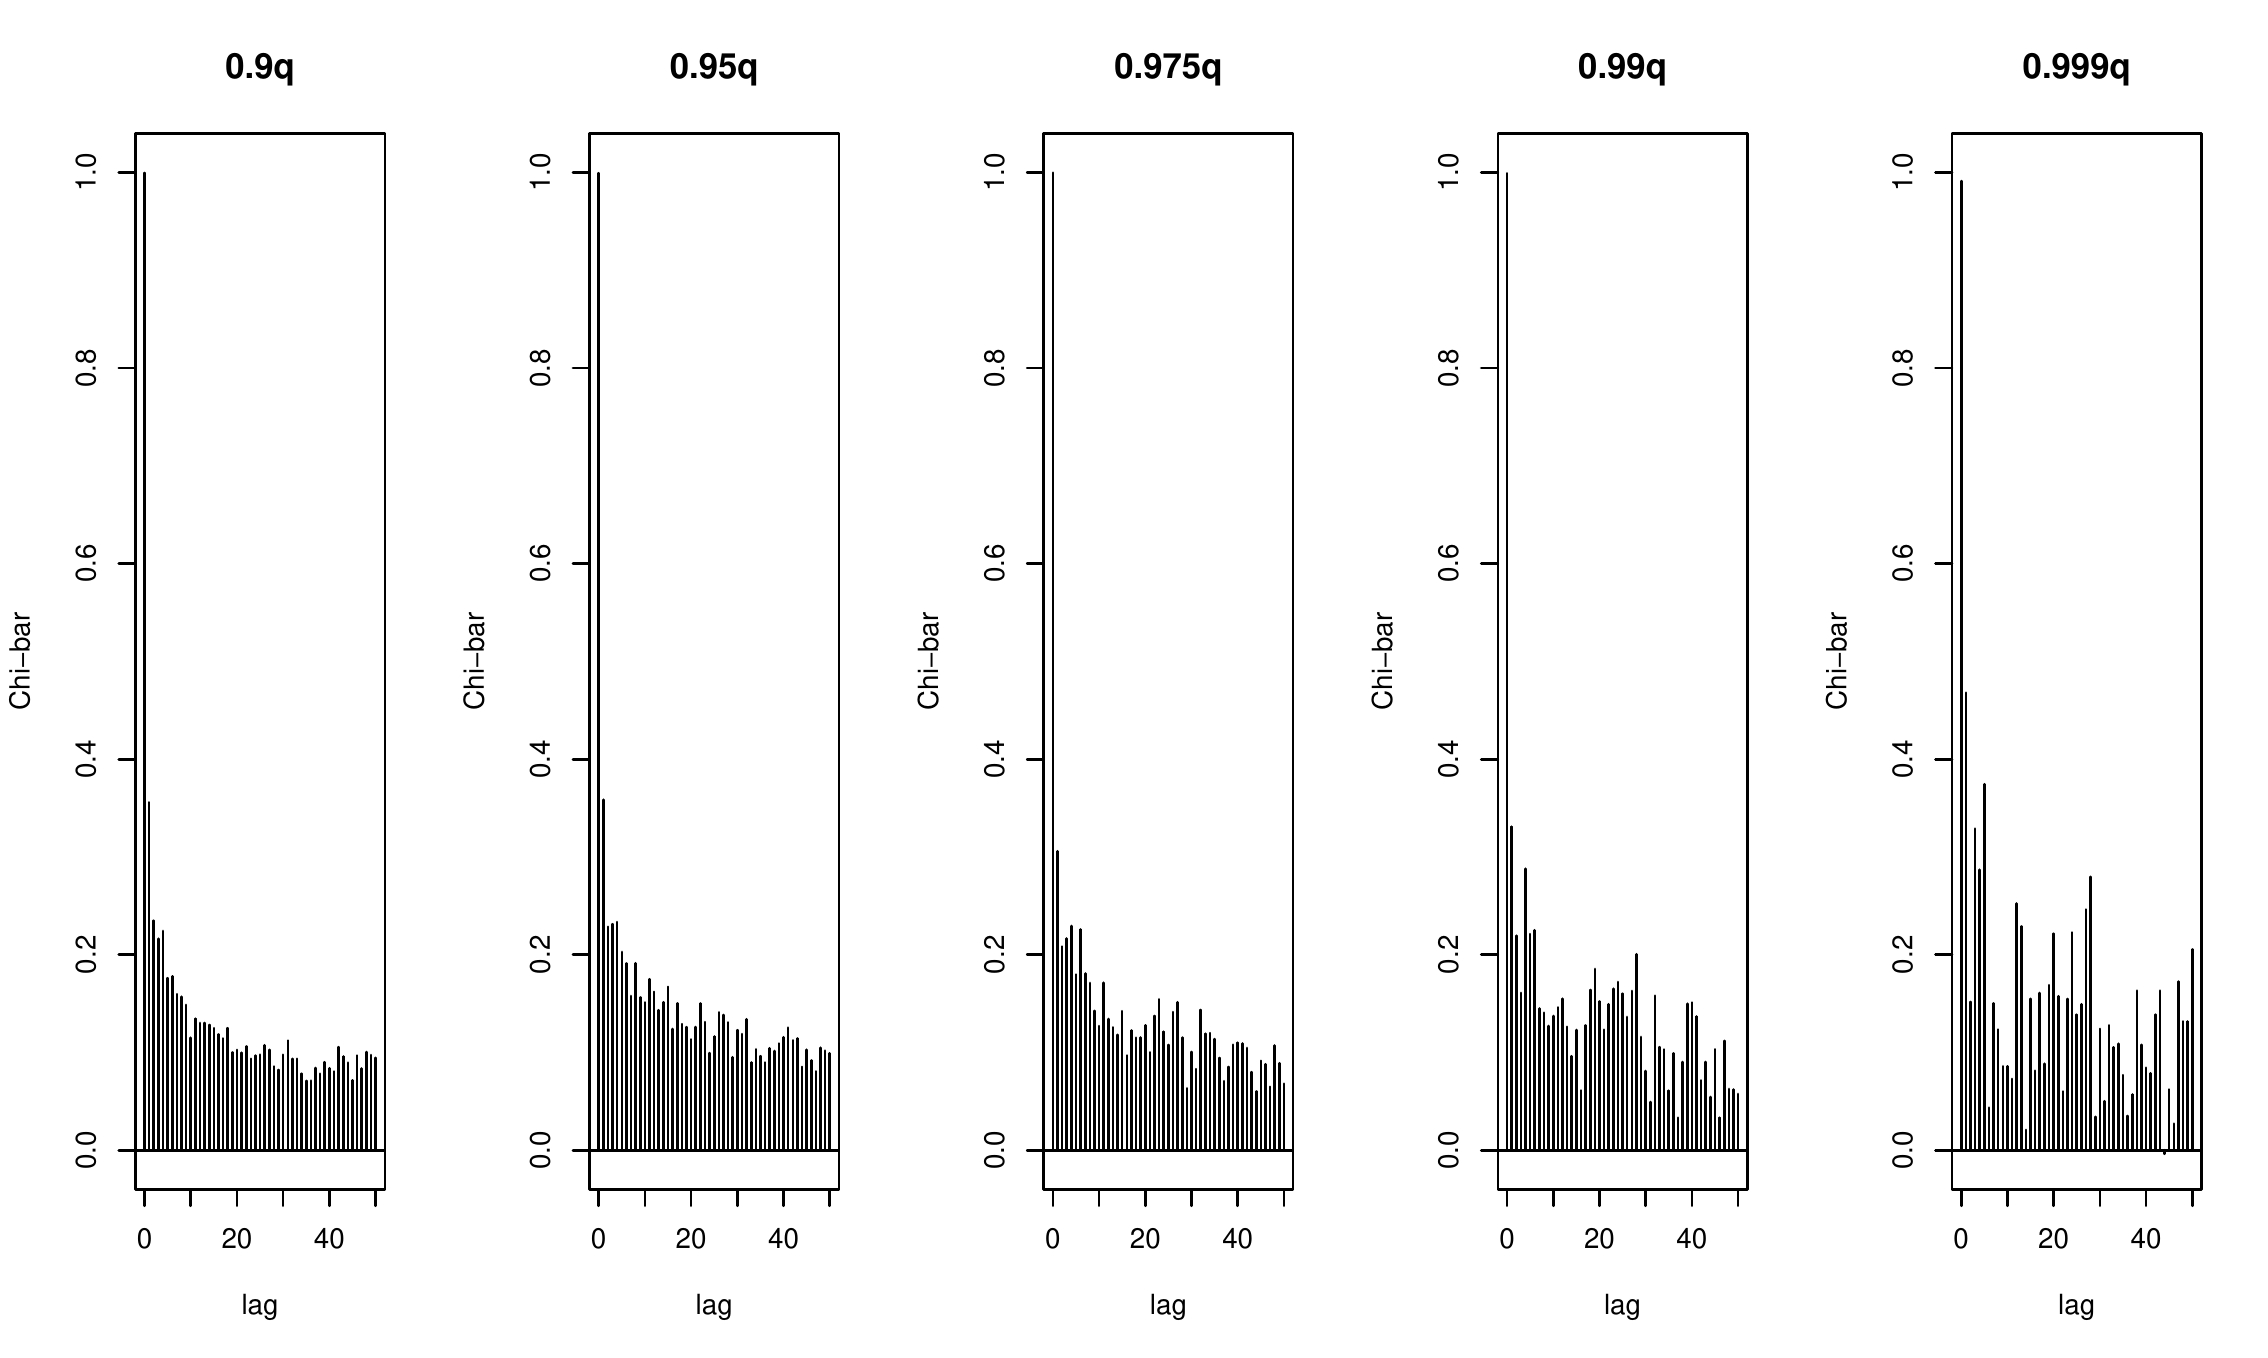}
    \caption{$\bar\chi$ for Heysham, Lowestoft, Newlyn and Sheerness (from top to bottom) for exceedances of the 0.9, 0.95, 0.975, 0.99 and 0.999 quantiles for various lags.}
    \label{fig::chibar}
\end{figure}

%\subsection{Modelling the Exceedance Probability with Tide and Day}

\begin{figure}[h]
    \centering
    \includegraphics[width=0.49\textwidth]{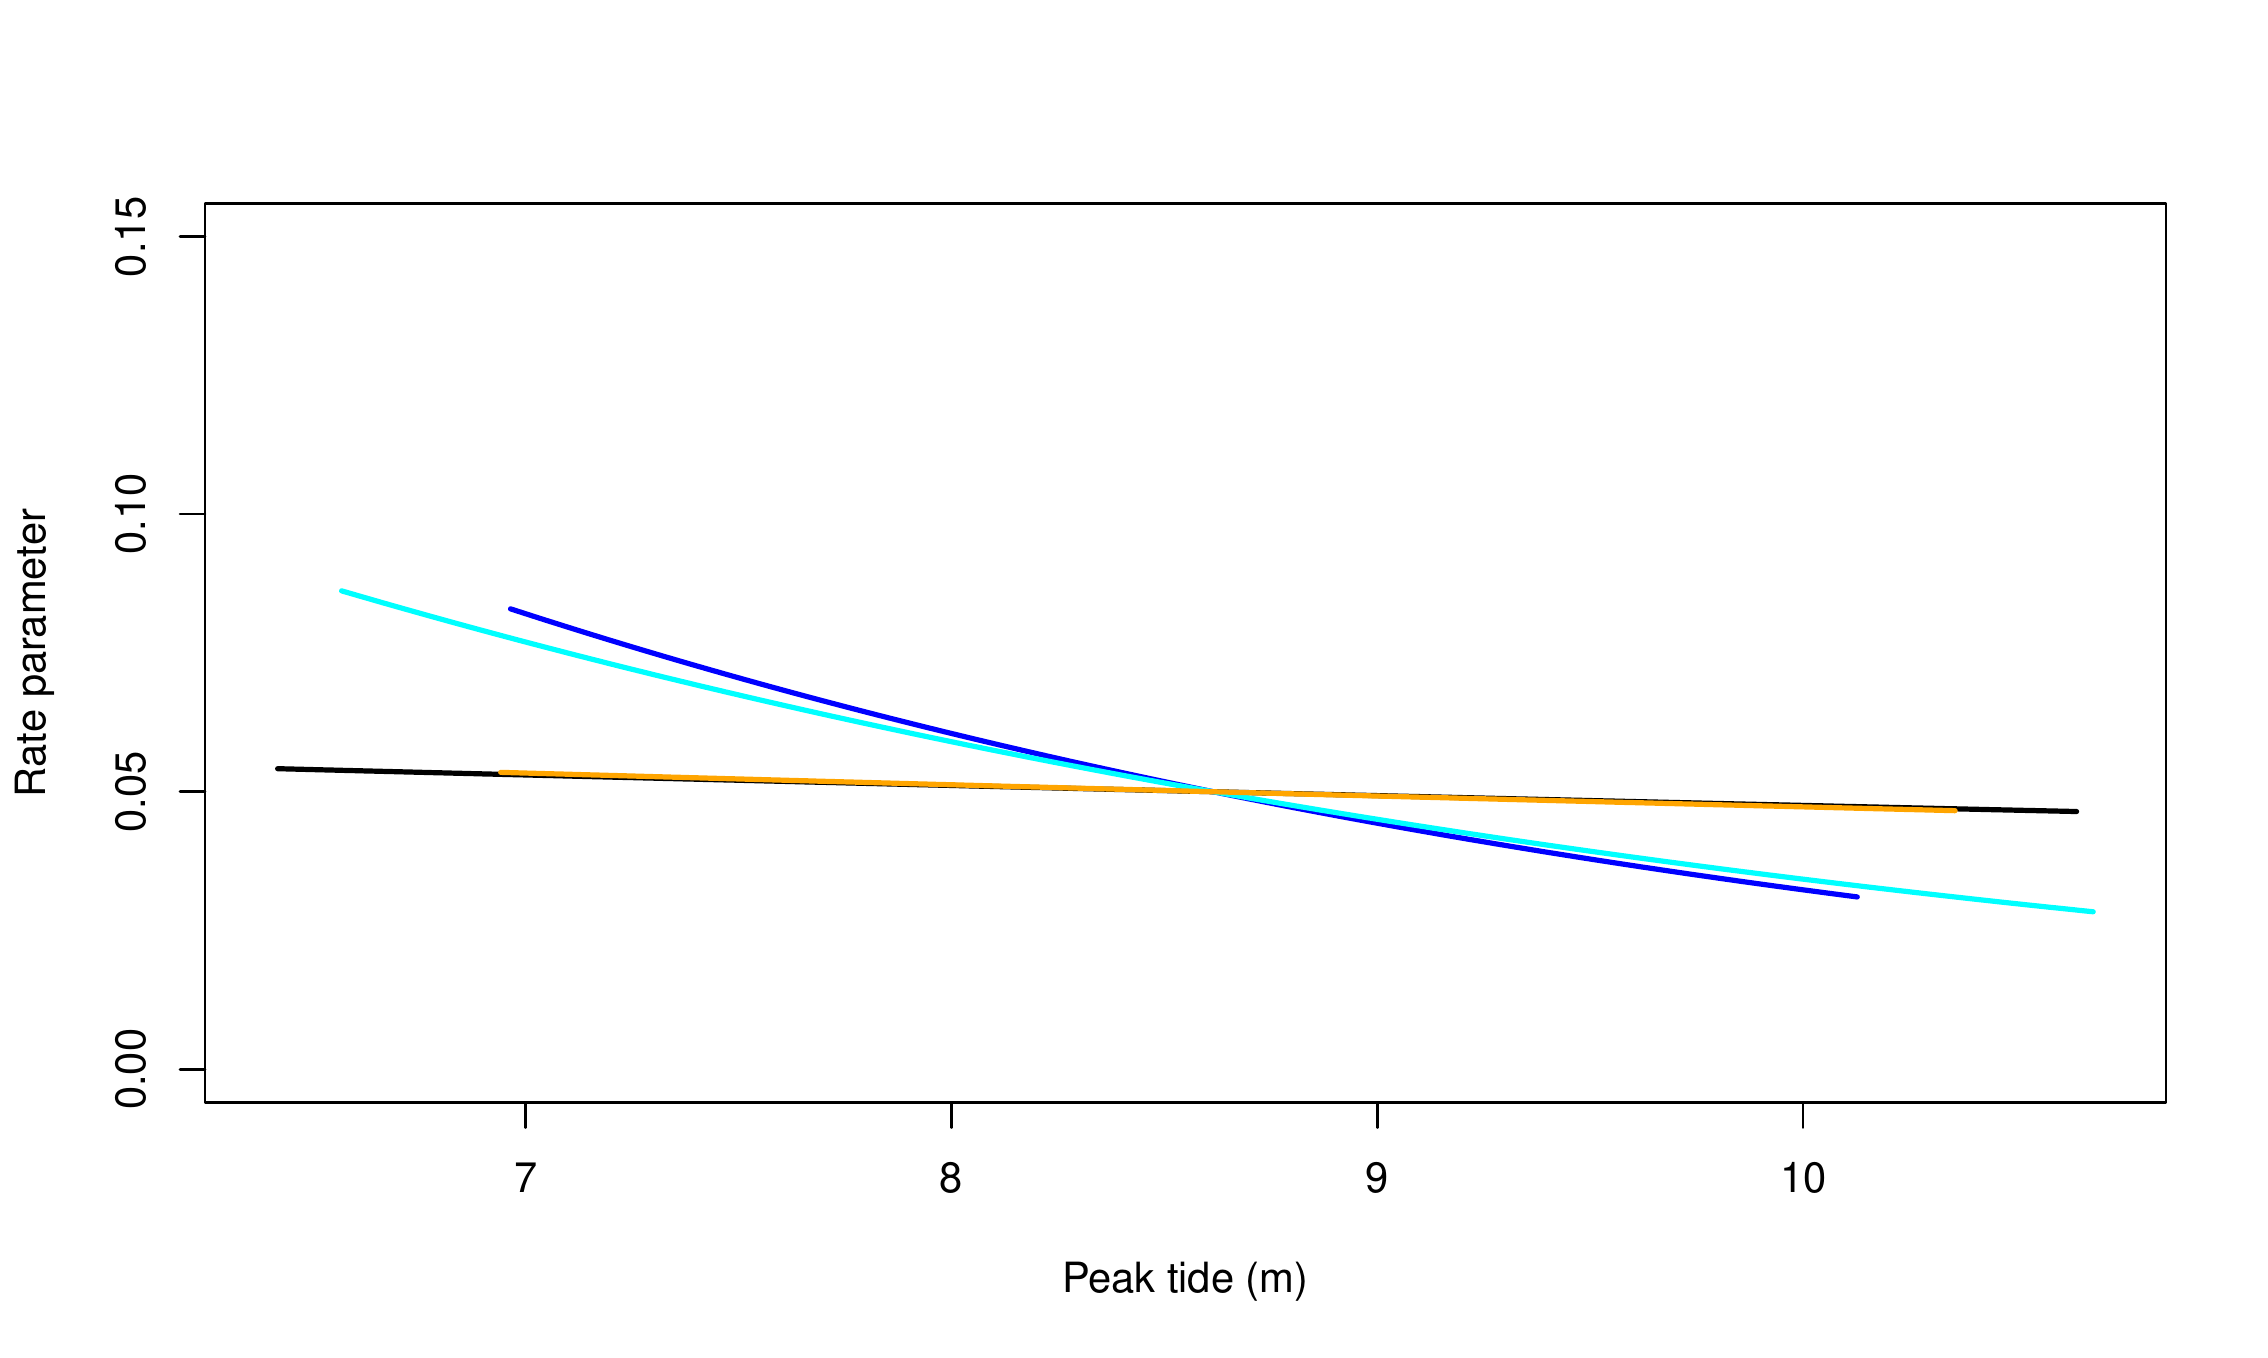}
    \includegraphics[width=0.49\textwidth]{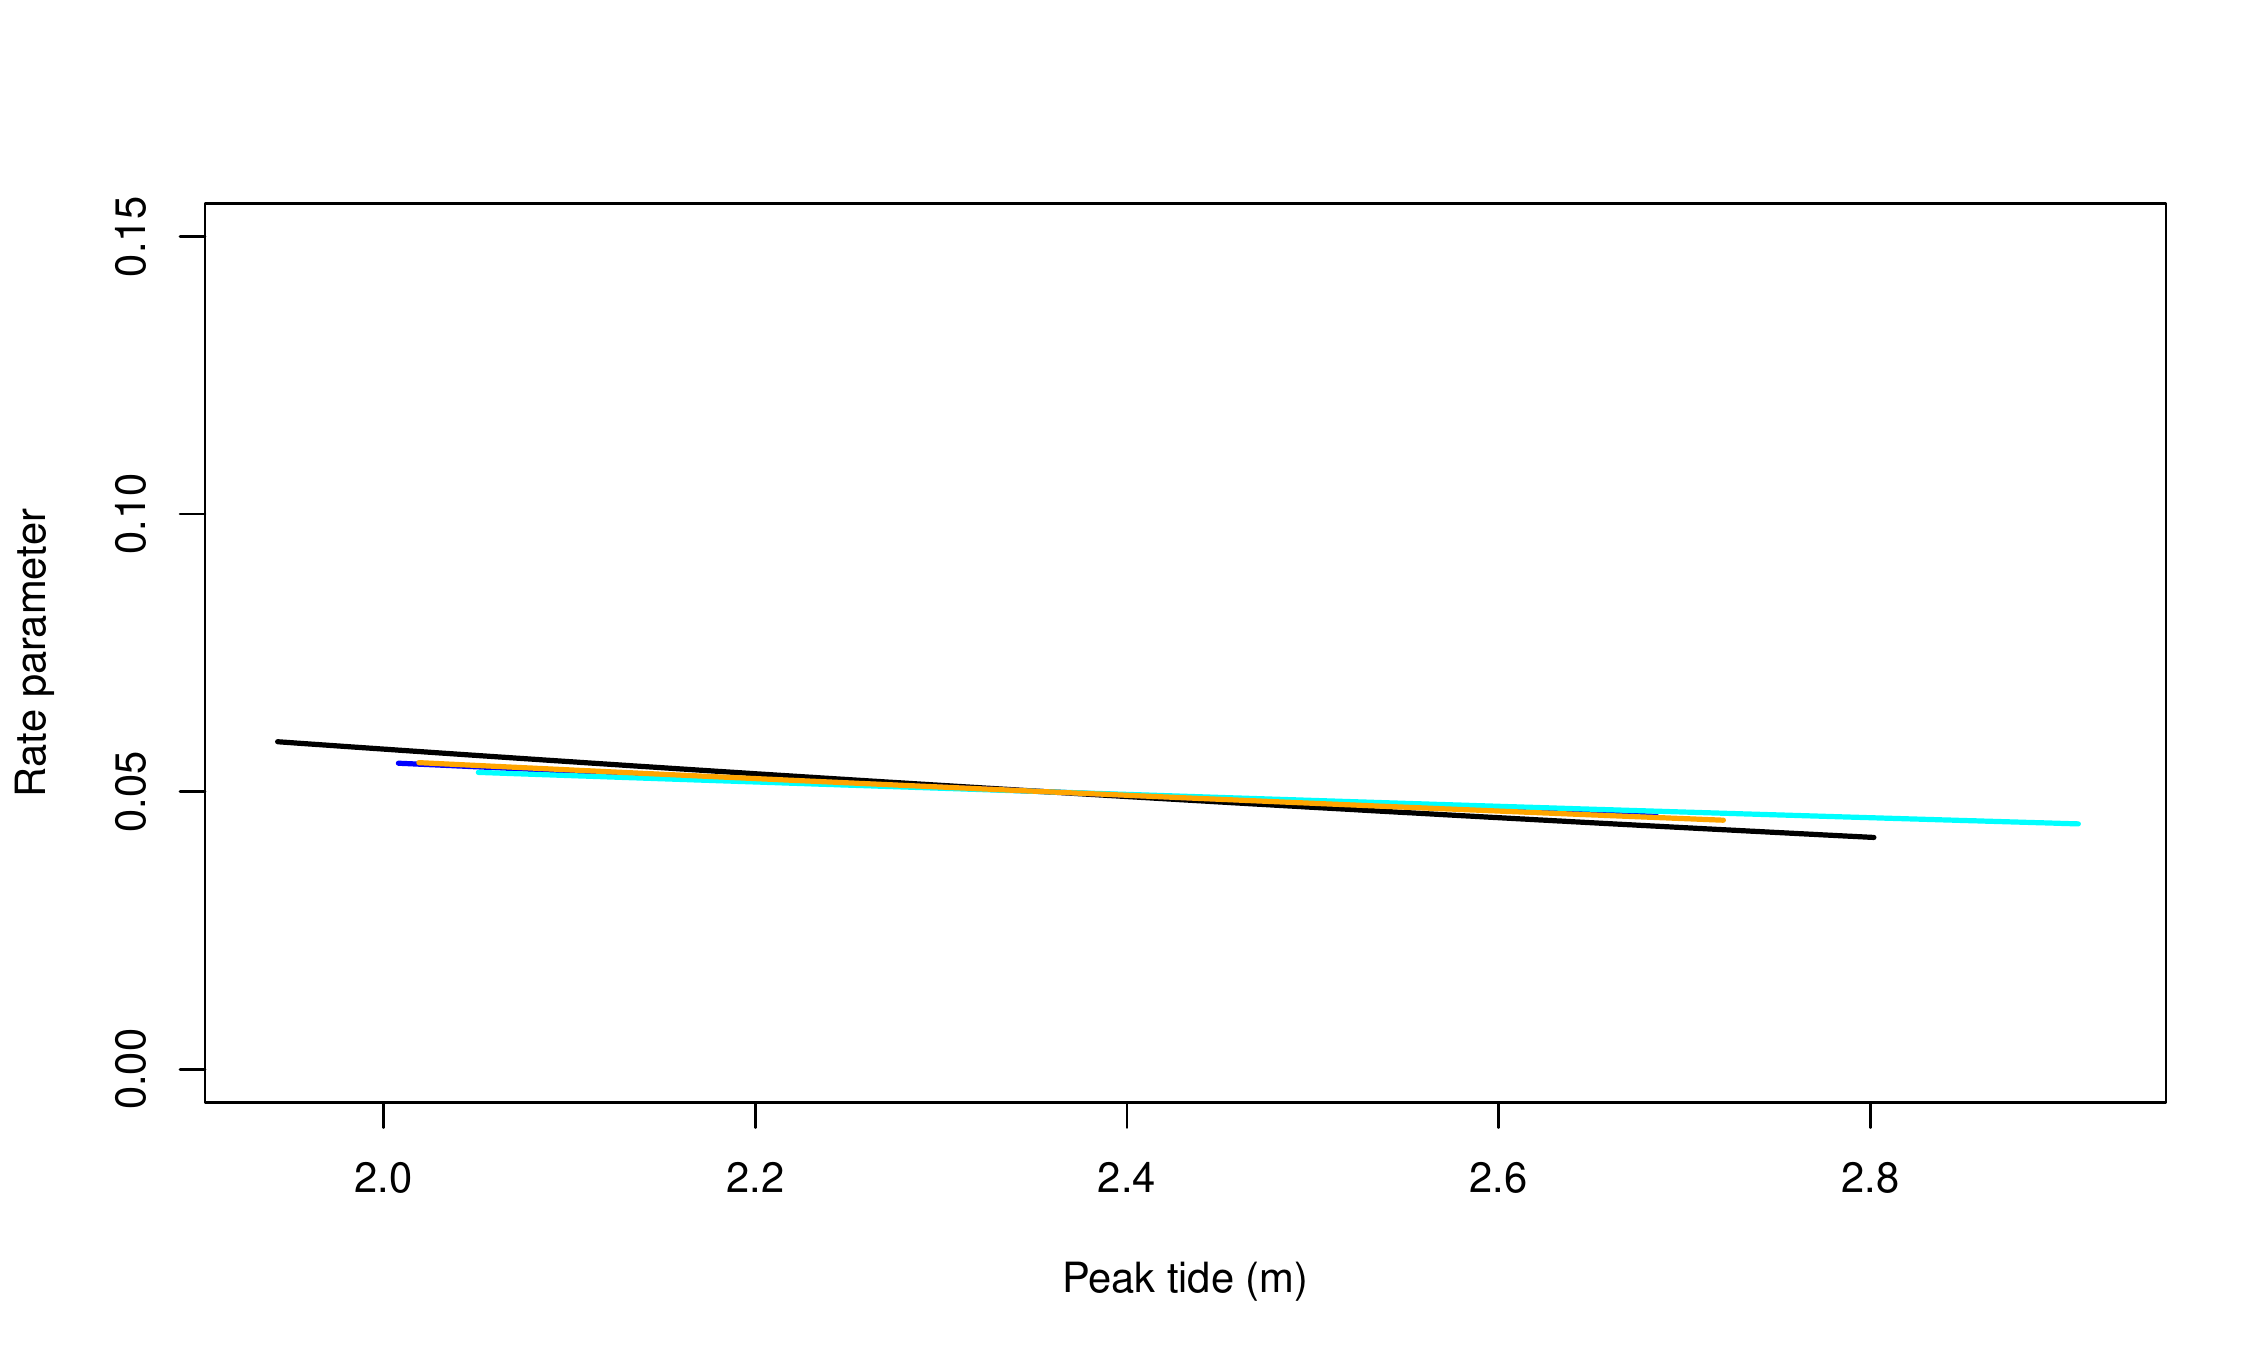}
    \includegraphics[width=0.49\textwidth]{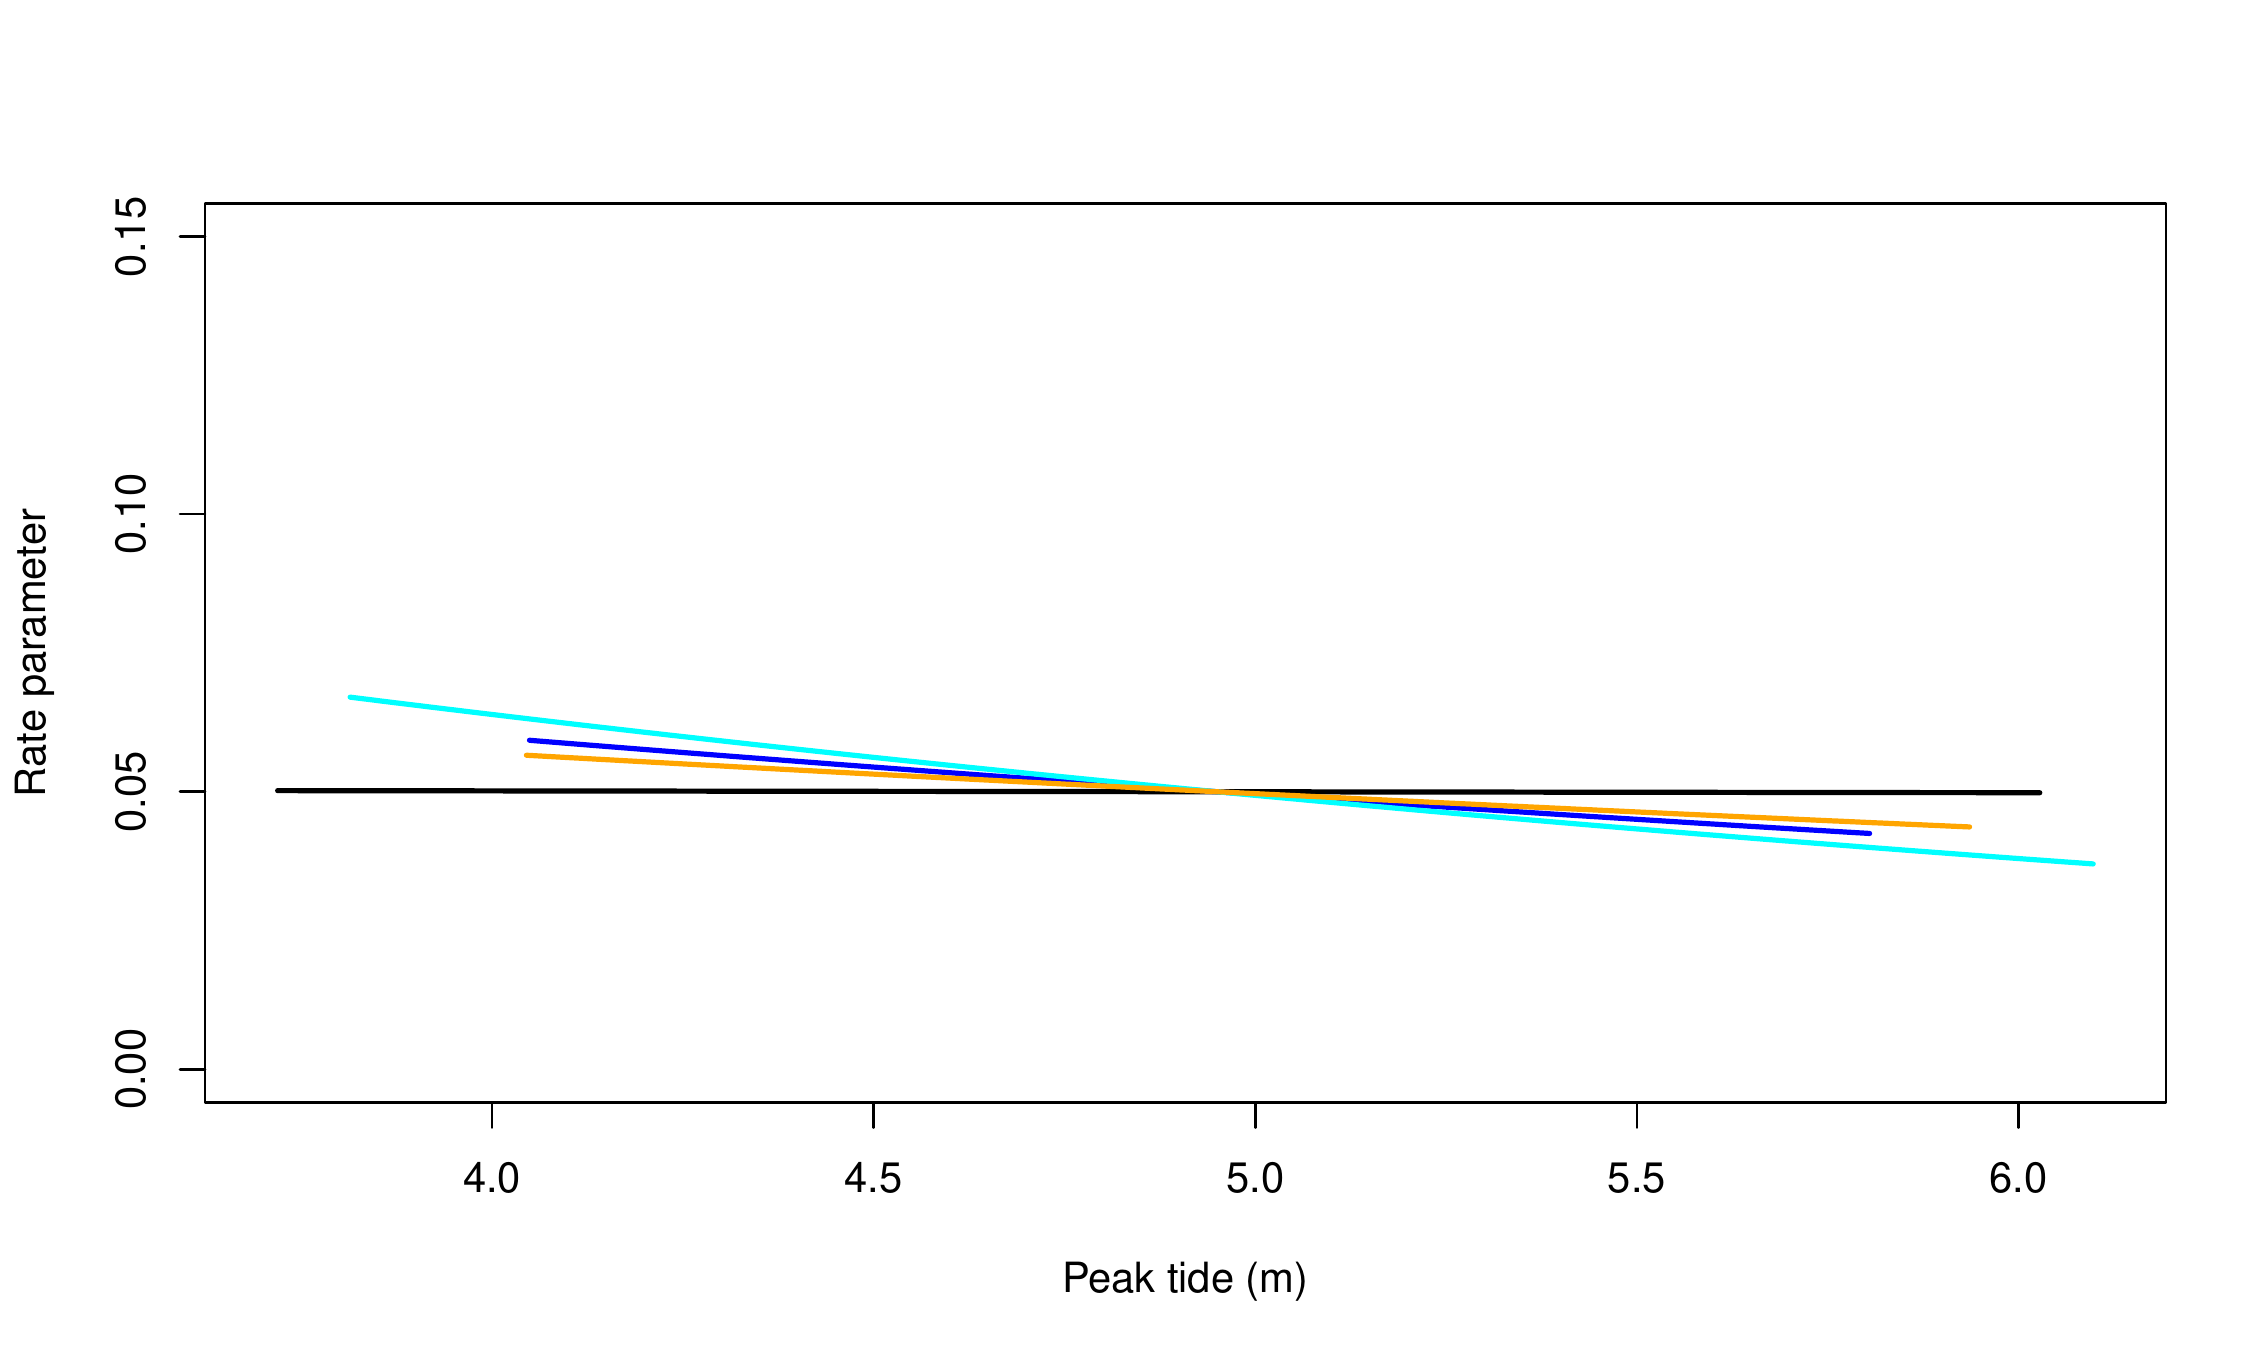}        \includegraphics[width=0.49\textwidth]{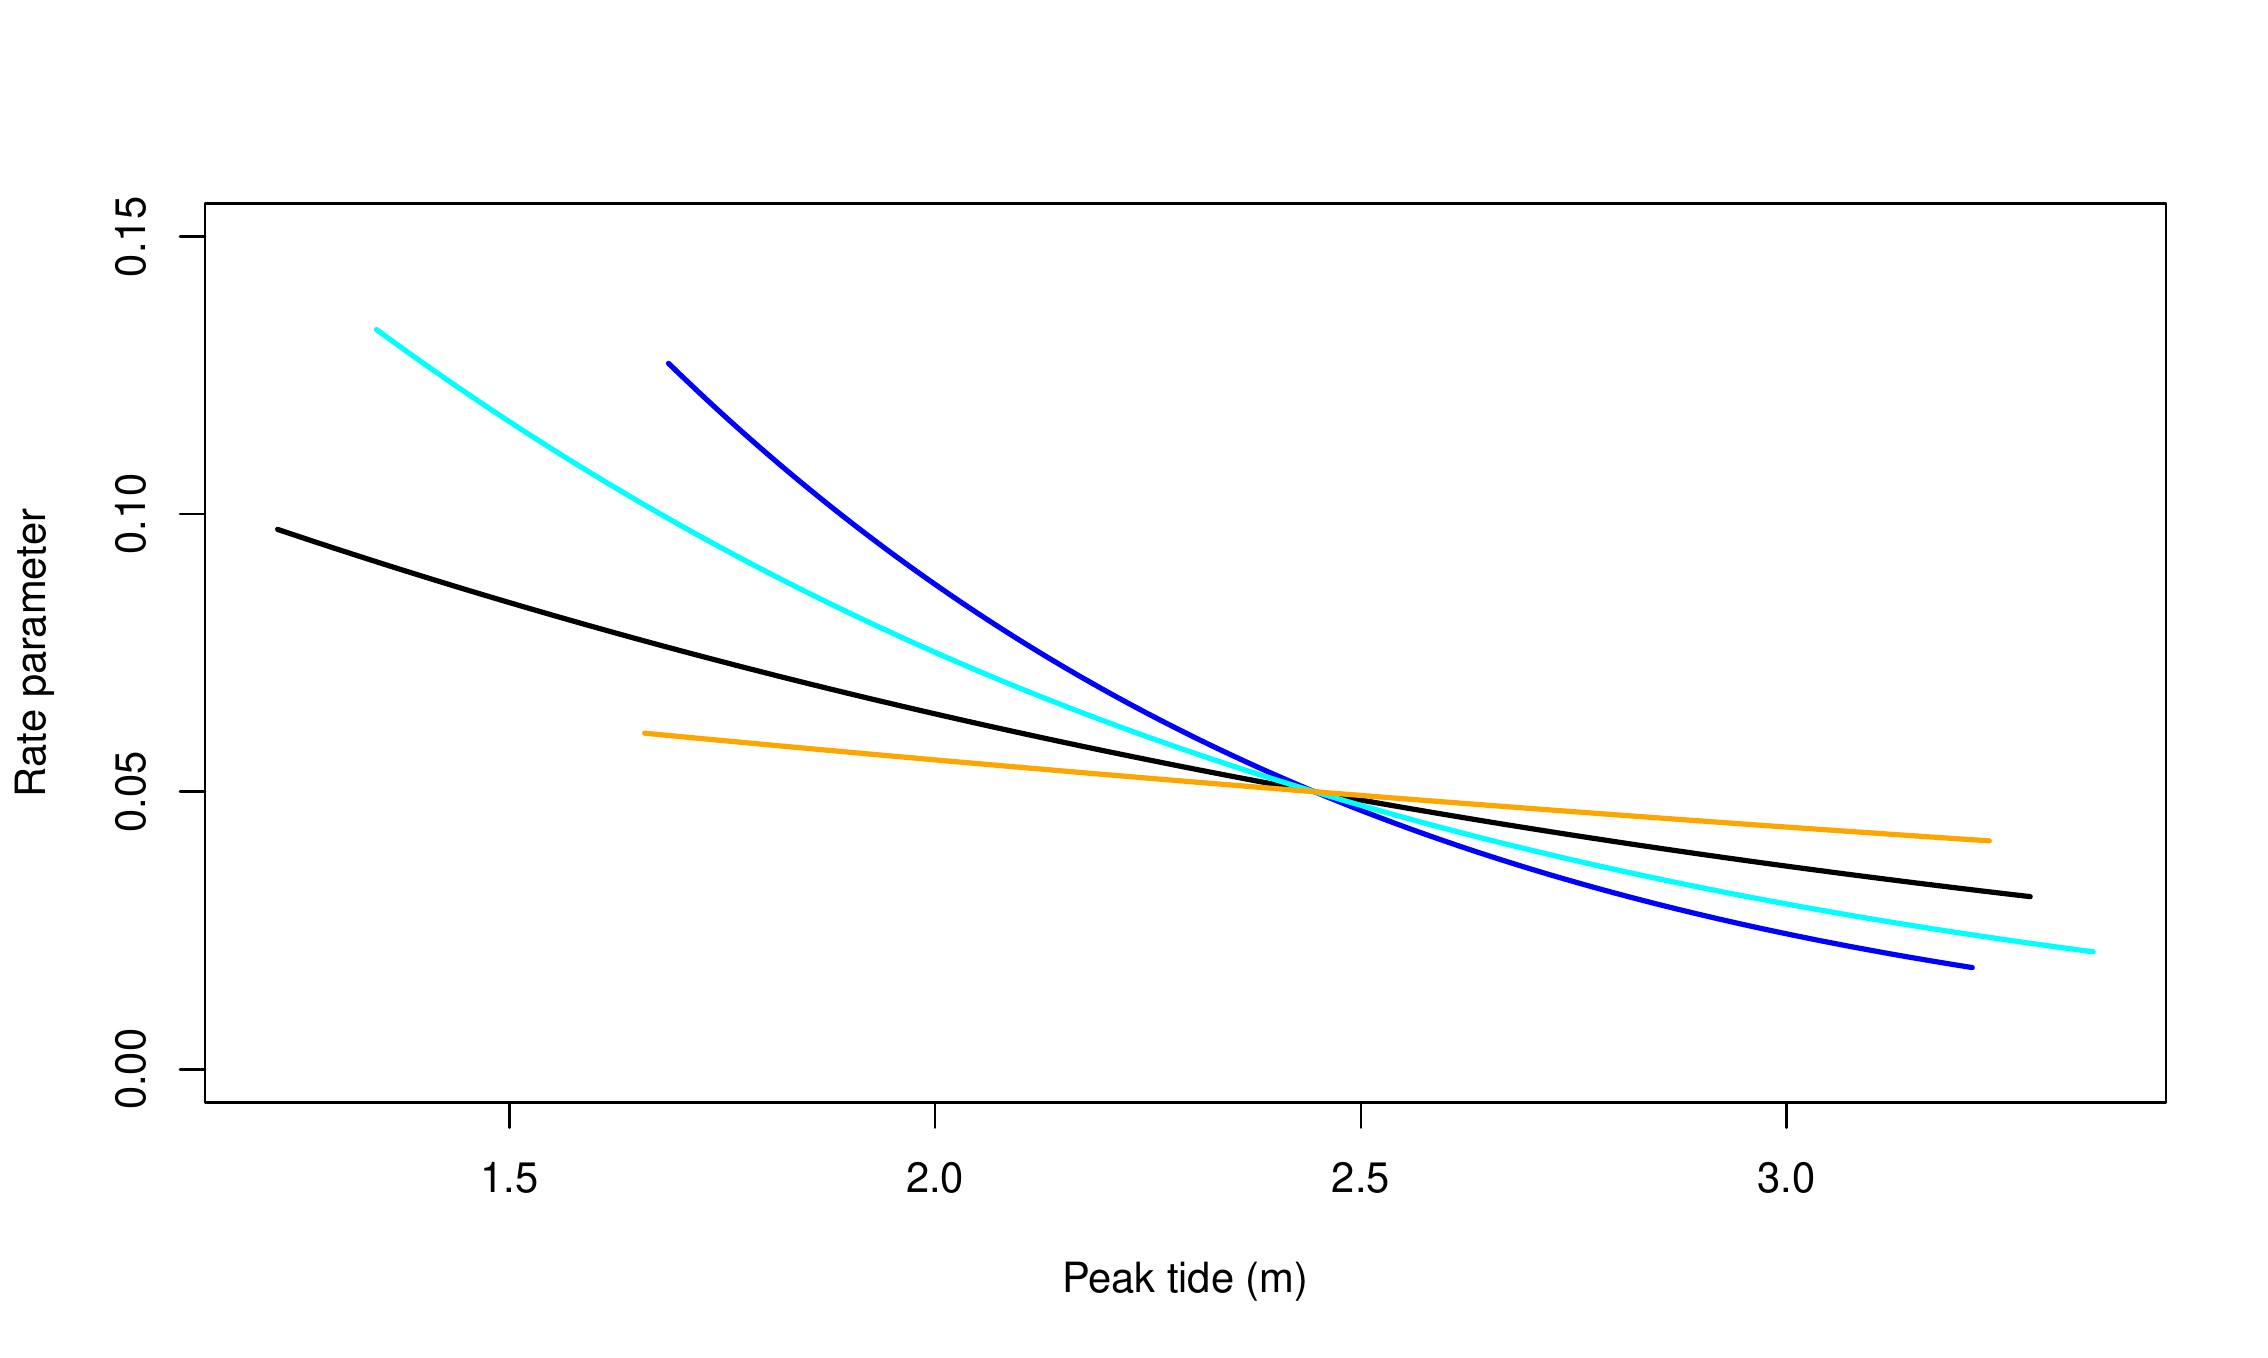}
    \caption{Estimated trend in exceedance probability per month with respect to peak tide and day, averaged over day at Heysham (top left), Lowestoft (top right), Newlyn (bottom left) and Sheerness (bottom right). Trends for March (blue), June (black), September (cyan) and December (orange) are shown here.}
    \label{fig::exprobtide_av_all}
\end{figure}

\begin{figure}[h]
    \centering
    \includegraphics[width=0.75\textwidth]{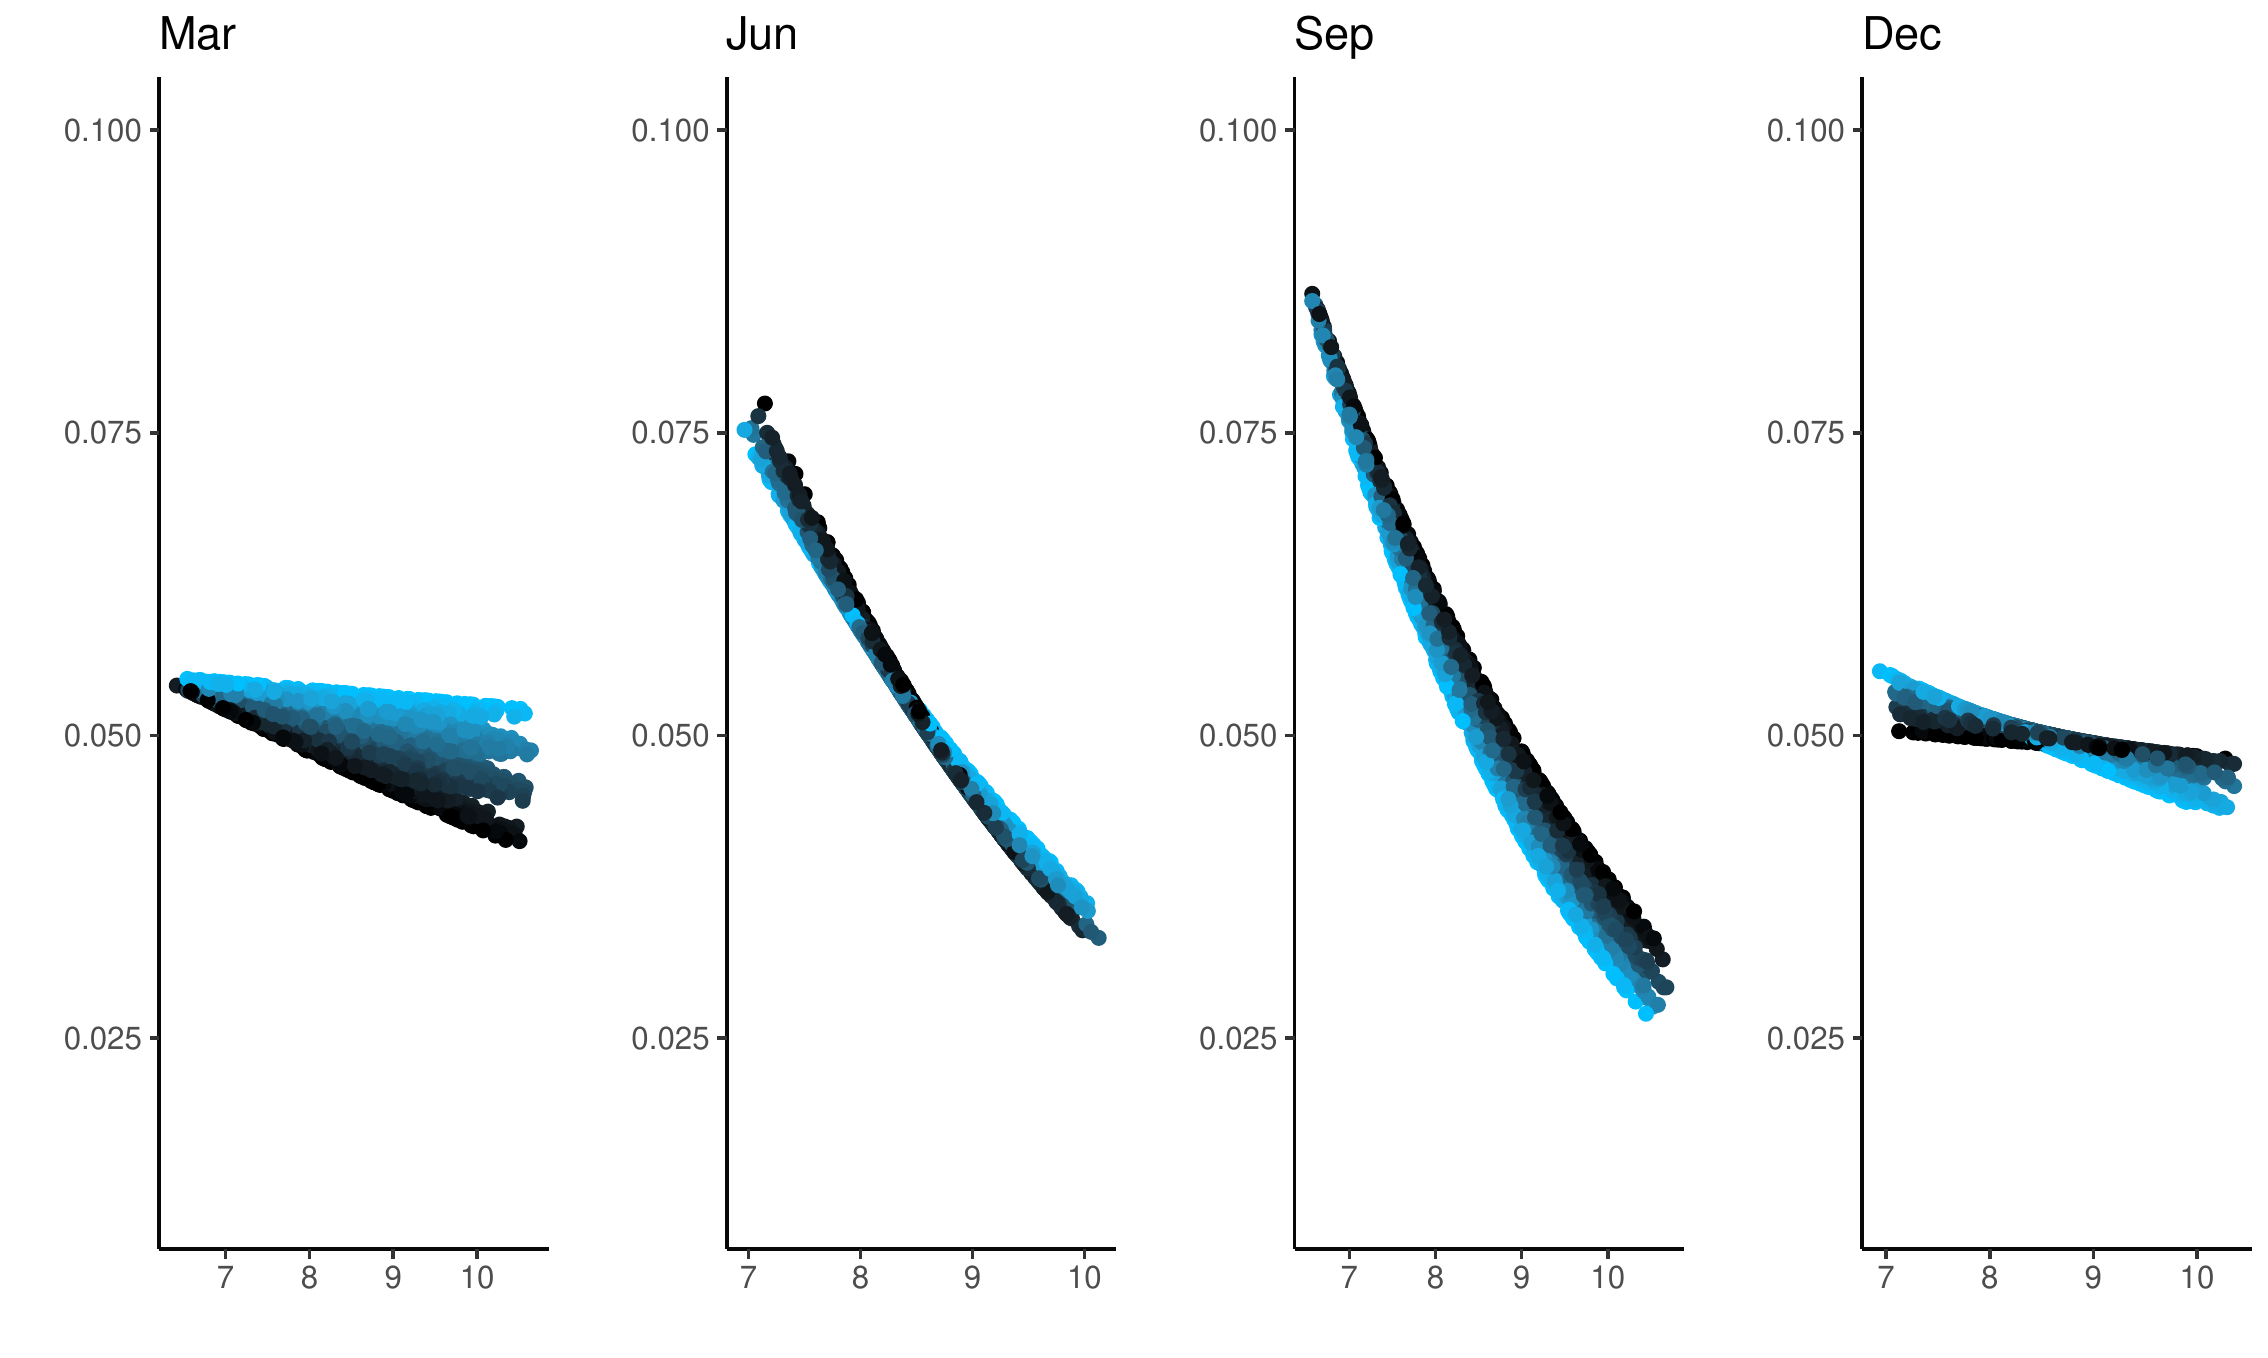}
    \includegraphics[width=0.75\textwidth]{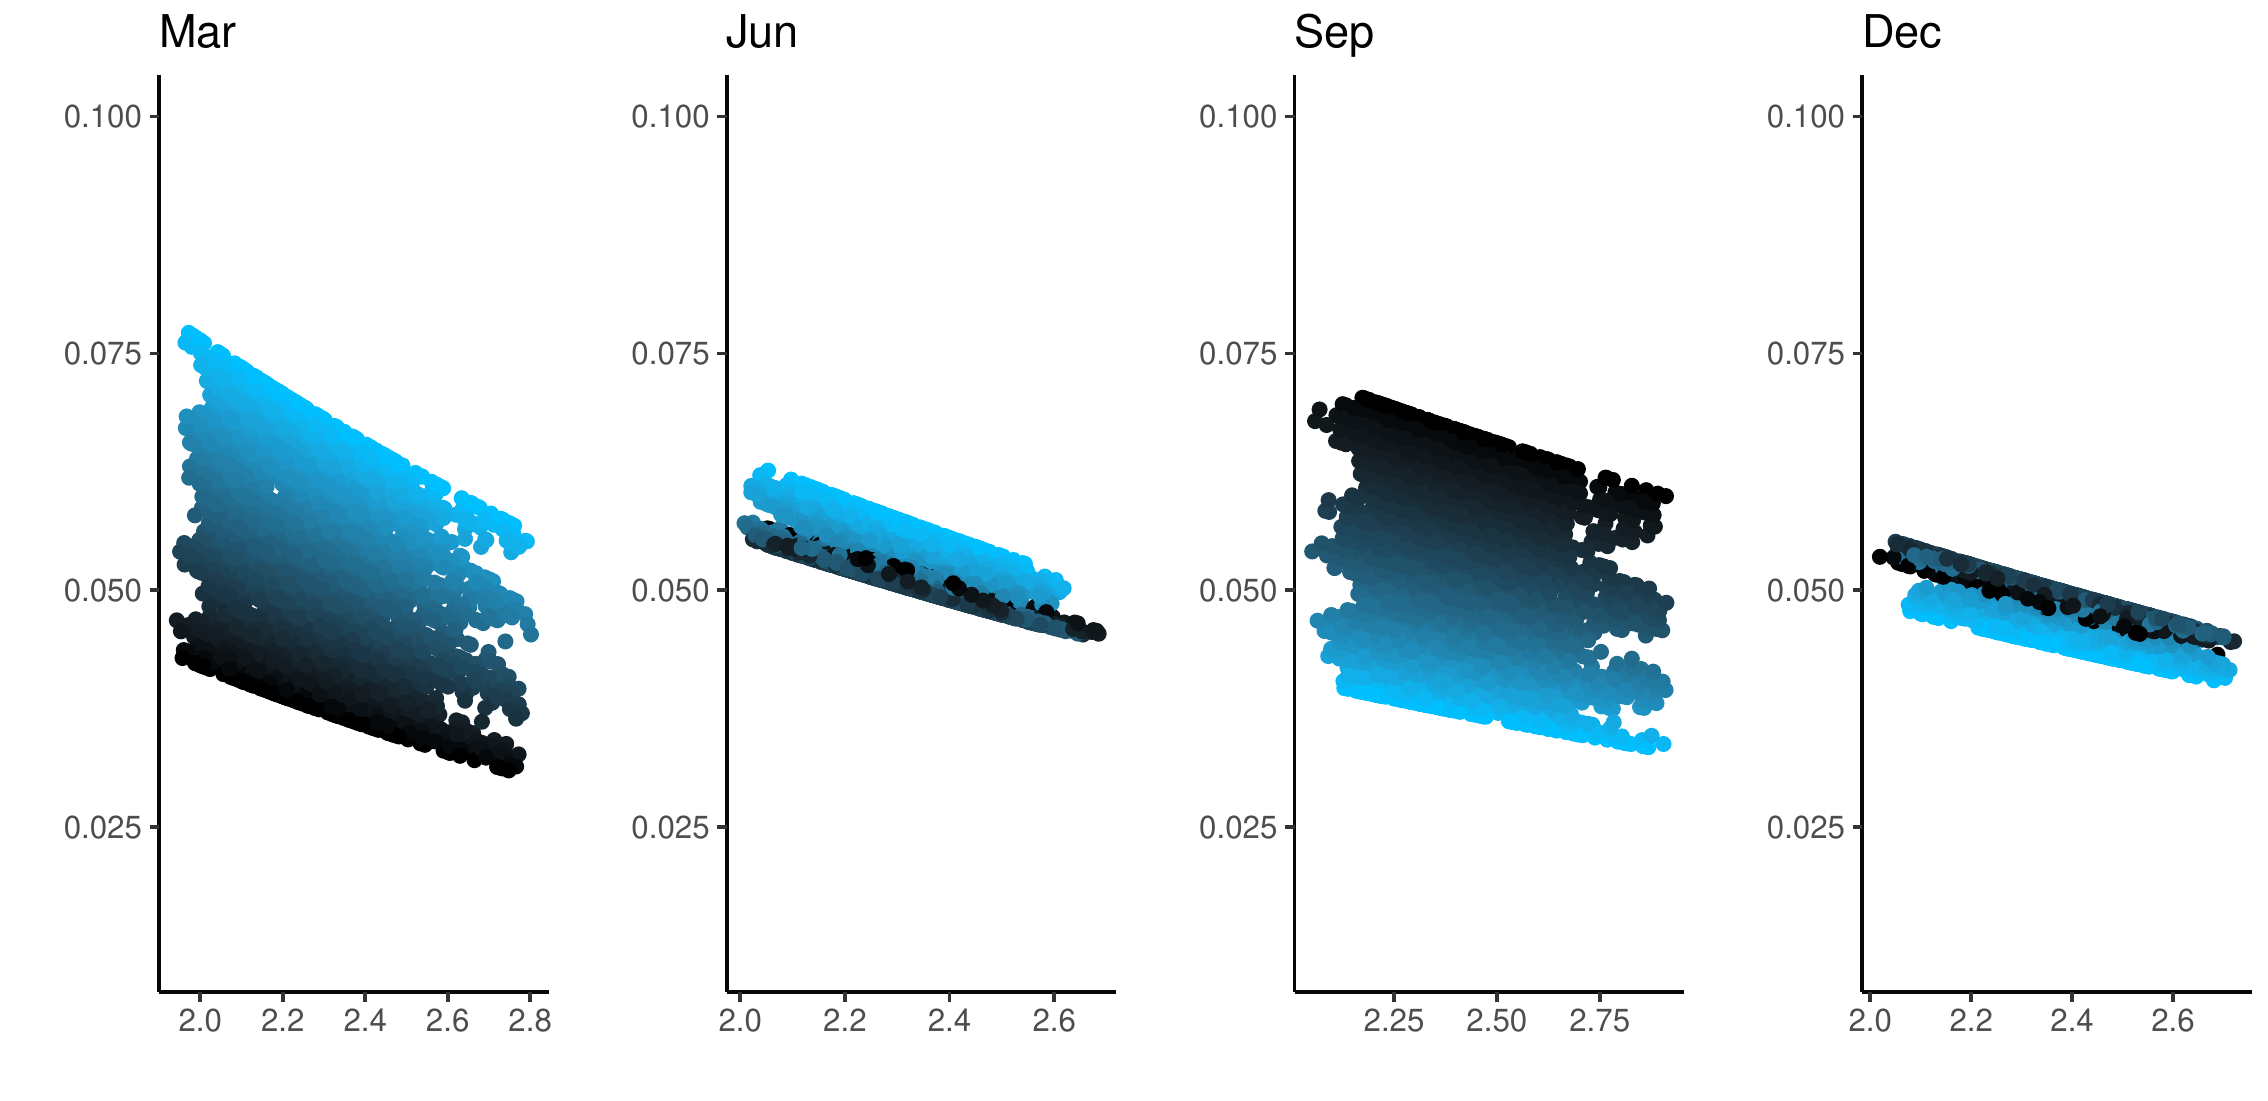}
    \includegraphics[width=0.75\textwidth]{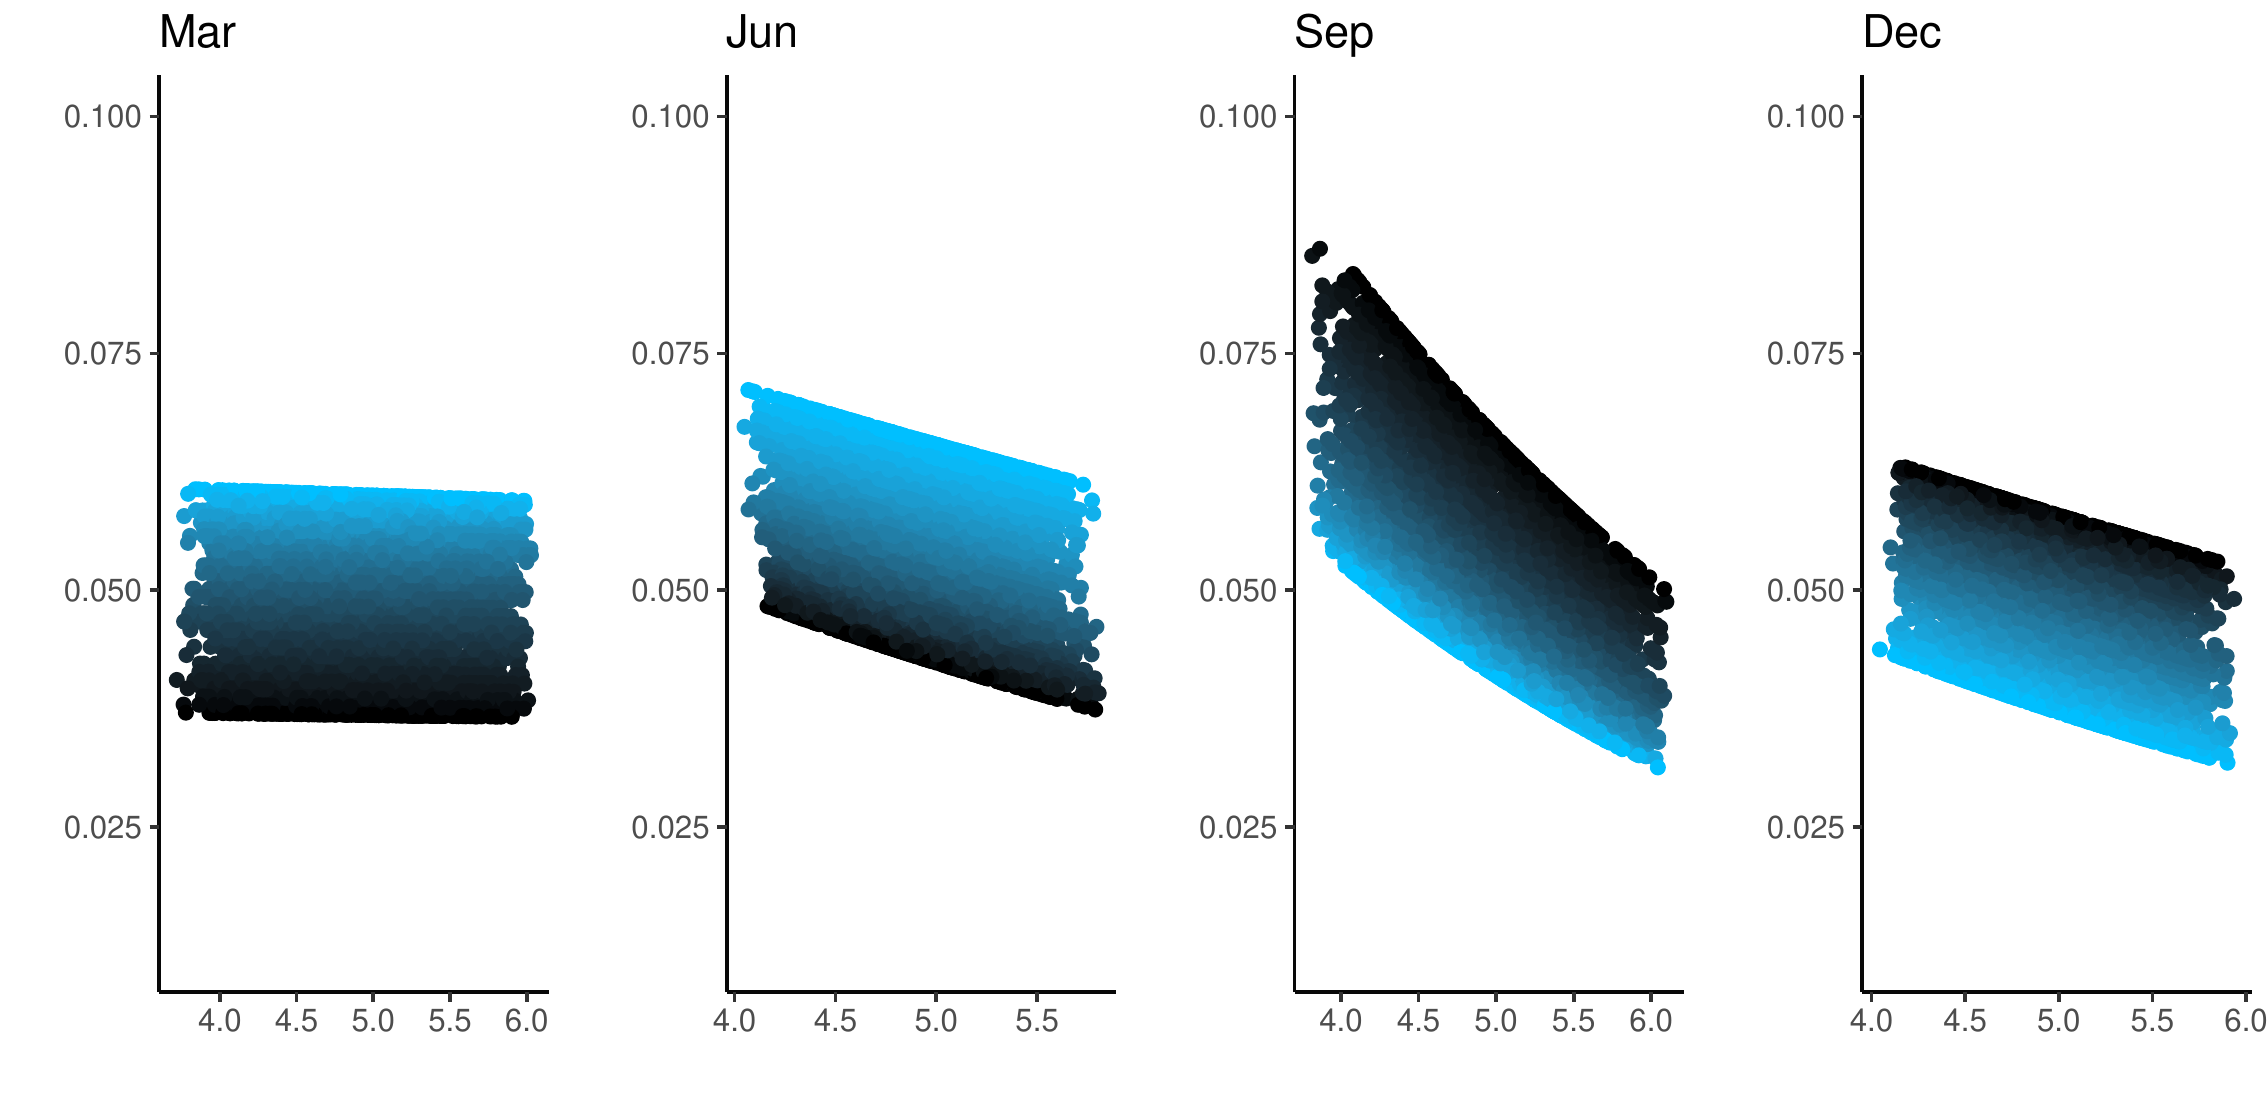}
    \caption{Estimated trend in exceedance probability per month with respect to peak tide and day at Heysham (top), Lowestoft (middle) and Newlyn (bottom). Darker points represent days later in the month, whilst lighter point represent days early in the month.}
    \label{fig::exprobtide_MJSD_all}
\end{figure}

%\subsection{Return Level Estimates}\label{extra_RLs}
%Here we show the return level estimates, monthly and annually, for all four scenarios listed in Section \ref{RLs}.

%\begin{figure}[h]
%    \centering
%    \includegraphics[width=0.9\textwidth]{HEY_monmax_3x4_4.pdf}
%    \caption{Monthly return level estimates at Heysham for the proposed method (cyan), the current method (purple), intermediate solution I (blue) and intermediate solution II (magenta), compared with empirical estimates (red). We also show the highest astronomical tidal level (black dashed line).}
%    \label{HEY_monmax_4}
%\end{figure}

%\begin{figure}
%    \centering
%    \includegraphics[width=0.9\textwidth]{LOW_monmax_3x4_4.pdf}
%    \caption{Monthly return level estimates at Lowestoft for the proposed method (cyan), the current method (purple), intermediate solution I (blue) and intermediate solution II (magenta), compared with empirical estimates (red). We also show the highest astronomical tidal level (black dashed line).}
%    \label{LOW_monmax_4}
%\end{figure}

%\begin{figure}
%    \centering
%    \includegraphics[width=0.45\textwidth]{HEY_annmax_2.pdf}\includegraphics[width=0.45\textwidth]{LOW_annmax_4.pdf}
%    \caption{Annual return level estimates at Heysham (left) and Lowestoft (right) for the proposed method (cyan), the current method (purple), intermediate solution I (blue) and intermediate solution II (magenta), compared with empirical estimates (red). We also show the highest astronomical tidal level (black dashed line).}
%    \label{annmax_4}
%\end{figure}

\begin{figure}
    \centering
    \includegraphics[width=0.8\textwidth]{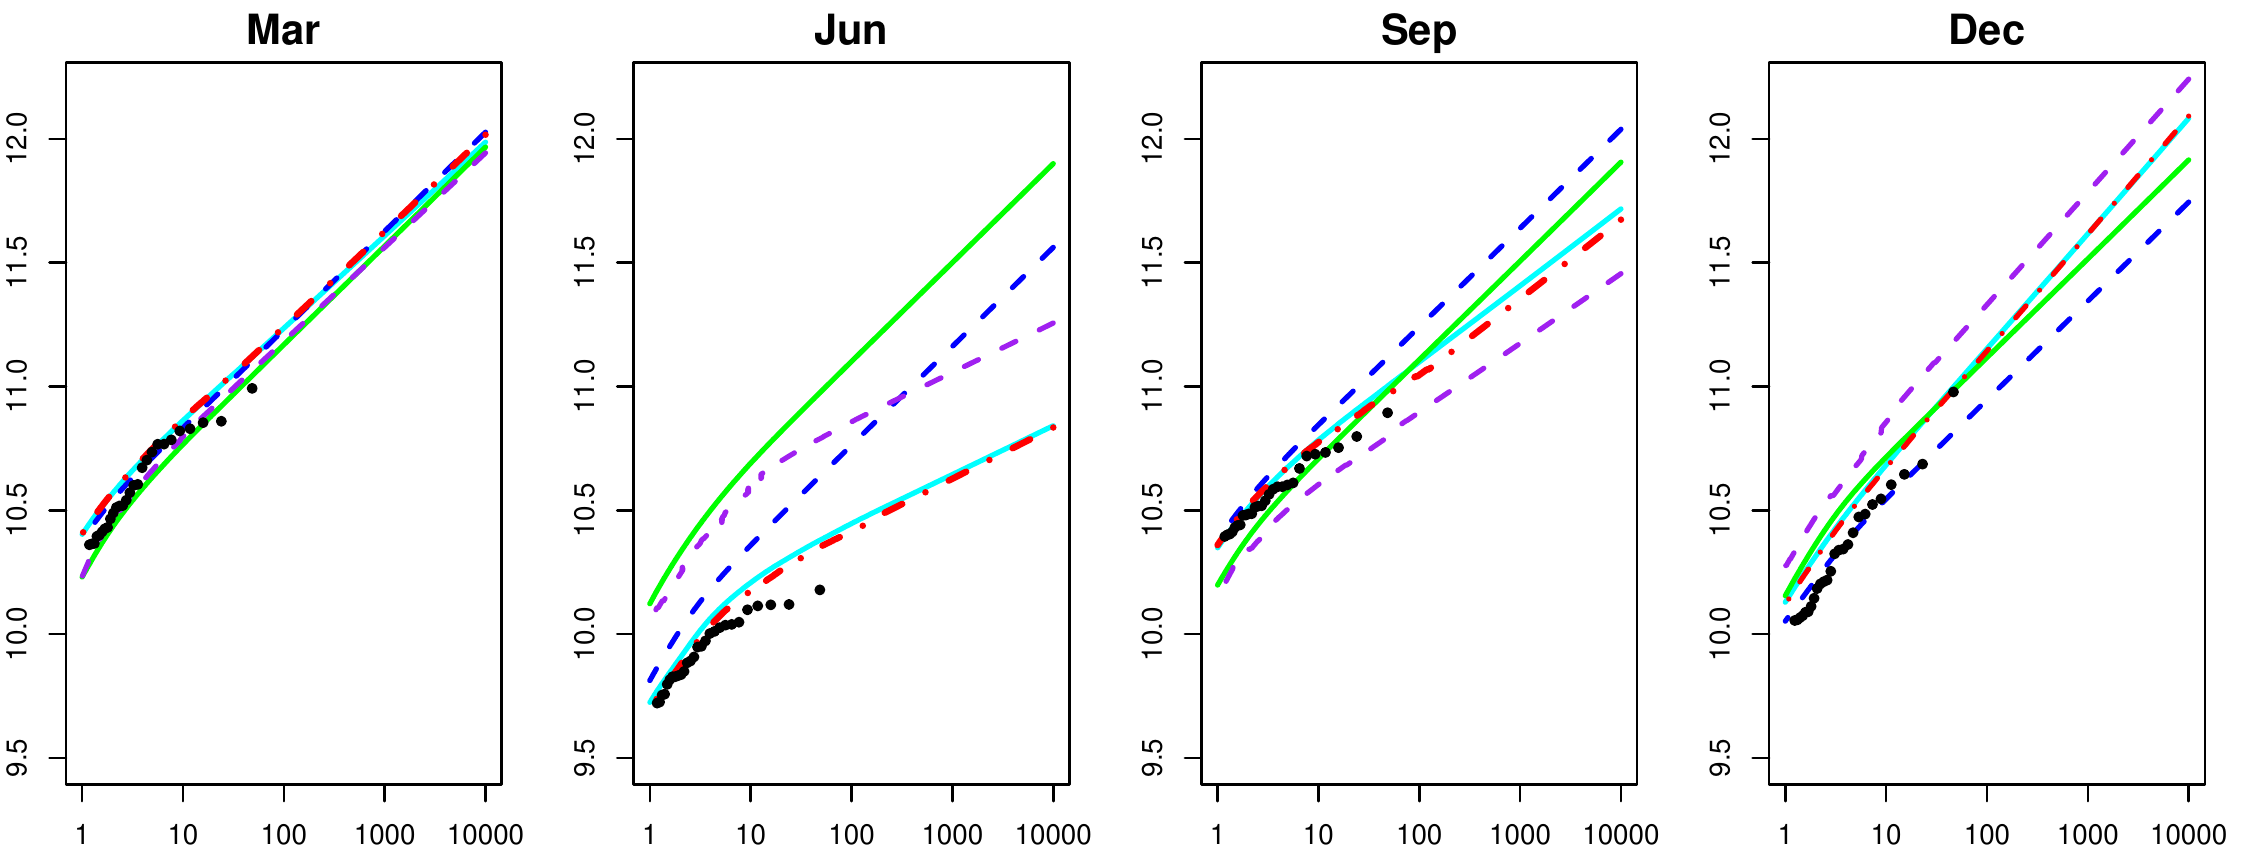} \\
    \includegraphics[width=0.8\textwidth]{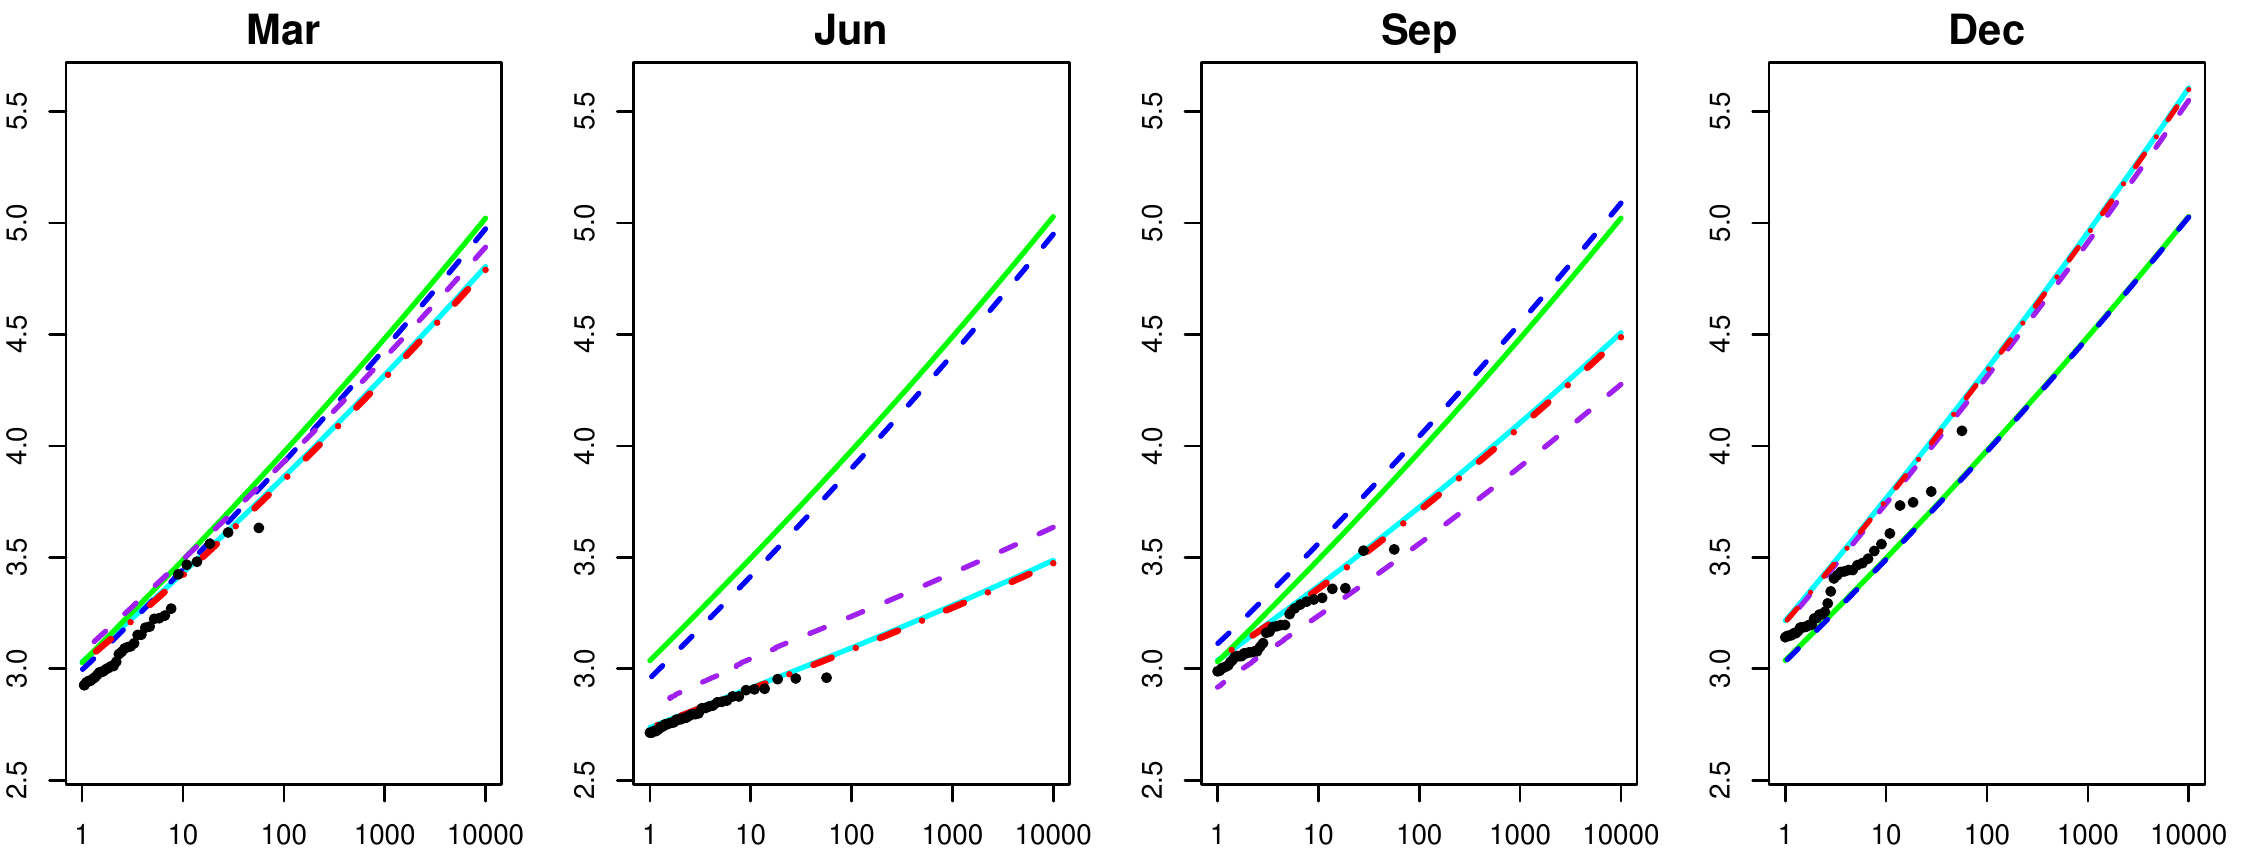} \\
    \includegraphics[width=0.8\textwidth]{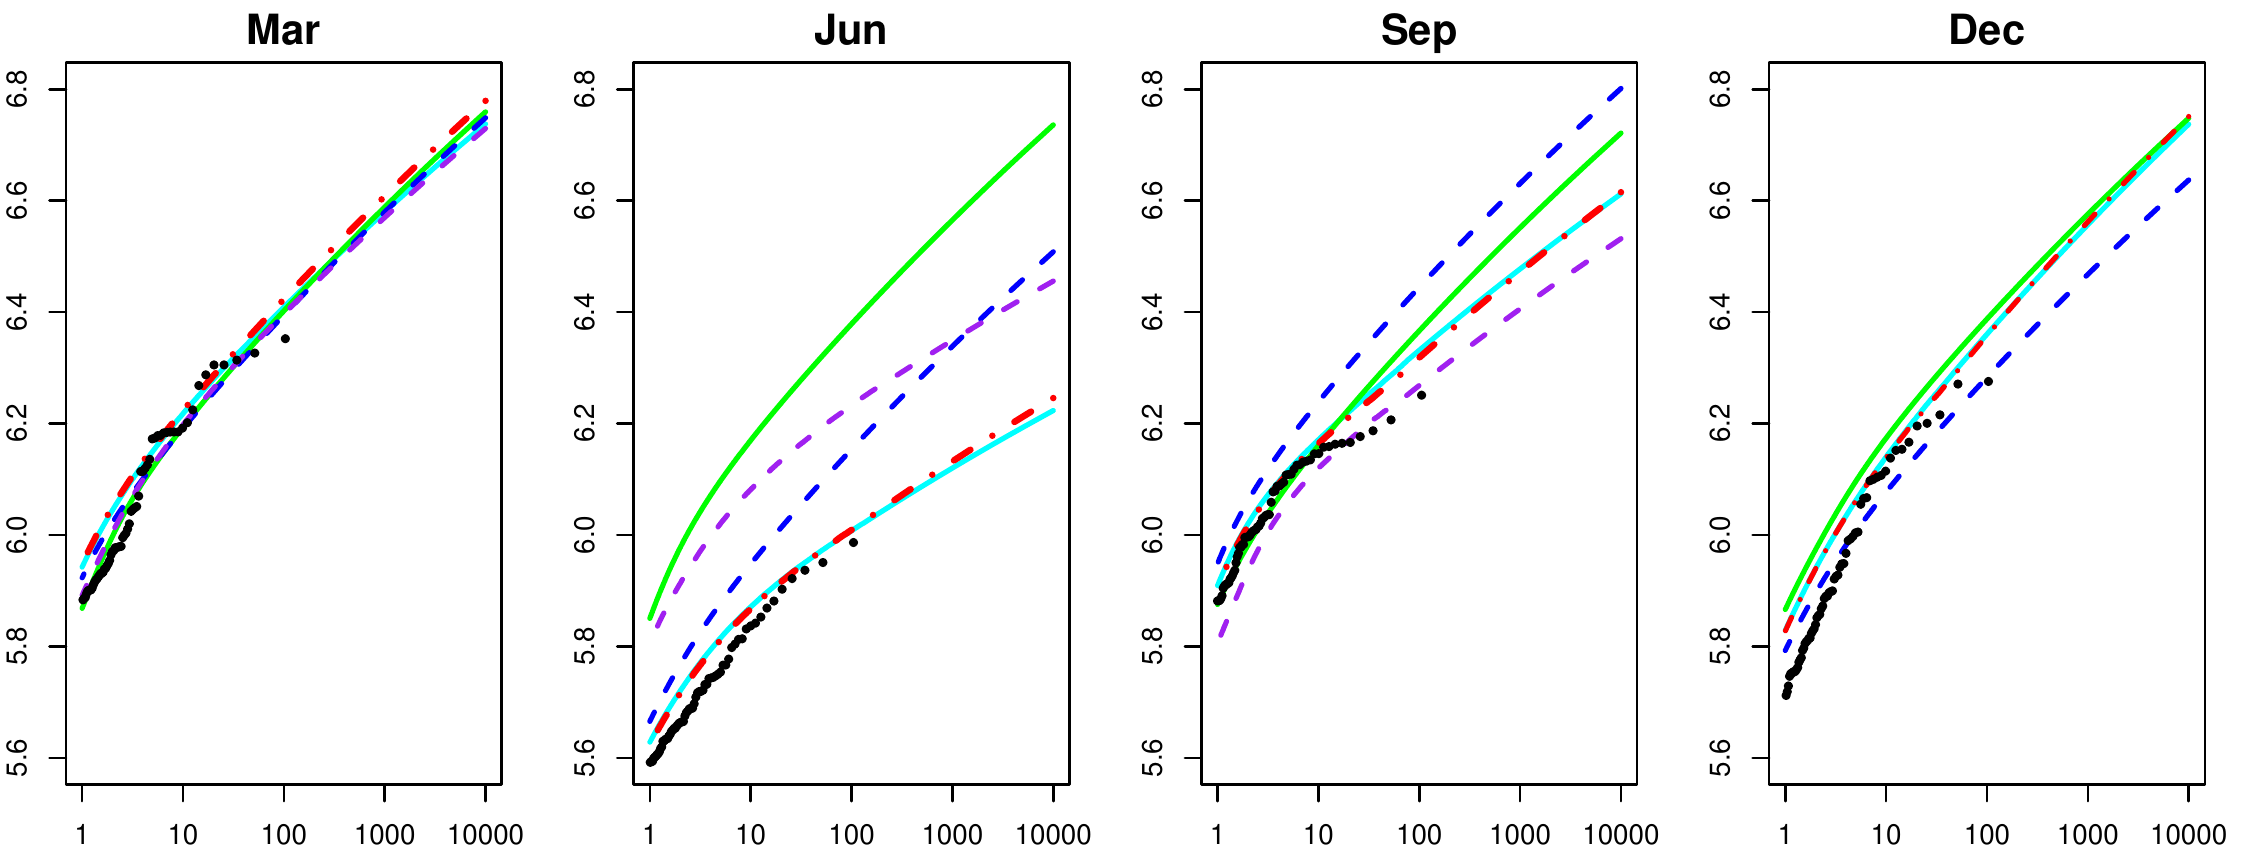} \\
    \includegraphics[width=0.8\textwidth]{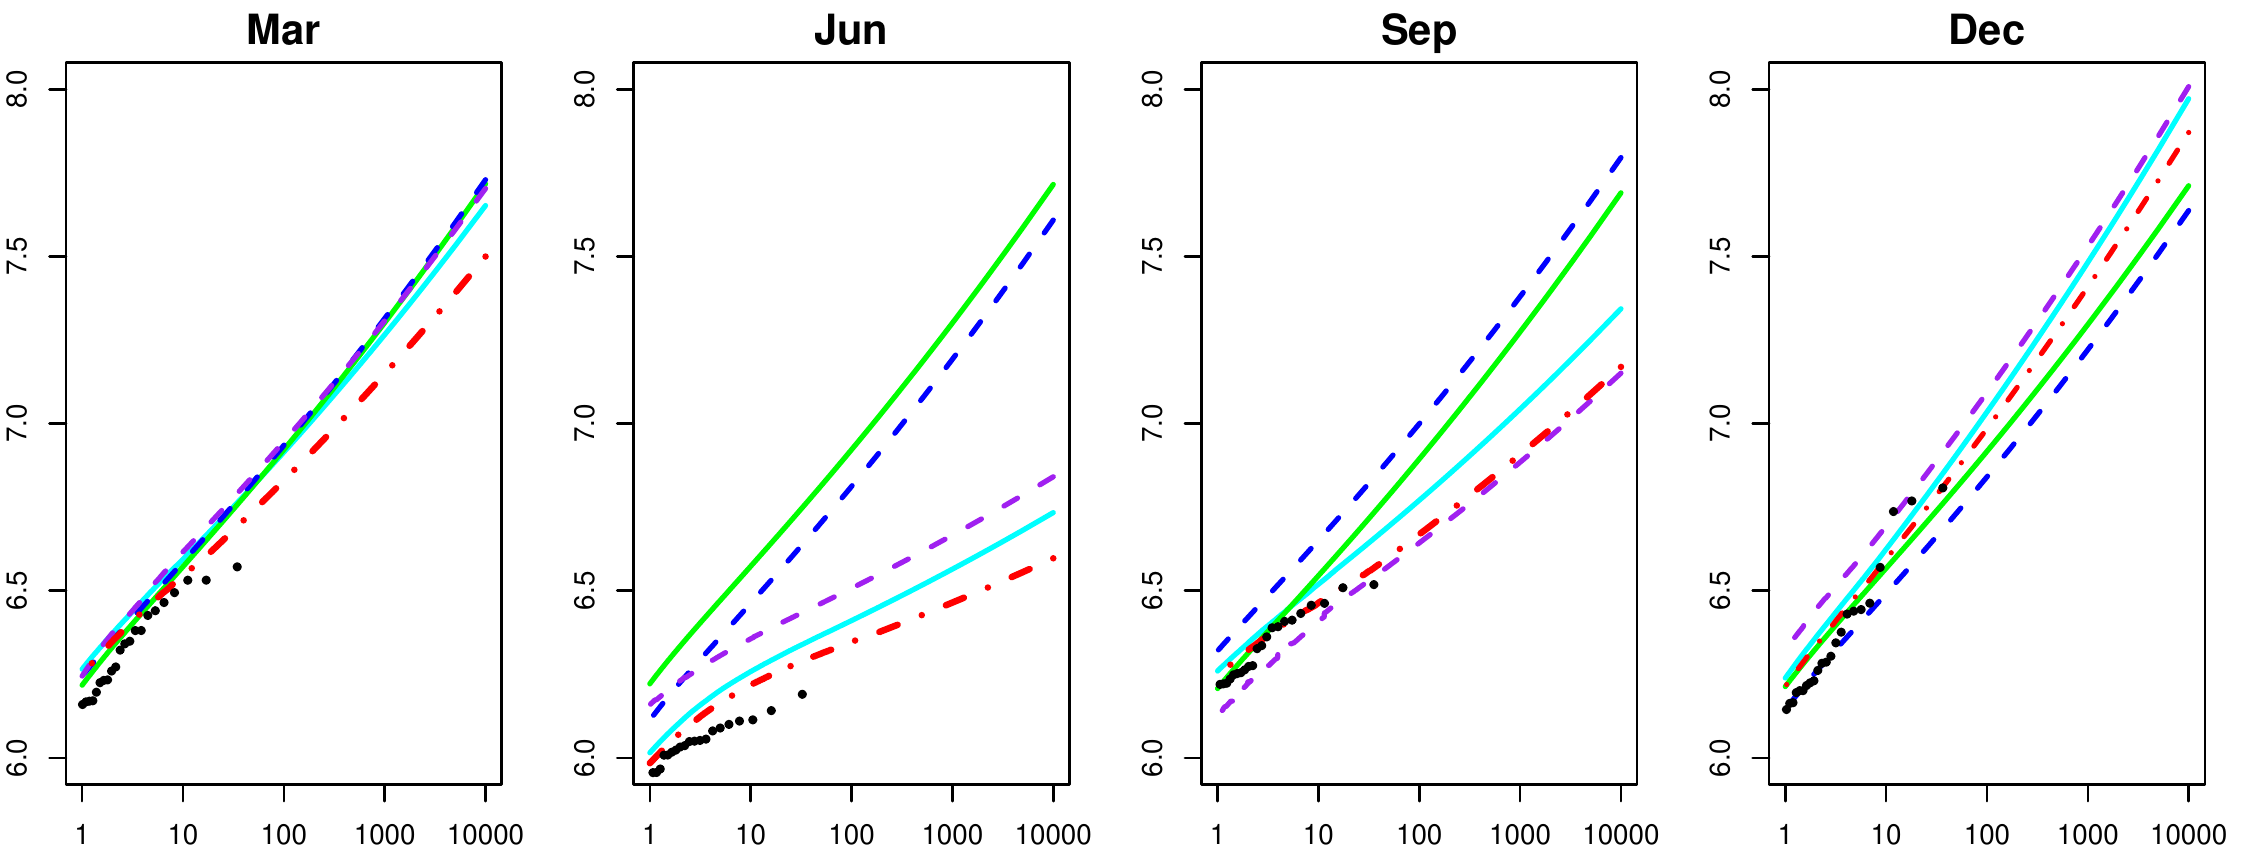} 
    \caption{Monthly sea level return level estimates for Heysham, Lowestoft, Newlyn and Sheerness (from top to bottom) in March, June, September and December, derived under \textit{baseline} (green), \textit{seasonal surge} (purple dashed), \textit{seasonal tide} (blue dashed), \textit{full seasonal} (cyan) methods and \textit{interaction} (red dot-dashed).}
    \label{fig::monmax_all_RL_NEW_1x4}
\end{figure}

\begin{figure}
    \centering 
    \includegraphics[width=0.49\textwidth]{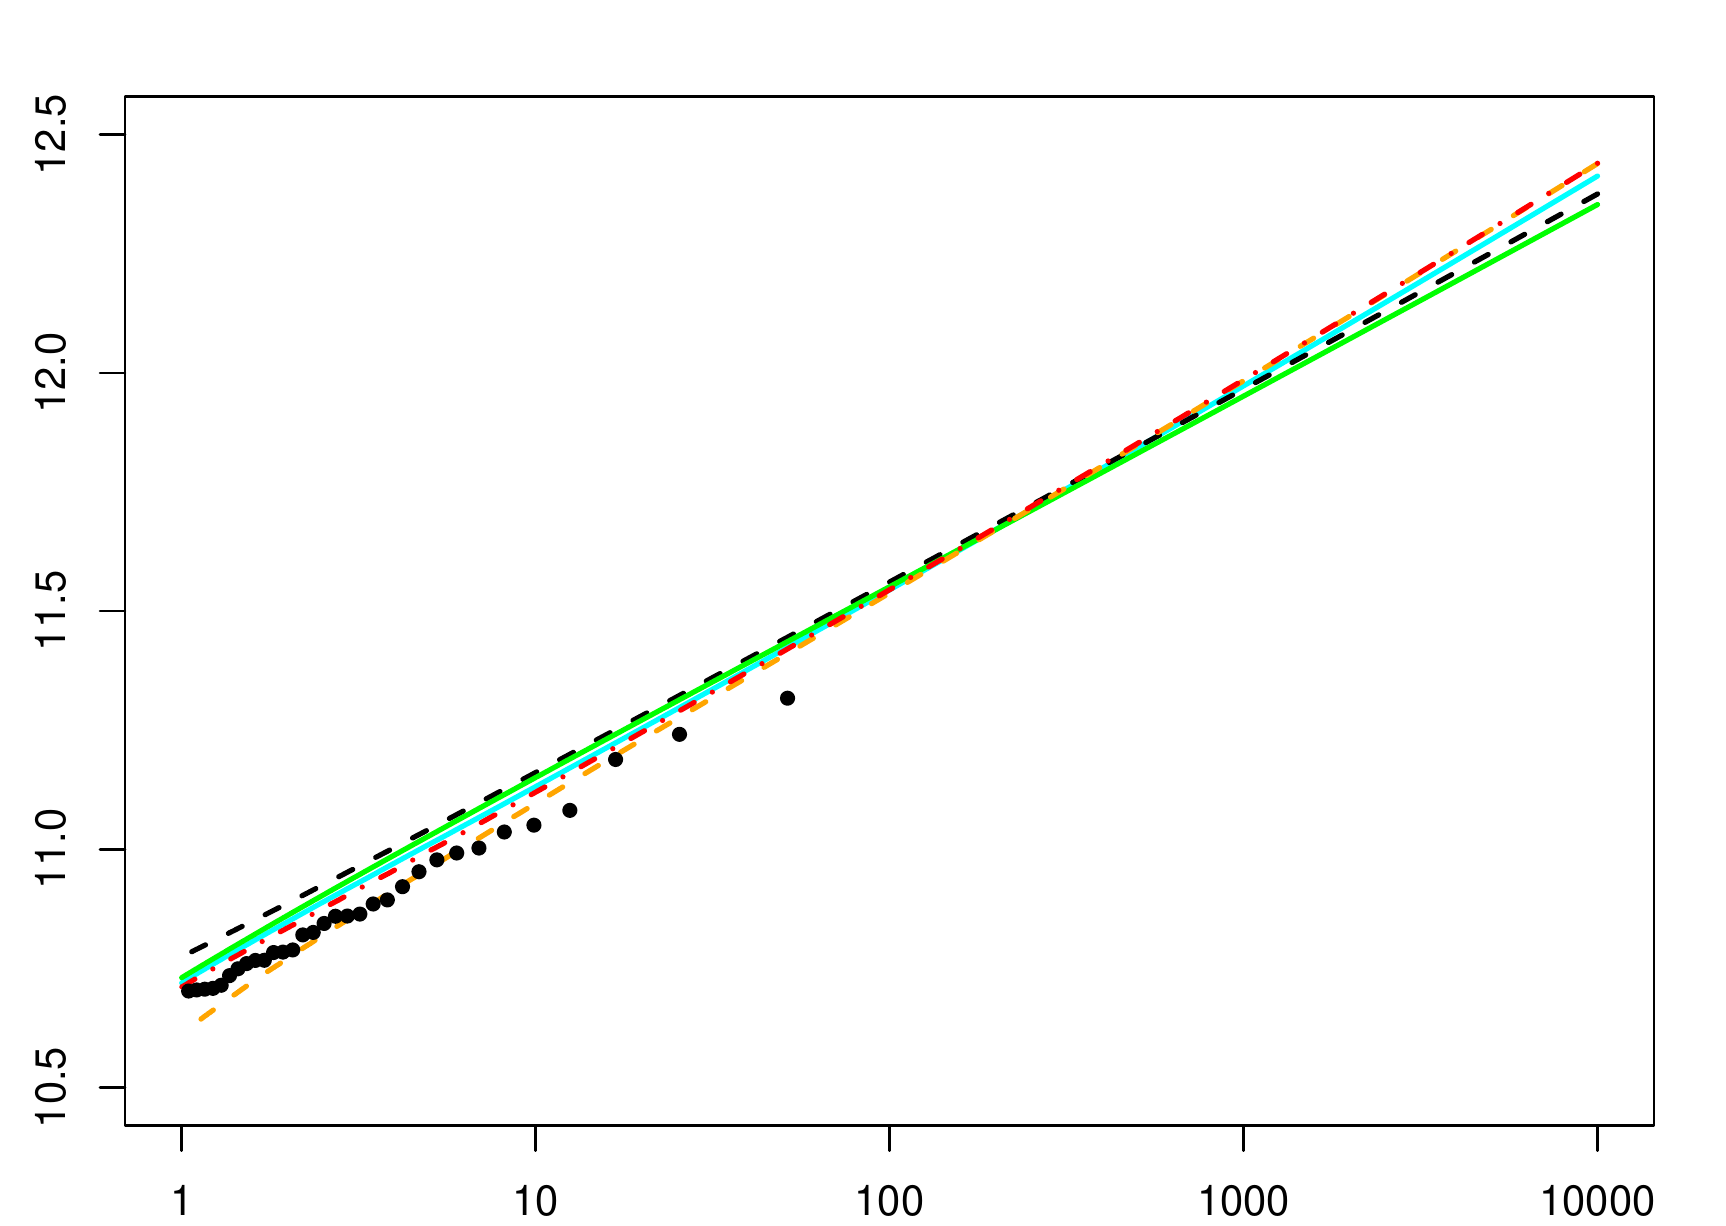}
    \includegraphics[width=0.49\textwidth]{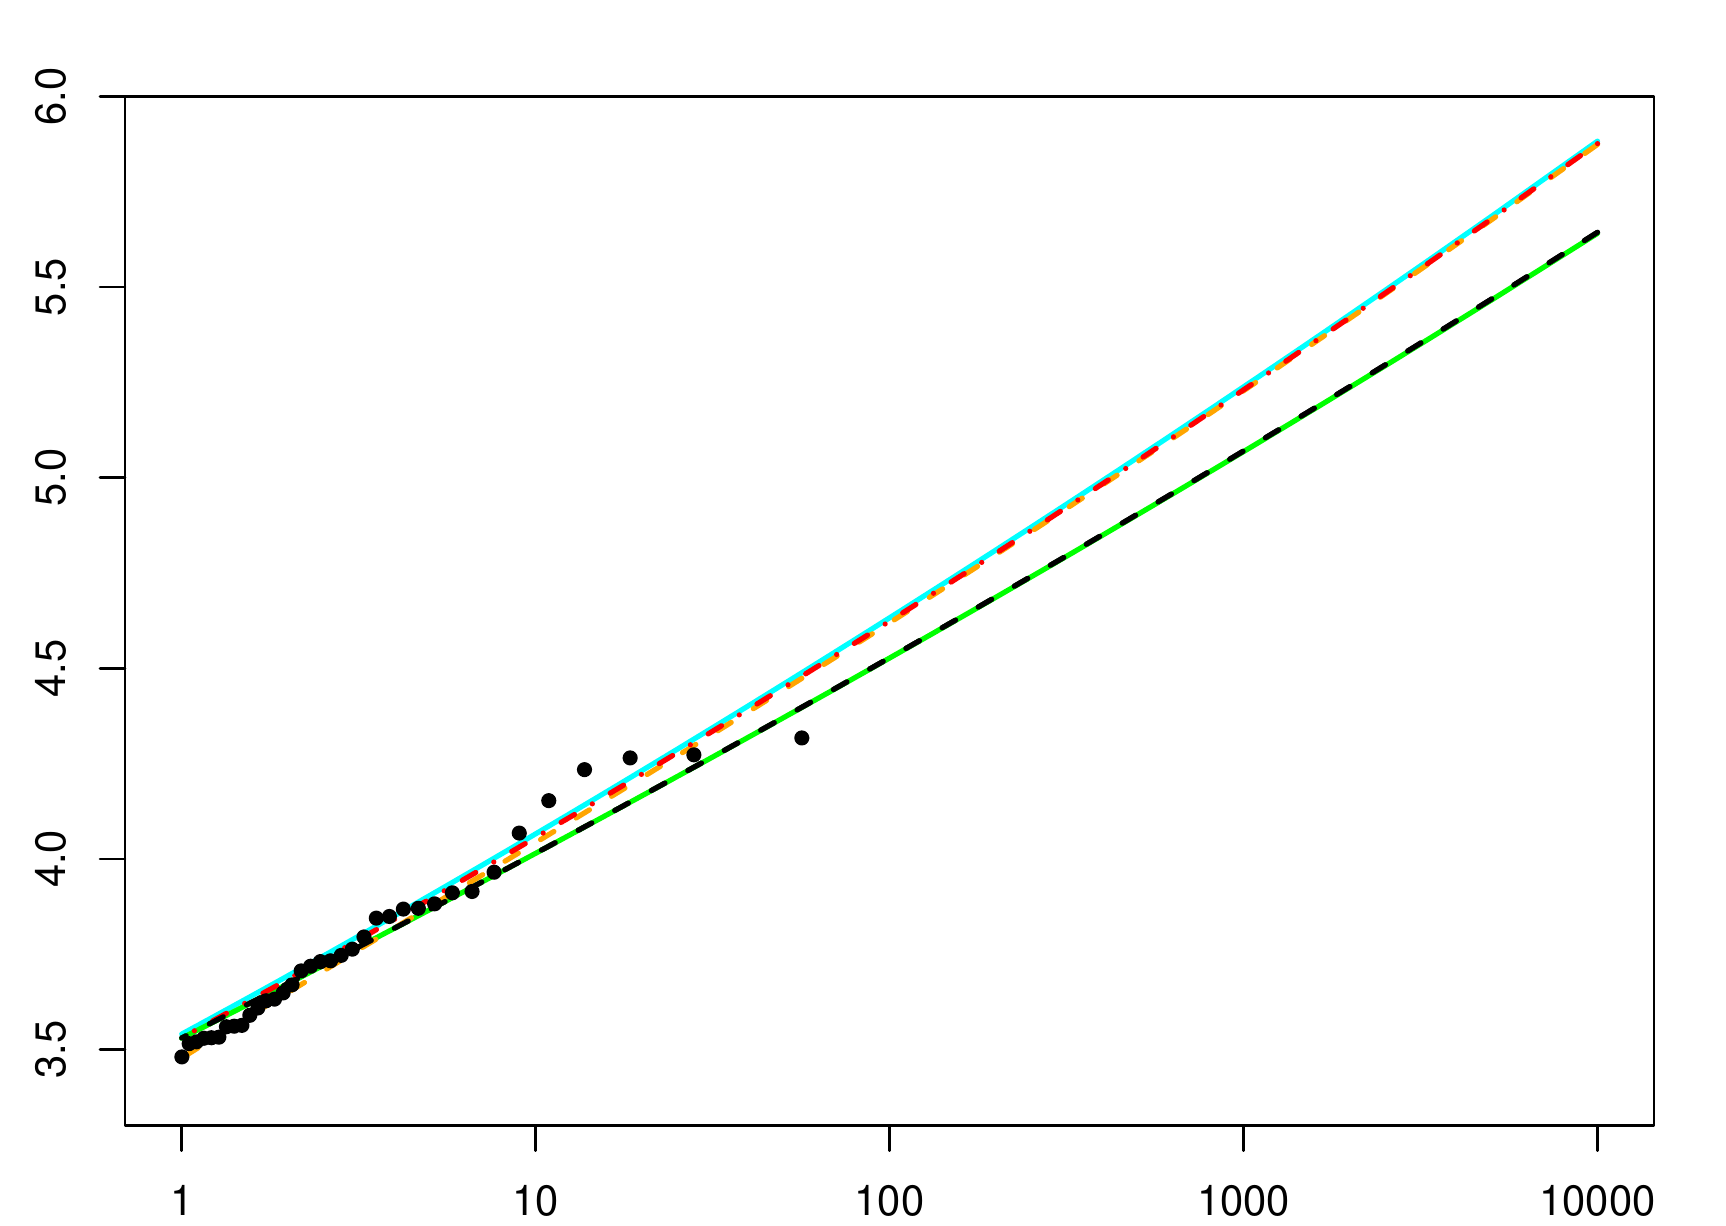} \\
    \includegraphics[width=0.49\textwidth]{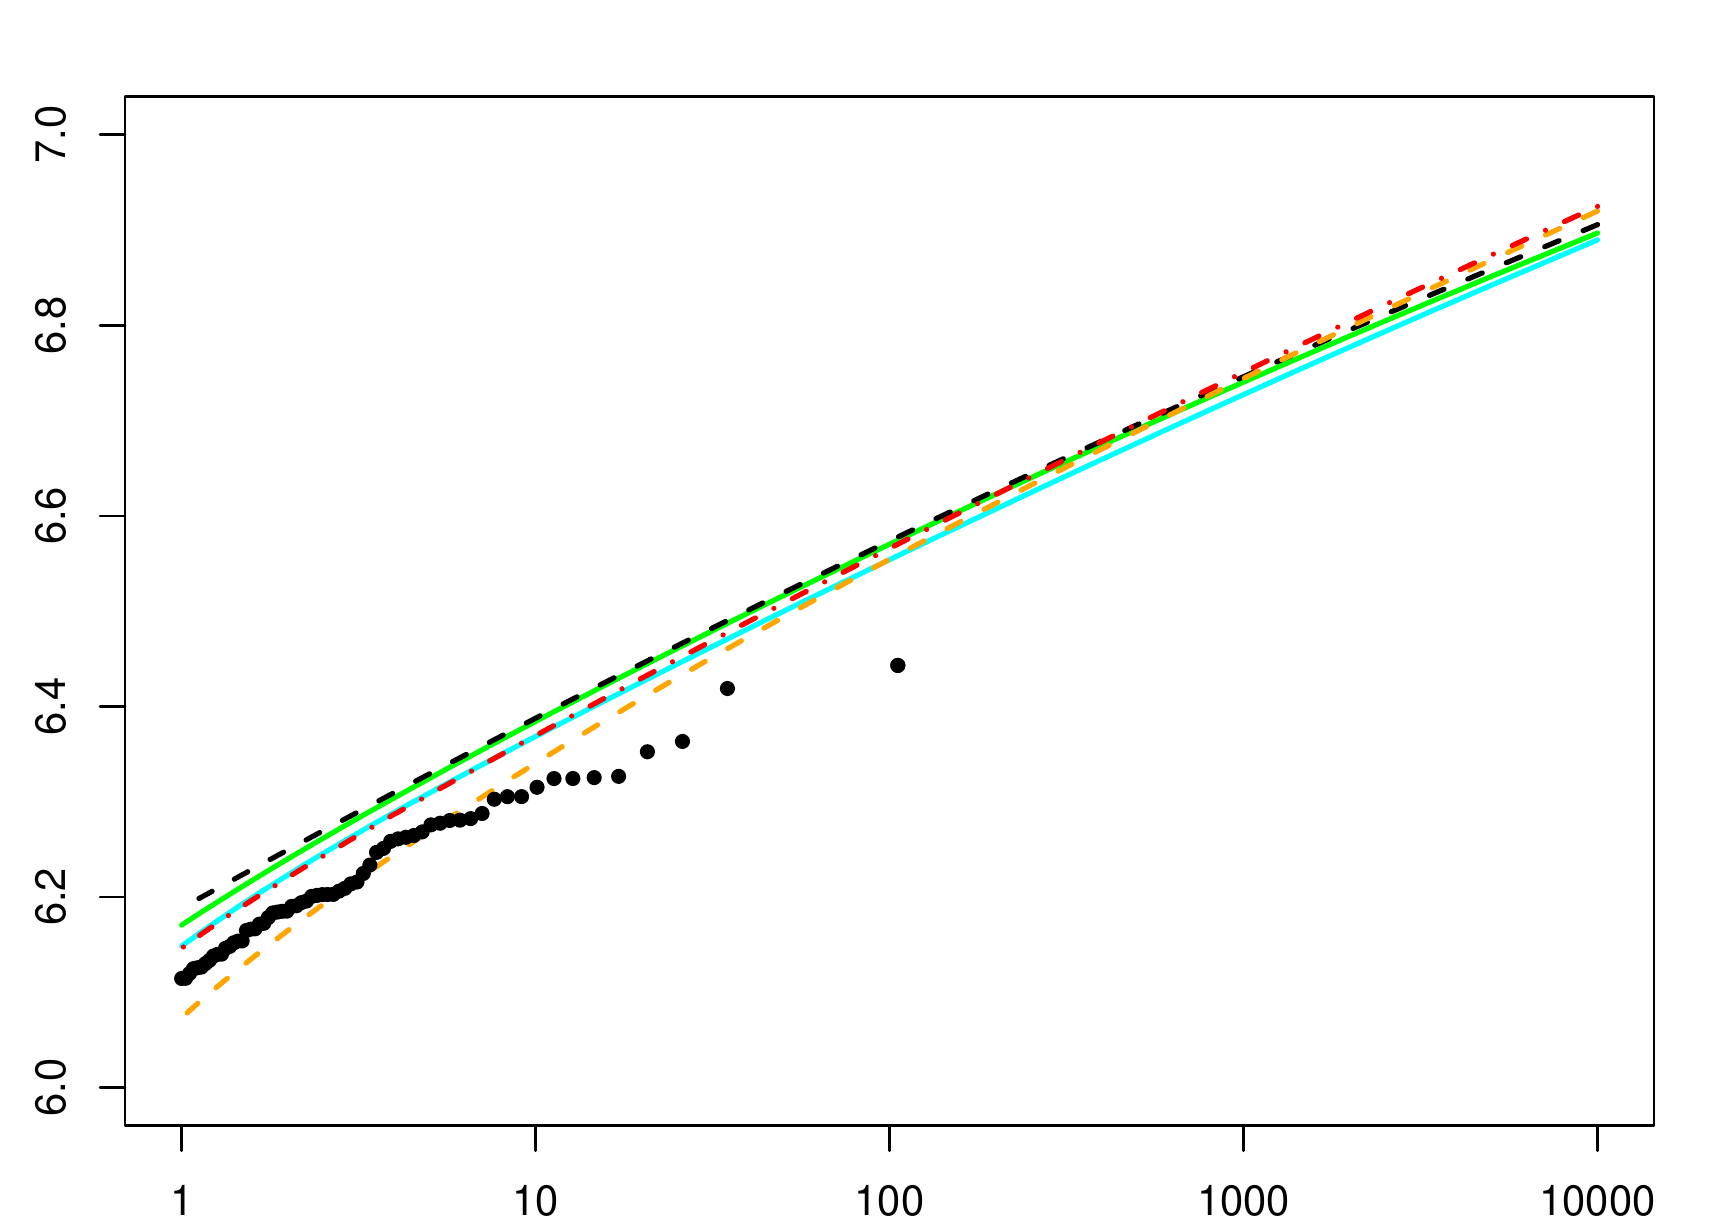}
    \includegraphics[width=0.49\textwidth]{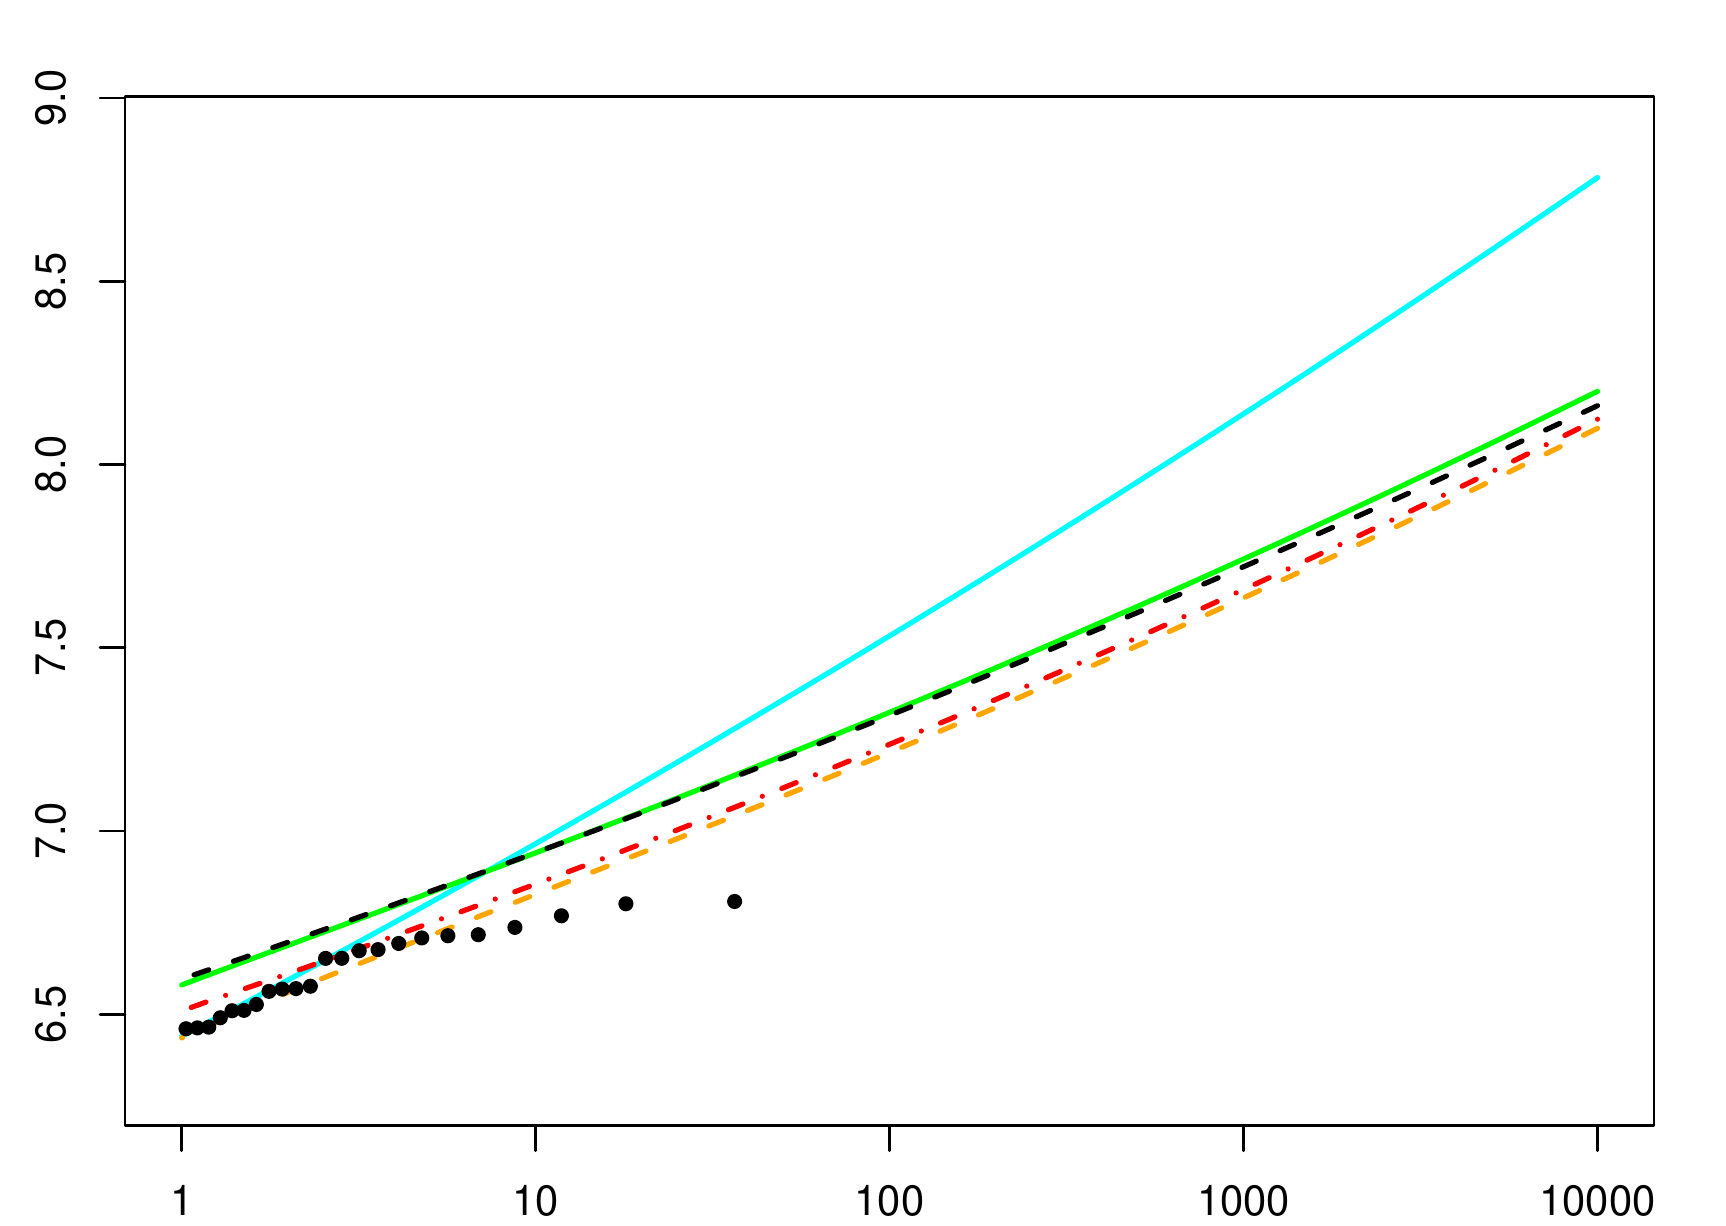} 
    \caption{Annual sea level return level estimates for Heysham (top left), Lowestoft (top right), Sheerness (bottom left) and Newlyn (bottom right) derived under \textit{current} (black dashed), \textit{baseline} (green), \textit{full seasonal} (cyan), \textit{interaction} (red dot-dashed) and \textit{temporal dependence} (orange dashed) methods, up to the 10,000 year level (right).}
    \label{fig::annmax_RL_NEW}
\end{figure}

\begin{figure}
    \centering
    \includegraphics[width=\textwidth]{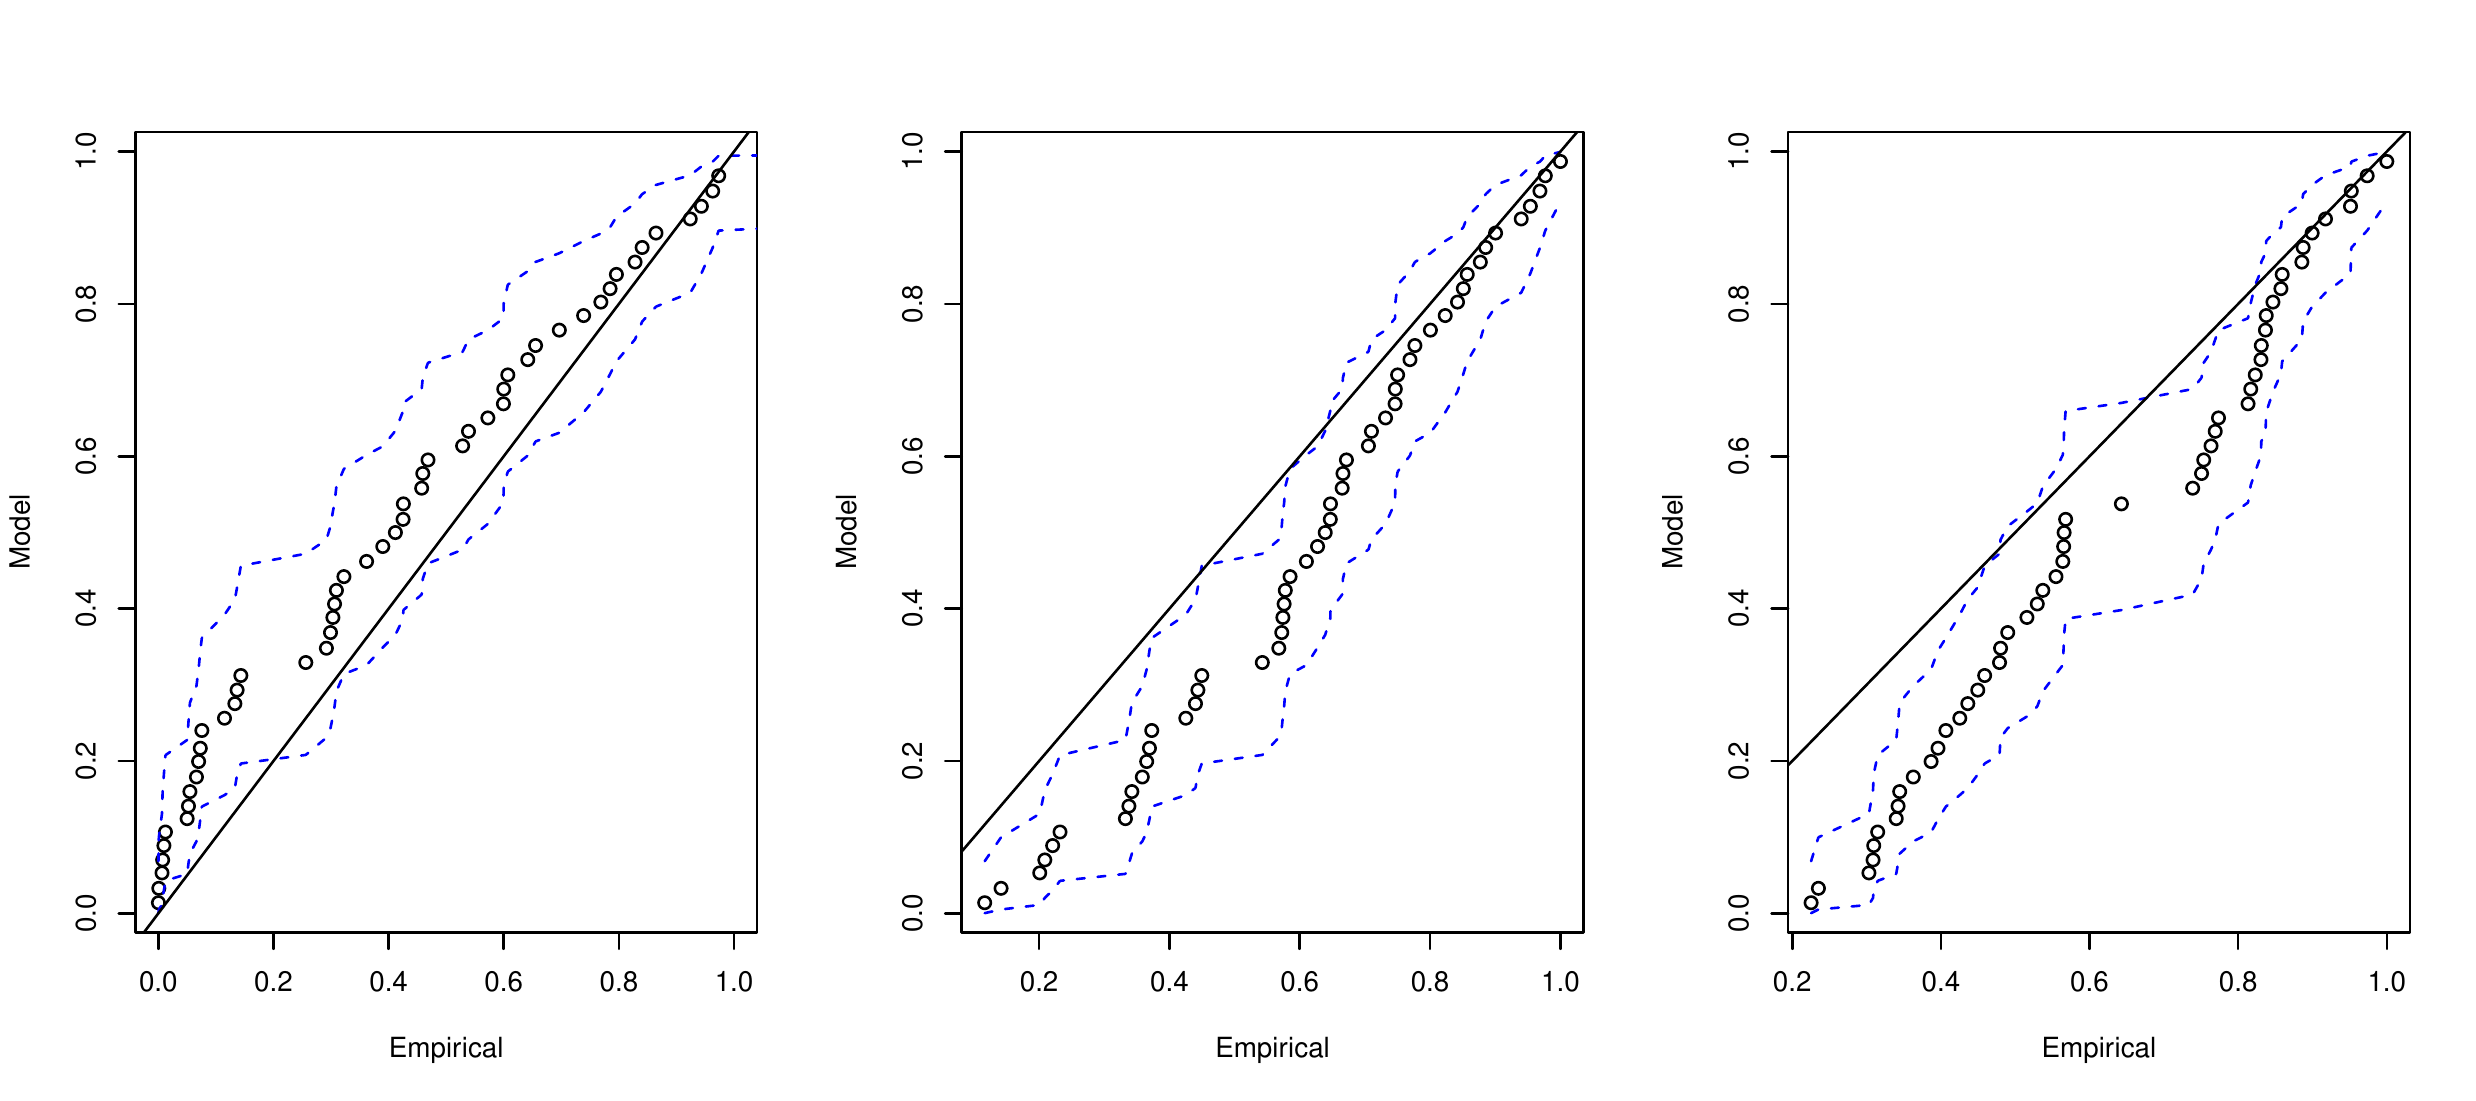}
    \includegraphics[width=\textwidth]{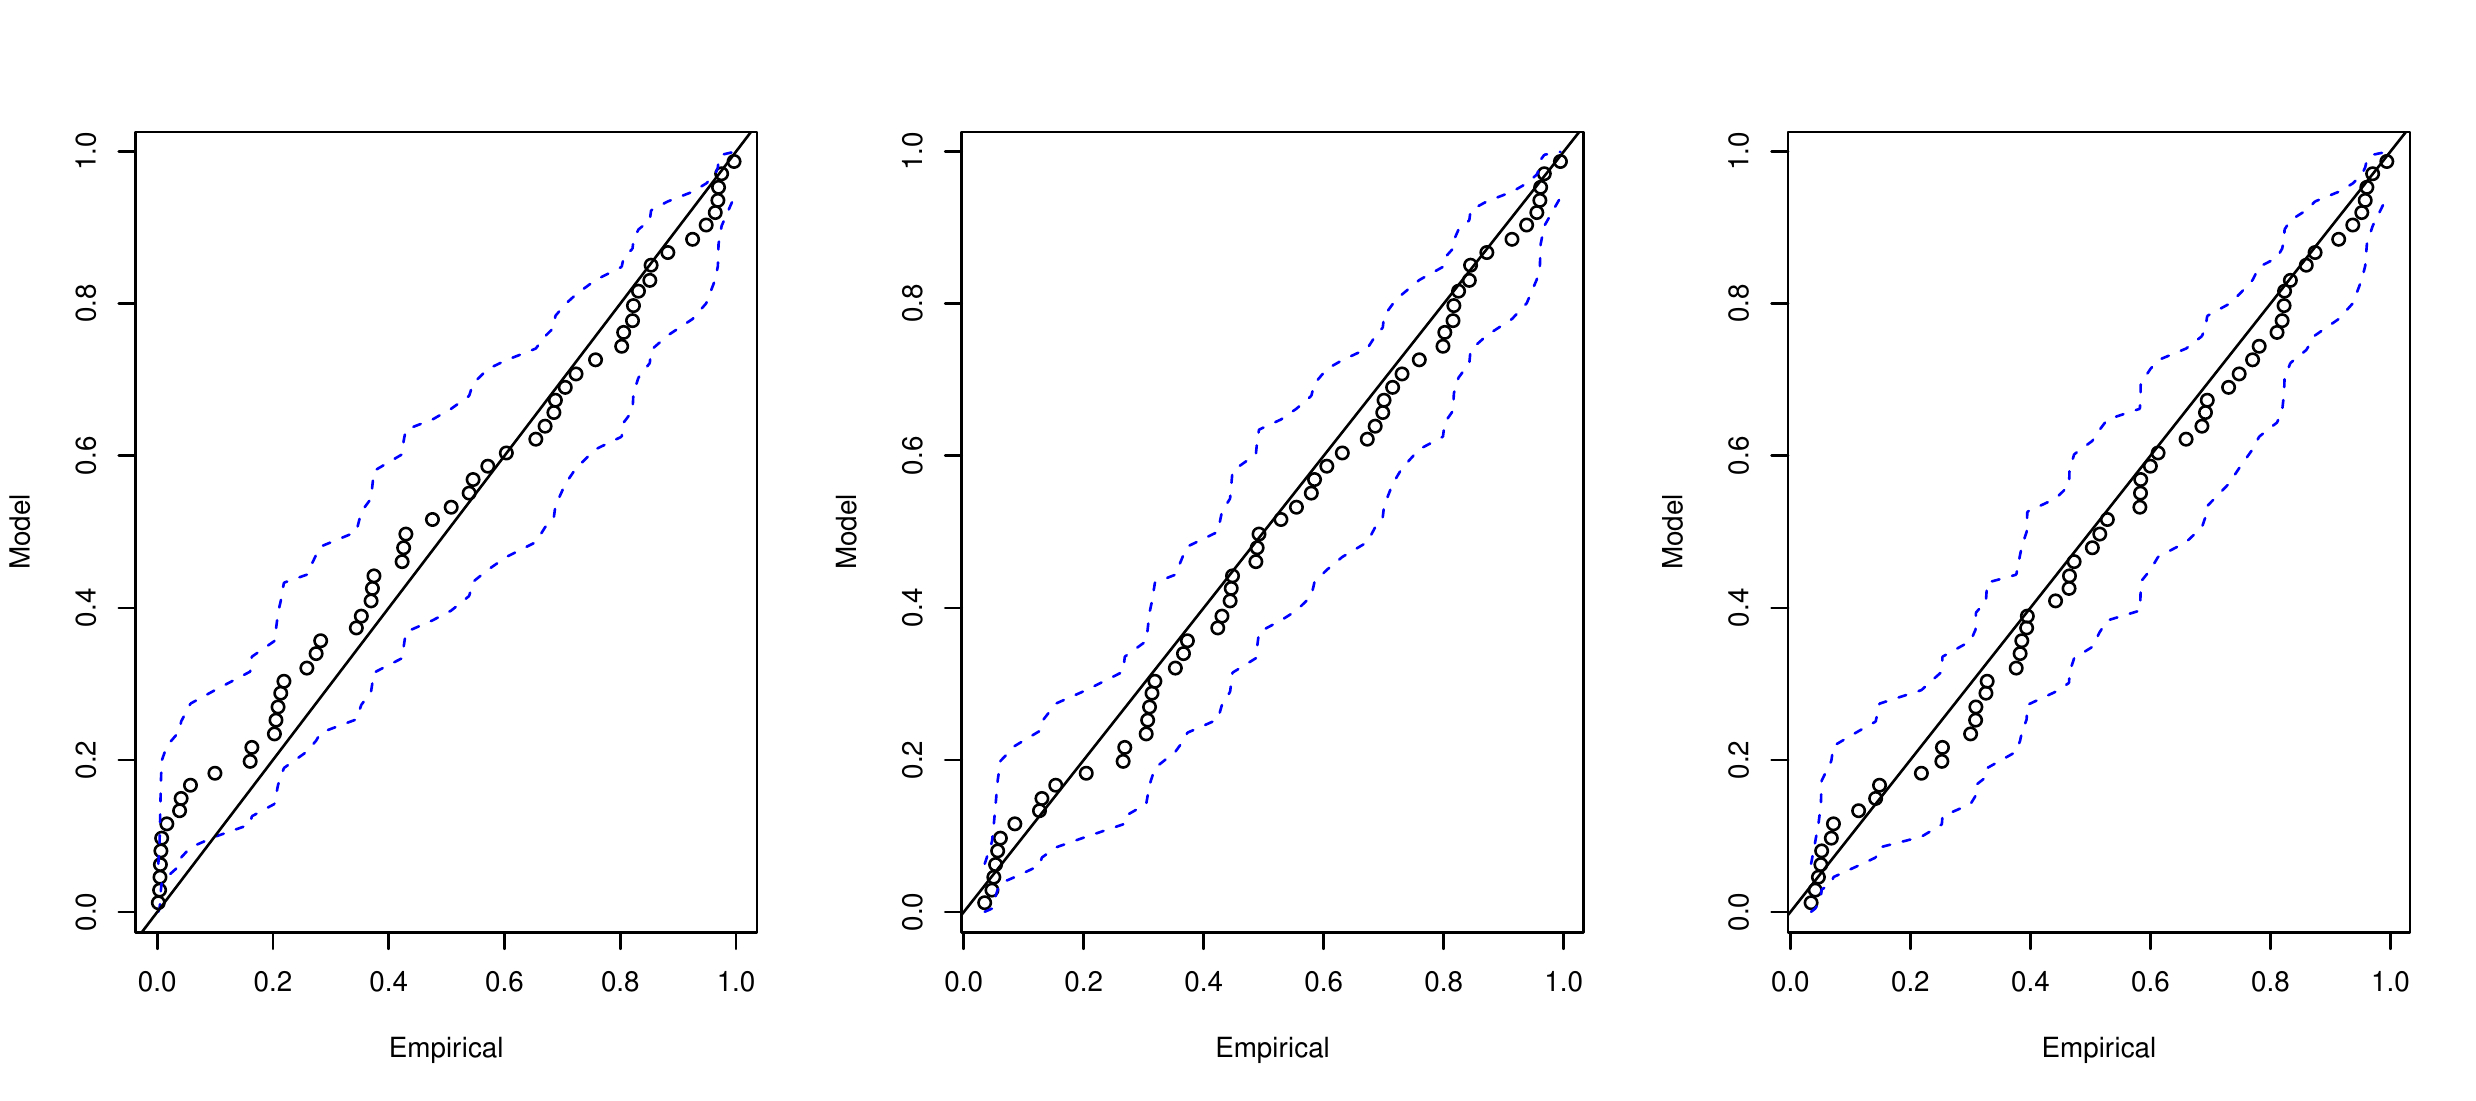}
    \includegraphics[width=\textwidth]{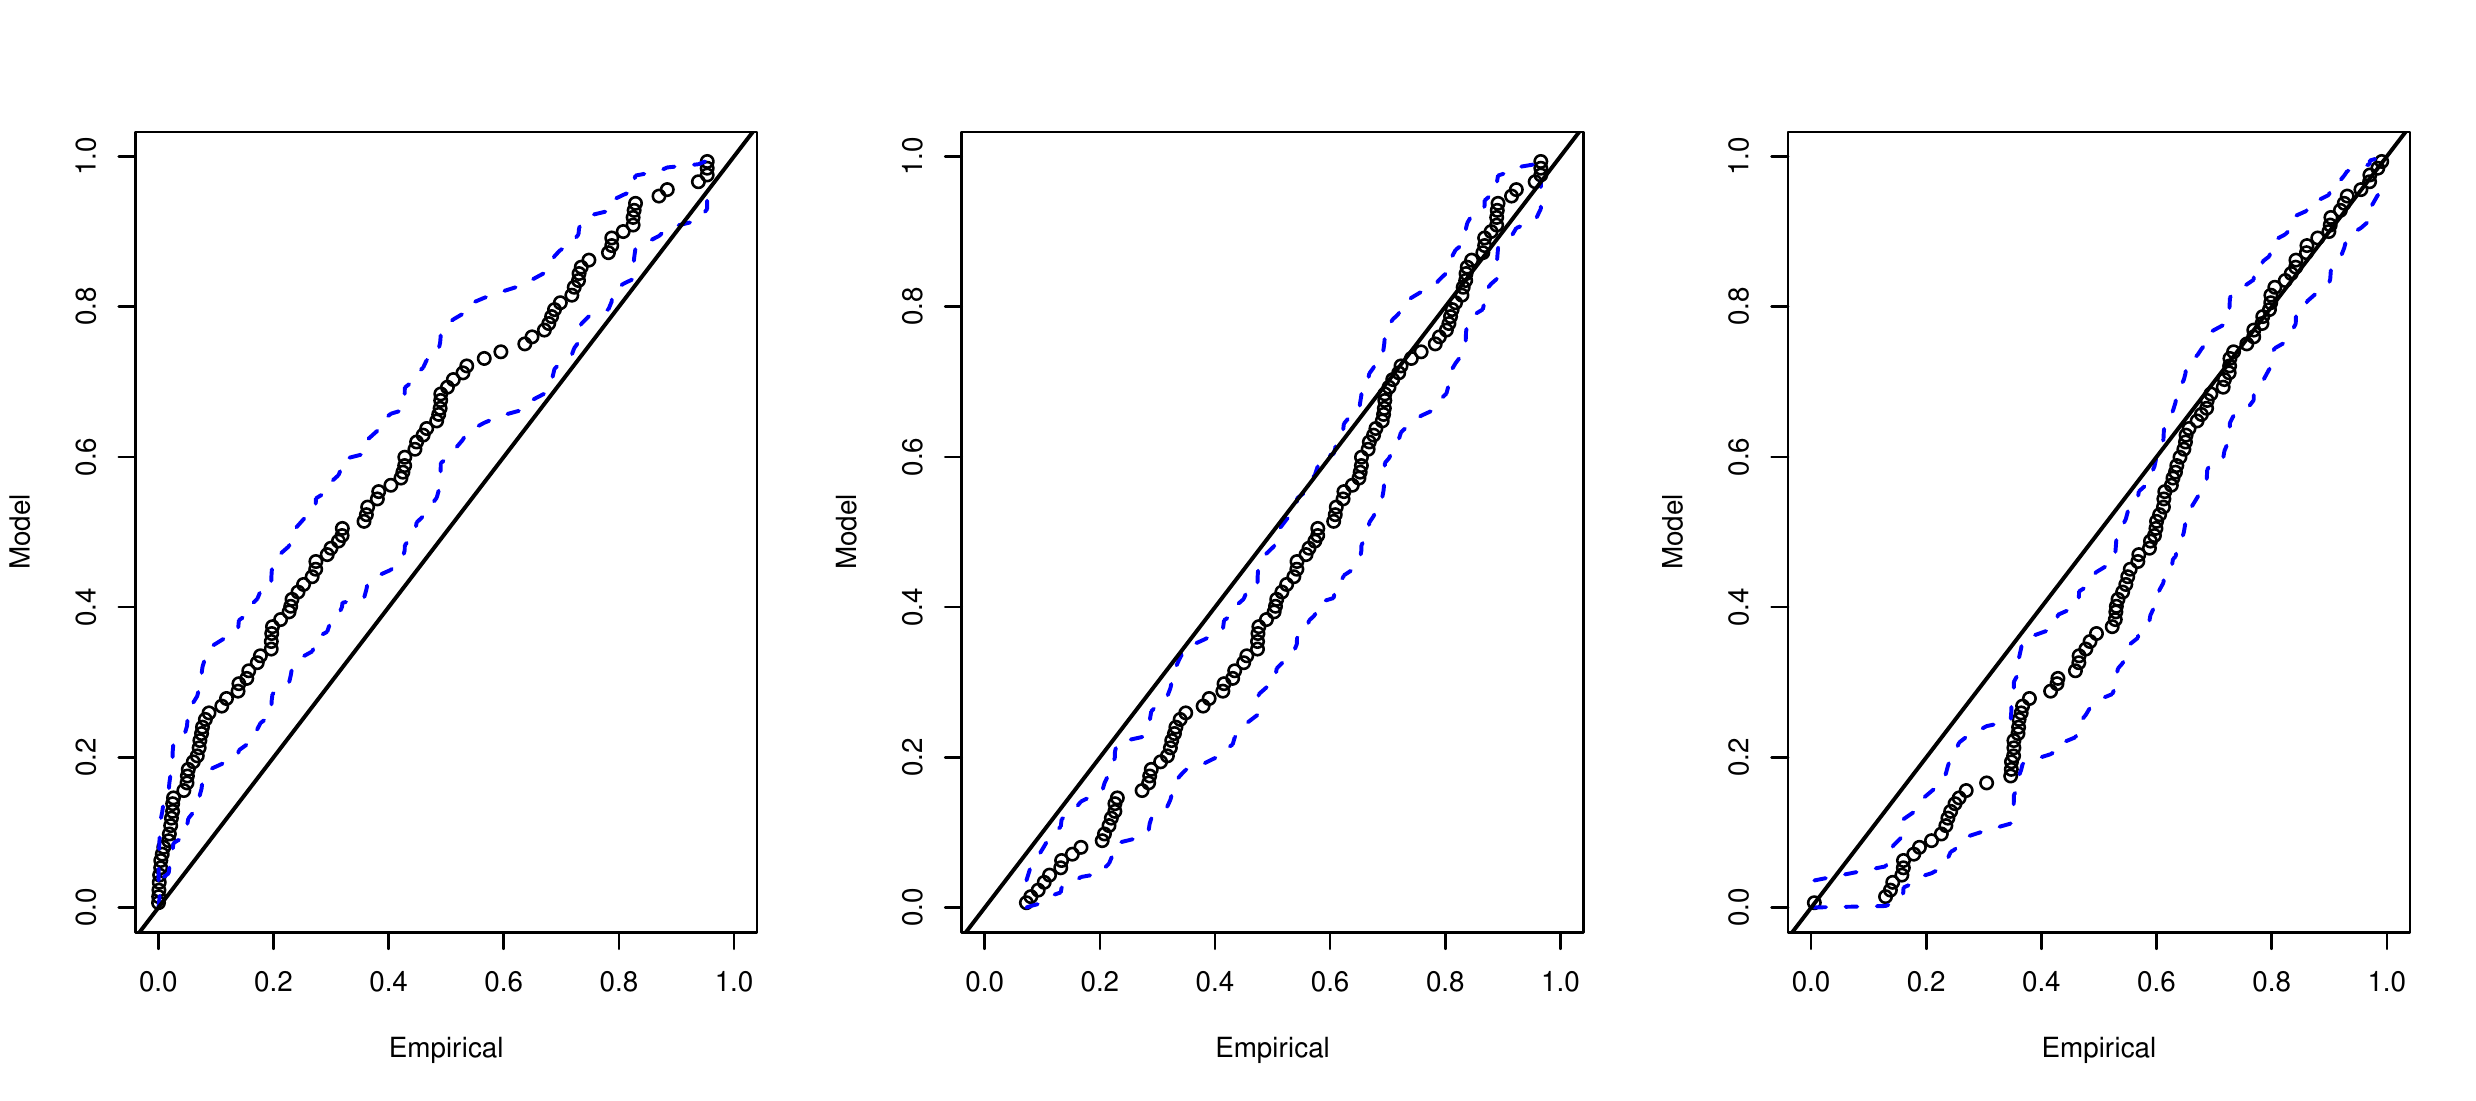}
    \caption{PP plots for the transformed annual maximum sea levels to a uniform scale at Heysham (top), Lowestoft (middle) and Newlyn (bottom). These are transformed using the \textit{baseline} (left) and final (\textit{temporal dependence}) (centre) distribution function for the annual maxima, as well as the year specific final model (right). The black line shows the line of equality, $y=x$.}
    \label{fig::mapannmax_all}
\end{figure}

\begin{figure}
    \centering
    \includegraphics[width=0.49\textwidth]{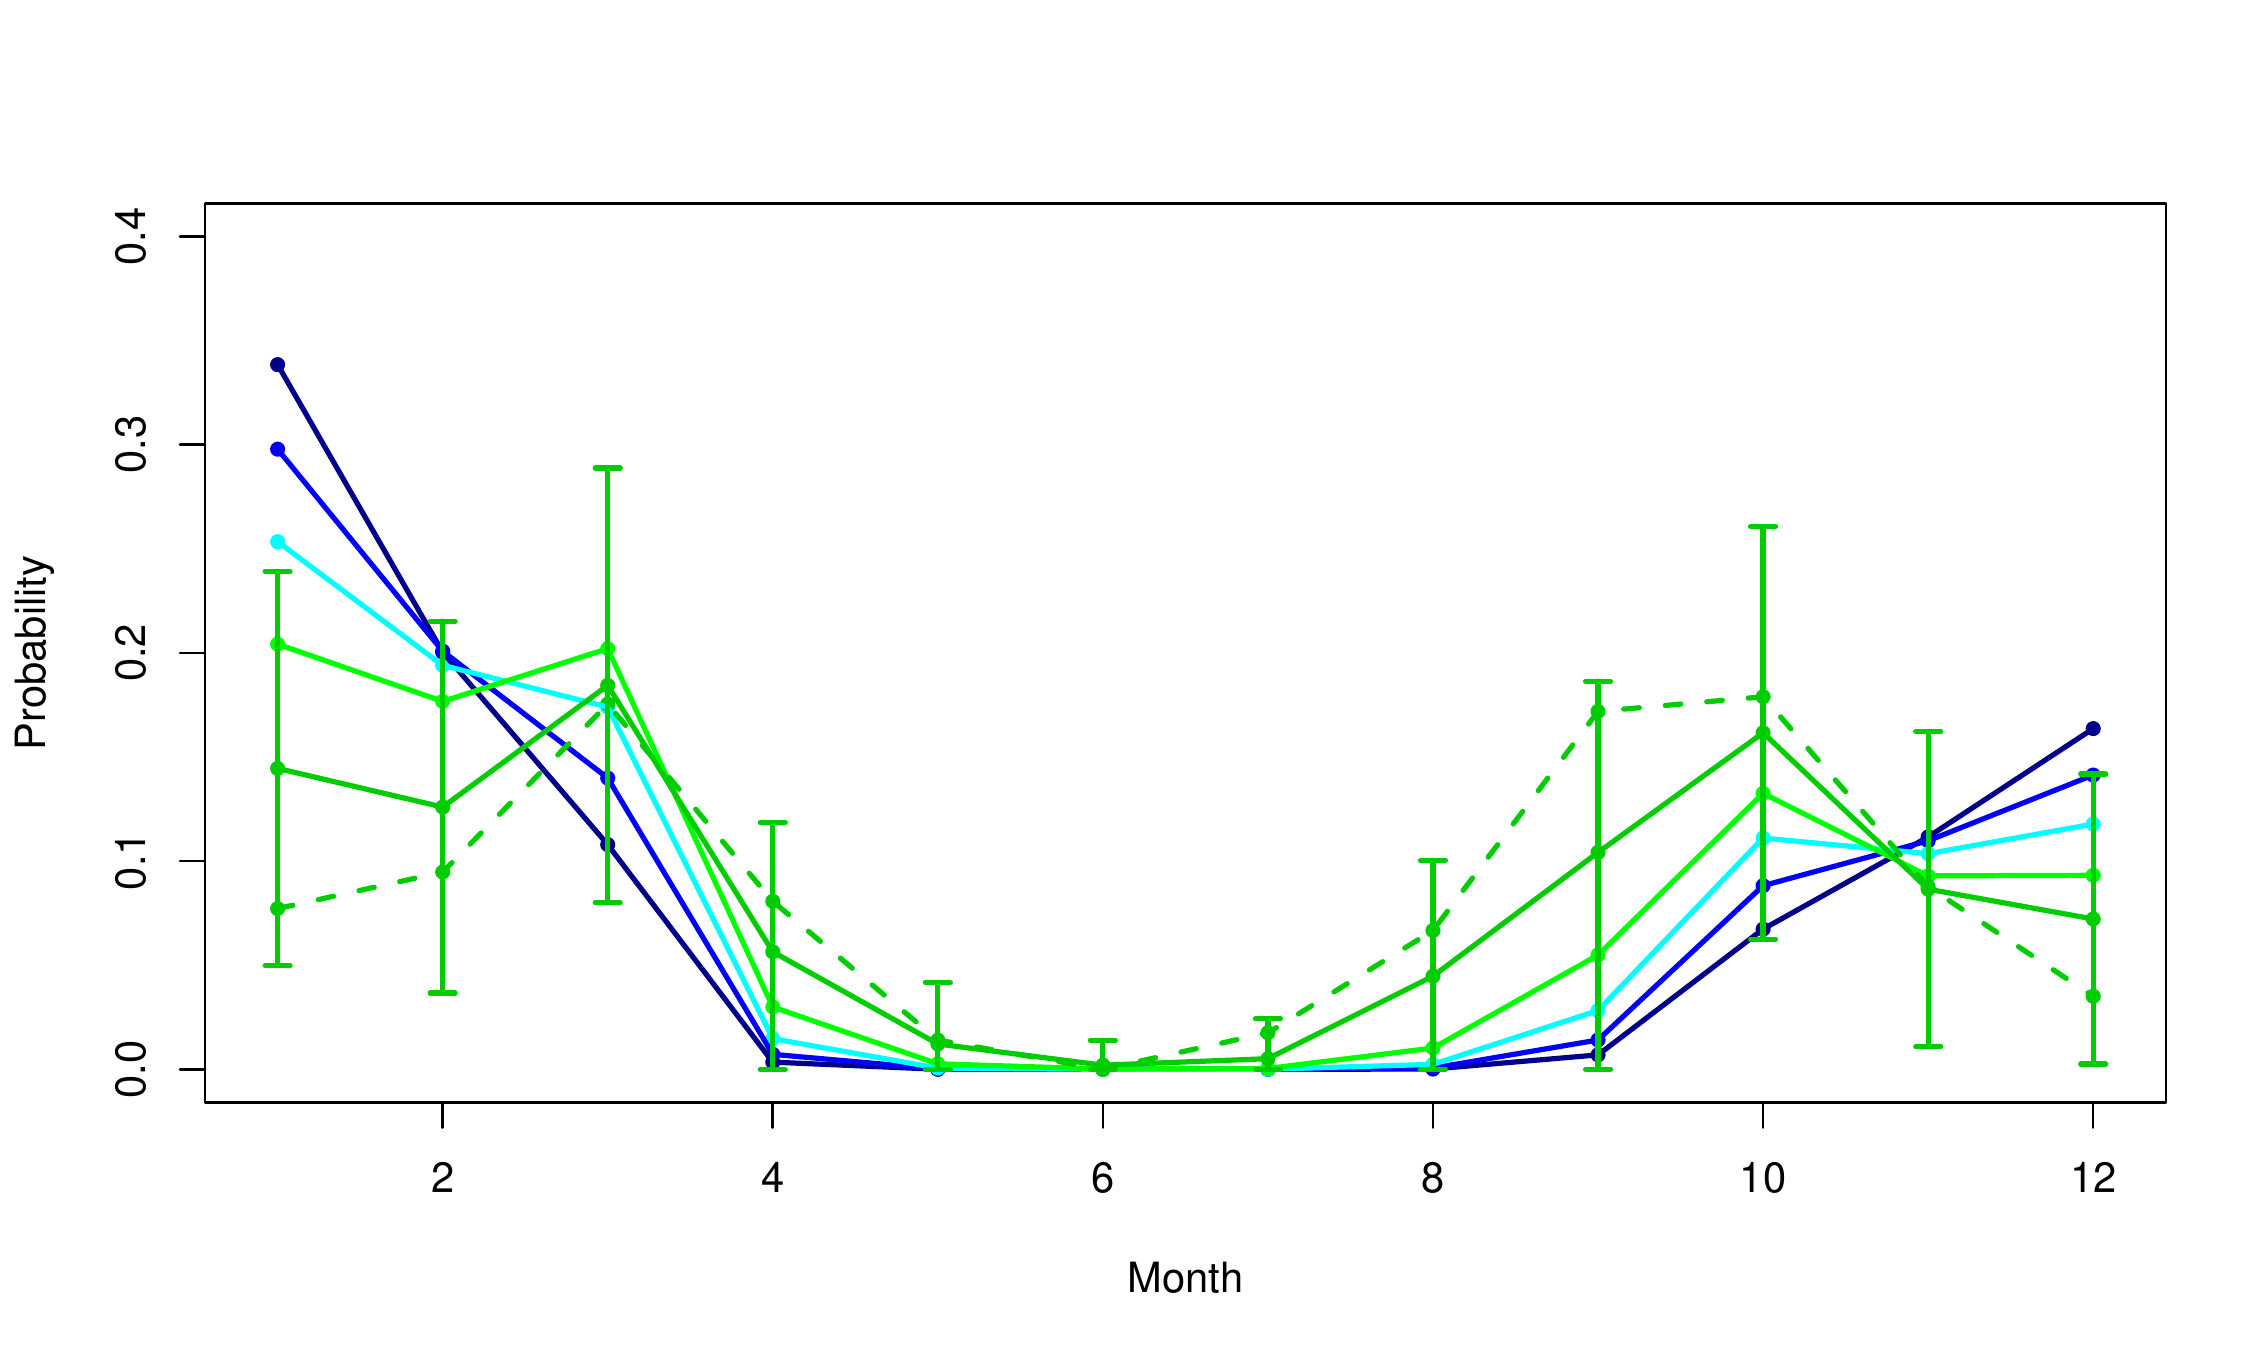}
    \includegraphics[width=0.49\textwidth]{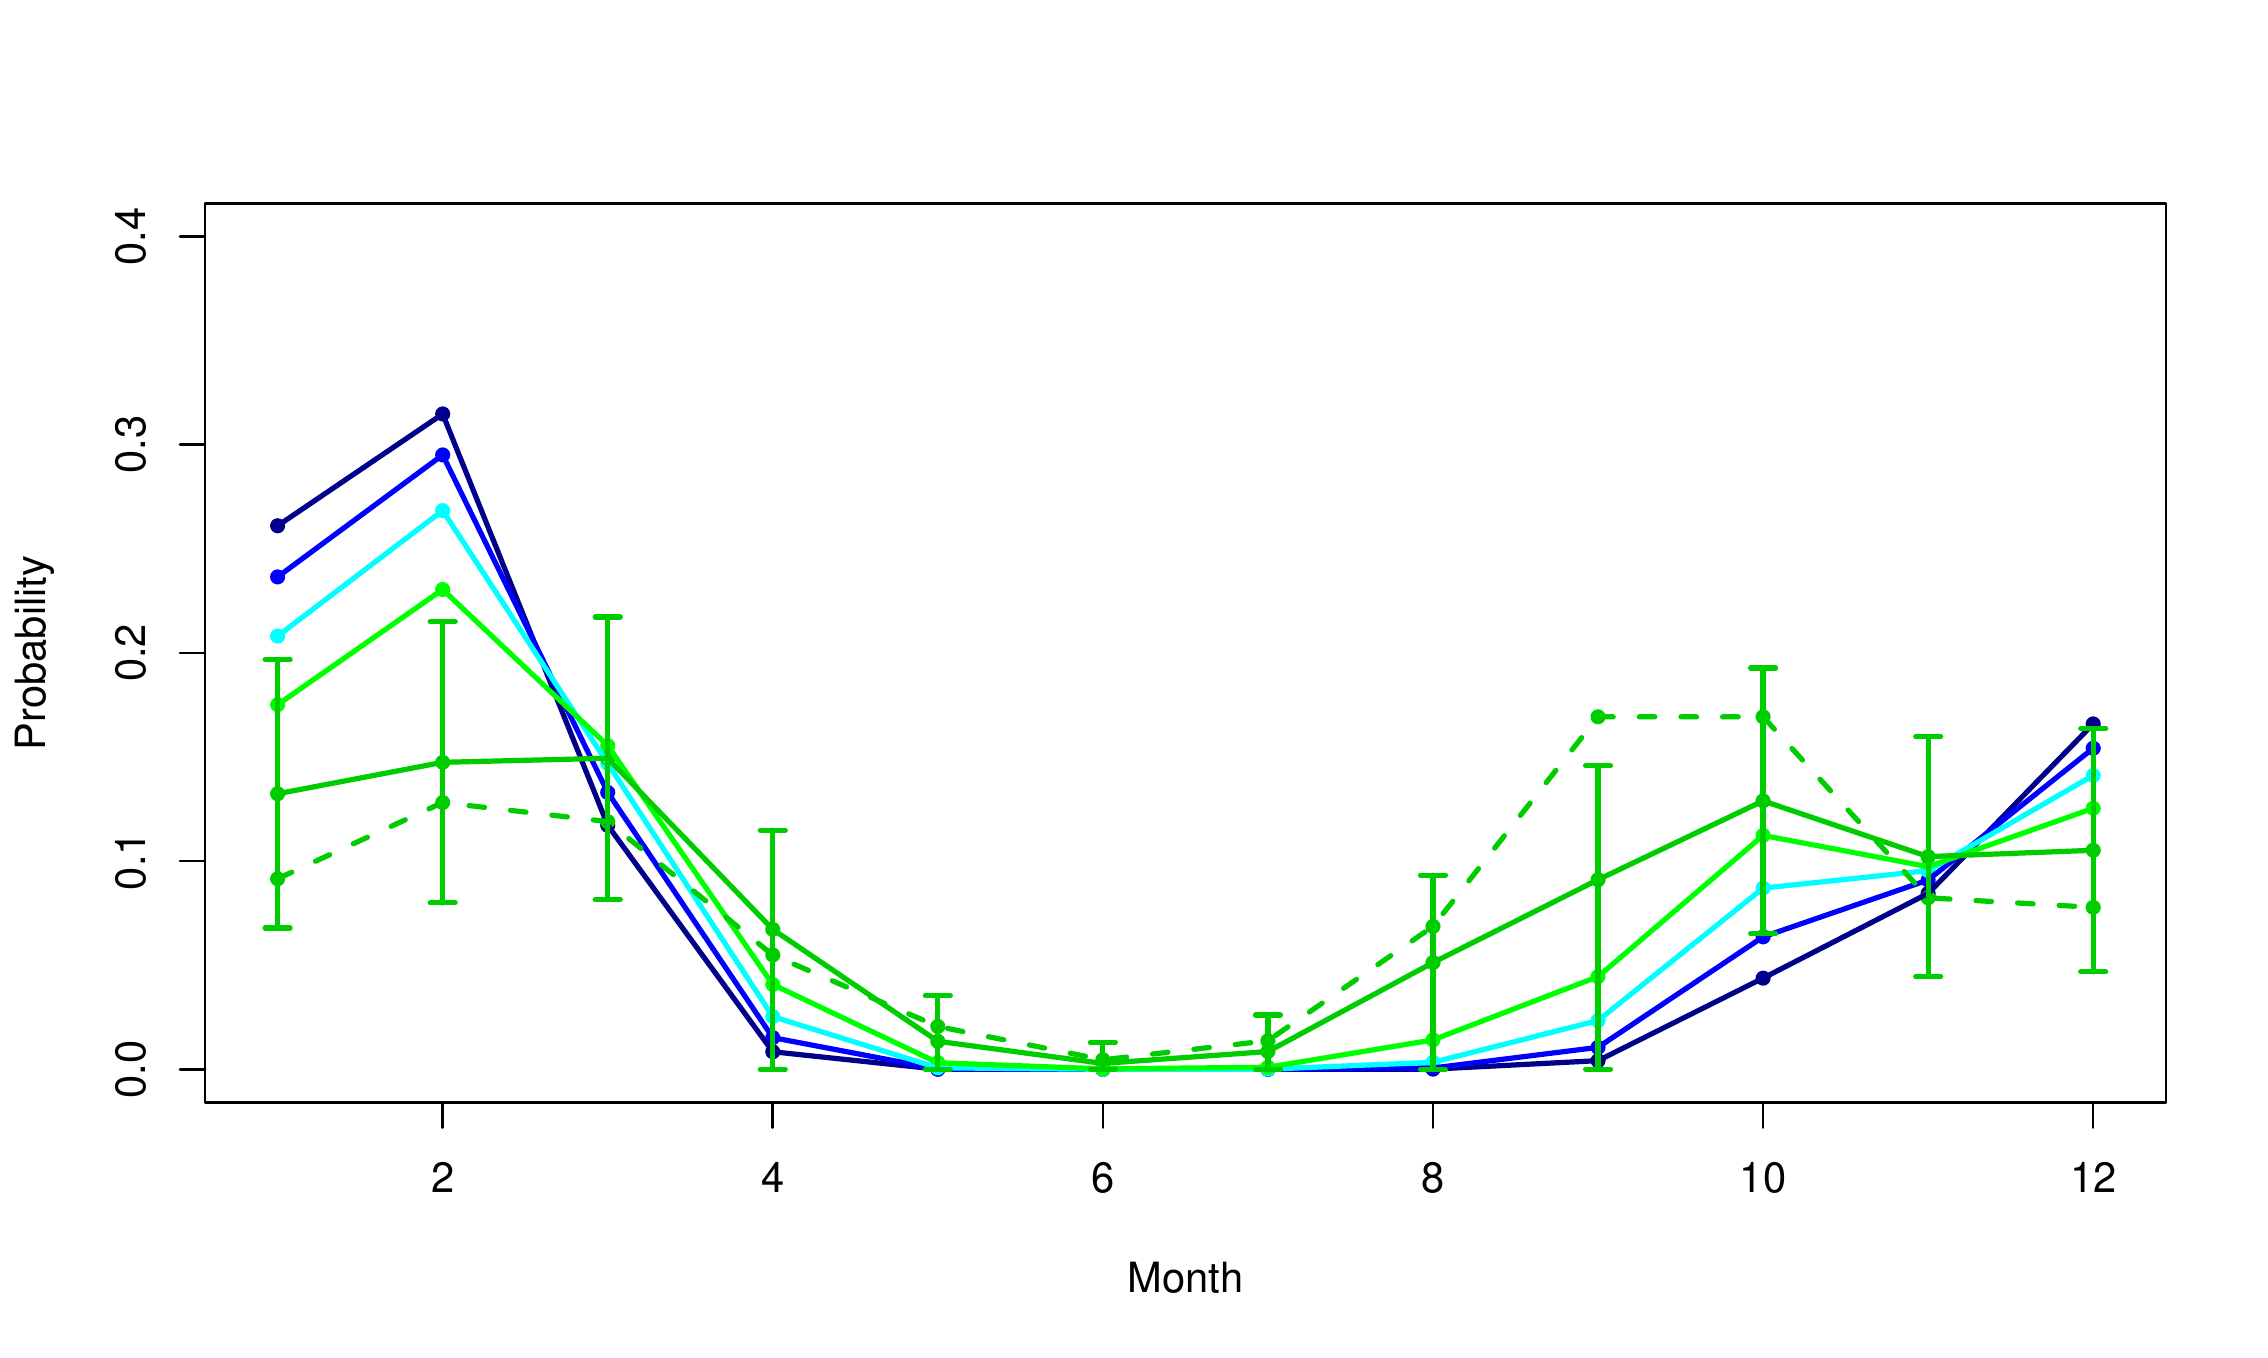}
    \caption{Estimates of $\hat P_M(j;z_p)$ for all months $j=1,\ldots,12$ at Heysham (left) and Newlyn (right), for $p=1$ (dark green), 0.1 (green), 0.01 (cyan), 0.001 (blue), and 0.0001 (dark blue). The dashed dark green line is the empirical estimate of $P_M(j;z_p)$ for $p=1$.}
    \label{fig::Annmaxprob_HEYNEW}
\end{figure}
